# Supplementary material for: A Formal Specification of Operating System based on ARINC 653
Source: arXiv:2206.14189 source file (2022-06-27)
Supplement: Supplementary file 1 [file Article_+_Appendix_50.pdf]

# A Formal Specification of Operating System based on ARINC 653

Ziyan Wang<sup>1</sup> and Yan Zhang<sup>2</sup> \*

<sup>1,2</sup> College of Information Science and Technology  
Nanjing Forestry University, P. R. China

June 27, 2022

## Abstract

In this paper, by using the formal language *Circus*, we give a formal specification of an operating system based on ARINC 653 standard. Our specification includes interrupt handling, time and memory management, partition and process scheduling, system call response and related APEX services. Especially, the concurrent behaviours of partitions and processes are also specified.

## 1 Introduction

### 1.1 ARINC 653

In avionic industry, a new architecture of embedded real-time operating system called Integrated Modular Avionics (IMA) has gradually become the mainstream. Compared with old avionic architectures, IMA enables a variety of applications to execute on the same hardware and significantly reduces the power requirements, weight and costs of maintenance.

The guidelines for the design of IMA architecture have been developed by Aeronautical Radio Incorporated (ARINC). It is known as ARINC 653 [14] and first released in 1997. The document proposes the baselines of operating environment for application software used in IMA architecture by defining a general-purpose APEX (APplication/EXecutive) interface between the operating system and application software. It also ensures the portability that application software, which uses the APEX interface, can execute on any operating system based on ARINC 653 standard.

The most important part of an IMA is ARINC 653 module. Figure 1 is the typical architecture of it. As shown in Figure 1, an integrated module contains a core module and application software running on it. The core module is composed of core hardware and core software.

An ARINC 653 module is divided into five layers: Core Hardware, Hardware Interface Software, ARINC 653 O/S, APEX and Application Software. The bottom layer Core Hardware is a layer of hardware units including CPU, MMU, clock, interrupt controller and etc. This layer provides hardware foundations for all the software of ARINC 653 architecture. The three layers in the middle make up the core software in an ARINC 653 module. The layer above Core Hardware is Hardware Interface Software, which provides functions to manipulate hardware units. ARINC 653 O/S layer is the most important part of the system because it makes decisions on scheduling and provides system calls to support the functions in APEX layer. There are also many functional modules in this layer, like Exception Handler and Health Monitor. APEX, which is similar to API in general-purpose operating system, provides an interface for application software.

The philosophy of ARINC 653 is partitioning. Applications resident in a module are partitioned with respect to space (spatial partitioning) and time (temporal partitioning). To support spatial partitioning, each partition is allocated with an amount of space in memory where the application of the partition resides. The space of each partition is specified during system configuration and initialization. To support temporal partitioning, the operating system maintains a major time frame of fixed duration, which is periodically repeated throughout the module's run

---

\*This work received financial support of the Youth Program of National Natural Science Foundation of China (No 61802191). Corresponding authors: 821651646@qq.com and zhangyan@njfu.edu.cn.

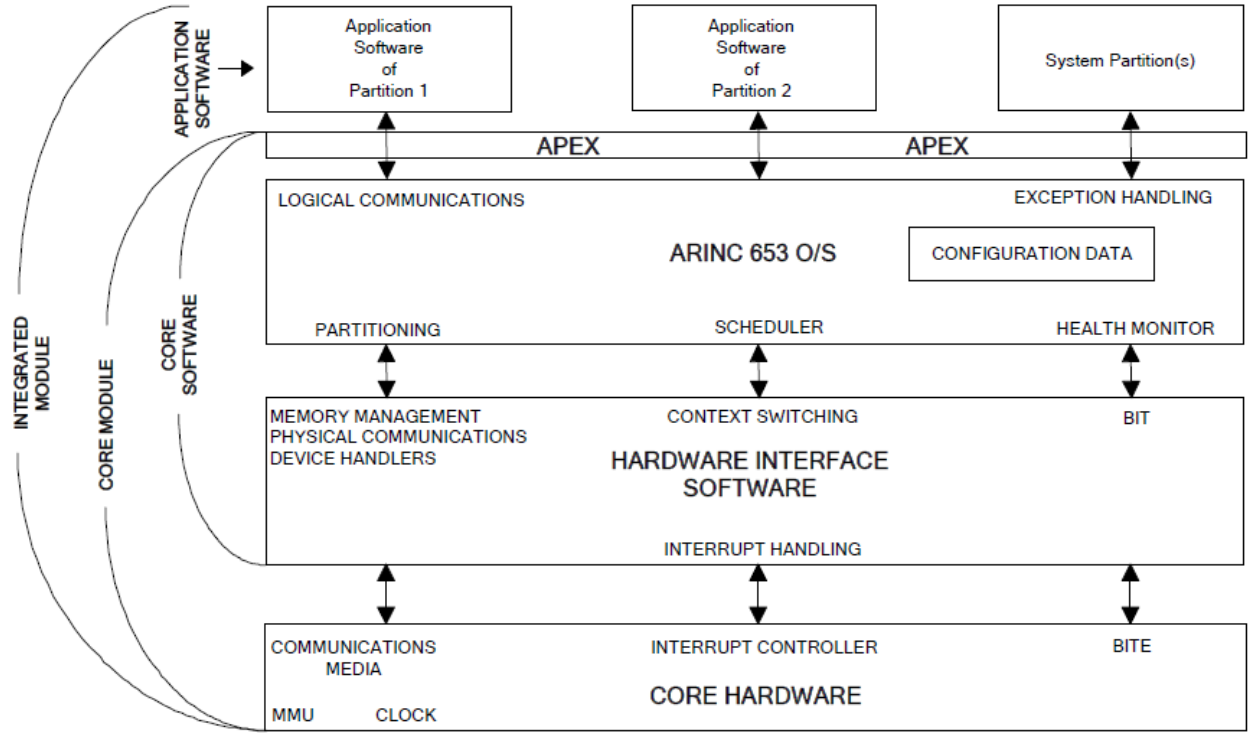

Figure 1: Architecture of ARINC 653 Module

time. Each partition is allocated with one or more time windows within a major time frame. The application of each partition is accessible to resources only during its own time window.

In ARINC 653, a partition comprises one or more processes that operate alone or cooperate with each other to provide functions of the application. The processes in a partition which are scheduled according to their priority can be divided into two kinds: aperiodic and periodic. Each process is also associated with a deadline time before which the process should finish its execution if its deadline time is set to a finite value.

## 1.2 Circus

Circus [10, 11, 17] is a formal language that combines Z [15], CSP [8], Morgan's specification statements, and Dijkstra's guarded commands. One main advantage of Circus is that the states and behaviours of a process can be captured in the same specification. It can be used for specification, programming, and verification by refinement. Its semantics is based on Hoare and He's Unifying Theories of Programming [9].

A Circus program is composed of a sequence of Circus paragraphs and each paragraph can be a definition of a channel, a channelset or a Circus process.

Channels are used for communication between Circus processes. They are declared by their names and defined by the types of what they send or receive; if a declared channel does not deliver any value it only gives a signal to indicate that some synchronizing event happens. A channelset is a set of channels that are used to connect several Circus processes or several actions inside a Circus process.

Circus process is the main part of the Circus language which can be defined explicitly or implicitly. The explicit definition of a Circus process is delimited by the key words *begin* and *end*, whose actions are enumerated between them. At the start of a Circus process, a schema is defined after the keyword *state* if the process maintains a set of variables as its local state. At the end of a Circus process, a nameless action, which follows after a spot, defines the behaviours of the process. The implicit definitions of the Circus processes are compositions of defined processes with Circus operators. For example, given two Circus processes  $P_1$  and  $P_2$ , combine them with a binary operator

sequence, we get  $P_1$ ;  $P_2$  which means that it will execute the process  $P_2$  after termination of execution of  $P_1$ .

For the whole definition of Circus, the readers could refer to [10]. Here we only present some typical examples in our project to illustrate how to use Circus.

We can define types by declaration. For example,

```
[PSU]
[INTERRUPT]
```

Here, PSU is short for Primary Storage Unit which is a 64-bit number. The type INTERRUPT denotes the set of all interrupts produced by hardware units which are electronic signals in core hardware layer.

Constants are defined by axiomatic definition. For example,

```
0PSU : PSU
1PSU : PSU
ClockTickInterval : PSU
CLOCK_TICK : INTERRUPT
```

where  $0_{PSU}$  and  $1_{PSU}$  are the values zero and one respectively in a 64-bit system. ClockTickInterval is the time interval between two clock ticks and  $CLOCK\_TICK$  is a kind of interrupt generated by the timer.

In Circus, we can use the reserved word *channel* to define channels. For example,

```
channel module_init, module_end
channel rtclock_power_on, rtclock_power_off
channel clock_pause
channel hardware_interrupts : INTERRUPT
```

*module\_init* and *module\_end* are two signals from the environment. They denote two life stages of ARINC 653 modules. Similarly, the two signals *rtclock\_power\_on* and *rtclock\_power\_off* denote two life stages of real-time clocks. *clock\_pause* is a kind of signal generated by real-time clock and received by timer. The channel *hardware\_interrupts* is used by various hardware units to send external interrupts to Interrupt Controller.

Next we give two Circus processes to model real-time clock and timer one by one.

```
process RTClock ≡
begin
state RTCLOCK_TYPE == [Value : PSU]

Initialize ≡ Value := 0PSU

RunClockPause ≡ μX • (wait(1) ; Value := Value + 1PSU ; clock_pause) ; X

• rtclock_power_on → (Initialize ; RunClockPause) Δ rtclock_power_off → Skip

end
```

In real-time clock, a local state is maintained. It is defined by a Z schema which includes a variable Value whose type is PSU. Then, two Circus actions, Initialize and RunClockPause, are defined. The former is simple that the local variable Value is set to  $0_{PSU}$ . The latter is a recursive composition that the sequent action

$$\mathbf{wait}(1) ; Value := Value + 1_{PSU} ; clock\_pause \quad (1)$$

will be repeated infinitely many times. (1) means that it signals a clock pause after waiting for a basic time unit which is a nanosecond according to ARINC 653. Then, the behaviour of the Circus process RTClock is defined at last. After receiving the power-on signal, it initializes its state and then generates clock pauses until the power runs out.  $\Delta$  is used to describe that *Initialize ; RunClockPause* is interrupted on occurrence of the signal *rtclock\_power\_off*.

The model of timer is defined as follows:

|                                      |       |
|--------------------------------------|-------|
| $InitTimer$                          | _____ |
| $TIMER\_TYPE'$<br>$p? : PSU$         |       |
| $Value' = 0_{PSU}$<br>$Period' = p?$ |       |

```

process Timer  $\hat{=}$ 
begin
state  $TIMER\_TYPE == [Value, Period : PSU]$ 

  Initialize  $\hat{=}$   $InitTimer[ClockTickInterval/p?]$ 

  ClockTick  $\hat{=}$   $clock\_pause \longrightarrow Value := Value + 1_{PSU};$ 
                $\left( \begin{array}{l} \text{if } (Value \neq Period) \longrightarrow \text{Skip} \\ \quad \parallel (Value = Period) \longrightarrow Value := 0_{PSU}; \\ \quad \quad hardware\_interrupts \ !CLOCK\_TICK \longrightarrow \text{Skip} \\ \text{fi} \end{array} \right)$ 

  RunClockTick  $\hat{=}$   $\mu X \bullet ClockTick ; X$ 

   $\bullet module\_init \longrightarrow (Initialize ; RunClockTick) \Delta module\_end \longrightarrow \text{Skip}$ 

end

```

The structure of Circus process *Timer* is similar to that of *RTClock*. We give an initialization by a Z operation, the schema *InitTimer*, to initialize the state of *Timer*. The action *ClockTick* expresses that the local variable *Value* will be updated by adding  $1_{PSU}$  when a clock pause is received, then compare the value of two local variables, if *Value* is not equal to *Period*, terminate immediately, otherwise, reset *Value* to  $0_{PSU}$  and send a signal *CLOCK\_TICK* via Circus channel *hardware\_interrupts*.

Next by using a binary synchronization operator, we define a Circus process *PeriodicTicker* as follows.

```

channelset  $RTC\_TIMER == \{ clock\_pause \}$ 
process PeriodicTicker  $\hat{=}$   $RTClock \parallel [RTC\_TIMER] Timer$ 

```

where two Circus processes *RTClock* and *Timer* communicate with each other by the channelset *RTC\_TIMER* which contains only one channel *clock\_pause*.

We end this subsection by a complex example, the definition of ARINC 653 O/S Layer.

```

process ARINC653_OS_Layer  $\hat{=}$   $OSKernelConfig : OS\_KERNEL\_CONFIG\_TYPE \bullet$ 

   $CoreKernel(OSKernelConfig) \parallel [OSLayerChannels] (\parallel_{partid : \text{dom}(OSKernelConfig.Partitions)} \bullet$ 
     $PartitionKernel(partid, OSKernelConfig.Partitions(partid)))$ 

```

The process has an parameter *OSKernelConfig* which is the configuration of OS kernel. It can be used as a local variable. This Circus process is introduced by implicit definition of Circus processes *CoreKernel* and *PartitionKernel* with the binary synchronization operator  $\parallel$  and the general interleaving operator  $\parallel\parallel\parallel$ . Circus process *CoreKernel* and *PartitionKernel* are defined in Appendix D.3. The former has one argument *OSKernelConfig* and the latter has two: *partid*, which is a variable ranging over all identifiers of the partitions, and *OSKernelConfig.Partitions(partid)*, which is the configuration of the partition indexed by *partid* (the structure of *OSKernelConfig* is in Appendix A.5). The specification of ARINC 653 OS layer reflects that several partition kernels interleave with each other according to time partitioning. They all synchronize with core kernel via the channelset *OSLayerChannels* in their own time windows.

## 1.3 Related Work

There are plenty of researches on formal models of operating systems and ARINC 653 standard.

Craig presents several formal models of classical system kernels, ranging from simple ones to complex ones, who also proves a lot of desired properties of the models [6, 7]. These models of general-purpose kernels inspire us when we try to model a real-time kernel which meets ARINC 653 standard. Oliveira Gomes gives a formal model of an operating system with IMA architecture, which covers a small part of ARINC 653 services and kernel functions [12]. In [13] and [5], the researchers focus on the partition scheduler and process scheduler of IMA-architecture system, the characteristics of temporal partitioning are captured while the spatial partitioning is omitted. In the series of Zhao's works [16, 19, 18], separation kernels as well as APEX interface have been modelled and verified. Moreover, three errors in ARINC 653 document have been detected. In our model, we also propose some solutions to avoid these errors.

In industry, there are several real-time operating systems based on ARINC 653 standard [1, 2, 3, 4], such as VxWorks 653 and LynxOS-178. In VxWorks 653, the operating system is implemented as a Multi-Virtual Machine (MVM) framework. The core OS is the host OS and each partition OS is a guest OS. The advantage of this framework is the diversity of guest OS that each partition can install a different operating system from each other, such as real-time OS with APEX interface, general-purpose OS with POSIX interface. And what resides in a partition can even be some very old software that executes on bare machine. The disadvantage of this framework is the high cost of address translation and privilege instruction handling. A virtual machine manager for each partition is also necessary.

According to ARINC 653 document, we give a formal model of partition operating system where each partition OS is a real-time system with APEX interface.

## 2 A Circus Model of OS based on ARINC 653

In this section, we give a brief illustration of the structure of our model in Appendix. Firstly, we list all titles of the sections and subsections of Appendix and their associated page numbers.

### A Types and Constants

- A.1 Core Hardware Layer 10
- A.2 Hardware Interface Software Layer 14
- A.3 ARINC 653 O/S Layer(Core Kernel) 18
- A.4 ARINC 653 O/S Layer(Partition Kernel) 20
- A.5 ARINC 653 O/S Layer(Operating System Kernel) 25
- A.6 Application/Executive(APEX) 26
- A.7 Core Module 26

### B Z Operations

- B.1 Core Hardware Layer 27
- B.2 Hardware Interface Software Layer 32
- B.3 ARINC 653 O/S Layer 35

### C Circus Channels

### D Circus Processes

- D.1 Core Hardware Layer 57
- D.2 Hardware Interface Software Layer 65
- D.3 ARINC 653 O/S Layer 79
- D.4 Application/Executive(APEX) 113
- D.5 Core Module 136

The Appendix is divided into four parts: Types and Constants (see Appendix A), Z Operations (see Appendix B), Circus Channels (see Appendix C) and Circus Processes (see Appendix D). In Appendix A, we define all types and constants of each layer as well as some related functions. They are simply declared, declared by abbreviation or axiom, or defined as schemas. In Appendix B, we define operations in Z schema to illustrate initializations and state transitions. All these schemas can be defined within the Circus processes where they belong, for simplicity, we put them in a separate section. In Appendix C, we define all channels. The channelsets are presented in Circus Processes where they are used. In Appendix D, for each layer, we define behaviours of all components in this layer, and then compose them to form its behaviours. Further, we connect the Circus processes of each layer with channelsets so that the behaviours of ARINC 653 Core Module can be specified.

In Core Hardware Layer, the model includes a generic CPU, a MMU, main memory, a real-time clock, a timer, a high-precision timer and an Interrupt Controller. We list their corresponding processes' definition associated with their page numbers as follows:

D.1.1 Generic CPU 57

D.1.2 Memory Management Unit (MMU) 58

D.1.3 Main Memory 59

D.1.4 Real-Time Clock 59

D.1.5 Timer 60

D.1.6 High-Precision Timer 61

D.1.7 Interrupt Controller 63

The generic CPU, which can be regarded as a single-core processor, is the centre of this layer because all the external events are reported to it as interrupts or exceptions. The MMU is used for address translation and the main memory is where the data and instructions are stored temporarily. The real-time clock is responsible for providing current time for operating system at its initialization phase. The timer is used to time after the initialization of the system and generate periodic clock ticks to update system time. The high-precision timer is used to time during the time window of a partition and generate aperiodic clock ticks to update the time counters of current partition. The interrupt controller has many duties including recording hardware interrupts, masking certain interrupt and reporting interrupts to CPU according to their priorities. Then the model of this layer, *Core\_Hardware\_Layer* (see Page 64), is constructed by connecting these hardware units together with the channelset in this layer so that they can synchronize with CPU directly or indirectly.

In Hardware Interface Software Layer, the component Circus processes consist of context switching, memory management, system clock, interrupt controlling and interrupt handler. We list their corresponding processes' definition associated with their page numbers as follows:

D.2.1 Context Switching 65

D.2.2 Memory Management 67

D.2.3 System Clock 70

D.2.4 Interrupt Controlling 73

D.2.5 Interrupt Handler 75

Context switching and interrupt controlling are both sets of instructions for specific functions. The former is used to switch contexts and the latter is used to mask and unmask, enable and disable interrupts. By contrast, memory management, system clock and interrupt handler are functional modules in this layer. Memory management is responsible for managing physical memory, creating virtual address space for processes (and loading pages of processes into main memory). System clock is responsible for providing system time to the whole system. Interrupt handler is the main part to deal with interrupts but it must support interrupt nesting in a real-time system so that all kinds of external interrupts can be handled in time. The model of this layer, *Hardware\_Interface\_Software\_Layer*

(see Page 77), can be defined as context switching and interrupt controlling synchronize on the channelset of layer and interleave with memory management and system clock.

In ARINC 653 O/S Layer, there are two component Circus processes: CoreKernel (see Page 79) and PartitionKernel (see Page 85). The core kernel manages the kernel processes and all the partitions. The partitions are scheduled by core kernel based on round robin. Partition kernel manages the processes in its own partition and schedule them based on their priorities. The model of this layer, *ARINC653\_OS\_Layer* (see Page 112), consists of a CoreKernel process and several PartitionKernel processes. Several partition kernels interleave with each other but they all synchronize with core kernel via the channelset in this layer.

In APEX Layer, the component Circus process is APEX Interface (see Page 113). It includes many services which we list below. The model of APEX Layer, *APEX\_Layer* (see Page 136), can be seen as several APEX interface processes interleave with each other because the APEX interface is used by all the processes of all partitions of this ARINC 653 module.

1. Partition Management Service

- (a) *Get\_Partition\_Status* 113
- (b) *Set\_Partition\_Mode* 114

2. Process Management Sservice

- (a) *Get\_Process\_Id* 115
- (b) *Get\_Process\_Status* 115
- (c) *Create\_Process* 116
- (d) *Set\_Priority* 119
- (e) *Suspend\_Self* 120
- (f) *Suspend* 121
- (g) *Resume* 122
- (h) *Stop\_Self* 122
- (i) *Stop* 123
- (j) *Start* 124
- (k) *Delayed\_Start* 127
- (l) *Lock\_Preemption* 130
- (m) *Unlock\_Preemption* 131
- (n) *Get\_My\_Id* 131

3. Time Management Service

- (a) *Timed\_Wait* 132
- (b) *Periodic\_Wait* 133
- (c) *Get\_Time* 133
- (d) *Replenish* 134

### 3 Conclusion and Future Work

In this paper, we present a formal model of a real-time operating system based on ARINC 653 standard. By defining the workflow of the core module of ARINC 653, our model specifies the mechanism how the kernel operates, including interrupt response, partitions scheduling, processes scheduling and system calls to support the related APEX functions.

Contrary to other formal models of operating system based on ARINC 653, the concurrent behaviours of partitions and processes are also specified in this model. In ARINC 653 O/S Layer of the model, several partition

kernels interleave with each other. They run concurrently according to its time window in major time frame, it is the concurrent execution with a fixed order. In APEX Layer of the model, all the APEX interfaces, which is used by all the processes of all the partitions in this ARINC 653 Module, interleave. Since each APEX interface is specified by a unique process, the interleaving execution of APEX interfaces is the interleaving execution of processes. And the concurrent execution is not in a fixed order because the scheduling of process is based on its priority.

The following are some works we would do in the future.

Our work includes Partition Management, Process Management and Time Management of the document. A number of services, which are related to Interpartition/Intrapartition Communication as well as Health Monitor, are not included in this paper. We will add these services and their associated system calls in the future.

The second work is to prove the correctness of this model. There are two kinds of properties we should prove, basic ones of general operating systems and special ones of ARINC 653 standard. For the former, many essential properties are taken into consideration, for example, we can easily prove that ‘The kernel stack of different processes will not overlap both physically and virtually’ in this model by contradiction. For the latter, our concentration will be focused on the rules of process scheduling as stated in the document.

As we know, in this paper, the hardware model we present is rather simple and generic. A lot of work is required when we try to build a model of a more complex system, where there will be a correspondingly complex hardware architecture. This area covers the hardware units, like DMA chips, disks and various sensors, as well as the processor architecture like Symmetrical Multi-Processing (SMP) and Asymmetric Multi-processing (AMP), Unified Memory Access (UMA) and Non-Unified Memory Access (NUMA) and so on. The software model can also be specified with more details, such as file system and exception handler, they both need support from corresponding hardware units.

## References

- [1] Lynxsecure separation kernel hypervisor. <http://www.lynx.com/products/hypervisors/>.
- [2] Sysgo pikeos hypervisor. <https://www.sysgo.com/products/pikeos-rtos-and-virtualizationconcept/>.
- [3] Wind river vxworks 653 platform. <http://www.windriver.com/products/vxworks/certificationprofiles/>.
- [4] Wind river vxworks mils platform. <http://www.windriver.com/products/vxworks/certificationprofiles/>.
- [5] Laura Carnevali, Giuseppe Lipari, Alessandro Pinzuti, and Enrico Vicario. A formal approach to design and verification of two-level hierarchical scheduling systems. In *International Conference on Reliable Software Technologies*, pages 118–131. Springer, 2011.
- [6] Iain D Craig. *Formal models of operating system kernels*. Springer Science & Business Media, 2007.
- [7] Iain D Craig. *Formal refinement for operating system kernels*. Springer Science & Business Media, 2007.
- [8] Charles Antony Richard Hoare. Communicating sequential processes. *Communications of the ACM*, 21(8):666–677, 1978.
- [9] Charles Antony Richard Hoare and He Jifeng. *Unifying theories of programming*, volume 14. Prentice Hall Englewood Cliffs, 1998.
- [10] Marcel Oliveira, Ana Cavalcanti, and Jim Woodcock. A denotational semantics for circus. *Electronic Notes in Theoretical Computer Science*, 187:107–123, 2007.
- [11] Marcel Vinicius Medeiros Oliveira. *Formal derivation of state-rich reactive programs using Circus*. PhD thesis, University of York, 2005.
- [12] Artur Oliveira Gomes. *Formal specification of the ARINC 653 architecture using circus*. PhD thesis, University of York, 2012.



- [13] Frank Singhoff and Alain Plantec. Aadl modeling and analysis of hierarchical schedulers. In *Proceedings of the 2007 ACM international Conference on Sigada Annual international Conference*, pages 41–50, 2007.
- [14] ARINC Specification. Arinc 653: Avionics application software standard interface, part 1-required services, aeronautical radio. *Inc., November*, 2010.
- [15] J Michael Spivey and JR Abrial. *The Z notation*, volume 29. Prentice Hall Hemel Hempstead, 1992.
- [16] Ying Wang, Dianfu Ma, Yongwang Zhao, Lu Zou, and Xianqi Zhao. An aadl-based modeling method for arinc653-based avionics software. In *2011 IEEE 35th Annual Computer Software and Applications Conference*, pages 224–229. IEEE, 2011.
- [17] Jim Woodcock and Ana Cavalcanti. The semantics of circus. In *International Conference of B and Z Users*, pages 184–203. Springer, 2002.
- [18] Yongwang Zhao. Formal specification and verification of separation kernels: An overview. *ArXiv e-prints*, no, 2015.
- [19] Yongwang Zhao, Zhibin Yang, David Sanán, and Yang Liu. Event-based formalization of safety-critical operating system standards: An experience report on arinc 653 using event-b. In *2015 IEEE 26th International Symposium on Software Reliability Engineering (ISSRE)*, pages 281–292. IEEE, 2015.

## A Types and Constants

### A.1 Core Hardware Layer

#### A.1.1 Basic Definition

1.The Bit Length of the Hardware and the System, namely N, which should be 64 according to ARINC 653

$$\mid N : \mathbb{N}_1$$

2.The type of the value stored in a Bit, which can be zero or one

$$BIT ::= 0 \mid 1$$

3.The type of the content stored in Primary Storage Unit (PSU), which is the set of N-Bit binary numbers

$$[PSU]$$

4.The value zero and one of PSU

$$\mid \begin{array}{l} 0_{PSU} : PSU \\ 1_{PSU} : PSU \end{array}$$

5.The limit value of PSU, which appears to be 1 in each digit of the N-Bit binary number

$$\mid LIMIT_{PSU} : PSU$$

6.The type of System Address

$$SYSTEM\_ADDRESS\_TYPE == PSU$$

7.The type of the content stored in Memory Storage Unit (MSU)

$$MSU == PSU$$

8.The definition of function *bintounsigned* and *unsignedtobin*

$$\mid \begin{array}{l} bintounsigned : PSU \rightarrow \mathbb{N} \\ unsignedtobin : \mathbb{N} \rightarrow PSU \end{array}$$

9.The definition of function *bintosigned* and *signedtobin*

$$\mid \begin{array}{l} bintosigned : PSU \rightarrow \mathbb{Z} \\ signedtobin : \mathbb{Z} \rightarrow PSU \end{array}$$

10.The amount of interrupt kinds(which should be greater than or equal to 1 in this text)

$$\mid amount_i : \mathbb{N}_1$$

11.The type of interrupt

$$INTERRUPT\_TYPE == 0 \dots (amount_i - 1)$$

## 12.The Clock Tick

$$\begin{array}{|l} \hline \text{CLOCK\_TICK} : \text{INTERRUPT\_TYPE} \\ \hline \text{CLOCK\_TICK} = \min(\text{INTERRUPT\_TYPE}) \end{array}$$

## 13.The amount of exception kinds(which should be greater than or equal to 2 in this text)

$$\text{amount}_e : \mathbb{N}_1$$

## 14.The type of exception

$$\text{EXCEPTION\_TYPE} == 0 \dots (\text{amount}_e - 1)$$

## 15.The Page Fault and Access Violation

$$\begin{array}{|l} \hline \text{PAGE\_FAULT} : \text{EXCEPTION\_TYPE} \\ \text{ACCESS\_VIOLATION} : \text{EXCEPTION\_TYPE} \\ \hline \end{array}$$

### A.1.2 Generic CPU

#### 1.The amount of General-Purpose Registers

$$\begin{array}{|l} \hline \text{amount}_{gpr} : \mathbb{N}_1 \\ \hline \end{array}$$

#### 2.The number of General-Purpose Registers

$$\text{GPNumber} == 0 \dots (\text{amount}_{gpr} - 1)$$

#### 3.The type of General-Purpose Registers

$$\text{GPREGISTER\_TYPE} == \text{GPNumber} \rightarrow \text{PSU}$$

#### 4.The type of Registers for Stack Segment

$$\begin{array}{|l} \hline \text{SSREGISTER\_TYPE} \\ \hline \text{SS} : \text{PSU} \\ \text{SL} : \text{PSU} \\ \text{BP} : \text{PSU} \\ \text{SP} : \text{PSU} \\ \hline \end{array}$$

#### 5.The type of Registers for Data Segment

$$\begin{array}{|l} \hline \text{DSREGISTER\_TYPE} \\ \hline \text{DS} : \text{PSU} \\ \text{DL} : \text{PSU} \\ \text{SI} : \text{PSU} \\ \text{DI} : \text{PSU} \\ \hline \end{array}$$

#### 6.The type of Registers for Code Segment

$$\begin{array}{|l} \hline \text{CSREGISTER\_TYPE} \\ \hline \text{CS} : \text{PSU} \\ \text{CL} : \text{PSU} \\ \text{IP} : \text{PSU} \\ \hline \end{array}$$

## 7.The type of Registers for Program Status Word

$PSWREGISTER\_TYPE$

$CF : BIT$   
 $PF : BIT$   
 $AF : BIT$   
 $ZF : BIT$   
 $SF : BIT$   
 $OF : BIT$   
 $TF : BIT$   
 $DF : BIT$   
 $IF : BIT$

## 8.The type of CPU Register

$CPU\_REGISTER\_TYPE$

$GPRegister : GPREGISTER\_TYPE$   
 $SSRegister : SSREGISTER\_TYPE$   
 $DSRegister : DSREGISTER\_TYPE$   
 $CSRegister : CSREGISTER\_TYPE$   
 $PSWRegister : PSWREGISTER\_TYPE$

### A.1.3 Memory Management Unit (MMU)

#### 1.The Bit Length used for page, namely PAGE, and the Bit Length used for offset, namely OFFSET

$PAGE : \mathbb{N}_1$   
 $OFFSET : \mathbb{N}_1$

$PAGE + OFFSET = N$

#### 2.The constant PAGE \_ SIZE

$PAGE\_SIZE : \mathbb{N}_1$

$PAGE\_SIZE = 2^{OFFSET}$

#### 3.The definition of function *getpage* and *getoffset*

$getpage : SYSTEM\_ADDRESS\_TYPE \rightarrow SYSTEM\_ADDRESS\_TYPE$   
 $getoffset : SYSTEM\_ADDRESS\_TYPE \rightarrow SYSTEM\_ADDRESS\_TYPE$

$\forall a : SYSTEM\_ADDRESS\_TYPE \bullet$   
 $getpage(a) = a - getoffset(a)$   
 $getoffset(a) = a \bmod unsignedtobin(PAGE\_SIZE)$

#### 4.The type of Page

$PAGE\_TYPE == \{a : SYSTEM\_ADDRESS\_TYPE \mid a \bmod unsignedtobin(PAGE\_SIZE) = 0_{PSU}\}$

#### 5.The definition of function *pagespace*

$pagespace : PAGE\_TYPE \rightarrow \mathbb{P} SYSTEM\_ADDRESS\_TYPE$

$\forall p : PAGE\_TYPE \bullet$   
 $pagespace(p) = \{a : SYSTEM\_ADDRESS\_TYPE \mid a \geq p \wedge a < p + unsignedtobin(PAGE\_SIZE)\}$

## 6.The definition of function *nextpage*

|                                                                                                       |
|-------------------------------------------------------------------------------------------------------|
| $nextpage : SYSTEM\_ADDRESS\_TYPE \rightarrow PAGE\_TYPE$                                             |
| $\forall a : SYSTEM\_ADDRESS\_TYPE \bullet$<br>$nextpage(a) = getpage(a) + unsignedtobin(PAGE\_SIZE)$ |

## 7.The type of Page Table

$$PAGE\_TABLE\_TYPE == PAGE\_TYPE \mapsto PAGE\_TYPE$$

## 8.The type of Piece which is the content of a Page

$$PIECE\_TYPE == \{\emptyset\} \cup \{p : SYSTEM\_ADDRESS\_TYPE \mapsto PSU \mid p \neq \emptyset \\ \wedge \min(\text{dom } p) \in PAGE\_TYPE \wedge \# p \leq PAGE\_SIZE\}$$

## 9.The type of Memory Management Unit

|                                       |
|---------------------------------------|
| $MEMORY\_MANAGEMENT\_UNIT\_TYPE$      |
| $PageTableBuffer : PAGE\_TABLE\_TYPE$ |

### A.1.4 Main Memory

#### 1.The type of Main Memory

|                                             |
|---------------------------------------------|
| $MAIN\_MEMORY\_TYPE$                        |
| $Store : SYSTEM\_ADDRESS\_TYPE \mapsto MSU$ |

### A.1.5 Real-Time Clock

#### 1.The type of RTClock

|                 |
|-----------------|
| $RTCLOCK\_TYPE$ |
| $Value : PSU$   |

### A.1.6 Timer

#### 1.The definition of Clock Tick Interval

|                           |
|---------------------------|
| $ClockTickInterval : PSU$ |
|---------------------------|

#### 2.The type of Timer

|                |
|----------------|
| $TIMER\_TYPE$  |
| $Value : PSU$  |
| $Period : PSU$ |

### A.1.7 High-Precision Timer

#### 1.The type of HPTimer

|                 |
|-----------------|
| $HPTIMER\_TYPE$ |
| $Value : PSU$   |
| $Alarm : PSU$   |

### A.1.8 Interrupt Controller

#### 1.The type of Interrupt Controller Registers

$$ICREGISTER\_TYPE == INTERRUPT\_TYPE \rightarrow BIT$$

#### 2.The type of Interrupt Controller

$$\begin{array}{l} INTERRUPT\_CONTROLLER\_TYPE \\ \hline IRRegister : ICREGISTER\_TYPE \\ IMRegister : ICREGISTER\_TYPE \\ ISRegister : ICREGISTER\_TYPE \end{array}$$

## A.2 Hardware Interface Software Layer

### A.2.1 Basic Definition

#### 1.The definition of sequence of a generic type

$$seq[X] == \{s : \mathbb{N} \mapsto X \mid \exists n : \mathbb{N} \bullet \text{dom } s = 1 \dots n\}$$

#### 2.The definition of non-empty sequence of a generic type

$$seq_1[X] == \{s : seq[X] \mid s \neq \langle \rangle\}$$

#### 3.The definition of function *slide*

$$\begin{array}{l} slide : seq_1[X] \times \mathbb{N} \rightarrow (\mathbb{N}_1 \mapsto X) \\ \hline \forall s : seq_1[X]; n : \mathbb{N} \bullet \\ slide(s, n) = \{i : \mathbb{N} \mid i \in \text{dom } s \bullet (i + n) \mapsto s(i)\} \end{array}$$

#### 4.The type of Unsigned Integer

$$\begin{array}{l} UNSIGNED\_INTEGER\_TYPE : \mathbb{P}\mathbb{N} \\ \hline \forall n : \mathbb{N} \bullet \\ n \in UNSIGNED\_INTEGER\_TYPE \Leftrightarrow n \geq bintounsinged(0_{PSU}) \wedge n \leq bintounsinged(LIMIT_{PSU}) \end{array}$$

#### 5.The type of Signed Integer

$$\begin{array}{l} SIGNED\_INTEGER\_TYPE : \mathbb{P}\mathbb{Z} \\ \hline \forall z : \mathbb{Z} \bullet \\ z \in SIGNED\_INTEGER\_TYPE \Leftrightarrow z \geq bintosigned(LIMIT_{PSU}) - 1 \wedge z \leq -bintosigned(LIMIT_{PSU}) \end{array}$$

#### 6.The type of Option

$$OPTION\_TYPE ::= PART \mid ALL$$

#### 7.The type of Segment

$$SEGMENT\_TYPE == \{\emptyset\} \cup \{seg : SYSTEM\_ADDRESS\_TYPE \mapsto PSU \mid \exists end : SYSTEM\_ADDRESS\_TYPE \bullet \text{dom } seg = 0_{PSU} \dots end\}$$

## 8. The type of Executable File

|                                                                              |
|------------------------------------------------------------------------------|
| $EXECUTABLE\_FILE\_TYPE$<br>$Data : SEGMENT\_TYPE$<br>$Code : SEGMENT\_TYPE$ |
|------------------------------------------------------------------------------|

## 9. The definition of function *pagecount*

|                                                                                                                                                                                             |
|---------------------------------------------------------------------------------------------------------------------------------------------------------------------------------------------|
| $pagecount : UNSIGNED\_INTEGER\_TYPE \rightarrow UNSIGNED\_INTEGER\_TYPE$<br>$\forall n : UNSIGNED\_INTEGER\_TYPE \bullet$<br>$pagecount(n) = (n + PAGE\_SIZE - 1) \text{ div } PAGE\_SIZE$ |
|---------------------------------------------------------------------------------------------------------------------------------------------------------------------------------------------|

## 10. The definition of function *sizecount*

|                                                                                                                                                                          |
|--------------------------------------------------------------------------------------------------------------------------------------------------------------------------|
| $sizecount : UNSIGNED\_INTEGER\_TYPE \rightarrow UNSIGNED\_INTEGER\_TYPE$<br>$\forall n : UNSIGNED\_INTEGER\_TYPE \bullet$<br>$sizecount(n) = pagecount(n) * PAGE\_SIZE$ |
|--------------------------------------------------------------------------------------------------------------------------------------------------------------------------|

## 11. The definition of function *paging*

|                                                                                                                                                                                                                                                                                                                                                                                              |
|----------------------------------------------------------------------------------------------------------------------------------------------------------------------------------------------------------------------------------------------------------------------------------------------------------------------------------------------------------------------------------------------|
| $paging : SEGMENT\_TYPE \rightarrow seq[PIECE\_TYPE]$<br>$\forall seg : SEGMENT\_TYPE \bullet$<br>$paging(seg) = \{i : \mathbb{N}_1 \mid i \in 1 \dots pagecount(\# seg) \bullet i \mapsto \{a : SYSTEM\_ADDRESS\_TYPE \mid$<br>$a \in \text{dom } seg \wedge a \geq \text{unsignedtobin}((i - 1) * PAGE\_SIZE) \wedge a < \text{unsignedtobin}$<br>$(i * PAGE\_SIZE)\} \triangleleft seg\}$ |
|----------------------------------------------------------------------------------------------------------------------------------------------------------------------------------------------------------------------------------------------------------------------------------------------------------------------------------------------------------------------------------------------|

## 12. The definition of function *randompage*

|                                                                                                                                                                                  |
|----------------------------------------------------------------------------------------------------------------------------------------------------------------------------------|
| $randompage : \mathbb{P} PAGE\_TYPE \rightarrow PAGE\_TYPE$<br>$randompage = (\lambda ps : \mathbb{P} PAGE\_TYPE \mid ps \neq \emptyset \bullet (p : PAGE\_TYPE \mid p \in ps))$ |
|----------------------------------------------------------------------------------------------------------------------------------------------------------------------------------|

## 13. The type of Kernel Identifier

$$KERNEL\_ID\_TYPE == UNSIGNED\_INTEGER\_TYPE$$

## 14. The constant Core Kernel

|                                                         |
|---------------------------------------------------------|
| $CORE\_KERNEL : KERNEL\_ID\_TYPE$<br>$CORE\_KERNEL = 0$ |
|---------------------------------------------------------|

### A.2.2 Context Switching

#### 1. The type of Context

$$CONTEXT\_TYPE == CPU\_REGISTER\_TYPE \times PAGE\_TABLE\_TYPE$$

#### 2. The definition of function *makecontext*

|                                                                                                                                                                                                              |
|--------------------------------------------------------------------------------------------------------------------------------------------------------------------------------------------------------------|
| $makecontext : CPU\_REGISTER\_TYPE \times PAGE\_TABLE\_TYPE \rightarrow CONTEXT\_TYPE$<br>$\forall cpureg : CPU\_REGISTER\_TYPE; pt : PAGE\_TABLE\_TYPE \bullet$<br>$makecontext(cpureg, pt) = (cpureg, pt)$ |
|--------------------------------------------------------------------------------------------------------------------------------------------------------------------------------------------------------------|

### A.2.3 Memory Management

#### 1. The type of Memory Block

|                                  |
|----------------------------------|
| $MEMORY\_BLOCK\_TYPE$            |
| $Start : PAGE\_TYPE$             |
| $Size : UNSIGNED\_INTEGER\_TYPE$ |
| $Size \bmod PAGE\_SIZE = 0$      |

#### 2. The constant `NULL_BLOCK` which denotes a Memory Block with no size

|                                     |
|-------------------------------------|
| $NULL\_BLOCK : MEMORY\_BLOCK\_TYPE$ |
| $NULL\_BLOCK.Size = 0$              |

#### 3. The definition of function `blockspace`

|                                                                                                                                                                       |
|-----------------------------------------------------------------------------------------------------------------------------------------------------------------------|
| $blockspace : MEMORY\_BLOCK\_TYPE \rightarrow \mathbb{P} SYSTEM\_ADDRESS\_TYPE$                                                                                       |
| $\forall mb : MEMORY\_BLOCK\_TYPE \bullet$<br>$blockspace(mb) = \{a : SYSTEM\_ADDRESS\_TYPE \mid a \geq mb.Start$<br>$\wedge a < mb.Start + unsignedtobin(mb.Size)\}$ |

#### 4. The definition of function `totalpage`

|                                                                                                              |
|--------------------------------------------------------------------------------------------------------------|
| $totalpage : MEMORY\_BLOCK\_TYPE \rightarrow \mathbb{P} PAGE\_TYPE$                                          |
| $\forall mb : MEMORY\_BLOCK\_TYPE \bullet$<br>$totalpage(mb) = \{p : PAGE\_TYPE \mid p \in blockspace(mb)\}$ |

#### 5. The type of Physical Memory Block

$$PHYSICAL\_MEMORY\_BLOCK\_TYPE == MEMORY\_BLOCK\_TYPE$$

#### 6. The type of Virtual Memory Block

|                                                     |
|-----------------------------------------------------|
| $VIRTUAL\_MEMORY\_BLOCK\_TYPE$                      |
| $Memory : MEMORY\_BLOCK\_TYPE$                      |
| $Base : \mathbb{P} PAGE\_TYPE$                      |
| $PageTable : PAGE\_TABLE\_TYPE$                     |
| $\text{dom } PageTable \subseteq totalpage(Memory)$ |
| $\text{ran } PageTable \subseteq Base$              |

#### 7. The constant `NULL` which is a reserved System Address in virtual address space for denoting empty

|                                |
|--------------------------------|
| $NULL : SYSTEM\_ADDRESS\_TYPE$ |
| $NULL = 0_{PSU}$               |



**8.The constant `PROCESS _ VIRTUAL _ ADDRESS _ SPACE` and `KERNEL _ VIRTUAL _ ADDRESS _ SPACE`**

|                                                                                                                     |
|---------------------------------------------------------------------------------------------------------------------|
| $PROCESS\_VIRTUAL\_ADDRESS\_SPACE : MEMORY\_BLOCK\_TYPE$<br>$KERNEL\_VIRTUAL\_ADDRESS\_SPACE : MEMORY\_BLOCK\_TYPE$ |
|---------------------------------------------------------------------------------------------------------------------|

|                                                                                                                                                                                                                                             |
|---------------------------------------------------------------------------------------------------------------------------------------------------------------------------------------------------------------------------------------------|
| $NULL \notin blockspace(PROCESS\_VIRTUAL\_ADDRESS\_SPACE)$<br>$NULL \notin blockspace(KERNEL\_VIRTUAL\_ADDRESS\_SPACE)$<br>$blockspace(PROCESS\_VIRTUAL\_ADDRESS\_SPACE) \cap$<br>$blockspace(KERNEL\_VIRTUAL\_ADDRESS\_SPACE) = \emptyset$ |
|---------------------------------------------------------------------------------------------------------------------------------------------------------------------------------------------------------------------------------------------|

**9.The constant `KERNEL _ STACK _ SIZE` which is the size of kernel stack of a process**

|                                                 |
|-------------------------------------------------|
| $KERNEL\_STACK\_SIZE : UNSIGNED\_INTEGER\_TYPE$ |
|-------------------------------------------------|

|                                                                            |
|----------------------------------------------------------------------------|
| $KERNEL\_STACK\_SIZE \neq 0$<br>$KERNEL\_STACK\_SIZE \bmod PAGE\_SIZE = 0$ |
|----------------------------------------------------------------------------|

**10.The type of Process Virtual Memory**

|                                                                                                                                                                               |
|-------------------------------------------------------------------------------------------------------------------------------------------------------------------------------|
| $PROCESS\_VIRTUAL\_MEMORY\_TYPE$<br>$VMBlock : VIRTUAL\_MEMORY\_BLOCK\_TYPE$<br>$Stack : MEMORY\_BLOCK\_TYPE$<br>$Data : MEMORY\_BLOCK\_TYPE$<br>$Code : MEMORY\_BLOCK\_TYPE$ |
|-------------------------------------------------------------------------------------------------------------------------------------------------------------------------------|

|                                                                                                                                                                                                                                                                                                                                                               |
|---------------------------------------------------------------------------------------------------------------------------------------------------------------------------------------------------------------------------------------------------------------------------------------------------------------------------------------------------------------|
| $blockspace(VMBlock.Memory) \subseteq blockspace(PROCESS\_VIRTUAL\_ADDRESS\_SPACE)$<br>$blockspace(VMBlock.Memory) = blockspace(Stack) \cup blockspace(Data) \cup blockspace(Code)$<br>$blockspace(Stack) \cap blockspace(Data) = \emptyset$<br>$blockspace(Stack) \cap blockspace(Code) = \emptyset$<br>$blockspace(Data) \cap blockspace(Code) = \emptyset$ |
|---------------------------------------------------------------------------------------------------------------------------------------------------------------------------------------------------------------------------------------------------------------------------------------------------------------------------------------------------------------|

**11.The type of Area Memory Management**

|                                                                                                                                                       |
|-------------------------------------------------------------------------------------------------------------------------------------------------------|
| $AREA\_MEMORY\_MANAGEMENT\_TYPE$<br>$Memory : PHYSICAL\_MEMORY\_BLOCK\_TYPE$<br>$Allocated : \mathbb{P} PAGE\_TYPE$<br>$Free : \mathbb{P} PAGE\_TYPE$ |
|-------------------------------------------------------------------------------------------------------------------------------------------------------|

|                                                                                |
|--------------------------------------------------------------------------------|
| $Allocated \cap Free = \emptyset$<br>$Allocated \cup Free = totalpage(Memory)$ |
|--------------------------------------------------------------------------------|

**12.The type of Memory Management State**

|                                                                                                 |
|-------------------------------------------------------------------------------------------------|
| $MEMORY\_MANAGEMENT\_STATE\_TYPE$<br>$AreaMemoryManagementRef : AREA\_MEMORY\_MANAGEMENT\_TYPE$ |
|-------------------------------------------------------------------------------------------------|

**A.2.4 System Clock**

**1.The type of System Time**

$SYSTEM\_TIME\_TYPE == SIGNED\_INTEGER\_TYPE$

**2.The constant `DEFAULT _ TIME` which is a default value for uncertain time**

|                                      |
|--------------------------------------|
| $DEFAULT\_TIME : SYSTEM\_TIME\_TYPE$ |
|--------------------------------------|

|                      |
|----------------------|
| $DEFAULT\_TIME = -1$ |
|----------------------|

### 3.The type of System Clock State

|                                                                                                                                                                                                                          |
|--------------------------------------------------------------------------------------------------------------------------------------------------------------------------------------------------------------------------|
| $SYSTEM\_CLOCK\_STATE\_TYPE$<br>$BaseTime : SYSTEM\_TIME\_TYPE$<br>$TickInterval : SYSTEM\_TIME\_TYPE$<br>$TickCounter : UNSIGNED\_INTEGER\_TYPE$<br>$Time : SYSTEM\_TIME\_TYPE$<br>$InterruptTime : SYSTEM\_TIME\_TYPE$ |
|--------------------------------------------------------------------------------------------------------------------------------------------------------------------------------------------------------------------------|

### A.2.5 Interrupt Handler

#### 1.The type of Interrupt Handler State

|                                                                                                                                                               |
|---------------------------------------------------------------------------------------------------------------------------------------------------------------|
| $INTERRUPT\_HANDLER\_STATE\_TYPE$<br>$KernelPageTableRef : PAGE\_TABLE\_TYPE$<br>$InterruptStack : MEMORY\_BLOCK\_TYPE$<br>$TempContext : seq[CONTEXT\_TYPE]$ |
|---------------------------------------------------------------------------------------------------------------------------------------------------------------|

#### 2.The type of Interrupt Handler Configuration

|                                                                                                                                                                  |
|------------------------------------------------------------------------------------------------------------------------------------------------------------------|
| $INTERRUPT\_HANDLER\_CONFIG\_TYPE$<br>$InterruptStackSize : UNSIGNED\_INTEGER\_TYPE$<br>$InterruptStackSize \neq 0$<br>$InterruptStackSize \bmod PAGE\_SIZE = 0$ |
|------------------------------------------------------------------------------------------------------------------------------------------------------------------|

### A.3 ARINC 653 O/S Layer(Core Kernel)

#### A.3.1 Basic Definition

##### 1.The definition of non-empty injective sequence of a generic type

$$iseq_1[X] == \{s : seq[X] \mid s \neq \langle \rangle \wedge s \in \mathbb{N} \mapsto X\}$$

##### 2.The type of Boolean

$$BOOLEAN ::= TRUE \mid FALSE$$

##### 3.The type of String

$$[STRING]$$

##### 4.The constant PARTITION \_ NUMBER \_ LIMIT which is the Limit Number of Partitions of the System

$$\mid PARTITION\_NUMBER\_LIMIT : UNSIGNED\_INTEGER\_TYPE$$

#### A.3.2 Core Kernel

##### 1.The type of Kernel Process Management

*KERNEL\_PROCESS\_MANAGEMENT\_TYPE* \_\_\_\_\_

*ProcessTable* : *PROCESS\_TABLE\_TYPE*

*CurrentProcess* : *PROCESS\_ID\_TYPE*

$(\forall i, j : \text{PROCESS\_ID\_TYPE} \mid i, j \in \text{dom } \text{ProcessTable} \bullet$

$i \neq j \Rightarrow \text{blockspace}(\text{ProcessTable}(i).\text{KernelStack}) \cap \text{blockspace}(\text{ProcessTable}(j).\text{KernelStack}) = \emptyset)$

$(\forall i : \text{PROCESS\_ID\_TYPE} \mid i \in \text{dom } \text{ProcessTable} \bullet$

$\text{ProcessTable}(i).\text{VirtualMemory.VMBlock.Memory} = \text{NULL\_BLOCK})$

$(\forall i : \text{PROCESS\_ID\_TYPE} \mid i \in \text{dom } \text{ProcessTable} \bullet$

$\text{ProcessTable}(i).\text{VirtualMemory.VMBlock.Base} = \emptyset)$

$(\forall i : \text{PROCESS\_ID\_TYPE} \mid i \in \text{dom } \text{ProcessTable} \bullet$

$\text{ProcessTable}(i).\text{UserTempContext} = \langle \rangle)$

$\text{CurrentProcess} \in \{\text{NULL\_PROCESS\_ID}\} \cup \text{dom } \text{ProcessTable}$

$(\forall i, j : \text{PROCESS\_ID\_TYPE} \mid i, j \in \text{dom } \text{ProcessTable} \bullet$

$\text{ProcessTable}(i).\text{ProcessState} = \text{RUNNING} \wedge \text{ProcessTable}(j).\text{ProcessState} = \text{RUNNING} \Rightarrow i = j = \text{CurrentProcess})$

## 2.The type of Partition Table

*PARTITION\_TABLE\_TYPE* == *PARTITION\_ID\_TYPE*  $\bowtie$  *PARTITION\_CONTROL\_BLOCK\_TYPE*

## 3.The type of Partition Time Window

*PARTITION\_TIME\_WINDOW\_TYPE* \_\_\_\_\_

*PartitionId* : *PARTITION\_ID\_TYPE*

*Periodicity* : *PARTITION\_PERIODICITY\_TYPE*

*Offset* : *SYSTEM\_TIME\_TYPE*

*PeriodicProcStart* : *BOOLEAN*

## 4.The type of Partition Time Window Configuration

*PARTITION\_TIME\_WINDOW\_CONFIG\_TYPE* \_\_\_\_\_

*Name* : *PARTITION\_NAME\_TYPE*

*PeriodicProcStart* : *BOOLEAN*

## 5.The type of MajorTimeFrame

*MAJOR\_TIME\_FRAME\_TYPE* \_\_\_\_\_

*PartitionQueue* : *iseq*<sub>1</sub>[*PARTITION\_TIME\_WINDOW\_TYPE*]

*Length* : *SYSTEM\_TIME\_TYPE*

## 6.The type of Partition Management

*PARTITION\_MANAGEMENT\_TYPE* \_\_\_\_\_

*PartitionTable* : *PARTITION\_TABLE\_TYPE*

*MajorTimeFrame* : *MAJOR\_TIME\_FRAME\_TYPE*

*CurrentPartition* : *PARTITION\_ID\_TYPE*

$(\forall i, j : \text{PARTITION\_ID\_TYPE} \mid i, j \in \text{dom } \text{PartitionTable} \bullet$

$i \neq j \Rightarrow \text{blockspace}(\text{PartitionTable}(i).\text{Memory}) \cap \text{blockspace}(\text{PartitionTable}(j).\text{Memory}) = \emptyset)$

$\text{CurrentPartition} \in \{\text{NULL\_PARTITION\_ID}\} \cup \text{dom } \text{PartitionTable}$

## 7.The type of Core Kernel State

*CORE\_KERNEL\_STATE\_TYPE*

*MemoryManagement* : *AREA\_MEMORY\_MANAGEMENT\_TYPE*

*KernelPageTable* : *PAGE\_TABLE\_TYPE*

*KernelProcManagement* : *KERNEL\_PROCESS\_MANAGEMENT\_TYPE*

*PartitionManagement* : *PARTITION\_MANAGEMENT\_TYPE*

$\text{dom } \text{KernelPageTable} \subseteq \text{totalpage}(\text{KERNEL\_VIRTUAL\_ADDRESS\_SPACE})$

$\text{ran } \text{KernelPageTable} = \text{totalpage}(\text{MemoryManagement.Memory})$

## A.4 ARINC 653 O/S Layer(Partition Kernel)

### A.4.1 Basic Definition

#### 1.The definition of injective sequence of a generic type

$$\text{isseq}[X] == \{s : \text{seq}[X] \mid s \in \mathbb{N} \mapsto X\}$$

#### 2.The constant **PROCESS \_ NUMBER \_ LIMIT** which is the Limit Number of Processes in any Partition of the System

| *PROCESS\_NUMBER\_LIMIT* : *UNSIGNED\_INTEGER\_TYPE*

#### 3.The type of Disk Address

[*DISK\_ADDRESS*]

#### 4.The constant **NULL \_ DISK \_ ADDRESS** which is a Disk Address for denoting empty

| *NULL\_DISK\_ADDRESS* : *DISK\_ADDRESS*

#### 5.The type of Path

*PATH\_TYPE* == *DISK\_ADDRESS*

#### 6.The constant **MIN \_ STACK \_ SIZE** and **MAX \_ STACK \_ SIZE**

| *MIN\_STACK\_SIZE* : *UNSIGNED\_INTEGER\_TYPE*

| *MAX\_STACK\_SIZE* : *UNSIGNED\_INTEGER\_TYPE*

|  $\text{MIN\_STACK\_SIZE} > 0$

|  $\text{MAX\_STACK\_SIZE} > \text{MIN\_STACK\_SIZE}$

#### 7.The range of Process Stack Size

$\text{STACK\_SIZE\_RANGE} == \text{MIN\_STACK\_SIZE} .. \text{MAX\_STACK\_SIZE}$

#### 8.The constant **MIN \_ PRIORITY \_ VALUE** and **MAX \_ PRIORITY \_ VALUE**

| *MIN\_PRIORITY\_VALUE* : *SIGNED\_INTEGER\_TYPE*

| *MAX\_PRIORITY\_VALUE* : *SIGNED\_INTEGER\_TYPE*

|  $\text{MIN\_PRIORITY\_VALUE} > 0$

|  $\text{MAX\_PRIORITY\_VALUE} > \text{MIN\_PRIORITY\_VALUE}$

## 9.The range of Process Priority

$PRIORITY\_RANGE == MIN\_PRIORITY\_VALUE .. MAX\_PRIORITY\_VALUE$

## 10.The constant MIN \_ LOCK \_ LEVEL and MAX \_ LOCK \_ LEVEL

|                                                                                              |
|----------------------------------------------------------------------------------------------|
| $MIN\_LOCK\_LEVEL : UNSIGNED\_INTEGER\_TYPE$<br>$MAX\_LOCK\_LEVEL : UNSIGNED\_INTEGER\_TYPE$ |
| $MIN\_LOCK\_LEVEL = 0$<br>$MAX\_LOCK\_LEVEL > MIN\_LOCK\_LEVEL$                              |

## 11.The range of Partition Lock Level

$LOCK\_LEVEL\_RANGE == MIN\_LOCK\_LEVEL .. MAX\_LOCK\_LEVEL$

## 12.The type of System Call

$SYSTEM\_CALL\_TYPE ::= GET\_OPERATING\_MODE | GET\_PARTITION\_STATUS$   
 $| SET\_OPERATING\_MODE$   
 $| GET\_PROCESS\_NAMES | GET\_PROCESS\_IDS$   
 $| GET\_FREE\_PROCESS\_IDS | GET\_FREE\_SPACE$   
 $| GET\_PARTITION\_PERIOD | GET\_PROCESS\_STATE$   
 $| GET\_NEXT\_PERIODIC\_START | GET\_DELAYED\_PERIODIC\_START$   
 $| GET\_PROCESS\_KIND | GET\_PROCESS\_PERIOD$   
 $| GET\_PROCESS\_TIME\_CAPACITY | GET\_PARTITION\_LOCK\_LEVEL$   
 $| GET\_PROCESS\_ID | GET\_PROCESS\_STATUS | CREATE\_PROCESS$   
 $| SET\_PRIORITY | SUSPEND\_SELF | SUSPEND | RESUME | STOP\_SELF$   
 $| STOP | START | DELAYED\_START | LOCK\_PREEMPTION$   
 $| UNLOCK\_PREEMPTION | GET\_MY\_ID$   
 $| GET\_CURRENT\_TIME | GET\_NEXT\_RELEASE\_POINT | TIMED\_WAIT$   
 $| PERIODIC\_WAIT | GET\_TIME | REPLENISH$

## 13.The System Call(Partition Management),System Call(Process Management) and System Call(Time Management)

|                                                                                                                                                                                                                                                                                                                                                                                                                                                                                                                                                                                                                                                                                                                                                                       |
|-----------------------------------------------------------------------------------------------------------------------------------------------------------------------------------------------------------------------------------------------------------------------------------------------------------------------------------------------------------------------------------------------------------------------------------------------------------------------------------------------------------------------------------------------------------------------------------------------------------------------------------------------------------------------------------------------------------------------------------------------------------------------|
| $SystemCall\_Partition : \mathbb{P} SYSTEM\_CALL\_TYPE$<br>$SystemCall\_Process : \mathbb{P} SYSTEM\_CALL\_TYPE$<br>$SystemCall\_Time : \mathbb{P} SYSTEM\_CALL\_TYPE$                                                                                                                                                                                                                                                                                                                                                                                                                                                                                                                                                                                                |
| $SystemCall\_Partition = \{ GET\_OPERATING\_MODE, GET\_PARTITION\_STATUS, SET\_OPERATING\_MODE \}$<br>$SystemCall\_Process = \{ GET\_PROCESS\_NAMES, GET\_PROCESS\_IDS, GET\_FREE\_PROCESS\_IDS, GET\_FREE\_SPACE, GET\_PARTITION\_PERIOD, GET\_PROCESS\_STATE, GET\_NEXT\_PERIODIC\_START, GET\_DELAYED\_PERIODIC\_START, GET\_PROCESS\_KIND, GET\_PROCESS\_PERIOD, GET\_PROCESS\_TIME\_CAPACITY, GET\_PARTITION\_LOCK\_LEVEL, GET\_PROCESS\_ID, GET\_PROCESS\_STATUS, CREATE\_PROCESS, SET\_PRIORITY, SUSPEND\_SELF, SUSPEND, RESUME, STOP\_SELF, STOP, START, DELAYED\_START, LOCK\_PREEMPTION, UNLOCK\_PREEMPTION, GET\_MY\_ID \}$<br>$SystemCall\_Time = \{ GET\_CURRENT\_TIME, GET\_NEXT\_RELEASE\_POINT, TIMED\_WAIT, PERIODIC\_WAIT, GET\_TIME, REPLENISH \}$ |

### A.4.2 Process

#### 1.The type of Process Identifier

$PROCESS\_ID\_TYPE == UNSIGNED\_INTEGER\_TYPE$

## 2.The type of Process Name

$PROCESS\_NAME\_TYPE == STRING$

## 3.The type of Process Kind

$PROCESS\_KIND\_TYPE ::= PERIODIC \mid APERIODIC \mid ERROR\_HANDLER$

## 4.The type of Process Stack Size

$STACK\_SIZE\_TYPE == \{n : UNSIGNED\_INTEGER\_TYPE \mid n > 0 \wedge n \bmod PAGE\_SIZE = 0\}$

## 5.The type of Process Priority

$PRIORITY\_TYPE == SIGNED\_INTEGER\_TYPE$

## 6.The constant DEFAULT \_ PRIORITY which is a default value for uncertain priority

|                                      |
|--------------------------------------|
| $DEFAULT\_PRIORITY : PRIORITY\_TYPE$ |
| $DEFAULT\_PRIORITY = 0$              |

## 7.The type of Process Deadline

$DEADLINE\_TYPE ::= SOFT \mid HARD$

## 8.The type of Process Attributes

|                                      |
|--------------------------------------|
| $PROCESS\_ATTRIBUTE\_TYPE$           |
| $Name : PROCESS\_NAME\_TYPE$         |
| $ProcessKind : PROCESS\_KIND\_TYPE$  |
| $EntryPoint : SYSTEM\_ADDRESS\_TYPE$ |
| $StackSize : STACK\_SIZE\_TYPE$      |
| $BasePriority : PRIORITY\_TYPE$      |
| $Period : SYSTEM\_TIME\_TYPE$        |
| $TimeCapacity : SYSTEM\_TIME\_TYPE$  |
| $Deadline : DEADLINE\_TYPE$          |

## 9.The type of Process State

$PROCESS\_STATE\_TYPE ::= DORMANT \mid READY \mid RUNNING \mid WAITING$

## 10.The type of Process Status

|                                        |
|----------------------------------------|
| $PROCESS\_STATUS\_TYPE$                |
| $Attribute : PROCESS\_ATTRIBUTE\_TYPE$ |
| $CurrentPriority : PRIORITY\_TYPE$     |
| $DeadlineTime : SYSTEM\_TIME\_TYPE$    |
| $ProcessState : PROCESS\_STATE\_TYPE$  |

## 11.The type of Process Control Block

*PROCESS\_CONTROL\_BLOCK\_TYPE*

*Name* : *PROCESS\_NAME\_TYPE*  
*ProcessKind* : *PROCESS\_KIND\_TYPE*  
*ExeFilePath* : *PATH\_TYPE*  
*SwapFilePath* : *PATH\_TYPE*  
*EntryPoint* : *SYSTEM\_ADDRESS\_TYPE*  
*KernelStack* : *MEMORY\_BLOCK\_TYPE*  
*VirtualMemory* : *PROCESS\_VIRTUAL\_MEMORY\_TYPE*  
*Period* : *SYSTEM\_TIME\_TYPE*  
*TimeCapacity* : *SYSTEM\_TIME\_TYPE*  
*Deadline* : *DEADLINE\_TYPE*  
*BasePriority* : *PRIORITY\_TYPE*  
*CurrentPriority* : *PRIORITY\_TYPE*  
*ReleasePoint* : *SYSTEM\_TIME\_TYPE*  
*DeadlineTime* : *SYSTEM\_TIME\_TYPE*  
*ProcessState* : *PROCESS\_STATE\_TYPE*  
*UserTempContext* : *seq[CONTEXT\_TYPE]*  
*KernelTempContext* : *seq[CONTEXT\_TYPE]*

$\text{blockspace}(\text{KernelStack}) \subset \text{blockspace}(\text{KERNEL\_VIRTUAL\_ADDRESS\_SPACE})$   
 $\text{KernelStack.Size} = \text{KERNEL\_STACK\_SIZE}$

## 12.The constants relates to NULL Process

*NULL\_PROCESS\_ID* : *PROCESS\_ID\_TYPE*  
*NULL\_PROCESS\_STATUS* : *PROCESS\_STATUS\_TYPE*  
 $\text{NULL\_PROCESS\_ID} \notin 0 \dots \text{PROCESS\_NUMBER\_LIMIT}$

## 13.The constants relates to Idle Process

*IDLE\_PROCESS\_ID* : *PROCESS\_ID\_TYPE*  
*IDLE\_PROCESS\_REGSTATE* : *CPU\_REGISTER\_TYPE*  
*IDLE\_PROCESS\_CONTROL\_BLOCK* : *PROCESS\_CONTROL\_BLOCK\_TYPE*  
 $\text{IDLE\_PROCESS\_ID} = 0$   
 $\text{IDLE\_PROCESS\_CONTROL\_BLOCK.Name} = \text{IdleProcess}$   
 $\text{IDLE\_PROCESS\_CONTROL\_BLOCK.ProcessKind} = \text{APERIODIC}$   
 $\text{IDLE\_PROCESS\_CONTROL\_BLOCK.ExeFilePath} = \text{NULL\_DISK\_ADDRESS}$   
 $\text{IDLE\_PROCESS\_CONTROL\_BLOCK.SwapFilePath} = \text{NULL\_DISK\_ADDRESS}$   
 $\text{IDLE\_PROCESS\_CONTROL\_BLOCK.VirtualMemory.VMBlock.Memory} = \text{NULL\_BLOCK}$   
 $\text{IDLE\_PROCESS\_CONTROL\_BLOCK.VirtualMemory.VMBlock.Base} = \emptyset$   
 $\text{IDLE\_PROCESS\_CONTROL\_BLOCK.Period} = -1$   
 $\text{IDLE\_PROCESS\_CONTROL\_BLOCK.TimeCapacity} = -1$   
 $\text{IDLE\_PROCESS\_CONTROL\_BLOCK.CurrentPriority} = 0$   
 $\text{IDLE\_PROCESS\_CONTROL\_BLOCK.ProcessState} \in \{\text{RUNNING}, \text{READY}\}$   
 $\text{IDLE\_PROCESS\_CONTROL\_BLOCK.UserTempContext} = \langle \rangle$

### A.4.3 Partition Kernel

#### 1.The type of Partition Identifier

$\text{PARTITION\_ID\_TYPE} == \text{KERNEL\_ID\_TYPE} \setminus \{\text{CORE\_KERNEL}\}$

## 2.The constant NULL \_ PARTITION \_ ID

|                                                               |
|---------------------------------------------------------------|
| $NULL\_PARTITION\_ID : PARTITION\_ID\_TYPE$                   |
| $NULL\_PARTITION\_ID \notin 1 \dots PARTITION\_NUMBER\_LIMIT$ |

## 3.The type of Partition Name

$PARTITION\_NAME\_TYPE == STRING$

## 4.The type of Partition Periodicity

|                                                     |
|-----------------------------------------------------|
| $PARTITION\_PERIODICITY\_TYPE$                      |
| $Period : SYSTEM\_TIME\_TYPE$                       |
| $Duration : SYSTEM\_TIME\_TYPE$                     |
| $Period \geq Duration$                              |
| $Period \bmod bintosigned(ClockTickInterval) = 0$   |
| $Duration > 0$                                      |
| $Duration \bmod bintosigned(ClockTickInterval) = 0$ |

## 5.The type of Partition Lock Level

$LOCK\_LEVEL\_TYPE == UNSIGNED\_INTEGER\_TYPE$

## 6.The type of Partition Operating Mode

$OPERATING\_MODE\_TYPE ::= IDLE \mid COLD\_START \mid WARM\_START \mid NORMAL$

## 7.The type of Partition Start Condition

$START\_CONDITION\_TYPE ::= NORMAL\_START \mid PARTITION\_RESTART$   
 $\mid HM\_MODULE\_RESTART \mid HM\_PARTITION\_RESTART$

## 8.The type of Partition Status

|                                           |
|-------------------------------------------|
| $PARTITION\_STATUS\_TYPE$                 |
| $PartitionId : PARTITION\_ID\_TYPE$       |
| $Period : SYSTEM\_TIME\_TYPE$             |
| $Duration : SYSTEM\_TIME\_TYPE$           |
| $Locklevel : LOCK\_LEVEL\_TYPE$           |
| $OperatingMode : OPERATING\_MODE\_TYPE$   |
| $StartCondition : START\_CONDITION\_TYPE$ |

## 9.The type of Partition Control Block

|                                              |
|----------------------------------------------|
| $PARTITION\_CONTROL\_BLOCK\_TYPE$            |
| $Name : PARTITION\_NAME\_TYPE$               |
| $Memory : PHYSICAL\_MEMORY\_BLOCK\_TYPE$     |
| $Periodicity : PARTITION\_PERIODICITY\_TYPE$ |
| $LockLevel : LOCK\_LEVEL\_TYPE$              |
| $OperatingMode : OPERATING\_MODE\_TYPE$      |
| $StartCondition : START\_CONDITION\_TYPE$    |



## 10.The type of Process Table

$PROCESS\_TABLE\_TYPE == PROCESS\_ID\_TYPE \bowtie PROCESS\_CONTROL\_BLOCK\_TYPE$

## 11.The type of Time Counter

$TIME\_COUNTER\_TYPE$

$ProcessId : PROCESS\_ID\_TYPE$

$Alarm : SYSTEM\_TIME\_TYPE$

## 12.The type of Partition Kernel State

$PARTITION\_KERNEL\_STATE\_TYPE$

$MemoryManagement : AREA\_MEMORY\_MANAGEMENT\_TYPE$

$KernelPageTableRef : PAGE\_TABLE\_TYPE$

$Periodicity : PARTITION\_PERIODICITY\_TYPE$

$TotalProcess : UNSIGNED\_INTEGER\_TYPE$

$ProcessTable : PROCESS\_TABLE\_TYPE$

$TimeCounterQueue : iseq[TIME\_COUNTER\_TYPE]$

$ReadyQueue : iseq[PROCESS\_ID\_TYPE]$

$WaitingQueue : iseq[PROCESS\_ID\_TYPE]$

$CurrentProcess : PROCESS\_ID\_TYPE$

$(\forall i : PROCESS\_ID\_TYPE \mid i \in \text{dom } ProcessTable \bullet i \in 0 \dots TotalProcess)$

$(\forall i, j : PROCESS\_ID\_TYPE \mid i, j \in \text{dom } ProcessTable \bullet$

$i \neq j \Rightarrow \text{blockspace}(ProcessTable(i).KernelStack) \cap \text{blockspace}(ProcessTable(j).KernelStack) = \emptyset)$

$(\forall i, j : PROCESS\_ID\_TYPE \mid i, j \in \text{dom } ProcessTable \bullet$

$i \neq j \Rightarrow ProcessTable(i).VirtualMemory.VMBlock.Base \cap ProcessTable(j).VirtualMemory.VMBlock.Base = \emptyset)$

$(\forall tc : TIME\_COUNTER\_TYPE \mid tc \in \text{ran } TimeCounterQueue \bullet tc.ProcessId \in \text{dom } ProcessTable)$

$(\forall i, j : \mathbb{N}_1 \mid i, j \in \text{dom } TimeCounterQueue \bullet$

$i < j \Rightarrow |TimeCounterQueue(i).Alarm| \leq |TimeCounterQueue(j).Alarm|)$

$(\forall i : PROCESS\_ID\_TYPE \mid i \in \text{ran } ReadyQueue \bullet$

$i \in \text{dom } ProcessTable \wedge ProcessTable(i).ProcessState \in \{READY, WAITING\})$

$(\forall i : PROCESS\_ID\_TYPE \mid i \in \text{ran } WaitingQueue \bullet$

$i \in \text{dom } ProcessTable \wedge ProcessTable(i).ProcessState = WAITING)$

$CurrentProcess \in \{NULL\_PROCESS\_ID\} \cup \text{dom } ProcessTable$

$(\forall i, j : PROCESS\_ID\_TYPE \mid i, j \in 0 \dots (TotalProcess - 1) \cap \text{dom } ProcessTable \bullet$

$ProcessTable(i).ProcessState = RUNNING \wedge ProcessTable(j).ProcessState = RUNNING \Rightarrow i = j)$

## 13.The type of Partition Kernel Configuration

$PARTITION\_KERNEL\_CONFIG\_TYPE$

$Name : PARTITION\_NAME\_TYPE$

$Memory : PHYSICAL\_MEMORY\_BLOCK\_TYPE$

$Periodicity : PARTITION\_PERIODICITY\_TYPE$

$TotalProcess : UNSIGNED\_INTEGER\_TYPE$

$Memory.Size > 0$

$TotalProcess + 1 \leq PROCESS\_NUMBER\_LIMIT$

## A.5 ARINC 653 O/S Layer(Operating System Kernel)

### A.5.1 Operating System Kernel

#### 1.The type of OS Kernel Configuration

---

*OS\_KERNEL\_CONFIG\_TYPE*

*PhysicalMemory* : *PHYSICAL\_MEMORY\_BLOCK\_TYPE*

*KernelMemory* : *PHYSICAL\_MEMORY\_BLOCK\_TYPE*

*KernelImage* : *PHYSICAL\_MEMORY\_BLOCK\_TYPE*

*Partitions* : *iseq<sub>1</sub>*[*PARTITION\_KERNEL\_CONFIG\_TYPE*]

*PartitionOperationSequence* : *iseq<sub>1</sub>*[*PARTITION\_TIME\_WINDOW\_CONFIG\_TYPE*]

---

*PhysicalMemory.Start* = 0<sub>PSU</sub>

*PhysicalMemory.Size* ≤ *KERNEL\_VIRTUAL\_ADDRESS\_SPACE.Size*

*KernelMemory.Start* = 0<sub>PSU</sub>

*KernelMemory.Size* < *PhysicalMemory.Size*

*blockspace*(*KernelImage*) ⊂ *blockspace*(*KernelMemory*)

# *Partitions* ≤ *PARTITION\_NUMBER\_LIMIT*

*blockspace*(*KernelMemory*) ∪  $\bigcup_{i \in \text{dom } \textit{Partitions}}$  *blockspace*(*Partitions*(*i*).*Memory*) = *blockspace*(*PhysicalMemory*)

(∀ *i* :  $\mathbb{N}_1$  | *i*, *j* ∈ dom *Partitions* •

*blockspace*(*Partitions*(*i*).*Memory*) ∩ *blockspace*(*KernelMemory*) = ∅)

(∀ *i*, *j* :  $\mathbb{N}_1$  | *i*, *j* ∈ dom *Partitions* •

*i* ≠ *j* ⇒ *Partitions*(*i*).*Name* ≠ *Partitions*(*j*).*Name*

∧ *blockspace*(*Partitions*(*i*).*Memory*) ∩ *blockspace*(*Partitions*(*j*).*Memory*) = ∅)

(∀ *i*, *j* :  $\mathbb{N}_1$  | *i*, *j* ∈ dom *Partitions* •

*Partitions*(*i*).*Periodicity.Period* ≥ *Partitions*(*j*).*Periodicity.Period* ⇒

*Partitions*(*i*).*Periodicity.Period* mod *Partitions*(*j*).*Periodicity.Period* = 0)

---

## A.6 Application/Executive(APEX) Layer

### A.6.1 Basic Definition

#### 1.The type of Return Code

*RETURN\_CODE\_TYPE* ::= *NO\_ERROR* | *NO\_ACTION* | *NOT\_AVAILABLE* | *INVALID\_PARAM*  
| *INVALID\_CONFIG* | *INVALID\_MODE* | *TIMED\_OUT*

## A.7 Core Module

### A.7.1 Core Module

#### 1.The type of Module Identifier

*MODULE\_ID\_TYPE* == *UNSIGNED\_INTEGER\_TYPE*

#### 2.The type of Module Name

*MODULE\_NAME\_TYPE* == *STRING*

#### 3.The type of Module Base Information

---

*MODULE\_BASE\_TYPE*

*ModuleId* : *MODULE\_ID\_TYPE*

*ModuleName* : *MODULE\_NAME\_TYPE*

---

#### 4.The type of Module Configuration

---

*MODULE\_CONFIG\_TYPE*

*ModuleBase* : *MODULE\_BASE\_TYPE*

*InterruptHandlerConfig* : *INTERRUPT\_HANDLER\_CONFIG\_TYPE*

*OSKernelConfig* : *OS\_KERNEL\_CONFIG\_TYPE*

---

## B Z Operations

### B.1 Core Hardware Layer

#### B.1.1 Generic CPU

##### 1.The initialization of CPU Registers

|                                                                                                                                                                                                                                                                                                                                                                                                                                                                                                                                                                                                                                                                                                                                                                                                                                      |
|--------------------------------------------------------------------------------------------------------------------------------------------------------------------------------------------------------------------------------------------------------------------------------------------------------------------------------------------------------------------------------------------------------------------------------------------------------------------------------------------------------------------------------------------------------------------------------------------------------------------------------------------------------------------------------------------------------------------------------------------------------------------------------------------------------------------------------------|
| $\begin{aligned} & \text{InitCPURegister} \\ & \text{CPU\_REGISTER\_TYPE'} \\ & (\forall i : \mathbb{N} \mid i \in \text{dom } GPRegisters' \bullet GPRegisters'(i) = 0_{PSU}) \\ & (SSRegisters').SS = 0_{PSU} \\ & (SSRegisters').SL = 0_{PSU} \\ & (SSRegisters').BP = 0_{PSU} \\ & (SSRegisters').SP = 0_{PSU} \\ & (DSRegisters').DS = 0_{PSU} \\ & (DSRegisters').DL = 0_{PSU} \\ & (DSRegisters').SI = 0_{PSU} \\ & (DSRegisters').DI = 0_{PSU} \\ & (CSRegisters').CS = 0_{PSU} \\ & (CSRegisters').CL = 0_{PSU} \\ & (CSRegisters').IP = 0_{PSU} \\ & (PSWRegisters').CF = 0 \\ & (PSWRegisters').PF = 0 \\ & (PSWRegisters').AF = 0 \\ & (PSWRegisters').ZF = 0 \\ & (PSWRegisters').SF = 0 \\ & (PSWRegisters').OF = 0 \\ & (PSWRegisters').TF = 0 \\ & (PSWRegisters').DF = 0 \\ & (PSWRegisters').IF = 0 \end{aligned}$ |
|--------------------------------------------------------------------------------------------------------------------------------------------------------------------------------------------------------------------------------------------------------------------------------------------------------------------------------------------------------------------------------------------------------------------------------------------------------------------------------------------------------------------------------------------------------------------------------------------------------------------------------------------------------------------------------------------------------------------------------------------------------------------------------------------------------------------------------------|

##### 2.The saving of part CPU Registers

*SavePartCPURegister*

$cpureg! : CPU\_REGISTER\_TYPE$

$(\exists reg : CPU\_REGISTER\_TYPE \bullet$   
   $(\exists stackreg : SSREGISTER\_TYPE; dsreg : DSREGISTER\_TYPE;$   
     $csreg : CSREGISTER\_TYPE; pswreg : PSWREGISTER\_TYPE \bullet$   
     $(\forall i : \mathbb{N} \mid i \in \text{dom}(reg.GPRegisters) \bullet reg.GPRegisters(i) = 0_{PSU})$   
     $\wedge reg.SSRegisters.SS = stackreg.SS$   
     $\wedge reg.SSRegisters.SL = stackreg.SL$   
     $\wedge reg.SSRegisters.BP = stackreg.BP$   
     $\wedge reg.SSRegisters.SP = stackreg.SP$   
     $\wedge reg.DSRegisters.DS = dsreg.DS$   
     $\wedge reg.DSRegisters.DI = dsreg.DI$   
     $\wedge reg.DSRegisters.SI = dsreg.SI$   
     $\wedge reg.DSRegisters.DI = dsreg.DI$   
     $\wedge reg.CSRegisters.CS = csreg.CS$   
     $\wedge reg.CSRegisters.CL = csreg.CL$   
     $\wedge reg.CSRegisters.IP = csreg.IP$   
     $\wedge reg.PSWRegisters.CF = pswreg.CF$   
     $\wedge reg.PSWRegisters.PF = pswreg.PF$   
     $\wedge reg.PSWRegisters.AF = pswreg.AF$   
     $\wedge reg.PSWRegisters.ZF = pswreg.ZF$   
     $\wedge reg.PSWRegisters.SF = pswreg.SF$   
     $\wedge reg.PSWRegisters.OF = pswreg.OF$   
     $\wedge reg.PSWRegisters.TF = pswreg.TF$   
     $\wedge reg.PSWRegisters.DF = pswreg.DF$   
     $\wedge reg.PSWRegisters.IF = pswreg.IF)$   
     $\wedge cpureg! = reg)$

### 3.The saving of all CPU Registers

*SaveAllCPURegister*

*cpureg!* : *CPU\_REGISTER\_TYPE*

$$\begin{aligned}
& (\exists \text{ reg} : \text{CPU\_REGISTER\_TYPE}; \\
& (\exists \text{ gpreg} : \text{GPREGISTER\_TYPE}; \text{stackreg} : \text{SSREGISTER\_TYPE}; \text{dsreg} : \text{DSREGISTER\_TYPE}; \\
& \quad \text{csreg} : \text{CSREGISTER\_TYPE}; \text{pswreg} : \text{PSWREGISTER\_TYPE} \bullet \\
& (\forall i : \mathbb{N} \mid i \in \text{dom}(\text{reg.GPRegisters}) \bullet \text{reg.GPRegisters}(i) = \text{gpreg}(i)) \\
& \wedge \text{reg.SSRegisters.SS} = \text{stackreg.SS} \\
& \wedge \text{reg.SSRegisters.SL} = \text{stackreg.SL} \\
& \wedge \text{reg.SSRegisters.BP} = \text{stackreg.BP} \\
& \wedge \text{reg.SSRegisters.SP} = \text{stackreg.SP} \\
& \wedge \text{reg.DSRegisters.DS} = \text{dsreg.DS} \\
& \wedge \text{reg.DSRegisters.DI} = \text{dsreg.DI} \\
& \wedge \text{reg.DSRegisters.SI} = \text{dsreg.SI} \\
& \wedge \text{reg.DSRegisters.DI} = \text{dsreg.DI} \\
& \wedge \text{reg.CSRegisters.CS} = \text{csreg.CS} \\
& \wedge \text{reg.CSRegisters.CL} = \text{csreg.CL} \\
& \wedge \text{reg.CSRegisters.IP} = \text{csreg.IP} \\
& \wedge \text{reg.PSWRegisters.CF} = \text{pswreg.CF} \\
& \wedge \text{reg.PSWRegisters.PF} = \text{pswreg.PF} \\
& \wedge \text{reg.PSWRegisters.AF} = \text{pswreg.AF} \\
& \wedge \text{reg.PSWRegisters.ZF} = \text{pswreg.ZF} \\
& \wedge \text{reg.PSWRegisters.SF} = \text{pswreg.SF} \\
& \wedge \text{reg.PSWRegisters.OF} = \text{pswreg.OF} \\
& \wedge \text{reg.PSWRegisters.TF} = \text{pswreg.TF} \\
& \wedge \text{reg.PSWRegisters.DF} = \text{pswreg.DF} \\
& \wedge \text{reg.PSWRegisters.IF} = \text{pswreg.IF}) \\
& \wedge \text{cpureg!} = \text{reg})
\end{aligned}$$

#### 4.The restoring of part CPU Registers

*RestorePartCPURegister*

*cpureg?* : CPU\_REGISTER\_TYPE

$(\exists \text{stackreg} : \text{SSREGISTER\_TYPE}; \text{dsreg} : \text{DSREGISTER\_TYPE};$   
 $\text{csreg} : \text{CSREGISTER\_TYPE}; \text{pswreg} : \text{PSWREGISTER\_TYPE} \bullet$   
 $\text{stackreg.SS} = (\text{cpureg?}).\text{SSRegisters.SS}$   
 $\wedge \text{stackreg.SL} = (\text{cpureg?}).\text{SSRegisters.SL}$   
 $\wedge \text{stackreg.BP} = (\text{cpureg?}).\text{SSRegisters.BP}$   
 $\wedge \text{stackreg.SP} = (\text{cpureg?}).\text{SSRegisters.SP}$   
 $\wedge \text{dsreg.DS} = (\text{cpureg?}).\text{DSRegisters.DS}$   
 $\wedge \text{dsreg.DI} = (\text{cpureg?}).\text{DSRegisters.DI}$   
 $\wedge \text{dsreg.SI} = (\text{cpureg?}).\text{DSRegisters.SI}$   
 $\wedge \text{dsreg.DI} = (\text{cpureg?}).\text{DSRegisters.DI}$   
 $\wedge \text{csreg.CS} = (\text{cpureg?}).\text{CSRegisters.CS}$   
 $\wedge \text{csreg.CL} = (\text{cpureg?}).\text{CSRegisters.CL}$   
 $\wedge \text{csreg.IP} = (\text{cpureg?}).\text{CSRegisters.IP}$   
 $\wedge \text{pswreg.CF} = (\text{cpureg?}).\text{PSWRegisters.CF}$   
 $\wedge \text{pswreg.PF} = (\text{cpureg?}).\text{PSWRegisters.PF}$   
 $\wedge \text{pswreg.AF} = (\text{cpureg?}).\text{PSWRegisters.AF}$   
 $\wedge \text{pswreg.ZF} = (\text{cpureg?}).\text{PSWRegisters.ZF}$   
 $\wedge \text{pswreg.SF} = (\text{cpureg?}).\text{PSWRegisters.SF}$   
 $\wedge \text{pswreg.OF} = (\text{cpureg?}).\text{PSWRegisters.OF}$   
 $\wedge \text{pswreg.TF} = (\text{cpureg?}).\text{PSWRegisters.TF}$   
 $\wedge \text{pswreg.DF} = (\text{cpureg?}).\text{PSWRegisters.DF}$   
 $\wedge \text{pswreg.IF} = (\text{cpureg?}).\text{PSWRegisters.IF})$

## 5.The restoring of all CPU Registers

*RestoreAllCPURegister*

*cpureg?* : CPU\_REGISTER\_TYPE

$(\exists \text{gpreg} : \text{GPREGISTER\_TYPE}; \text{stackreg} : \text{SSREGISTER\_TYPE}; \text{dsreg} : \text{DSREGISTER\_TYPE};$   
 $\text{csreg} : \text{CSREGISTER\_TYPE}; \text{pswreg} : \text{PSWREGISTER\_TYPE} \bullet$   
 $(\forall i : \mathbb{N} \mid i \in \text{dom gpreg} \bullet \text{gpreg}(i) = (\text{cpureg?}).\text{GPRegisters}(i))$   
 $\wedge \text{stackreg.SS} = (\text{cpureg?}).\text{SSRegisters.SS}$   
 $\wedge \text{stackreg.SL} = (\text{cpureg?}).\text{SSRegisters.SL}$   
 $\wedge \text{stackreg.BP} = (\text{cpureg?}).\text{SSRegisters.BP}$   
 $\wedge \text{stackreg.SP} = (\text{cpureg?}).\text{SSRegisters.SP}$   
 $\wedge \text{dsreg.DS} = (\text{cpureg?}).\text{DSRegisters.DS}$   
 $\wedge \text{dsreg.DI} = (\text{cpureg?}).\text{DSRegisters.DI}$   
 $\wedge \text{dsreg.SI} = (\text{cpureg?}).\text{DSRegisters.SI}$   
 $\wedge \text{dsreg.DI} = (\text{cpureg?}).\text{DSRegisters.DI}$   
 $\wedge \text{csreg.CS} = (\text{cpureg?}).\text{CSRegisters.CS}$   
 $\wedge \text{csreg.CL} = (\text{cpureg?}).\text{CSRegisters.CL}$   
 $\wedge \text{csreg.IP} = (\text{cpureg?}).\text{CSRegisters.IP}$   
 $\wedge \text{pswreg.CF} = (\text{cpureg?}).\text{PSWRegisters.CF}$   
 $\wedge \text{pswreg.PF} = (\text{cpureg?}).\text{PSWRegisters.PF}$   
 $\wedge \text{pswreg.AF} = (\text{cpureg?}).\text{PSWRegisters.AF}$   
 $\wedge \text{pswreg.ZF} = (\text{cpureg?}).\text{PSWRegisters.ZF}$   
 $\wedge \text{pswreg.SF} = (\text{cpureg?}).\text{PSWRegisters.SF}$   
 $\wedge \text{pswreg.OF} = (\text{cpureg?}).\text{PSWRegisters.OF}$   
 $\wedge \text{pswreg.TF} = (\text{cpureg?}).\text{PSWRegisters.TF}$   
 $\wedge \text{pswreg.DF} = (\text{cpureg?}).\text{PSWRegisters.DF}$   
 $\wedge \text{pswreg.IF} = (\text{cpureg?}).\text{PSWRegisters.IF})$

## 6.The setting of Stack Segment Registers

|                                                                                                                                              |
|----------------------------------------------------------------------------------------------------------------------------------------------|
| <i>SetStackSegRegister</i>                                                                                                                   |
| $\Delta CPU\_REGISTER\_TYPE$                                                                                                                 |
| $ssreg? : SSREGISTER\_TYPE$                                                                                                                  |
| $(SSRegister').SS = (ssreg?).SS$<br>$(SSRegister').SL = (ssreg?).SL$<br>$(SSRegister').BP = (ssreg?).BP$<br>$(SSRegister').SP = (ssreg?).SP$ |

### B.1.2 Memory Management Unit (MMU)

#### 1.The translation of linear address

|                                                                                                                                                                                          |
|------------------------------------------------------------------------------------------------------------------------------------------------------------------------------------------|
| <i>TransLinearAddress</i>                                                                                                                                                                |
| $\exists MEMORY\_MANAGEMENT\_UNIT\_TYPE$                                                                                                                                                 |
| $la? : SYSTEM\_ADDRESS\_TYPE$                                                                                                                                                            |
| $pa! : SYSTEM\_ADDRESS\_TYPE$                                                                                                                                                            |
| $(\exists a : SYSTEM\_ADDRESS\_TYPE \mid a \in \text{ran } PageTableBuffer \bullet$<br>$getpage(a) = PageTableBuffer(getpage(la?)) \wedge getoffset(a) = getoffset(la?) \wedge pa! = a)$ |

### B.1.3 Main Memory

#### 1.The loading of a page in Main Memory

|                                                                                                                        |
|------------------------------------------------------------------------------------------------------------------------|
| <i>LoadPage</i>                                                                                                        |
| $\Delta MAIN\_MEMORY\_TYPE$                                                                                            |
| $page? : PAGE\_TYPE$                                                                                                   |
| $piece? : PIECE\_TYPE$                                                                                                 |
| $(\forall a : SYSTEM\_ADDRESS\_TYPE \mid a \in \text{dom } piece? \bullet Store'(page? + getoffset(a)) = (piece?)(a))$ |

#### 2.The extraction of a page in Main Memory

|                                                                                                                                                                                               |
|-----------------------------------------------------------------------------------------------------------------------------------------------------------------------------------------------|
| <i>ExtractPage</i>                                                                                                                                                                            |
| $\exists MAIN\_MEMORY\_TYPE$                                                                                                                                                                  |
| $page? : PAGE\_TYPE$                                                                                                                                                                          |
| $piece! : PIECE\_TYPE$                                                                                                                                                                        |
| $(\exists p : PIECE\_TYPE \bullet$<br>$(\forall a : SYSTEM\_ADDRESS\_TYPE \mid a \in \text{dom } Store \wedge a \in \text{pagespace}(page?) \bullet p(a) = Store(a))$<br>$\wedge piece! = p)$ |

### B.1.4 Timer

#### 1.The initialization of Timer

|                                      |
|--------------------------------------|
| <i>InitTimer</i>                     |
| $TIMER\_TYPE'$                       |
| $p? : PSU$                           |
| $Value' = 0_{PSU}$<br>$Period' = p?$ |

### B.1.5 High-Precision Timer

#### 1.The initialization of High-Precision Timer

|                        |                  |
|------------------------|------------------|
| $InitHPTimer$          | $HPTIMER\_TYPE'$ |
| $Value' = 0_{PSU}$     |                  |
| $Alarm' = LIMIT_{PSU}$ |                  |

### B.1.6 Interrupt Controller

#### 1.The initialization of Interrupt Controller

|                                                                                           |                                |
|-------------------------------------------------------------------------------------------|--------------------------------|
| $InitInterruptController$                                                                 | $INTERRUPT\_CONTROLLER\_TYPE'$ |
| $(\forall i : \mathbb{N} \mid i \in \text{dom } IRRegisters' \bullet IRRegister'(i) = 0)$ |                                |
| $(\forall j : \mathbb{N} \mid j \in \text{dom } IMRegisters' \bullet IMRegister'(j) = 0)$ |                                |
| $(\forall k : \mathbb{N} \mid k \in \text{dom } ISRegisters' \bullet ISRegister'(k) = 0)$ |                                |

#### 2.The information of Requesting interrupts

|                                                                                         |                                       |
|-----------------------------------------------------------------------------------------|---------------------------------------|
| $GetRequestInterrupts$                                                                  | $\exists INTERRUPT\_CONTROLLER\_TYPE$ |
| $ints! : \mathbb{P} INTERRUPT\_TYPE$                                                    |                                       |
| $ints! = \{i : \mathbb{N} \mid i \in \text{dom } IRRegister \wedge IRRegister(i) = 1\}$ |                                       |

#### 3.The information of Masked interrupts

|                                                                                         |                                       |
|-----------------------------------------------------------------------------------------|---------------------------------------|
| $GetMaskedInterrupts$                                                                   | $\exists INTERRUPT\_CONTROLLER\_TYPE$ |
| $ints! : \mathbb{P} INTERRUPT\_TYPE$                                                    |                                       |
| $ints! = \{i : \mathbb{N} \mid i \in \text{dom } IMRegister \wedge IMRegister(i) = 1\}$ |                                       |

#### 4.The information of In-Service interrupts

|                                                                                         |                                       |
|-----------------------------------------------------------------------------------------|---------------------------------------|
| $GetInServiceInterrupts$                                                                | $\exists INTERRUPT\_CONTROLLER\_TYPE$ |
| $ints! : \mathbb{P} INTERRUPT\_TYPE$                                                    |                                       |
| $ints! = \{i : \mathbb{N} \mid i \in \text{dom } ISRegister \wedge ISRegister(i) = 1\}$ |                                       |

## B.2 Hardware Interface Software Layer

### B.2.1 Context Switching

#### 1.The creating of Stack Segment



*CreateStackSegment* \_\_\_\_\_

$ss? : PSU$   
 $sl? : PSU$   
 $bp? : PSU$   
 $sp? : PSU$   
 $ssreg! : SSREGISTER\_TYPE$

$(\exists reg : SSREGISTER\_TYPE \bullet$   
 $reg.SS = ss? \wedge reg.Sl = sl? \wedge reg.BP = bp? \wedge reg.SP = sp? \wedge ssreg! = reg)$

## B.2.2 Memory Management

### 1.The initialization of Memory Management

*InitMemoryManagement* \_\_\_\_\_

$MEMORY\_MANAGEMENT\_STATE\_TYPE'$   
 $areamm? : AREA\_MEMORY\_MANAGEMENT\_TYPE$

$AreaMemoryManagementRef' = areamm?$

### 2.The information of the max Free Block

*GetMaxFreeBlock* \_\_\_\_\_

$\exists MEMORY\_MANAGEMENT\_STATE\_TYPE$   
 $maxblk! : MEMORY\_BLOCK\_TYPE$

$(\exists maxblk : MEMORY\_BLOCK\_TYPE \bullet$   
 $totalpage(maxblk) \subseteq AreaMemoryManagementRef.Free$   
 $\wedge (\forall blk : MEMORY\_BLOCK\_TYPE \bullet$   
 $totalpage(blk) \subseteq AreaMemoryManagementRef.Free \Rightarrow blk.Size \leq maxblk.Size)$   
 $\wedge maxblk! = maxblk)$

### 3.The allocation of Physical Memory Page

*AllocPhysicalMemoryPage* \_\_\_\_\_

$\Delta MEMORY\_MANAGEMENT\_STATE\_TYPE$   
 $n? : UNSIGNED\_INTEGER\_TYPE$   
 $pages! : \mathbb{P} PAGE\_TYPE$

$(\exists ps : \mathbb{P} PAGE\_TYPE \bullet$   
 $ps \subseteq AreaMemoryManagementRef.Free \wedge \#ps = n? \wedge pages! = ps$   
 $\wedge (AreaMemoryManagementRef').Allocated = AreaMemoryManagementRef.Allocated \cup ps$   
 $\wedge (AreaMemoryManagementRef').Free = AreaMemoryManagementRef.Free \setminus ps)$

### 4.The allocation of Physical Memory Block

*AllocPhysicalMemoryBlock* \_\_\_\_\_

$\Delta MEMORY\_MANAGEMENT\_STATE\_TYPE$   
 $size? : UNSIGNED\_INTEGER\_TYPE$   
 $block! : MEMORY\_BLOCK\_TYPE$

$(\exists blk : MEMORY\_BLOCK\_TYPE \bullet$   
 $totalpage(blk) \subseteq AreaMemoryManagementRef.Free \wedge blk.Size = size? \wedge block! = blk$   
 $\wedge (AreaMemoryManagementRef').Allocated = AreaMemoryManagementRef.Allocated \cup totalpage(blk)$   
 $\wedge (AreaMemoryManagementRef').Free = AreaMemoryManagementRef.Free \setminus totalpage(blk))$

## 5.The deallocation of Physical Memory Page

*DeallocPhysicalMemoryPage* \_\_\_\_\_

$\Delta MEMORY\_MANAGEMENT\_STATE\_TYPE$

$pages? : \mathbb{P} PAGE\_TYPE$

$(AreaMemoryManagementRef').Allocated = AreaMemoryManagementRef.Allocated \setminus pages?$   
 $(AreaMemoryManagementRef').Free = AreaMemoryManagementRef.Free \cup pages?$

## 6.The creating of Memory Block

*CreateMemoryBlock* \_\_\_\_\_

$start? : PAGE\_TYPE$

$size? : UNSIGNED\_INTEGER\_TYPE$

$block! : MEMORY\_BLOCK\_TYPE$

$(\exists blk : MEMORY\_BLOCK\_TYPE \bullet blk.Start = start? \wedge blk.Size = size? \wedge block! = blk)$

## 7.The creating of Process Virtual Memory

*CreateProcessVirtualMemory* \_\_\_\_\_

$block? : MEMORY\_BLOCK\_TYPE$

$base? : \mathbb{P} PAGE\_TYPE$

$stack? : MEMORY\_BLOCK\_TYPE$

$data? : MEMORY\_BLOCK\_TYPE$

$code? : MEMORY\_BLOCK\_TYPE$

$procvm! : PROCESS\_VIRTUAL\_MEMORY\_TYPE$

$(\exists vm : PROCESS\_VIRTUAL\_MEMORY\_TYPE \bullet$   
 $vm.VMBlock.Memory = block? \wedge vm.VMBlock.Base = base? \wedge vm.VMBlock.PageTable = \emptyset$   
 $Stack = stack? \wedge Data = data? \wedge Code = code? \wedge procvm! = vm)$

## 8.The full loading of Process Page Table

*FullLoadProcPageTable* \_\_\_\_\_

$procvm? : PROCESS\_VIRTUAL\_MEMORY\_TYPE$

$entrypoint? : SYSTEM\_ADDRESS\_TYPE$

$pagetable! : PAGE\_TABLE\_TYPE$

$(\exists pt : PAGE\_TABLE\_TYPE \bullet$   
 $\text{dom } pt \subseteq \text{totalpage}((procvm?).VMBlock.Memory) \wedge \text{ran } pt = (procvm?).VMBlock.Base$   
 $\wedge \text{getpage}(\text{entrypoint?}) \in \text{dom } pt \wedge \text{pagetable!} = pt)$

### B.2.3 System Clock

#### 1.The initialization of System Clock

*InitSystemClock*

*SYSTEM\_CLOCK\_STATE\_TYPE'*

*bt?* : *SYSTEM\_TIME\_TYPE*

*ti?* : *SYSTEM\_TIME\_TYPE*

*BaseTime'* = *bt?*

*TickInterval'* = *ti?*

*TickCounter'* = 0

*Time'* = - 2 \* *ti?*

*InterruptTime'* = *max*(*SYSTEM\_TIME\_TYPE*)

## 2.The update of System Clock

*UpdateSystemClock*

*ΔSYSTEM\_CLOCK\_STATE\_TYPE*

*TickCounter'* = *TickCounter* + 1

*Time'* = *Time* + *TickInterval*

### B.2.4 Interrupt Handler

#### 1.The initialization of Interrupt Handler

*InitInterruptHandler*

*INTERRUPT\_HANDLER\_STATE\_TYPE'*

*intstack?* : *MEMORY\_BLOCK\_TYPE*

*pagetable?* : *PAGE\_TABLE\_TYPE*

*KernelPageTableRef'* = *pagetable?*

*InterruptStack'* = *intstack?*

*TempContexts'* =  $\langle \rangle$

## B.3 ARINC 653 O/S Layer

### B.3.1 Core Kernel

#### 1.The initialization of Core Kernel

*InitCoreKernel*

*CORE\_KERNEL\_STATE\_TYPE'*

*config? : OS\_KERNEL\_CONFIG\_TYPE*

$(MemoryManagement').Memory = (config?).KernelMemory$   
 $(MemoryManagement').Allocated = totalpage((config?).KernelImage)$   
 $(MemoryManagement').Free = totalpage((MemoryManagement').Memory) \setminus (MemoryManagement').Allocated$   
 $dom(KernelPageTable') = \{p : PAGE\_TYPE \mid p \in totalpage((config?).PhysicalMemory) \bullet$   
 $p + KERNEL\_VIRTUAL\_ADDRESS\_SPACE.Start\}$   
 $ran(KernelPageTable') = totalpage((config?).PhysicalMemory)$   
 $(\forall p : PAGE\_TYPE \mid p \in dom(KernelPageTable') \bullet$   
 $(KernelPageTable')(p) = p - KERNEL\_VIRTUAL\_ADDRESS\_SPACE.Start)$   
 $(KernelProcManagement').ProcessTable = \{IDLE\_PROCESS\_ID \mapsto IDLE\_PROCESS\_CONTROL\_BLOCK\}$   
 $(KernelProcManagement').ProcessTable(IDLE\_PROCESS\_ID).KernelTempContext = \langle makecontext(IDLE\_PROCESS\_REGSTATE, KernelPageTable') \rangle$   
 $(KernelProcManagement').CurrentProcess = NULL\_PROCESS\_ID$   
 $(\forall i : \mathbb{N}_1 \mid i \in dom((config?).Partitions) \bullet$   
 $(PartitionManagement').PartitionTable(i).Name = (config?).Partitions(i).Name$   
 $(PartitionManagement').PartitionTable(i).Memory = (config?).Partitions(i).Memory$   
 $(PartitionManagement').PartitionTable(i).Periodicity = (config?).Partitions(i).Periodicity$   
 $(PartitionManagement').PartitionTable(i).LockLevel = MIN\_LOCK\_LEVEL$   
 $(PartitionManagement').PartitionTable(i).OperatingMode = IDLE$   
 $(PartitionManagement').PartitionTable(i).StartCondition = NORMAL\_START)$   
 $(\forall i : \mathbb{N}_1 \mid i \in dom((config?).PartitionOperationSequence) \bullet$   
 $(\exists_1 j : PARTITION\_ID\_TYPE \mid j \in dom((PartitionManagement').PartitionTable) \bullet$   
 $(config?).PartitionOperationSequence(i).Name = (PartitionManagement').PartitionTable(j).Name$   
 $\wedge (PartitionManagement').MajorTimeFrame.PartitionQueue(i).PartitionId = j$   
 $\wedge (PartitionManagement').MajorTimeFrame.PartitionQueue(i).Periodicity =$   
 $(PartitionManagement').PartitionTable(i).Periodicity$   
 $\wedge (PartitionManagement').MajorTimeFrame.PartitionQueue(i).PeriodicProcStart =$   
 $(config?).PartitionOperationSequence(i).PeriodicProcStart))$   
 $(PartitionManagement').MajorTimeFrame.Length = max$   
 $(\{i : \mathbb{N}_1 \mid i \in dom((PartitionManagement').MajorTimeFrame.PartitionQueue) \bullet$   
 $(PartitionManagement').MajorTimeFrame.PartitionQueue(i).Periodicity.Period\})$   
 $(PartitionManagement').MajorTimeFrame.PartitionQueue(1).Offset = 0$   
 $(\forall i : \mathbb{N}_1 \mid i \in dom((PartitionManagement').MajorTimeFrame.PartitionQueue) \bullet$   
 $i > 1 \Rightarrow (\forall j : \mathbb{N}_1 \mid j < i \bullet$   
 $(PartitionManagement').MajorTimeFrame.PartitionQueue(i).PartitionId \neq$   
 $(PartitionManagement').MajorTimeFrame.PartitionQueue(j).PartitionId \Rightarrow$   
 $(PartitionManagement').MajorTimeFrame.PartitionQueue(i).Offset =$   
 $(PartitionManagement').MajorTimeFrame.PartitionQueue(i-1).Offset +$   
 $(PartitionManagement').MajorTimeFrame.PartitionQueue(i-1).Periodicity.Duration)$   
 $\vee (\exists k : \mathbb{N}_1 \bullet$   
 $k = max(\{j : \mathbb{N}_1 \mid j \in dom((PartitionManagement').MajorTimeFrame.PartitionQueue)$   
 $\wedge (PartitionManagement').MajorTimeFrame.PartitionQueue(i).PartitionId =$   
 $(PartitionManagement').MajorTimeFrame.PartitionQueue(j).PartitionId$   
 $\wedge j < i\})$   
 $\wedge (PartitionManagement').MajorTimeFrame.PartitionQueue(i).Offset =$   
 $(PartitionManagement').MajorTimeFrame.PartitionQueue(k).Offset +$   
 $(PartitionManagement').MajorTimeFrame.PartitionQueue(k).Periodicity.Period))$   
 $(PartitionManagement').CurrentPartition = NULL\_PARTITION\_ID$

## 2.The information of Status of current Partition

*GetPartitionStatus*

$\exists \text{CORE\_KERNEL\_STATE\_TYPE}$

$\text{parts!} : \text{PARTITION\_STATUS\_TYPE}$

$(\exists \text{status} : \text{PARTITION\_STATUS\_TYPE} \bullet$

$\wedge \text{status.PartitionId} = \text{PartitionManagement.CurrentPartition}$

$\wedge \text{status.Period} = \text{PartitionManagement.PartitionTable}(\text{PartitionManagement.CurrentPartition}).$   
 $\text{Periodicity.Period}$

$\wedge \text{status.Duration} = \text{PartitionManagement.PartitionTable}(\text{PartitionManagement.CurrentPartition}).$   
 $\text{Periodicity.Duration}$

$\wedge \text{status.LockLevel} = \text{PartitionManagement.PartitionTable}(\text{PartitionManagement.CurrentPartition}).$   
 $\text{LockLevel}$

$\wedge \text{status.OperatingMode} = \text{PartitionManagement.PartitionTable}(\text{PartitionManagement.CurrentPartition}).$   
 $\text{OperatingMode}$

$\wedge \text{status.StartCondition} = \text{PartitionManagement.PartitionTable}(\text{PartitionManagement.CurrentPartition}).$   
 $\text{StartCondition}$

$\wedge \text{parts!} = \text{status})$

### 3.The information of next Periodic Start of current Partition

*GetNextPeriodicStart*

$\exists \text{CORE\_KERNEL\_STATE\_TYPE}$

$\text{ct?} : \text{SYSTEM\_TIME\_TYPE}$

$\text{nps!} : \text{SYSTEM\_TIME\_TYPE}$

$((\exists j : \mathbb{N}_1 \mid j \in \text{dom}(\text{PartitionManagement.MajorTimeFrame.PartitionQueue}) \bullet$

$\text{PartitionManagement.MajorTimeFrame.PartitionQueue}(j).\text{PartitionId} = \text{PartitionManagement.}$   
 $\text{CurrentPartition}$

$\wedge \text{PartitionManagement.MajorTimeFrame.PartitionQueue}(j).\text{PeriodicProcStart} = \text{TRUE}$

$\wedge \text{nps!} = \min(\{k : \mathbb{N}_1; n : \mathbb{N} \mid k \in \text{dom}(\text{PartitionManagement.MajorTimeFrame.PartitionQueue})$

$\wedge \text{PartitionManagement.MajorTimeFrame.PartitionQueue}(k).\text{PartitionId} =$   
 $\text{PartitionManagement.CurrentPartition}$

$\wedge \text{PartitionManagement.MajorTimeFrame.PartitionQueue}(k).\text{PeriodicProcStart} = \text{TRUE}$

$\wedge \text{PartitionManagement.MajorTimeFrame.PartitionQueue}(k).\text{Offset} + \text{PartitionManagement.}$   
 $\text{MajorTimeFrame.Length} * n \geq \text{ct?} \bullet$

$\text{PartitionManagement.MajorTimeFrame.PartitionQueue}(k).\text{Offset} + \text{PartitionManagement.}$   
 $\text{MajorTimeFrame.Length} * n\})$

$\vee (\forall j : \mathbb{N}_1 \mid j \in \text{dom}(\text{PartitionManagement.MajorTimeFrame.PartitionQueue}) \bullet$

$\text{PartitionManagement.MajorTimeFrame.PartitionQueue}(j).\text{PartitionId} = \text{PartitionManagement.}$   
 $\text{CurrentPartition}$

$\wedge \text{PartitionManagement.MajorTimeFrame.PartitionQueue}(j).\text{PeriodicProcStart} = \text{FALSE} \Rightarrow$

$\text{nps!} = \max(\text{SYSTEM\_TIME\_TYPE}))$

### 4.The information of next Periodic Start of current Partition including the delay time

*GetDelayedPeriodicStart*

$\exists \text{CORE\_KERNEL\_STATE\_TYPE}$

$ct? : \text{SYSTEM\_TIME\_TYPE}$

$dt? : \text{SYSTEM\_TIME\_TYPE}$

$dps! : \text{SYSTEM\_TIME\_TYPE}$

$((\exists j : \mathbb{N}_1 \mid j \in \text{dom}(\text{PartitionManagement.MajorTimeFrame.PartitionQueue}) \bullet$   
 $\text{PartitionManagement.MajorTimeFrame.PartitionQueue}(j).\text{PartitionId} = \text{PartitionManagement.}$   
 $\text{CurrentPartition}$   
 $\wedge \text{PartitionManagement.MajorTimeFrame.PartitionQueue}(j).\text{PeriodicProcStart} = \text{TRUE}$   
 $\wedge dps! = \min(\{k : \mathbb{N}_1; n : \mathbb{N} \mid k \in \text{dom}(\text{PartitionManagement.MajorTimeFrame.PartitionQueue})$   
 $\wedge \text{PartitionManagement.MajorTimeFrame.PartitionQueue}(k).\text{PartitionId} =$   
 $\text{PartitionManagement.CurrentPartition}$   
 $\wedge \text{PartitionManagement.MajorTimeFrame.PartitionQueue}(k).\text{PeriodicProcStart} = \text{TRUE}$   
 $\wedge \text{PartitionManagement.MajorTimeFrame.PartitionQueue}(k).\text{Offset} + \text{PartitionManagement.}$   
 $\text{MajorTimeFrame.Length} * n \geq (ct? + dt?) \bullet$   
 $\text{PartitionManagement.MajorTimeFrame.PartitionQueue}(k).\text{Offset} + \text{PartitionManagement.}$   
 $\text{MajorTimeFrame.Length} * n\})$   
 $\vee (\forall j : \mathbb{N}_1 \mid j \in \text{dom}(\text{PartitionManagement.MajorTimeFrame.PartitionQueue}) \bullet$   
 $\text{PartitionManagement.MajorTimeFrame.PartitionQueue}(j).\text{PartitionId} = \text{PartitionManagement.}$   
 $\text{CurrentPartition}$   
 $\wedge \text{PartitionManagement.MajorTimeFrame.PartitionQueue}(j).\text{PeriodicProcStart} = \text{FALSE} \Rightarrow$   
 $dps! = \max(\text{SYSTEM\_TIME\_TYPE}))$

## 5.The information of next Partition

*GetNextPartition*

$\exists \text{CORE\_KERNEL\_STATE\_TYPE}$

$t? : \text{SYSTEM\_TIME\_TYPE}$

$partid! : \text{PARTITION\_ID\_TYPE}$

$((\exists i : \mathbb{N}_1 \mid i \in \text{dom}(\text{PartitionManagement.MajorTimeFrame.PartitionQueue}) \bullet$   
 $\text{PartitionManagement.MajorTimeFrame.PartitionQueue}(i).\text{Offset} \leq$   
 $(t? \bmod \text{PartitionManagement.MajorTimeFrame.Length})$   
 $\wedge \text{PartitionManagement.MajorTimeFrame.PartitionQueue}(i).\text{Offset} +$   
 $\text{PartitionManagement.MajorTimeFrame.PartitionQueue}(i).\text{Periodicity.Duration} >$   
 $(t? \bmod \text{PartitionManagement.MajorTimeFrame.Length})$   
 $\wedge partid! = \text{PartitionManagement.MajorTimeFrame.PartitionQueue}(i).\text{PartitionId})$   
 $\vee (\forall i : \mathbb{N}_1 \mid i \in \text{dom}(\text{PartitionManagement.MajorTimeFrame.PartitionQueue}) \bullet$   
 $\text{PartitionManagement.MajorTimeFrame.PartitionQueue}(i).\text{Offset} +$   
 $\text{PartitionManagement.MajorTimeFrame.PartitionQueue}(i).\text{Periodicity.Duration} \leq$   
 $(t? \bmod \text{PartitionManagement.MajorTimeFrame.Length})$   
 $\vee \text{PartitionManagement.MajorTimeFrame.PartitionQueue}(i).\text{Offset} >$   
 $(t? \bmod \text{PartitionManagement.MajorTimeFrame.Length}) \Rightarrow$   
 $partid! = \text{NULL\_PARTITION\_ID}))$

### B.3.2 Partition Kernel

#### 1.The initialization of Partition Kernel

*InitPartitionKernel*

$\exists \text{PARTITION\_KERNEL\_STATE\_TYPE}'$

$\text{config?} : \text{PARTITION\_KERNEL\_CONFIG\_TYPE}$

$\text{pagetable?} : \text{PAGE\_TABLE\_TYPE}$

$(\text{MemoryManagement}').\text{Memory} = (\text{config?}).\text{Memory}$

$(\text{MemoryManagement}').\text{Allocated} = \emptyset$

$(\text{MemoryManagement}').\text{Free} = \text{totalpage}((\text{MemoryManagement}').\text{Memory})$

$\text{KernelPageTableRef}' = \text{pagetable?}$

$\text{Periodicity}' = (\text{config?}).\text{Periodicity}$

$\text{TotalProcess}' = (\text{config?}).\text{TotalProcess}$

$\text{ProcessTable}' = \{\text{IDLE\_PROCESS\_ID} \mapsto \text{IDLE\_PROCESS\_CONTROL\_BLOCK}\}$

$\text{ProcessTable}'(\text{IDLE\_PROCESS\_ID}).\text{KernelTempContext} = \langle \text{makecontext}(\text{IDLE\_PROCESS\_REGSTATE}, \text{pagetable?}) \rangle$

$\text{TimeCounterQueue}' = \langle \rangle$

$\text{ReadyQueue}' = \langle \rangle$

$\text{WaitingQueue}' = \langle \rangle$

$\text{CurrentProcess}' = \text{NULL\_PROCESS\_ID}$

## 2.The information of Names of Processes

*GetProcessNames*

$\exists \text{PARTITION\_KERNEL\_STATE\_TYPE}$

$\text{procns!} : \mathbb{P} \text{PROCESS\_NAME\_TYPE}$

$\text{procns!} = \{i : \text{PROCESS\_ID\_TYPE} \mid i \in \text{dom ProcessTable} \bullet \text{ProcessTable}(i).\text{Name}\}$

## 3.The information of Process Id

*GetProcessId*

$\exists \text{PARTITION\_KERNEL\_STATE\_TYPE}$

$\text{procn?} : \text{PROCESS\_NAME\_TYPE}$

$\text{procid!} : \text{PROCESS\_ID\_TYPE}$

$(\exists_1 i : \text{PROCESS\_ID\_TYPE} \mid i \in \text{dom ProcessTable} \bullet \text{ProcessTable}(i).\text{Name} = \text{procn?} \wedge \text{procid!} = i)$

## 4.The information of Process Status

*GetProcessStatus*

$\exists \text{PARTITION\_KERNEL\_STATE\_TYPE}$

$\text{procid?} : \text{PROCESS\_ID\_TYPE}$

$\text{procs!} : \text{PROCESS\_STATUS\_TYPE}$

$(\exists \text{status} : \text{PROCESS\_STATUS\_TYPE} \bullet$

$\text{status.Attribute.Name} = \text{ProcessTable}(\text{procid?}).\text{Name}$

$\wedge \text{status.Attribute.EntryPoint} = \text{ProcessTable}(\text{procid?}).\text{EntryPoint}$

$\wedge \text{status.Attribute.StackSize} = \text{ProcessTable}(\text{procid?}).\text{VirtualMemory.Stack.Size}$

$\wedge \text{status.Attribute.BasePriority} = \text{ProcessTable}(\text{procid?}).\text{BasePriority}$

$\wedge \text{status.Attribute.Period} = \text{ProcessTable}(\text{procid?}).\text{Period}$

$\wedge \text{status.Attribute.TimeCapacity} = \text{ProcessTable}(\text{procid?}).\text{TimeCapacity}$

$\wedge \text{status.Attribute.Deadline} = \text{ProcessTable}(\text{procid?}).\text{Deadline}$

$\wedge \text{status.CurrentPriority} = \text{ProcessTable}(\text{procid?}).\text{CurrentPriority}$

$\wedge \text{status.DeadlineTime} = \text{ProcessTable}(\text{procid?}).\text{DeadlineTime}$

$\wedge \text{status.ProcessState} = \text{ProcessTable}(\text{procid?}).\text{ProcessState}$

$\wedge \text{procs!} = \text{status})$

## 5. The initialization of Register State of Process Context

*InitProcRegisterState*

*entrypoint?* : *SYSTEM\_ADDRESS\_TYPE*

*procv?* : *PROCESS\_VIRTUAL\_MEMORY\_TYPE*

*regstate!* : *CPU\_REGISTER\_TYPE*

$(\exists \text{reg} : \text{CPU\_REGISTER\_TYPE} \bullet$   
   $(\forall i : \mathbb{N} \mid i \in \text{dom}(\text{reg.GPRegisters}) \bullet \text{reg.GPRegisters}(i) = 0_{PSU})$   
   $\wedge \text{reg.SSRegisters.SS} = (\text{procv?}).\text{Stack.Start}$   
   $\wedge \text{reg.SSRegisters.BP} = 0_{PSU}$   
   $\wedge \text{reg.SSRegisters.SP} = 0_{PSU}$   
   $\wedge \text{reg.DSRegisters.DS} = (\text{procv?}).\text{Data.Start}$   
   $\wedge \text{reg.DSRegisters.SI} = 0_{PSU}$   
   $\wedge \text{reg.DSRegisters.DI} = 0_{PSU}$   
   $\wedge \text{reg.CSRegisters.CS} = (\text{procv?}).\text{Code.Start}$   
   $\wedge \text{reg.CSRegisters.IP} = \text{entrypoint?}$   
   $\wedge \text{reg.PSWRegisters.CF} = 0$   
   $\wedge \text{reg.PSWRegisters.PF} = 0$   
   $\wedge \text{reg.PSWRegisters.AF} = 0$   
   $\wedge \text{reg.PSWRegisters.ZF} = 0$   
   $\wedge \text{reg.PSWRegisters.SF} = 0$   
   $\wedge \text{reg.PSWRegisters.OF} = 0$   
   $\wedge \text{reg.PSWRegisters.TF} = 0$   
   $\wedge \text{reg.PSWRegisters.DF} = 0$   
   $\wedge \text{reg.PSWRegisters.IF} = 1$   
   $\wedge \text{regstate!} = \text{reg})$

## 6. The creating of Process Control Block



*CreateProcessControlBlock* \_\_\_\_\_

$proca? : PROCESS\_ATTRIBUTE\_TYPE$   
 $exefilepath? : PATH\_TYPE$   
 $swapfilepath? : PATH\_TYPE$   
 $kstack? : MEMORY\_BLOCK\_TYPE$   
 $procv? : PROCESS\_VIRTUAL\_MEMORY\_TYPE$   
 $proccb! : PROCESS\_CONTROL\_BLOCK\_TYPE$

$(\exists pcb : PROCESS\_CONTROL\_BLOCK\_TYPE \bullet$   
 $pcb.Name = (proca?).Name$   
 $\wedge pcb.ProcessKind = (proca?).ProcessKind$   
 $\wedge pcb.ExeFilePath = exefilepath?$   
 $\wedge pcb.SwapFilePath = swapfilepath?$   
 $\wedge pcb.EntryPoint = (proca?).EntryPoint$   
 $\wedge pcb.KernelStack = kstack?$   
 $\wedge pcb.VirtualMemory = procv?$   
 $\wedge pcb.Period = (proca?).Period$   
 $\wedge pcb.TimeCapacity = (proca?).TimeCapacity$   
 $\wedge pcb.Deadline = (proca?).Deadline$   
 $\wedge pcb.BasePriority = (proca?).BasePriority$   
 $\wedge pcb.CurrentPriority = DEFAULT\_PRIORITY$   
 $\wedge pcb.ReleasePoint = DEFAULT\_TIME$   
 $\wedge pcb.DeadlineTime = DEFAULT\_TIME$   
 $\wedge pcb.ProcessState = DORMANT$   
 $\wedge pcb.UserTempContext = \langle \rangle$   
 $\wedge pcb.KernelTempContext = \langle \rangle$   
 $\wedge proccb! = pcb)$

## 7.The enqueueing an element into Ready Queue(From Head)

*EnqReadyQueue<sub>1</sub>* \_\_\_\_\_

$\Delta PARTITION\_KERNEL\_STATE\_TYPE$   
 $procid? : PROCESS\_ID\_TYPE$

$ReadyQueue' = \langle procid? \rangle \wedge ReadyQueue$

## 8.The enqueueing an element into Ready Queue(From Tail)

*EnqReadyQueue<sub>2</sub>* \_\_\_\_\_

$\Delta PARTITION\_KERNEL\_STATE\_TYPE$   
 $procid? : PROCESS\_ID\_TYPE$

$ReadyQueue' = ReadyQueue \wedge \langle procid? \rangle$

## 9.The dequeuing an element from Ready Queue

*DeqReadyQueue* \_\_\_\_\_

$\Delta PARTITION\_KERNEL\_STATE\_TYPE$   
 $procid? : PROCESS\_ID\_TYPE$

$ReadyQueue' = squash(ReadyQueue \triangleright \{procid?\})$

## 10.The enqueueing an element into Waiting Queue

|                                                                                               |
|-----------------------------------------------------------------------------------------------|
| $EnqWaitingQueue$<br>$\Delta PARTITION\_KERNEL\_STATE\_TYPE$<br>$procid? : PROCESS\_ID\_TYPE$ |
| $WaitingQueue' = WaitingQueue \cap \langle procid? \rangle$                                   |

#### 11. The dequeuing an element from Waiting Queue

|                                                                                               |
|-----------------------------------------------------------------------------------------------|
| $DeqWaitingQueue$<br>$\Delta PARTITION\_KERNEL\_STATE\_TYPE$<br>$procid? : PROCESS\_ID\_TYPE$ |
| $WaitingQueue' = squash (WaitingQueue \triangleright \{procid?\})$                            |

#### 12. The creating of Time Counter

|                                                                                                                                       |
|---------------------------------------------------------------------------------------------------------------------------------------|
| $CreateTimeCounter$<br>$procid? : PROCESS\_ID\_TYPE$<br>$alarm? : SYSTEM\_TIME\_TYPE$<br>$tc! : TIME\_COUNTER\_TYPE$                  |
| $(\exists counter : TIME\_COUNTER\_TYPE \bullet$<br>$counter.ProcessId = procid? \wedge counter.Alarm = alarm? \wedge tc! = counter)$ |

#### 13. The information of Timing Process Alarm

|                                                                                                                                                                       |
|-----------------------------------------------------------------------------------------------------------------------------------------------------------------------|
| $GetTimingProcessAlarm$<br>$\exists PARTITION\_KERNEL\_STATE\_TYPE$<br>$procid? : PROCESS\_ID\_TYPE$<br>$alarm! : SYSTEM\_TIME\_TYPE$                                 |
| $(\exists_1 i : \mathbb{N}_1 \mid i \in \text{dom } TimeCounterQueue \bullet$<br>$TimeCounterQueue(i).ProcessId = procid? \wedge alarm! = TimeCounterQueue(i).Alarm)$ |

#### 14. The turning over of Time Counter

|                                                                                                                                                                                             |
|---------------------------------------------------------------------------------------------------------------------------------------------------------------------------------------------|
| $TurnOverTimeCounter$<br>$\Delta PARTITION\_KERNEL\_STATE\_TYPE$<br>$procid? : PROCESS\_ID\_TYPE$                                                                                           |
| $(\exists_1 i : \mathbb{N}_1 \mid i \in \text{dom } TimeCounterQueue \bullet$<br>$TimeCounterQueue(i).ProcessId = procid? \wedge TimeCounterQueue'(i).Alarm = - TimeCounterQueue(i).Alarm)$ |

#### 15. The information of processes in Time Counter Queue

|                                                                                                                |
|----------------------------------------------------------------------------------------------------------------|
| $GetTimingProcess$<br>$\exists PARTITION\_KERNEL\_STATE\_TYPE$<br>$tprocs! : \mathbb{P} PROCESS\_ID\_TYPE$     |
| $tprocs! = \{i : \mathbb{N}_1 \mid i \in \text{dom } TimeCounterQueue \bullet TimeCounterQueue(i).ProcessId\}$ |

## 16. The enqueueing an element into Time Counter Queue

|                                                                                                                                                                                                                                                                                                                                                                                                                                                                                                                                                                                                                                                                                                                                                                                                   |
|---------------------------------------------------------------------------------------------------------------------------------------------------------------------------------------------------------------------------------------------------------------------------------------------------------------------------------------------------------------------------------------------------------------------------------------------------------------------------------------------------------------------------------------------------------------------------------------------------------------------------------------------------------------------------------------------------------------------------------------------------------------------------------------------------|
| <i>EnqTimeCounterQueue</i>                                                                                                                                                                                                                                                                                                                                                                                                                                                                                                                                                                                                                                                                                                                                                                        |
| $\Delta PARTITION\_KERNEL\_STATE\_TYPE$                                                                                                                                                                                                                                                                                                                                                                                                                                                                                                                                                                                                                                                                                                                                                           |
| $tc? : TIME\_COUNTER\_TYPE$                                                                                                                                                                                                                                                                                                                                                                                                                                                                                                                                                                                                                                                                                                                                                                       |
| $ \begin{aligned} & ((\exists s, t : iseq[TIME\_COUNTER\_TYPE] \mid s \frown t = TimeCounterQueue \wedge s, t \neq \langle \rangle \bullet \\ & \quad \mid (last\ s).Alarm \mid \leq (tc?).Alarm \wedge \mid (head\ t).Alarm \mid > (tc?).Alarm \wedge TimeCounterQueue' = s \frown \langle tc? \rangle \frown t) \\ & \vee (\forall i : \mathbb{N}_1 \mid i \in \text{dom } TimeCounterQueue \bullet \\ & \quad \mid TimeCounterQueue(i).Alarm \mid \leq (tc?).Alarm \Rightarrow TimeCounterQueue' = TimeCounterQueue \frown \langle tc? \rangle) \\ & \vee (\forall i : \mathbb{N}_1 \mid i \in \text{dom } TimeCounterQueue \bullet \\ & \quad \mid TimeCounterQueue(i).Alarm \mid > (tc?).Alarm \Rightarrow TimeCounterQueue' = \langle tc? \rangle \frown TimeCounterQueue)) \end{aligned} $ |

## 17. The dequeuing an element from Time Counter Queue

|                                                                                                                                                                                                                                                |
|------------------------------------------------------------------------------------------------------------------------------------------------------------------------------------------------------------------------------------------------|
| <i>DeqTimeCounterQueue</i>                                                                                                                                                                                                                     |
| $\Delta PARTITION\_KERNEL\_STATE\_TYPE$                                                                                                                                                                                                        |
| $procid? : PROCESS\_ID\_TYPE$                                                                                                                                                                                                                  |
| $ \begin{aligned} & (\exists_1 tc : TIME\_COUNTER\_TYPE \mid tc \in \text{ran } TimeCounterQueue \wedge tc.ProcessId = procid? \bullet \\ & \quad TimeCounterQueue' = \text{squash } (TimeCounterQueue \triangleright \{tc\})) \end{aligned} $ |

## 18. The information of the Hishest Priority of processes in the Ready Queue

|                                                                                                                                                                                                                                                                                                                                                                                                       |
|-------------------------------------------------------------------------------------------------------------------------------------------------------------------------------------------------------------------------------------------------------------------------------------------------------------------------------------------------------------------------------------------------------|
| <i>GetHighestPriority</i>                                                                                                                                                                                                                                                                                                                                                                             |
| $\Xi PARTITION\_KERNEL\_STATE\_TYPE$                                                                                                                                                                                                                                                                                                                                                                  |
| $hp! : PRIORITY\_TYPE$                                                                                                                                                                                                                                                                                                                                                                                |
| $ \begin{aligned} & (\exists i : PROCESS\_ID\_TYPE \mid i \in \text{ran } ReadyQueue \bullet \\ & \quad (\forall j : PROCESS\_ID\_TYPE \mid j \in \text{ran } ReadyQueue \bullet \\ & \quad \quad j \neq i \Rightarrow \mid ProcessTable(j).CurrentPriority \mid \leq \mid ProcessTable(i).CurrentPriority \mid) \\ & \quad \wedge (hp! = \mid ProcessTable(i).CurrentPriority \mid)) \end{aligned} $ |

## 19. The update of Time Counter Queue

|                                                                                                                                                                                                                                                                                                                                                                                                                                                                                                                                                                                                                                                                                                                                                          |
|----------------------------------------------------------------------------------------------------------------------------------------------------------------------------------------------------------------------------------------------------------------------------------------------------------------------------------------------------------------------------------------------------------------------------------------------------------------------------------------------------------------------------------------------------------------------------------------------------------------------------------------------------------------------------------------------------------------------------------------------------------|
| <i>UpdateTimeCounterQueue</i>                                                                                                                                                                                                                                                                                                                                                                                                                                                                                                                                                                                                                                                                                                                            |
| $\Delta PARTITION\_KERNEL\_STATE\_TYPE$                                                                                                                                                                                                                                                                                                                                                                                                                                                                                                                                                                                                                                                                                                                  |
| $hpt? : SYSTEM\_TIME\_TYPE$                                                                                                                                                                                                                                                                                                                                                                                                                                                                                                                                                                                                                                                                                                                              |
| $procids! : iseq[PROCESS\_ID\_TYPE]$                                                                                                                                                                                                                                                                                                                                                                                                                                                                                                                                                                                                                                                                                                                     |
| $ \begin{aligned} & ((\forall i : \mathbb{N}_1 \mid i \in \text{dom } TimeCounterQueue \bullet \\ & \quad \mid TimeCounterQueue(i).Alarm \mid > hpt? \Rightarrow procids! = \emptyset \wedge TimeCounterQueue' = TimeCounterQueue) \\ & \vee (\exists k : \mathbb{N}_1 \bullet \\ & \quad k = \max(\{i : \mathbb{N}_1 \mid i \in \text{dom } TimeCounterQueue \wedge \mid TimeCounterQueue(i).Alarm \mid \leq hpt?\}) \\ & \quad \wedge procids! = \text{squash } ((1..k \triangleleft TimeCounterQueue) \triangleright \{i : \mathbb{N}_1 \mid i \in \text{dom } TimeCounterQueue \\ & \quad \quad \wedge TimeCounterQueue(i).Alarm > 0\}) \\ & \quad \wedge TimeCounterQueue' = \text{squash } (1..k \triangleleft TimeCounterQueue))) \end{aligned} $ |

## 20. The Checking of Release Points

*CheckReleasePionts*

$\Xi \text{PARTITION\_KERNEL\_STATE\_TYPE}$

$t? : \text{SYSTEM\_TIME\_TYPE}$

$\text{procids!} : \text{iseq}[\text{PROCESS\_ID\_TYPE}]$

$((\forall i : \text{PROCESS\_ID\_TYPE} \mid i \in \text{dom } \text{ProcessTable} \bullet$

$\text{ProcessTable}(i).\text{ReleasePoint} \neq t? \Rightarrow \text{procids!} = \langle \rangle)$

$\vee (\exists \text{seq} : \text{iseq}[\text{PROCESS\_ID\_TYPE}] \mid \text{ran seq} \subseteq \text{dom } \text{ProcessTable} \bullet$

$(\forall i : \text{PROCESS\_ID\_TYPE} \mid i \in \text{ran seq} \bullet \text{ProcessTable}(i).\text{ReleasePoint} = t?)$

$\wedge (\forall i : \text{PROCESS\_ID\_TYPE} \mid i \in (\text{dom } \text{ProcessTable} \setminus \text{ran seq}) \bullet \text{ProcessTable}(i).\text{ReleasePoint} \neq t?)$

$\wedge \text{procids!} = \text{seq}))$

## C Circus Channels

### C.1 Channels for signals which indicates the life stage of a ARINC 653 Module

*channel module\_init, module\_end*

### C.2 Channels for signals which indicates the life stage of the Real-Time Clock

*channel rtclock\_power\_on, rtclock\_power\_off*

### C.3 Channel for signals which indicates the Clock Pause

*channel clock\_pause*

### C.4 Channel for signals which indicates the Hardware Interrupts

*channel hardware\_interrupts : INTERRUPT\_TYPE*

### C.5 Channel for signals which indicates the Exceptions

*channel exception : EXCEPTION\_TYPE*

### C.6 Channels for communication within Interrupt Controller

*channel irregister\_report\_new\_interrupt : INTERRUPT\_TYPE*

*channel isregister\_demand\_new\_interrupt*

*channel isregister\_service\_new\_interrupt : INTERRUPT\_TYPE*

*channel priority\_resolver\_report\_new\_interrupt : INTERRUPT\_TYPE*

### C.7 Channels for communication between different parts of Core Hardware Layer

*channel interrupt : INTERRUPT\_TYPE*

*channel interrupt\_acknowledged*

*channel interrupt\_handled : INTERRUPT\_TYPE*

*channel cpu\_request\_logical\_address\_translation : PAGE\_TYPE  $\times$  PSU  $\times$  SYSTEM\_ADDRESS\_TYPE*

*channel logical\_address\_translation\_fail*

*channel cpu\_get\_logical\_address\_translation : SYSTEM\_ADDRESS\_TYPE*

*channel cpu\_receive\_data\_from\_main\_memory : SYSTEM\_ADDRESS\_TYPE*

*channel cpu\_received\_data\_from\_main\_memory : PSU*

*channel cpu\_send\_data\_to\_main\_memory : SYSTEM\_ADDRESS\_TYPE  $\times$  PSU*

*channel cpu\_sent\_data\_to\_main\_memory*

## C.8 Channels for communication between Core Hardware Layer and Hardware Interface Software Layer

`channel context_switching_save_part_cpu_registers`  
`channel context_switching_saved_part_cpu_registers : CPU_REGISTER_TYPE`  
`channel context_switching_save_all_cpu_registers`  
`channel context_switching_saved_all_cpu_registers : CPU_REGISTER_TYPE`  
`channel context_switching_restore_part_cpu_registers : CPU_REGISTER_TYPE`  
`channel context_switching_restored_part_cpu_registers`  
`channel context_switching_restore_all_cpu_registers : CPU_REGISTER_TYPE`  
`channel context_switching_restored_all_cpu_registers`  
`channel context_switching_set_stack_segment_registers : SSREGISTER_TYPE`  
`channel context_switching_have_set_stack_segment_registers`  
`channel interrupt_controlling_enable_interrupt`  
`channel interrupt_controlling_enabled_interrupt`  
`channel interrupt_controlling_disable_interrupt`  
`channel interrupt_controlling_disabled_interrupt`  
`channel interrupt_handler_start_interrupt_handling : INTERRUPT_TYPE`  
`channel interrupt_handler_finish_interrupt_handling : INTERRUPT_TYPE`  
`channel exception_handler_start_exception_handling : EXCEPTION_TYPE`  
`channel exception_handler_finish_exception_handling`  
`channel context_switching_set_page_table : PAGE_TABLE_TYPE`  
`channel context_switching_have_set_page_table`  
`channel context_switching_request_page_table`  
`channel context_switching_get_page_table : PAGE_TABLE_TYPE`  
`channel memory_management_load_page_into_main_memory : PAGE_TYPE  $\times$  PIECE_TYPE`  
`channel memory_management_loaded_page_into_main_memory`  
`channel memory_management_extract_page_from_main_memory : PAGE_TYPE`  
`channel memory_management_extracted_page_from_main_memory : PIECE_TYPE`  
`channel system_clock_request_current_time`  
`channel system_clock_get_current_time : PSU`  
`channel system_clock_request_high_precision_time`  
`channel system_clock_get_high_precision_time : PSU`  
`channel system_clock_set_high_precision_timer_alarm : PSU`  
`channel system_clock_have_set_high_precision_timer_alarm`  
`channel system_clock_reset_high_precision_timer`  
`channel system_clock_have_reset_high_precision_timer`  
`channel system_clock_end_high_precision_timer`  
`channel system_clock_ended_high_precision_timer`  
`channel interrupt_controlling_mask_interrupt : INTERRUPT_TYPE`  
`channel interrupt_controlling_masked_interrupt`  
`channel interrupt_controlling_unmask_interrupt : INTERRUPT_TYPE`  
`channel interrupt_controlling_unmasked_interrupt`

## C.9 Channels for communication within Interrupt Handler

`channel interrupt_handler_invoke_service_routine_clocktick`  
`channel interrupt_service_routine_end : INTERRUPT_TYPE`

## C.10 Channels for communication between different parts of Hardware Interface Software Layer

**channel** *interrupt\_handler\_save\_context*  
**channel** *interrupt\_handler\_saved\_context* : *CPU\_REGISTER\_TYPE*  $\times$  *PAGE\_TABLE\_TYPE*  
**channel** *interrupt\_handler\_restore\_context* : *CPU\_REGISTER\_TYPE*  $\times$  *PAGE\_TABLE\_TYPE*  
**channel** *interrupt\_handler\_restored\_context*  
**channel** *interrupt\_handler\_switch\_stack* : *SSREGISTER\_TYPE*  $\times$  *PAGE\_TABLE\_TYPE*  
**channel** *interrupt\_handler\_switched\_stack*  
**channel** *isr\_clocktick\_update\_system\_time*  
**channel** *isr\_clocktick\_updated\_system\_time*  
**channel** *isr\_clocktick\_request\_high\_precision\_time*  
**channel** *isr\_clocktick\_get\_high\_precision\_time* : *SYSTEM\_TIME\_TYPE*  
**channel** *interrupt\_handler\_mask\_interrupt* : *INTERRUPT\_TYPE*  
**channel** *interrupt\_handler\_masked\_interrupt*  
**channel** *interrupt\_handler\_unmask\_interrupt* : *INTERRUPT\_TYPE*  
**channel** *interrupt\_handler\_unmasked\_interrupt*  
**channel** *interrupt\_handler\_enable\_interrupt*  
**channel** *interrupt\_handler\_enabled\_interrupt* **channel** *interrupt\_handler\_disable\_interrupt*  
**channel** *interrupt\_handler\_disabled\_interrupt*

## C.11 Channels for communication between Hardware Interface Software Layer and ARINC 653 O/S Layer

**channel** *kernel\_save\_context* : *KERNEL\_ID\_TYPE*  $\times$  *OPTION\_TYPE*  
**channel** *kernel\_saved\_context* : *KERNEL\_ID\_TYPE*  $\times$  *CPU\_REGISTER\_TYPE*  $\times$  *PAGE\_TABLE\_TYPE*  
**channel** *kernel\_restore\_context* : *KERNEL\_ID\_TYPE*  $\times$  *OPTION\_TYPE*  $\times$  *CPU\_REGISTER\_TYPE*  $\times$  *PAGE\_TABLE\_TYPE*  
**channel** *kernel\_restored\_context* : *KERNEL\_ID\_TYPE*  
**channel** *kernel\_switch\_stack* : *KERNEL\_ID\_TYPE*  $\times$  *SSREGISTER\_TYPE*  $\times$  *PAGE\_TABLE\_TYPE*  
**channel** *kernel\_switched\_stack* : *KERNEL\_ID\_TYPE*  
**channel** *kernel\_init\_memory\_management* : *AREA\_MEMORY\_MANAGEMENT\_TYPE*  
**channel** *kernel\_inited\_memory\_management*  
**channel** *kernel\_set\_area\_memory\_management\_reference* : *KERNEL\_ID\_TYPE*  $\times$  *AREA\_MEMORY\_MANAGEMENT\_TYPE*  
**channel** *kernel\_have\_set\_area\_memory\_management\_reference* : *KERNEL\_ID\_TYPE*  
**channel** *kernel\_request\_area\_memory\_management\_reference* : *KERNEL\_ID\_TYPE*  
**channel** *kernel\_get\_area\_memory\_management\_reference* : *KERNEL\_ID\_TYPE*  $\times$  *AREA\_MEMORY\_MANAGEMENT\_TYPE*  
**channel** *kernel\_request\_area\_free\_pages* : *KERNEL\_ID\_TYPE*  
**channel** *kernel\_get\_area\_free\_pages* : *KERNEL\_ID\_TYPE*  $\times$  *UNSIGNED\_INTEGER\_TYPE*  
**channel** *kernel\_request\_area\_free\_block* : *KERNEL\_ID\_TYPE*  
**channel** *kernel\_get\_area\_free\_block* : *KERNEL\_ID\_TYPE*  $\times$  *UNSIGNED\_INTEGER\_TYPE*  
**channel** *kernel\_allocate\_area\_free\_pages* : *KERNEL\_ID\_TYPE*  $\times$  *UNSIGNED\_INTEGER\_TYPE*  
**channel** *kernel\_allocated\_area\_free\_pages* : *KERNEL\_ID\_TYPE*  $\times$   $\mathbb{P}$  *PAGE\_TYPE*  
**channel** *kernel\_allocate\_area\_free\_block* : *KERNEL\_ID\_TYPE*  $\times$  *UNSIGNED\_INTEGER\_TYPE*  
**channel** *kernel\_allocated\_area\_free\_block* : *KERNEL\_ID\_TYPE*  $\times$  *MEMORY\_BLOCK\_TYPE*  
**channel** *kernel\_deallocate\_area\_used\_pages* : *KERNEL\_ID\_TYPE*  $\times$   $\mathbb{P}$  *PAGE\_TYPE*  
**channel** *kernel\_deallocated\_area\_used\_pages* : *KERNEL\_ID\_TYPE*  
**channel** *kernel\_deallocate\_area\_used\_block* : *KERNEL\_ID\_TYPE*  $\times$  *MEMORY\_BLOCK\_TYPE*  
**channel** *kernel\_deallocated\_area\_used\_block* : *KERNEL\_ID\_TYPE*

**channel** *kernel\_create\_virtual\_memory\_block* : *KERNEL\_ID\_TYPE*  $\times$  *PAGE\_TYPE*  $\times$  *UNSIGNED\_INTEGER\_TYPE*  
**channel** *kernel\_created\_virtual\_memory\_block* : *KERNEL\_ID\_TYPE*  $\times$  *MEMORY\_BLOCK\_TYPE*  
**channel** *kernel\_create\_process\_virtual\_memory* : *KERNEL\_ID\_TYPE*  $\times$   $\mathbb{P}$  *PAGE\_TYPE*  $\times$  *UNSIGNED\_INTEGER\_TYPE*  $\times$  *UNSIGNED\_INTEGER\_TYPE*  $\times$  *UNSIGNED\_INTEGER\_TYPE*  
**channel** *kernel\_created\_process\_virtual\_memory* : *KERNEL\_ID\_TYPE*  $\times$  *PROCESS\_VIRTUAL\_MEMORY\_TYPE*  
**channel** *kernel\_full\_load\_process\_pages* : *KERNEL\_ID\_TYPE*  $\times$  *SYSTEM\_ADDRESS\_TYPE*  $\times$  *EXECUTABLE\_FILE\_TYPE*  
**channel** *kernel\_full\_loaded\_process\_pages* : *KERNEL\_ID\_TYPE*  $\times$  *PAGE\_TABLE\_TYPE*  
**channel** *kernel\_init\_system\_clock*  
**channel** *kernel\_inited\_system\_clock*  
**channel** *kernel\_request\_system\_time* : *KERNEL\_ID\_TYPE*  
**channel** *kernel\_get\_system\_time* : *KERNEL\_ID\_TYPE*  $\times$  *SYSTEM\_TIME\_TYPE*  
**channel** *kernel\_request\_high\_precision\_time* : *KERNEL\_ID\_TYPE*  
**channel** *kernel\_get\_high\_precision\_time* : *KERNEL\_ID\_TYPE*  $\times$  *SYSTEM\_TIME\_TYPE*  
**channel** *kernel\_reset\_high\_precision\_timer* : *KERNEL\_ID\_TYPE*  
**channel** *kernel\_have\_reset\_high\_precision\_timer* : *KERNEL\_ID\_TYPE*  
**channel** *kernel\_set\_high\_precision\_timer\_alarm* : *KERNEL\_ID\_TYPE*  $\times$  *SYSTEM\_TIME\_TYPE*  
**channel** *kernel\_have\_set\_high\_precision\_timer\_alarm* : *KERNEL\_ID\_TYPE*  
**channel** *kernel\_end\_high\_precision\_timer* : *KERNEL\_ID\_TYPE*  
**channel** *kernel\_ended\_high\_precision\_timer* : *KERNEL\_ID\_TYPE*  
**channel** *kernel\_request\_interrupt\_time* : *KERNEL\_ID\_TYPE*  
**channel** *kernel\_get\_interrupt\_time* : *KERNEL\_ID\_TYPE*  $\times$  *SYSTEM\_TIME\_TYPE*  
**channel** *kernel\_mask\_interrupt* : *KERNEL\_ID\_TYPE*  $\times$  *INTERRUPT\_TYPE*  
**channel** *kernel\_masked\_interrupt* : *KERNEL\_ID\_TYPE*  
**channel** *kernel\_unmask\_interrupt* : *KERNEL\_ID\_TYPE*  $\times$  *INTERRUPT\_TYPE*  
**channel** *kernel\_unmasked\_interrupt* : *KERNEL\_ID\_TYPE*  
**channel** *kernel\_enable\_interrupt* : *KERNEL\_ID\_TYPE*  
**channel** *kernel\_enabled\_interrupt* : *KERNEL\_ID\_TYPE*  
**channel** *kernel\_disable\_interrupt* : *KERNEL\_ID\_TYPE*  
**channel** *kernel\_disabled\_interrupt* : *KERNEL\_ID\_TYPE*  
**channel** *kernel\_init\_interrupt\_handler* : *PAGE\_TABLE\_TYPE*  
**channel** *interrupt\_handler\_request\_interrupt\_stack* : *UNSIGNED\_INTEGER\_TYPE*  
**channel** *interrupt\_handler\_get\_interrupt\_stack* : *MEMORY\_BLOCK\_TYPE*  
**channel** *kernel\_inited\_interrupt\_handler*  
**channel** *interrupt\_handler\_invoke\_kernel*  
**channel** *kernel\_continue\_interrupted\_process* : *KERNEL\_ID\_TYPE*  
**channel** *kernel\_request\_interrupted\_process\_context* : *KERNEL\_ID\_TYPE*  
**channel** *kernel\_get\_interrupted\_process\_context* : *KERNEL\_ID\_TYPE*  $\times$  *CPU\_REGISTER\_TYPE*  $\times$  *PAGE\_TABLE\_TYPE*

## C.12 Channels for communication of Error Handler between its User Mode and Kernel Mode

**channel** *error\_process\_id* : *PROCESS\_ID\_TYPE*





### C.13 Channels for communication within each Partition Kernel

**channel** *system\_call\_handler\_invoke\_service\_routine\_get\_operating\_mode* : *PARTITION\_ID\_TYPE*  $\times$  *PROCESS\_ID\_TYPE*

**channel** *system\_call\_handler\_invoke\_service\_routine\_get\_partition\_status* : *PARTITION\_ID\_TYPE*  $\times$  *PROCESS\_ID\_TYPE*

**channel** *system\_call\_handler\_invoke\_service\_routine\_set\_operating\_mode* : *PARTITION\_ID\_TYPE*  $\times$  *PROCESS\_ID\_TYPE*

**channel** *system\_call\_handler\_invoke\_service\_routine\_get\_process\_names* : *PARTITION\_ID\_TYPE*  $\times$  *PROCESS\_ID\_TYPE*

**channel** *system\_call\_handler\_invoke\_service\_routine\_get\_process\_ids* : *PARTITION\_ID\_TYPE*  $\times$  *PROCESS\_ID\_TYPE*

**channel** *system\_call\_handler\_invoke\_service\_routine\_get\_free\_process\_ids* : *PARTITION\_ID\_TYPE*  $\times$  *PROCESS\_ID\_TYPE*

**channel** *system\_call\_handler\_invoke\_service\_routine\_get\_free\_space* : *PARTITION\_ID\_TYPE*  $\times$  *PROCESS\_ID\_TYPE*

**channel** *system\_call\_handler\_invoke\_service\_routine\_get\_partition\_period* : *PARTITION\_ID\_TYPE*  $\times$  *PROCESS\_ID\_TYPE*

**channel** *system\_call\_handler\_invoke\_service\_routine\_get\_process\_state* : *PARTITION\_ID\_TYPE*  $\times$  *PROCESS\_ID\_TYPE*

**channel** *system\_call\_handler\_invoke\_service\_routine\_get\_next\_periodic\_start* : *PARTITION\_ID\_TYPE*  $\times$  *PROCESS\_ID\_TYPE*

**channel** *system\_call\_handler\_invoke\_service\_routine\_get\_delayed\_periodic\_start* : *PARTITION\_ID\_TYPE*  $\times$  *PROCESS\_ID\_TYPE*

**channel** *system\_call\_handler\_invoke\_service\_routine\_get\_process\_kind* : *PARTITION\_ID\_TYPE*  $\times$  *PROCESS\_ID\_TYPE*

**channel** *system\_call\_handler\_invoke\_service\_routine\_get\_process\_period* : *PARTITION\_ID\_TYPE*  $\times$  *PROCESS\_ID\_TYPE*

**channel** *system\_call\_handler\_invoke\_service\_routine\_get\_process\_time\_capacity* : *PARTITION\_ID\_TYPE*  $\times$  *PROCESS\_ID\_TYPE*

**channel** *system\_call\_handler\_invoke\_service\_routine\_get\_partition\_lock\_level* : *PARTITION\_ID\_TYPE*  $\times$  *PROCESS\_ID\_TYPE*

**channel** *system\_call\_handler\_invoke\_service\_routine\_get\_process\_id* : *PARTITION\_ID\_TYPE*  $\times$  *PROCESS\_ID\_TYPE*

**channel** *system\_call\_handler\_invoke\_service\_routine\_get\_process\_status* : *PARTITION\_ID\_TYPE*  $\times$  *PROCESS\_ID\_TYPE*

**channel** *system\_call\_handler\_invoke\_service\_routine\_create\_process* : *PARTITION\_ID\_TYPE*  $\times$  *PROCESS\_ID\_TYPE*

**channel** *system\_call\_handler\_invoke\_service\_routine\_set\_priority* : *PARTITION\_ID\_TYPE*  $\times$  *PROCESS\_ID\_TYPE*

**channel** *system\_call\_handler\_invoke\_service\_routine\_suspend\_self* : *PARTITION\_ID\_TYPE*  $\times$  *PROCESS\_ID\_TYPE*

**channel** *system\_call\_handler\_invoke\_service\_routine\_suspend* : *PARTITION\_ID\_TYPE*  $\times$  *PROCESS\_ID\_TYPE*

**channel** *system\_call\_handler\_invoke\_service\_routine\_resume* : *PARTITION\_ID\_TYPE*  $\times$  *PROCESS\_ID\_TYPE*

**channel** *system\_call\_handler\_invoke\_service\_routine\_stop\_self* : *PARTITION\_ID\_TYPE*  $\times$  *PROCESS\_ID\_TYPE*

**channel** *system\_call\_handler\_invoke\_service\_routine\_stop* : *PARTITION\_ID\_TYPE*  $\times$  *PROCESS\_ID\_TYPE*

**channel** *system\_call\_handler\_invoke\_service\_routine\_start* : *PARTITION\_ID\_TYPE*  $\times$  *PROCESS\_ID\_TYPE*

**channel** *system\_call\_handler\_invoke\_service\_routine\_delayed\_start* : *PARTITION\_ID\_TYPE*  $\times$  *PROCESS\_ID\_TYPE*

**channel** *system\_call\_handler\_invoke\_service\_routine\_lock\_preemption* : *PARTITION\_ID\_TYPE*  $\times$  *PROCESS\_ID\_TYPE*

**channel** *system\_call\_handler\_invoke\_service\_routine\_unlock\_preemption* : *PARTITION\_ID\_TYPE*  $\times$  *PROCESS\_ID\_TYPE*

**channel** *system\_call\_handler\_invoke\_service\_routine\_get\_my\_id* : *PARTITION\_ID\_TYPE*  $\times$  *PROCESS\_ID\_TYPE*

**channel** *system\_call\_handler\_invoke\_service\_routine\_get\_current\_time* : *PARTITION\_ID\_TYPE* × *PROCESS\_ID\_TYPE*  
**channel** *system\_call\_handler\_invoke\_service\_routine\_get\_partition\_time* : *PARTITION\_ID\_TYPE* × *PROCESS\_ID\_TYPE*  
**channel** *system\_call\_handler\_invoke\_service\_routine\_get\_next\_release\_point* : *PARTITION\_ID\_TYPE* × *PROCESS\_ID\_TYPE*  
**channel** *system\_call\_handler\_invoke\_service\_routine\_timed\_wait* : *PARTITION\_ID\_TYPE* × *PROCESS\_ID\_TYPE*  
**channel** *system\_call\_handler\_invoke\_service\_routine\_periodic\_wait* : *PARTITION\_ID\_TYPE* × *PROCESS\_ID\_TYPE*  
**channel** *system\_call\_handler\_invoke\_service\_routine\_get\_time* : *PARTITION\_ID\_TYPE* × *PROCESS\_ID\_TYPE*  
**channel** *system\_call\_handler\_invoke\_service\_routine\_replenish* : *PARTITION\_ID\_TYPE* × *PROCESS\_ID\_TYPE*  
**channel** *suspended\_process\_get\_resumed* : *PARTITION\_ID\_TYPE* × *PROCESS\_ID\_TYPE*  
**channel** *time\_out\_expired* : *PARTITION\_ID\_TYPE* × *PROCESS\_ID\_TYPE*  
**channel** *system\_call\_service\_routine\_end* : *PARTITION\_ID\_TYPE* × *PROCESS\_ID\_TYPE*  
**channel** *partition\_kernel\_start\_service* : *PARTITION\_ID\_TYPE* × *OPTION\_TYPE*  
**channel** *partition\_kernel\_end\_service* : *PARTITION\_ID\_TYPE*  
**channel** *partition\_kernel\_start\_process\_scheduler* : *PARTITION\_ID\_TYPE*  
**channel** *partition\_kernel\_end\_process\_scheduler* : *PARTITION\_ID\_TYPE*  
**channel** *partition\_kernel\_enable\_error\_handler* : *PARTITION\_ID\_TYPE*  
**channel** *partition\_kernel\_enabled\_error\_handler* : *PARTITION\_ID\_TYPE*  
**channel** *partition\_kernel\_invoke\_health\_monitor* : *PARTITION\_ID\_TYPE* × *PROCESS\_ID\_TYPE*  
**channel** *general\_process\_scheduling* : *PARTITION\_ID\_TYPE*  
**channel** *specific\_process\_scheduling* : *PARTITION\_ID\_TYPE* × *PROCESS\_ID\_TYPE*

## C.14 Channels for communication between different parts of ARINC 653 O/S Layer

**channel** *core\_kernel\_init\_partition\_kernel* : *PARTITION\_ID\_TYPE* × *PAGE\_TABLE\_TYPE*  
**channel** *core\_kernel\_initied\_partition\_kernel* : *PARTITION\_ID\_TYPE*  
**channel** *core\_kernel\_service\_get\_operating\_mode* : *PARTITION\_ID\_TYPE*  
**channel** *core\_kernel\_service\_get\_operating\_mode\_output* : *PARTITION\_ID\_TYPE* × *OPERATING\_MODE\_TYPE*  
**channel** *core\_kernel\_service\_get\_operating\_mode\_return* : *PARTITION\_ID\_TYPE*  
**channel** *core\_kernel\_service\_get\_partition\_status* : *PARTITION\_ID\_TYPE*  
**channel** *core\_kernel\_service\_get\_partition\_status\_output* : *PARTITION\_ID\_TYPE* × *PARTITION\_STATUS\_TYPE*  
**channel** *core\_kernel\_service\_get\_partition\_status\_return* : *PARTITION\_ID\_TYPE*  
**channel** *core\_kernel\_service\_set\_operating\_mode* : *PARTITION\_ID\_TYPE*  
**channel** *core\_kernel\_service\_set\_operating\_mode\_input* : *PARTITION\_ID\_TYPE* × *OPERATING\_MODE\_TYPE*  
**channel** *core\_kernel\_service\_set\_operating\_mode\_return* : *PARTITION\_ID\_TYPE*  
**channel** *core\_kernel\_service\_get\_next\_periodic\_start* : *PARTITION\_ID\_TYPE*  
**channel** *core\_kernel\_service\_get\_next\_periodic\_start\_output* : *PARTITION\_ID\_TYPE* × *SYSTEM\_TIME\_TYPE*  
**channel** *core\_kernel\_service\_get\_next\_periodic\_start\_return* : *PARTITION\_ID\_TYPE*  
**channel** *core\_kernel\_service\_get\_delayed\_periodic\_start* : *PARTITION\_ID\_TYPE*  
**channel** *core\_kernel\_service\_get\_delayed\_periodic\_start\_input* : *PARTITION\_ID\_TYPE* × *SYSTEM\_TIME\_TYPE*  
**channel** *core\_kernel\_service\_get\_delayed\_periodic\_start\_output* : *PARTITION\_ID\_TYPE* × *SYSTEM\_TIME\_TYPE*  
**channel** *core\_kernel\_service\_get\_delayed\_periodic\_start\_return* : *PARTITION\_ID\_TYPE*  
**channel** *core\_kernel\_service\_get\_lock\_level* : *PARTITION\_ID\_TYPE*  
**channel** *core\_kernel\_service\_get\_lock\_level\_output* : *PARTITION\_ID\_TYPE* × *LOCK\_LEVEL\_TYPE*  
**channel** *core\_kernel\_service\_get\_lock\_level\_return* : *PARTITION\_ID\_TYPE*  
**channel** *core\_kernel\_service\_reset\_lock\_level* : *PARTITION\_ID\_TYPE*  
**channel** *core\_kernel\_service\_reset\_lock\_level\_return* : *PARTITION\_ID\_TYPE*  
**channel** *core\_kernel\_service\_increase\_lock\_level* : *PARTITION\_ID\_TYPE*  
**channel** *core\_kernel\_service\_increase\_lock\_level\_return* : *PARTITION\_ID\_TYPE*

**channel** *core\_kernel\_service\_decrease\_lock\_level* : *PARTITION\_ID\_TYPE*  
**channel** *core\_kernel\_service\_decrease\_lock\_level\_return* : *PARTITION\_ID\_TYPE*  
**channel** *partition\_kernel\_continue\_execution* : *PARTITION\_ID\_TYPE*  
**channel** *partition\_kernel\_suspend\_execution* : *PARTITION\_ID\_TYPE*  
**channel** *partition\_kernel\_suspended\_execution* : *PARTITION\_ID\_TYPE*  
**channel** *partition\_kernel\_idle\_execution* : *PARTITION\_ID\_TYPE*  
**channel** *partition\_kernel\_prepare\_execution* : *PARTITION\_ID\_TYPE*  
**channel** *partition\_kernel\_update\_system\_time* : *PARTITION\_ID\_TYPE*  $\times$  *SYSTEM\_TIME\_TYPE*  
**channel** *partition\_kernel\_start\_execution* : *PARTITION\_ID\_TYPE*

## C.15 Channels for communication between ARINC 653 O/S Layer and APEX Layer

**channel** *system\_call* : *PARTITION\_ID\_TYPE*  $\times$  *PROCESS\_ID\_TYPE*  $\times$  *SYSTEM\_CALL\_TYPE*  
**channel** *system\_call\_service\_routine\_get\_operating\_mode\_output* : *PARTITION\_ID\_TYPE*  $\times$  *PROCESS\_ID\_TYPE*  $\times$  *OPERATING\_MODE\_TYPE*  
**channel** *system\_call\_service\_routine\_get\_partition\_status\_output* : *PARTITION\_ID\_TYPE*  $\times$  *PROCESS\_ID\_TYPE*  $\times$  *PARTITION\_STATUS\_TYPE*  
**channel** *system\_call\_service\_routine\_set\_operating\_mode\_input* : *PARTITION\_ID\_TYPE*  $\times$  *PROCESS\_ID\_TYPE*  $\times$  *OPERATING\_MODE\_TYPE*  
**channel** *system\_call\_service\_routine\_get\_process\_names\_output* : *PARTITION\_ID\_TYPE*  $\times$  *PROCESS\_ID\_TYPE*  $\times$   $\mathbb{P}$  *PROCESS\_NAME\_TYPE*  
**channel** *system\_call\_service\_routine\_get\_process\_ids\_output* : *PARTITION\_ID\_TYPE*  $\times$  *PROCESS\_ID\_TYPE*  $\times$   $\mathbb{P}$  *PROCESS\_ID\_TYPE*  
**channel** *system\_call\_service\_routine\_get\_free\_process\_ids\_output* : *PARTITION\_ID\_TYPE*  $\times$  *PROCESS\_ID\_TYPE*  $\times$   $\mathbb{P}$  *PROCESS\_ID\_TYPE*  
**channel** *system\_call\_service\_routine\_get\_free\_space\_output* : *PARTITION\_ID\_TYPE*  $\times$  *PROCESS\_ID\_TYPE*  $\times$  *UNSIGNED\_INTEGER\_TYPE*  $\times$  *UNSIGNED\_INTEGER\_TYPE*  
**channel** *system\_call\_service\_routine\_get\_partition\_period\_output* : *PARTITION\_ID\_TYPE*  $\times$  *PROCESS\_ID\_TYPE*  $\times$  *SYSTEM\_TIME\_TYPE*  
**channel** *system\_call\_service\_routine\_get\_process\_state\_input* : *PARTITION\_ID\_TYPE*  $\times$  *PROCESS\_ID\_TYPE*  $\times$  *PROCESS\_ID\_TYPE*  
**channel** *system\_call\_service\_routine\_get\_process\_state\_output* : *PARTITION\_ID\_TYPE*  $\times$  *PROCESS\_ID\_TYPE*  $\times$  *PROCESS\_ID\_TYPE*  $\times$  *PROCESS\_STATE\_TYPE*  
**channel** *system\_call\_service\_routine\_get\_next\_periodic\_start\_output* : *PARTITION\_ID\_TYPE*  $\times$  *PROCESS\_ID\_TYPE*  $\times$  *SYSTEM\_TIME\_TYPE*  
**channel** *system\_call\_service\_routine\_get\_delayed\_periodic\_start\_input* : *PARTITION\_ID\_TYPE*  $\times$  *PROCESS\_ID\_TYPE*  $\times$  *SYSTEM\_TIME\_TYPE*  
**channel** *system\_call\_service\_routine\_get\_delayed\_periodic\_start\_output* : *PARTITION\_ID\_TYPE*  $\times$  *PROCESS\_ID\_TYPE*  $\times$  *SYSTEM\_TIME\_TYPE*  
**channel** *system\_call\_service\_routine\_get\_process\_kind\_input* : *PARTITION\_ID\_TYPE*  $\times$  *PROCESS\_ID\_TYPE*  $\times$  *PROCESS\_ID\_TYPE*  
**channel** *system\_call\_service\_routine\_get\_process\_kind\_output* : *PARTITION\_ID\_TYPE*  $\times$  *PROCESS\_ID\_TYPE*  $\times$  *PROCESS\_ID\_TYPE*  $\times$  *PROCESS\_KIND\_TYPE*  
**channel** *system\_call\_service\_routine\_get\_process\_period\_input* : *PARTITION\_ID\_TYPE*  $\times$  *PROCESS\_ID\_TYPE*  $\times$  *PROCESS\_ID\_TYPE*  
**channel** *system\_call\_service\_routine\_get\_process\_period\_output* : *PARTITION\_ID\_TYPE*  $\times$  *PROCESS\_ID\_TYPE*  $\times$  *PROCESS\_ID\_TYPE*  $\times$  *SYSTEM\_TIME\_TYPE*  
**channel** *system\_call\_service\_routine\_get\_process\_time\_capacity\_input* : *PARTITION\_ID\_TYPE*  $\times$  *PROCESS\_ID\_TYPE*  $\times$  *PROCESS\_ID\_TYPE*  $\times$  *PROCESS\_ID\_TYPE*  
**channel** *system\_call\_service\_routine\_get\_process\_time\_capacity\_output* : *PARTITION\_ID\_TYPE*  $\times$  *PROCESS\_ID\_TYPE*  $\times$  *PROCESS\_ID\_TYPE*  $\times$  *SYSTEM\_TIME\_TYPE*

**channel** *system\_call\_service\_routine\_get\_partition\_lock\_level\_output* : *PARTITION\_ID\_TYPE* × *PROCESS\_ID\_TYPE* × *LOCK\_LEVEL\_TYPE*  
**channel** *system\_call\_service\_routine\_get\_process\_id\_input* : *PARTITION\_ID\_TYPE* × *PROCESS\_ID\_TYPE* × *PROCESS\_NAME\_TYPE*  
**channel** *system\_call\_service\_routine\_get\_process\_id\_output* : *PARTITION\_ID\_TYPE* × *PROCESS\_ID\_TYPE* × *PROCESS\_ID\_TYPE*  
**channel** *system\_call\_service\_routine\_get\_process\_status\_input* : *PARTITION\_ID\_TYPE* × *PROCESS\_ID\_TYPE* × *PROCESS\_ID\_TYPE*  
**channel** *system\_call\_service\_routine\_get\_process\_status\_output* : *PARTITION\_ID\_TYPE* × *PROCESS\_ID\_TYPE* × *PROCESS\_STATUS\_TYPE*  
**channel** *system\_call\_service\_routine\_create\_process\_input* : *PARTITION\_ID\_TYPE* × *PROCESS\_ID\_TYPE* × *PROCESS\_ATTRIBUTE\_TYPE* × *EXECUTABLE\_FILE\_TYPE* × *PATH\_TYPE* × *PATH\_TYPE*  
**channel** *system\_call\_service\_routine\_create\_process\_output* : *PARTITION\_ID\_TYPE* × *PROCESS\_ID\_TYPE* × *PROCESS\_ID\_TYPE*  
**channel** *system\_call\_service\_routine\_set\_priority\_input* : *PARTITION\_ID\_TYPE* × *PROCESS\_ID\_TYPE* × *PROCESS\_ID\_TYPE* × *PRIORITY\_TYPE*  
**channel** *system\_call\_service\_routine\_suspend\_self\_input* : *PARTITION\_ID\_TYPE* × *PROCESS\_ID\_TYPE* × *SYSTEM\_TIME\_TYPE* × *SYSTEM\_TIME\_TYPE*  
**channel** *system\_call\_service\_routine\_suspend\_self\_output* : *PARTITION\_ID\_TYPE* × *PROCESS\_ID\_TYPE* × *BOOLEAN*  
**channel** *system\_call\_service\_routine\_suspend\_input* : *PARTITION\_ID\_TYPE* × *PROCESS\_ID\_TYPE* × *PROCESS\_ID\_TYPE*  
**channel** *system\_call\_service\_routine\_suspend\_output* : *PARTITION\_ID\_TYPE* × *PROCESS\_ID\_TYPE* × *BOOLEAN*  
**channel** *system\_call\_service\_routine\_resume\_input* : *PARTITION\_ID\_TYPE* × *PROCESS\_ID\_TYPE* × *PROCESS\_ID\_TYPE*  
**channel** *system\_call\_service\_routine\_stop\_input* : *PARTITION\_ID\_TYPE* × *PROCESS\_ID\_TYPE* × *PROCESS\_ID\_TYPE*  
**channel** *system\_call\_service\_routine\_start\_input* : *PARTITION\_ID\_TYPE* × *PROCESS\_ID\_TYPE* × *PROCESS\_ID\_TYPE* × *SYSTEM\_TIME\_TYPE* × *SYSTEM\_TIME\_TYPE* × *OPERATING\_MODE\_TYPE*  
**channel** *system\_call\_service\_routine\_delayed\_start\_input* : *PARTITION\_ID\_TYPE* × *PROCESS\_ID\_TYPE* × *PROCESS\_ID\_TYPE* × *SYSTEM\_TIME\_TYPE* × *SYSTEM\_TIME\_TYPE* × *SYSTEM\_TIME\_TYPE* × *OPERATING\_MODE\_TYPE*  
**channel** *system\_call\_service\_routine\_lock\_preemption\_output* : *PARTITION\_ID\_TYPE* × *PROCESS\_ID\_TYPE* × *LOCK\_LEVEL\_TYPE*  
**channel** *system\_call\_service\_routine\_unlock\_preemption\_output* : *PARTITION\_ID\_TYPE* × *PROCESS\_ID\_TYPE* × *LOCK\_LEVEL\_TYPE*  
**channel** *system\_call\_service\_routine\_get\_my\_id\_output* : *PARTITION\_ID\_TYPE* × *PROCESS\_ID\_TYPE* × *PROCESS\_ID\_TYPE*  
**channel** *system\_call\_service\_routine\_get\_current\_time\_output* : *PARTITION\_ID\_TYPE* × *PROCESS\_ID\_TYPE* × *SYSTEM\_TIME\_TYPE*  
**channel** *system\_call\_service\_routine\_get\_partition\_time\_output* : *PARTITION\_ID\_TYPE* × *PROCESS\_ID\_TYPE* × *SYSTEM\_TIME\_TYPE*  
**channel** *system\_call\_service\_routine\_get\_next\_release\_point\_input* : *PARTITION\_ID\_TYPE* × *PROCESS\_ID\_TYPE* × *PROCESS\_ID\_TYPE*  
**channel** *system\_call\_service\_routine\_get\_next\_release\_point\_output* : *PARTITION\_ID\_TYPE* × *PROCESS\_ID\_TYPE* × *SYSTEM\_TIME\_TYPE*  
**channel** *system\_call\_service\_routine\_timed\_wait\_input* : *PARTITION\_ID\_TYPE* × *PROCESS\_ID\_TYPE* × *SYSTEM\_TIME\_TYPE* × *SYSTEM\_TIME\_TYPE*  
**channel** *system\_call\_service\_routine\_periodic\_wait\_input* : *PARTITION\_ID\_TYPE* × *PROCESS\_ID\_TYPE* × *SYSTEM\_TIME\_TYPE* × *SYSTEM\_TIME\_TYPE*  
**channel** *system\_call\_service\_routine\_get\_time\_output* : *PARTITION\_ID\_TYPE* × *PROCESS\_ID\_TYPE* × *SYSTEM\_TIME\_TYPE*

**channel** *system\_call\_service\_routine\_replenish\_input* : *PARTITION\_ID\_TYPE* × *PROCESS\_ID\_TYPE* × *SYSTEM\_TIME\_TYPE* × *SYSTEM\_TIME\_TYPE*  
**channel** *system\_call\_return* : *PARTITION\_ID\_TYPE* × *PROCESS\_ID\_TYPE*

## C.16 Channels for communication between APEX Layer and File System

**channel** *apex\_function\_request\_executable\_file* : *PARTITION\_ID\_TYPE* × *PROCESS\_ID\_TYPE* × *PATH\_TYPE*  
**channel** *apex\_function\_get\_executable\_file* : *PARTITION\_ID\_TYPE* × *PROCESS\_ID\_TYPE* × *EXECUTABLE\_FILE\_TYPE*

## C.17 Channels for Return Code

**channel** *apex\_function\_return\_code* : *PARTITION\_ID\_TYPE* × *PROCESS\_ID\_TYPE* × *RETURN\_CODE\_TYPE*

## C.18 Channels for communication between APEX Layer and Application of each Partition

**channel** *apex\_function\_get\_partition\_status* : *PARTITION\_ID\_TYPE* × *PROCESS\_ID\_TYPE*  
**channel** *apex\_function\_get\_partition\_status\_output* : *PARTITION\_ID\_TYPE* × *PROCESS\_ID\_TYPE* × *PARTITION\_STATUS\_TYPE*  
**channel** *apex\_function\_get\_partition\_status\_return* : *PARTITION\_ID\_TYPE* × *PROCESS\_ID\_TYPE*  
**channel** *apex\_function\_set\_operating\_mode* : *PARTITION\_ID\_TYPE* × *PROCESS\_ID\_TYPE*  
**channel** *apex\_function\_set\_operating\_mode\_input* : *PARTITION\_ID\_TYPE* × *PROCESS\_ID\_TYPE* × *OPERATING\_MODE\_TYPE*  
**channel** *apex\_function\_set\_operating\_mode\_return* : *PARTITION\_ID\_TYPE* × *PROCESS\_ID\_TYPE*  
**channel** *apex\_function\_get\_process\_id* : *PARTITION\_ID\_TYPE* × *PROCESS\_ID\_TYPE*  
**channel** *apex\_function\_get\_process\_id\_input* : *PARTITION\_ID\_TYPE* × *PROCESS\_ID\_TYPE* × *PROCESS\_NAME\_TYPE*  
**channel** *apex\_function\_get\_process\_id\_output* : *PARTITION\_ID\_TYPE* × *PROCESS\_ID\_TYPE* × *PROCESS\_ID\_TYPE*  
**channel** *apex\_function\_get\_process\_id\_return* : *PARTITION\_ID\_TYPE* × *PROCESS\_ID\_TYPE*  
**channel** *apex\_function\_get\_process\_status* : *PARTITION\_ID\_TYPE* × *PROCESS\_ID\_TYPE*  
**channel** *apex\_function\_get\_process\_status\_input* : *PARTITION\_ID\_TYPE* × *PROCESS\_ID\_TYPE* × *PROCESS\_ID\_TYPE*  
**channel** *apex\_function\_get\_process\_status\_output* : *PARTITION\_ID\_TYPE* × *PROCESS\_ID\_TYPE* × *PROCESS\_STATUS\_TYPE*  
**channel** *apex\_function\_get\_process\_status\_return* : *PARTITION\_ID\_TYPE* × *PROCESS\_ID\_TYPE*  
**channel** *apex\_function\_create\_process* : *PARTITION\_ID\_TYPE* × *PROCESS\_ID\_TYPE*  
**channel** *apex\_function\_create\_process\_input* : *PARTITION\_ID\_TYPE* × *PROCESS\_ID\_TYPE* × *PROCESS\_ATTRIBUTE\_TYPE* × *PATH\_TYPE* × *PATH\_TYPE*  
**channel** *apex\_function\_create\_process\_output* : *PARTITION\_ID\_TYPE* × *PROCESS\_ID\_TYPE* × *PROCESS\_ID\_TYPE*  
**channel** *apex\_function\_create\_process\_return* : *PARTITION\_ID\_TYPE* × *PROCESS\_ID\_TYPE*  
**channel** *apex\_function\_set\_priority* : *PARTITION\_ID\_TYPE* × *PROCESS\_ID\_TYPE*  
**channel** *apex\_function\_set\_priority\_input* : *PARTITION\_ID\_TYPE* × *PROCESS\_ID\_TYPE* × *PROCESS\_ID\_TYPE* × *PRIORITY\_TYPE*  
**channel** *apex\_function\_set\_priority\_return* : *PARTITION\_ID\_TYPE* × *PROCESS\_ID\_TYPE*

**channel** *apex\_function\_suspend\_self* : *PARTITION\_ID\_TYPE* × *PROCESS\_ID\_TYPE*  
**channel** *apex\_function\_suspend\_self\_input* : *PARTITION\_ID\_TYPE* × *PROCESS\_ID\_TYPE* × *SYSTEM\_TIME\_TYPE*  
**channel** *apex\_function\_suspend\_self\_return* : *PARTITION\_ID\_TYPE* × *PROCESS\_ID\_TYPE*  
**channel** *apex\_function\_suspend* : *PARTITION\_ID\_TYPE* × *PROCESS\_ID\_TYPE*  
**channel** *apex\_function\_suspend\_input* : *PARTITION\_ID\_TYPE* × *PROCESS\_ID\_TYPE* × *PROCESS\_ID\_TYPE*  
**channel** *apex\_function\_suspend\_return* : *PARTITION\_ID\_TYPE* × *PROCESS\_ID\_TYPE*  
**channel** *apex\_function\_resume* : *PARTITION\_ID\_TYPE* × *PROCESS\_ID\_TYPE*  
**channel** *apex\_function\_resume\_input* : *PARTITION\_ID\_TYPE* × *PROCESS\_ID\_TYPE* × *PROCESS\_ID\_TYPE*  
**channel** *apex\_function\_resume\_return* : *PARTITION\_ID\_TYPE* × *PROCESS\_ID\_TYPE*  
**channel** *apex\_function\_stop\_self* : *PARTITION\_ID\_TYPE* × *PROCESS\_ID\_TYPE*  
**channel** *apex\_function\_stop* : *PARTITION\_ID\_TYPE* × *PROCESS\_ID\_TYPE*  
**channel** *apex\_function\_stop\_input* : *PARTITION\_ID\_TYPE* × *PROCESS\_ID\_TYPE* × *PROCESS\_ID\_TYPE*  
**channel** *apex\_function\_stop\_return* : *PARTITION\_ID\_TYPE* × *PROCESS\_ID\_TYPE*  
**channel** *apex\_function\_start* : *PARTITION\_ID\_TYPE* × *PROCESS\_ID\_TYPE*  
**channel** *apex\_function\_start\_input* : *PARTITION\_ID\_TYPE* × *PROCESS\_ID\_TYPE* × *PROCESS\_ID\_TYPE*  
**channel** *apex\_function\_start\_return* : *PARTITION\_ID\_TYPE* × *PROCESS\_ID\_TYPE*  
**channel** *apex\_function\_delayed\_start* : *PARTITION\_ID\_TYPE* × *PROCESS\_ID\_TYPE*  
**channel** *apex\_function\_delayed\_start\_input* : *PARTITION\_ID\_TYPE* × *PROCESS\_ID\_TYPE* × *PROCESS\_ID\_TYPE* × *SYSTEM\_TIME\_TYPE*  
**channel** *apex\_function\_delayed\_start\_return* : *PARTITION\_ID\_TYPE* × *PROCESS\_ID\_TYPE*  
**channel** *apex\_function\_lock\_preemption* : *PARTITION\_ID\_TYPE* × *PROCESS\_ID\_TYPE*  
**channel** *apex\_function\_lock\_preemption\_output* : *PARTITION\_ID\_TYPE* × *PROCESS\_ID\_TYPE* × *LOCK\_LEVEL\_TYPE*  
**channel** *apex\_function\_lock\_preemption\_return* : *PARTITION\_ID\_TYPE* × *PROCESS\_ID\_TYPE*  
**channel** *apex\_function\_unlock\_preemption* : *PARTITION\_ID\_TYPE* × *PROCESS\_ID\_TYPE*  
**channel** *apex\_function\_unlock\_preemption\_output* : *PARTITION\_ID\_TYPE* × *PROCESS\_ID\_TYPE* × *LOCK\_LEVEL\_TYPE*  
**channel** *apex\_function\_unlock\_preemption\_return* : *PARTITION\_ID\_TYPE* × *PROCESS\_ID\_TYPE*  
**channel** *apex\_function\_get\_my\_id* : *PARTITION\_ID\_TYPE* × *PROCESS\_ID\_TYPE*  
**channel** *apex\_function\_get\_my\_id\_output* : *PARTITION\_ID\_TYPE* × *PROCESS\_ID\_TYPE* × *PROCESS\_ID\_TYPE*  
**channel** *apex\_function\_get\_my\_id\_return* : *PARTITION\_ID\_TYPE* × *PROCESS\_ID\_TYPE*  
**channel** *apex\_function\_timed\_wait* : *PARTITION\_ID\_TYPE* × *PROCESS\_ID\_TYPE*  
**channel** *apex\_function\_timed\_wait\_input* : *PARTITION\_ID\_TYPE* × *PROCESS\_ID\_TYPE* × *SYSTEM\_TIME\_TYPE*  
**channel** *apex\_function\_timed\_wait\_return* : *PARTITION\_ID\_TYPE* × *PROCESS\_ID\_TYPE*  
**channel** *apex\_function\_periodic\_wait* : *PARTITION\_ID\_TYPE* × *PROCESS\_ID\_TYPE*  
**channel** *apex\_function\_periodic\_wait\_return* : *PARTITION\_ID\_TYPE* × *PROCESS\_ID\_TYPE*  
**channel** *apex\_function\_get\_time* : *PARTITION\_ID\_TYPE* × *PROCESS\_ID\_TYPE*  
**channel** *apex\_function\_get\_time\_output* : *PARTITION\_ID\_TYPE* × *PROCESS\_ID\_TYPE* × *SYSTEM\_TIME\_TYPE*  
**channel** *apex\_function\_get\_time\_return* : *PARTITION\_ID\_TYPE* × *PROCESS\_ID\_TYPE*  
**channel** *apex\_function\_replenish* : *PARTITION\_ID\_TYPE* × *PROCESS\_ID\_TYPE*  
**channel** *apex\_function\_replenish\_input* : *PARTITION\_ID\_TYPE* × *PROCESS\_ID\_TYPE* × *SYSTEM\_TIME\_TYPE*  
**channel** *apex\_function\_replenish\_return* : *PARTITION\_ID\_TYPE* × *PROCESS\_ID\_TYPE*





## D Circus Processes

### D.1 Core Hardware Layer

#### D.1.1 Generic CPU

```
process GenericCPU  $\hat{=}$   
begin  
state CPU_REGISTER_TYPE
```

*Initialize*  $\hat{=}$  *InitCPURegisters*

*SavePart*  $\hat{=}$  **var** *cpureg* : *CPU\_REGISTER\_TYPE* •  
    *context\_switching\_save\_part\_cpu\_registers*  $\longrightarrow$  *SavePartCPURegister*[*cpureg*/*cpureg*!];  
    *context\_switching\_saved\_part\_cpu\_registers* !*cpureg*  $\longrightarrow$  **Skip**

*SaveAll*  $\hat{=}$  **var** *cpureg* : *CPU\_REGISTER\_TYPE* •  
    *context\_switching\_save\_all\_cpu\_registers*  $\longrightarrow$  *SaveAllCPURegister*[*cpureg*/*cpureg*!];  
    *context\_switching\_saved\_all\_cpu\_registers* !*cpureg*  $\longrightarrow$  **Skip**

*RestorePart*  $\hat{=}$  *context\_switching\_restore\_part\_cpu\_registers* ?*cpureg*  $\longrightarrow$   
    *RestorePartCPURegister*[*cpureg*/*cpureg*?];  
    *context\_switching\_restored\_part\_cpu\_registers*  $\longrightarrow$  **Skip**

*RestoreAll*  $\hat{=}$  *context\_switching\_restore\_all\_cpu\_registers* ?*cpureg*  $\longrightarrow$   
    *RestoreAllCPURegister*[*cpureg*/*cpureg*?];  
    *context\_switching\_restored\_all\_cpu\_registers*  $\longrightarrow$  **Skip**

*SetStackSegment*  $\hat{=}$  *context\_switching\_set\_stack\_segment\_registers* ?*ssreg*  $\longrightarrow$  *SetStackSegRegister*[*ssreg*/*ssreg*?];  
    *context\_switching\_have\_set\_stack\_segment\_registers*  $\longrightarrow$  **Skip**

*SetIFOn*  $\hat{=}$  *interrupt\_controlling\_enable\_interrupt*  $\longrightarrow$  *PSWRegisters*.*IF* := 1;  
    *interrupt\_controlling\_enabled\_interrupt*  $\longrightarrow$  **Skip**

*SetIFOff*  $\hat{=}$  *interrupt\_controlling\_disable\_interrupt*  $\longrightarrow$  *PSWRegisters*.*IF* := 0;  
    *interrupt\_controlling\_disabled\_interrupt*  $\longrightarrow$  **Skip**

*CPURegisterService*  $\hat{=}$  *SavePart*  $\square$  *SaveAll*  $\square$  *RestorePart*  $\square$  *RestoreAll*  $\square$  *SetIFOn*  $\square$  *SetIFOff*

*InterruptResponse\_Pre*  $\hat{=}$  (*PSWRegisters*.*IF* = 1) & *interrupt* ?*i*  $\longrightarrow$  *interrupt\_acknowledged*  $\longrightarrow$   
    *interrupt\_handler\_start\_interrupt\_handling* !*i*  $\longrightarrow$  **Skip**  
     $\square$  (*PSWRegisters*.*IF* = 0) & **Skip**

*InterruptResponse\_Pro*  $\hat{=}$  *interrupt\_handler\_finish\_interrupt\_handling* ?*i*  $\longrightarrow$   
    *interrupt\_handled* !*i*  $\longrightarrow$  **Skip**

*InterruptResponse*  $\hat{=}$  *InterruptResponse\_Pre*  $\square$  *InterruptResponse\_Pro*

*ExceptionResponse\_Pre*  $\hat{=}$  *exception* ?*e*  $\longrightarrow$  *exception\_handler\_start\_exception\_handling* !*e*  $\longrightarrow$  **Skip**

*ExceptionResponse\_Pro*  $\hat{=}$  *exception\_handler\_finish\_exception\_handling*  $\longrightarrow$  **Skip**

*ExceptionResponse*  $\hat{=}$  *ExceptionResponse\_Pre*  $\square$  *ExceptionResponse\_Pro*

$CPUService \hat{=} CPURegisterService \sqcap InterruptResponse \sqcap ExceptionResponse$

$ExecCPUService \hat{=} \mu X \bullet CPUService ; X$

$\bullet module\_init \longrightarrow (Initialize ; ExecCPUService) \Delta module\_end \longrightarrow \mathbf{Skip}$

**end**

### D.1.2 Memory Management Unit (MMU)

**process** *MemoryManagementUnit*  $\hat{=}$

**begin**

**state** *MEMORY\_MANAGEMENT\_UNIT\_TYPE*

$Initialize \hat{=} PageTableBuffer := \emptyset$

$SetPageTableBuffer \hat{=} context\_switching\_set\_page\_table \ ?pt \longrightarrow PageTableBuffer := pt ;$   
 $context\_switching\_have\_set\_page\_table \longrightarrow \mathbf{Skip}$

$Translate \hat{=} \mathbf{var} \ la, pa : SYSTEM\_ADDRESS\_TYPE \bullet$   
 $cpu\_request\_logical\_address\_translation \ ?seg \ ?limit \ ?offset \longrightarrow$   
 $\left( \begin{array}{l} \mathbf{if} \ (offset > limit) \longrightarrow logical\_address\_translation\_fail \longrightarrow \\ \quad exception \ !ACCESS\_VIOLATION \longrightarrow \mathbf{Skip} \\ \quad \parallel \ (offset \leq limit) \longrightarrow la := seg + offset ; \\ \quad \left( \begin{array}{l} \mathbf{if} \ (getpage(la) \notin \text{dom } PageTableBuffer) \longrightarrow \\ \quad logical\_address\_translation\_fail \longrightarrow \\ \quad exception \ !PAGE\_FAULT \longrightarrow \mathbf{Skip} \\ \quad \parallel \ (getpage(la) \in \text{dom } PageTableBuffer) \longrightarrow \\ \quad \quad TransLinearAddress[la/la?, pa/pa!]; \\ \quad \quad cpu\_get\_logical\_address\_translation \ !pa \longrightarrow \mathbf{Skip} \\ \quad \mathbf{fi} \end{array} \right) \end{array} \right)$   
 $\mathbf{fi}$

$GetPageTableBuffer \hat{=} context\_switching\_request\_page\_table \longrightarrow$   
 $context\_switching\_get\_page\_table \ !PageTableBuffer \longrightarrow \mathbf{Skip}$

$MMUService \hat{=} SetPageTableBuffer \sqcap Translate \sqcap GetPageTableBuffer$

$ExecMMUService \hat{=} \mu X \bullet MMUService ; X$

$\bullet module\_init \longrightarrow (Initialize ; ExecMMUService) \Delta module\_end \longrightarrow \mathbf{Skip}$

**end**

### D.1.3 Main Memory

```

process MainMemory  $\hat{=}$ 
begin
state MAIN_MEMORY_TYPE

  Initialize  $\hat{=}$  Store :=  $\emptyset$ 

  Read  $\hat{=}$  cpu_receive_data_from_main_memory ?a  $\longrightarrow$ 
           cpu_received_data_from_main_memory !Store(a)  $\longrightarrow$  Skip

  Write  $\hat{=}$  cpu_send_data_to_main_memory ?a ?data  $\longrightarrow$  Store(a) := data
           cpu_sent_data_to_main_memory  $\longrightarrow$  Skip

  Load  $\hat{=}$  memory_management_load_page_into_main_memory ?page ?piece  $\longrightarrow$ 
           LoadPage[page/page?, piece/piece?];
           memory_management_loaded_page_into_main_memory  $\longrightarrow$  Skip

  Extract  $\hat{=}$  var piece : PIECE_TYPE •
             memory_management_extract_page_from_main_memory ?page  $\longrightarrow$ 
             ExtractPage[page/page?, piece/piece?];
             memory_management_extracted_page_from_main_memory !piece  $\longrightarrow$  Skip

  MainMemoryService  $\hat{=}$  Read  $\square$  Write  $\square$  Load  $\square$  Extract

  ExecMainMemoryService  $\hat{=}$   $\mu X \bullet$  MainMemoryService ; X

  • module_init  $\longrightarrow$  (Initialize ; ExecMainMemoryService)  $\Delta$  module_end  $\longrightarrow$  Skip
end

```

### D.1.4 Real-Time Clock

```

process RTClock  $\hat{=}$ 
begin
state RTCLOCK_TYPE

  Initialize  $\hat{=}$  Value := 0PSU

  RunClockPause  $\hat{=}$   $\mu X \bullet$  (wait(1) ; Value := Value + 1PSU ; clock_pause) ; X

  RTClockService  $\hat{=}$  system_clock_request_current_time  $\longrightarrow$ 
           system_clock_get_current_time !Value  $\longrightarrow$  Skip

  ExecRTClockService  $\hat{=}$   $\mu X \bullet$  RTClockService ; X

  • rtclock_power_on  $\longrightarrow$  (Initialize ; RunClockPause ||| ExecRTClockService)  $\Delta$  rtclock_power_off  $\longrightarrow$  Skip
end

```

### D.1.5 Timer

```

process Timer  $\hat{=}$ 
begin
state TIMER_TYPE

  Initialize  $\hat{=}$  InitTimer[ClockTickInterval/p?]

  ClockTick  $\hat{=}$  clock_pause  $\longrightarrow$  Value := Value + 1PSU;
                $\left( \begin{array}{l} \textbf{if} \quad (\textit{Value} \neq \textit{Period}) \longrightarrow \textbf{Skip} \\ \quad \parallel \quad (\textit{Value} = \textit{Period}) \longrightarrow \textit{Value} := 0_{\textit{PSU}}; \\ \quad \textit{hardware\_interrupts} \textbf{!} \textit{CLOCK\_TICK} \longrightarrow \textbf{Skip} \\ \textbf{fi} \end{array} \right)$ 

  RunClockTick  $\hat{=}$   $\mu X \bullet \textit{ClockTick} ; X$ 

   $\bullet \textit{module\_init} \longrightarrow (\textit{Initialize} ; \textit{RunClockTick}) \Delta \textit{module\_end} \longrightarrow \textbf{Skip}$ 

end

```

### D.1.6 High-Precision Timer

```

process HPTimer  $\hat{=}$ 
begin
state HPTIMER_TYPE

  Initialize  $\hat{=}$  InitHPTimer

  ClockTick  $\hat{=}$   $\text{clock\_pause} \longrightarrow \text{Value} := \text{Value} + 1_{PSU};$ 
     $\left( \begin{array}{l} \textbf{if} \quad (\text{Value} \neq \text{Alarm}) \longrightarrow \textbf{Skip} \\ \quad \parallel \quad (\text{Value} = \text{Alarm}) \longrightarrow \\ \quad \quad \text{hardware\_interrupts !CLOCK\_TICK} \longrightarrow \textbf{Skip} \\ \textbf{fi} \end{array} \right)$ 

  RunClockTick  $\hat{=}$   $\mu X \bullet \text{ClockTick} ; X$ 

  GetTime  $\hat{=}$   $\text{system\_clock\_request\_high\_precision\_time} \longrightarrow$ 
     $\text{system\_clock\_get\_high\_precision\_time !Value} \longrightarrow \textbf{Skip}$ 

  SetAlarm  $\hat{=}$   $\text{system\_clock\_set\_high\_precision\_timer\_alarm ?a} \longrightarrow \text{Alarm} := a;$ 
     $\text{system\_clock\_have\_set\_high\_precision\_timer\_alarm} \longrightarrow \textbf{Skip}$ 

  HPTimerService  $\hat{=}$  GetTime  $\square$  SetAlarm

  ExecHPTimerService  $\hat{=}$   $\mu X \bullet \text{HPTimerService} ; X$ 

  ResetHPTimer  $\hat{=}$   $\text{system\_clock\_reset\_high\_precision\_timer} \longrightarrow \text{InitHPTimer};$ 
     $\text{system\_clock\_have\_reset\_high\_precision\_timer} \longrightarrow \textbf{Skip}$ 

  EndHPTimer  $\hat{=}$   $\text{system\_clock\_end\_high\_precision\_timer} \longrightarrow \text{Alarm} := \text{LIMIT}_{PSU};$ 
     $\text{system\_clock\_ended\_high\_precision\_timer} \longrightarrow \textbf{Skip}$ 

  RunHPTimer  $\hat{=}$   $\mu X \bullet (\text{ResetHPTimer} ; (\text{RunClockInterrupt} \parallel \text{ExecHPTimerService}) \Delta \text{EndHPTimer}) ; X$ 

   $\bullet \text{ module\_init} \longrightarrow (\text{Initialize} ; \text{RunHPTimer}) \Delta \text{ module\_end} \longrightarrow \textbf{Skip}$ 
end

```

### D.1.7 ChannelSets for communication within Interrupt Controller

```

channelset IRR_PR ==  $\{ \text{irregister\_report\_new\_interrupt} \}$ 
channelset PR_ISR ==  $\{ \text{priority\_resolver\_report\_new\_interrupt} \}$ 
channelset ISR_IRR ==  $\{ \text{isregister\_service\_new\_interrupt}, \text{isregister\_demand\_new\_interrupt} \}$ 

channelset ICChannels ==  $\text{IRR\_PR} \cup \text{PR\_ISR} \cup \text{ISR\_IRR}$ 

```



### D.1.8 Interrupt Controller

**process** *InterruptController*  $\hat{=}$

**begin**

**state** *INTERRUPT\_HANDLER\_STATE\_TYPE*

*Initialize*  $\hat{=}$  *InitInterruptController*

*IRRServePre<sub>1</sub>*  $\hat{=}$  **var** *rints* :  $\mathbb{P}$  *INTERRUPT\_TYPE* •  
*hardware\_interrupts* ?*i*  $\longrightarrow$  *IRRegister*(*i*) := 1 ; *GetRequestInterrupts*[*rints*/*ints*];  
 $\left( \begin{array}{l} \textbf{if} \quad (i > \min(\textit{rints})) \longrightarrow \textbf{Skip} \\ \quad \parallel \\ \quad (i = \min(\textit{rints})) \longrightarrow \textit{irregister\_report\_new\_interrupt} \text{ !}i \longrightarrow \textbf{Skip} \\ \textbf{fi} \end{array} \right)$

*IRRServePre<sub>2</sub>*  $\hat{=}$  **var** *rints* :  $\mathbb{P}$  *INTERRUPT\_TYPE* •  
*isregister\_demand\_new\_interrupt*  $\longrightarrow$  *GetRequestInterrupts*[*rints*/*ints*];  
 $\left( \begin{array}{l} \textbf{if} \quad (\textit{rints} = \emptyset) \longrightarrow \textbf{Skip} \\ \quad \parallel \\ \quad (\textit{rints} \neq \emptyset) \longrightarrow \textit{irregister\_report\_new\_interrupt} \text{ !}\min(\textit{rints}) \longrightarrow \textbf{Skip} \\ \textbf{fi} \end{array} \right)$

*IRRServePro*  $\hat{=}$  *isregister\_service\_new\_interrupt* ?*i*  $\longrightarrow$  *IRRegister*(*i*) := 0

*IRRServe*  $\hat{=}$  *IRRServePre<sub>1</sub>*  $\square$  *IRRServePre<sub>2</sub>*  $\square$  *IRRServePro*

*ExecIRRServe*  $\hat{=}$   $\mu X \bullet \textit{IRRServe} ; X$

*IMRServeMask*  $\hat{=}$  *interrupt\_controlling\_mask\_interrupt* ?*i*  $\longrightarrow$  *IMRegister*(*i*) := 1;  
*interrupt\_controlling\_masked\_interrupt*  $\longrightarrow$  **Skip**

*IMRServeUnmask*  $\hat{=}$  *interrupt\_controlling\_unmask\_interrupt* ?*i*  $\longrightarrow$  *IMRegister*(*i*) := 0;  
*interrupt\_controlling\_unmasked\_interrupt*  $\longrightarrow$  **Skip**

*IMRServe*  $\hat{=}$  *IMRServeMask*  $\square$  *IMRServeUnmask*

*ExecIMRServe*  $\hat{=}$   $\mu X \bullet \textit{IMRServe} ; X$

*PRService*  $\hat{=}$  **var** *mints*, *isints* :  $\mathbb{P}$  *INTERRUPT\_TYPE* •  
*irregister\_report\_new\_interrupt* ?*i*  $\longrightarrow$  *GetMaskedInterrupts*[*mints*/*ints*!];  
 $\left( \begin{array}{l} \textbf{if} \quad (i \in \textit{mints}) \longrightarrow \textbf{Skip} \\ \quad \parallel \\ \quad (i \notin \textit{mints}) \longrightarrow \textit{GetInServiceInterrupts}[\textit{isints}/\textit{ints!}; \\ \quad \quad \left( \begin{array}{l} \textbf{if} \quad (\textit{isints} = \emptyset) \longrightarrow \\ \quad \quad \textit{priority\_resolver\_report\_new\_interrupt} \text{ !}i \longrightarrow \textbf{Skip} \\ \quad \quad \parallel \\ \quad \quad (\textit{isints} \neq \emptyset) \longrightarrow \\ \quad \quad \quad \left( \begin{array}{l} \textbf{if} \quad (\min(\textit{isints}) \leq i) \longrightarrow \textbf{Skip} \\ \quad \parallel \\ \quad \quad (\min(\textit{isints}) > i) \longrightarrow \\ \quad \quad \quad \textit{priority\_resolver\_report\_new\_interrupt} \\ \quad \quad \quad \text{ !}i \longrightarrow \textbf{Skip} \\ \textbf{fi} \end{array} \right) \\ \textbf{fi} \end{array} \right) \\ \textbf{fi} \end{array} \right)$

*ExecPRService*  $\hat{=}$   $\mu X \bullet \textit{PRService} ; X$

$$\begin{aligned}
ISRService\_Pre &\hat{=} \text{priority\_resolver\_report\_new\_interrupt } ?i \longrightarrow ISRegister(i) := 1; \\
&\quad isregister\_service\_new\_interrupt !i \longrightarrow \\
&\quad interrupt !i \longrightarrow interrupt\_acknowledged \longrightarrow \mathbf{Skip} \\
\\
ISRService\_Pro &\hat{=} \mathbf{var} \text{ isints} : \mathbb{P} \text{ INTERRUPT\_TYPE } \bullet \\
&\quad interrupt\_handled ?i \longrightarrow ISRegister(i) := 0 ; \text{ GetInServiceInterrupts[isints/s!];} \\
&\quad \left( \begin{array}{l} \mathbf{if} \quad (isints \neq \emptyset) \longrightarrow \mathbf{Skip} \\ \quad \parallel \quad (isints = \emptyset) \longrightarrow isregister\_demand\_new\_interrupt \longrightarrow \mathbf{Skip} \\ \mathbf{fi} \end{array} \right) \\
\\
ISRService &\hat{=} ISRService\_Pre \sqcap ISRService\_Pro \\
\\
ExecISRService &\hat{=} \mu X \bullet ISRService ; X \\
\\
ExecInterruptControllerService &\hat{=} ExecIMRService \parallel (ExecIRRService \llbracket ICChannels \rrbracket ExecPRService \\
&\quad \llbracket ICChannels \rrbracket ExecISRService) \\
\\
&\bullet \text{ module\_init } \longrightarrow (\text{Initialize} ; ExecInterruptControllerService) \Delta \text{ module\_end } \longrightarrow \mathbf{Skip} \\
\\
&\mathbf{end}
\end{aligned}$$

#### D.1.9 ChannelSets for communication between different parts of Core Hardware Layer

$$\begin{aligned}
\text{channelset } CPU\_IC &== \{ interrupt, interrupt\_acknowledged, interrupt\_handled \} \\
\text{channelset } CPU\_MMU &== \{ cpu\_request\_logical\_address\_translation, \\
&\quad logical\_address\_translation\_fail, exception, \\
&\quad cpu\_get\_logical\_address\_translation \} \\
\text{channelset } CPU\_MEMORY &== \{ cpu\_receive\_data\_from\_main\_memory, \\
&\quad cpu\_received\_data\_from\_main\_memory, \\
&\quad cpu\_send\_data\_to\_main\_memory, \\
&\quad cpu\_sent\_data\_to\_main\_memory \} \\
\\
\text{channelset } RTC\_TIMER &== \{ clock\_pause \} \\
\text{channelset } RTC\_HPTIMER &== \{ clock\_pause \} \\
\text{channelset } TIMER\_IC &== \{ hardware\_interrupts \} \\
\text{channelset } HPTIMER\_IC &== \{ hardware\_interrupts \} \\
\\
\text{channelset } CHLayerChannels &== CPU\_IC \cup CPU\_MMU \cup CPU\_MEMORY \\
&\quad \cup RTC\_TIMER \cup RTC\_HPTIMER \\
&\quad \cup TIMER\_IC \cup HPTIMER\_IC
\end{aligned}$$

#### D.1.10 Core Hardware Layer Model

$$\begin{aligned}
\mathbf{process} \text{ Core\_Hardware\_Layer} &\hat{=} \\
\\
&CPU \llbracket CHLayerChannels \rrbracket \text{MemoryManagementUnit} \llbracket CHLayerChannels \rrbracket \text{MainMemory} \\
&\llbracket CHLayerChannels \rrbracket \text{RTClock} \llbracket CHLayerChannels \rrbracket \text{Timer} \llbracket CHLayerChannels \rrbracket \text{HPTimer} \\
&\llbracket CHLayerChannels \rrbracket \text{InterruptController}
\end{aligned}$$



## D.2 Hardware Interface Software Layer

### D.2.1 Context Switching

**process** *ContextSwitching*  $\hat{=}$   
**begin**

*SwitchOut\_IntHandler*  $\hat{=}$  *interrupt\_handler\_save\_context*  $\longrightarrow$   
*context\_switching\_save\_all\_cpu\_registers*  $\longrightarrow$   
*context\_switching\_saved\_all\_cpu\_registers* *?cpureg*  $\longrightarrow$   
*context\_switching\_request\_page\_table*  $\longrightarrow$   
*context\_switching\_get\_page\_table* *?pt*  $\longrightarrow$   
*interrupt\_handler\_saved\_context* *!cpureg* *!pt*  $\longrightarrow$  **Skip**

*SwitchIn\_IntHandler*  $\hat{=}$  *interrupt\_handler\_restore\_context* *?cpureg* *?pt*  $\longrightarrow$   
*context\_switching\_restore\_all\_cpu\_registers* *!cpureg*  $\longrightarrow$   
*context\_switching\_restored\_all\_cpu\_registers*  $\longrightarrow$   
*context\_switching\_set\_page\_table* *!pt*  $\longrightarrow$   
*context\_switching\_have\_set\_page\_table*  $\longrightarrow$   
*interrupt\_handler\_restored\_context*  $\longrightarrow$  **Skip**

*SwitchStack\_IntHandler*  $\hat{=}$  *interrupt\_handler\_switch\_stack* *?ssreg* *?pt*  $\longrightarrow$   
*context\_switching\_set\_stack\_segment\_registers* *!ssreg*  $\longrightarrow$   
*context\_switching\_have\_set\_stack\_segment\_registers*  $\longrightarrow$   
*context\_switching\_set\_page\_table* *!pt*  $\longrightarrow$   
*context\_switching\_have\_set\_page\_table*  $\longrightarrow$   
*interrupt\_handler\_switched\_stack*  $\longrightarrow$  **Skip**

*ContextSwitching\_IntHandler*  $\hat{=}$  *SwitchOut\_IntHandler*  $\square$  *SwitchIn\_IntHandler*  $\square$  *SwitchStack\_IntHandler*

*SwitchOut\_Kernel*  $\hat{=}$  *kernel\_save\_context.kernelid* *?option*  $\longrightarrow$   
 $\left( \begin{array}{l} \textbf{if } (option = PART) \longrightarrow \\ \quad context\_switching\_save\_part\_cpu\_registers \longrightarrow \\ \quad context\_switching\_saved\_part\_cpu\_registers \text{ ?cpureg } \longrightarrow \\ \quad context\_switching\_request\_page\_table \longrightarrow \\ \quad context\_switching\_get\_page\_table \text{ ?pt } \longrightarrow \\ \quad kernel\_saved\_context.kernelid \text{ !cpureg !pt } \longrightarrow \textbf{Skip} \\ \quad \square \\ \quad (option = ALL) \longrightarrow \\ \quad context\_switching\_save\_all\_cpu\_registers \longrightarrow \\ \quad context\_switching\_saved\_all\_cpu\_registers \text{ ?cpureg } \longrightarrow \\ \quad context\_switching\_request\_page\_table \longrightarrow \\ \quad context\_switching\_get\_page\_table \text{ ?pt } \longrightarrow \\ \quad kernel\_saved\_context.kernelid \text{ !cpureg !pt } \longrightarrow \textbf{Skip} \\ \textbf{fi} \end{array} \right)$

$$\begin{aligned}
\text{SwitchIn\_Kernel} \quad \hat{=} \quad & \text{kernel\_restore\_context.kernelid} \text{ ?option ?cpureg ?pt} \longrightarrow \\
& \left( \begin{array}{l}
\text{if } (\text{option} = \text{PART}) \longrightarrow \\
\quad \text{context\_switching\_restore\_part\_cpu\_registers !cpureg} \longrightarrow \\
\quad \text{context\_switching\_restored\_part\_cpu\_registers} \longrightarrow \\
\quad \text{context\_switching\_set\_page\_table !pt} \longrightarrow \\
\quad \text{context\_switching\_have\_set\_page\_table} \longrightarrow \\
\quad \text{kernel\_restored\_context.kernelid} \longrightarrow \mathbf{Skip} \\
\quad \square \\
\quad (\text{option} = \text{ALL}) \longrightarrow \\
\quad \text{context\_switching\_restore\_all\_cpu\_registers !cpureg} \longrightarrow \\
\quad \text{context\_switching\_restored\_all\_cpu\_registers} \longrightarrow \\
\quad \text{context\_switching\_set\_page\_table !pt} \longrightarrow \\
\quad \text{context\_switching\_have\_set\_page\_table} \longrightarrow \\
\quad \text{kernel\_restored\_context.kernelid} \longrightarrow \mathbf{Skip} \\
\text{fi}
\end{array} \right)
\end{aligned}$$

$$\begin{aligned}
\text{SwitchStack\_Kernel} \quad \hat{=} \quad & \text{kernel\_switch\_stack.kernelid} \text{ ?ssreg ?pt} \longrightarrow \\
& \text{context\_switching\_set\_stack\_segment\_registers !ssreg} \longrightarrow \\
& \text{context\_switching\_have\_set\_stack\_segment\_registers} \longrightarrow \\
& \text{context\_switching\_set\_page\_table !pt} \longrightarrow \\
& \text{context\_switching\_have\_set\_page\_table} \longrightarrow \\
& \text{kernel\_switched\_stack.kernelid} \longrightarrow \mathbf{Skip}
\end{aligned}$$

$$\text{ContextSwitching\_Kernel} \quad \hat{=} \quad \text{SwitchOut\_Kernel} \square \text{SwitchIn\_Kernel} \square \text{SwitchStack\_Kernel}$$

$$\text{ContextSwitching} \quad \hat{=} \quad \text{ContextSwitching\_IntHandler} \square \text{ContextSwitching\_Kernel}$$

$$\text{ExecContextSwitching} \quad \hat{=} \quad \mu X \bullet \text{ContextSwitching} ; X$$

$$\bullet \text{ module\_init} \longrightarrow \text{ExecContextSwitching} \Delta \text{ module\_end} \longrightarrow \mathbf{Skip}$$

**end**

## D.2.2 Memory Management

```

process MemoryManagement  $\hat{=}$ 
begin
state MEMORY_MANAGEMENT_STATE_TYPE

  Initialize  $\hat{=}$  kernel_init_memory_management ?areamm  $\longrightarrow$  InitMemoryManagement[areamm/areamm?];
               kernel_inited_memory_management  $\longrightarrow$  Skip

  SetAreaMemoryManagementRef  $\hat{=}$  kernel_set_area_memory_management_reference.kernelid ?areamm  $\longrightarrow$ 
                                   AreaMemoryManagementRef := areamm;
                                   kernel_have_set_area_memory_management_reference.kernelid  $\longrightarrow$  Skip

  GetAreaMemoryManagementRef  $\hat{=}$  kernel_request_area_memory_management_reference.kernelid  $\longrightarrow$ 
                                   kernel_get_area_memory_management_reference.kernelid
                                   !AreaMemoryManagementRef  $\longrightarrow$  Skip

  GetAreaFreePages  $\hat{=}$  kernel_request_area_free_pages.kernelid  $\longrightarrow$ 
                                   kernel_get_area_free_pages.kernelid !#(AreaMemoryManagementRef.Free)  $\longrightarrow$  Skip

  GetAreaFreeBlock  $\hat{=}$  var maxblock : MEMORY_BLOCK_TYPE •
                                   kernel_request_area_free_block.kernelid  $\longrightarrow$  GetMaxFreeBlock[maxblock/maxblock!];
                                   kernel_get_area_free_block.kernelid !(maxblock.Size)  $\longrightarrow$  Skip

  AllocAreaFreePage  $\hat{=}$  var pages :  $\mathbb{P}$  PAGE_TYPE •
                                   kernel_allocate_area_free_pages.kernelid ?n  $\longrightarrow$ 
                                   AllocPhysicalMemoryPage[n/n?, pages/pages!];
                                   kernel_allocated_area_free_pages.kernelid !pages  $\longrightarrow$  Skip

  AllocAreaFreeBlock  $\hat{=}$  var block : MEMORY_BLOCK_TYPE •
                                   kernel_allocate_area_free_block.kernelid ?size  $\longrightarrow$ 
                                   AllocPhysicalMemoryBlock[size/size?, block/block!];
                                   kernel_allocated_area_free_block.kernelid !block  $\longrightarrow$  Skip

  AllocAreaFreeSpace  $\hat{=}$  AllocAreaFreePage  $\square$  AllocAreaFreeBlock

  DeallocAreaUsedPage  $\hat{=}$  kernel_deallocate_area_used_pages.kernelid ?pages  $\longrightarrow$ 
                                   DeallocPhysicalMemoryPage[pages/pages?];
                                   kernel_deallocated_area_used_pages.kernelid  $\longrightarrow$  Skip

  DeallocAreaUsedBlock  $\hat{=}$  kernel_deallocate_area_used_block.kernelid ?block  $\longrightarrow$ 
                                   DeallocPhysicalMemoryPage[totalpage(block)/pages?];
                                   kernel_deallocated_area_used_block.kernelid  $\longrightarrow$  Skip

  DeallocAreaUsedSpace  $\hat{=}$  DeallocAreaUsedPage  $\square$  DeallocAreaUsedBlock

  CreateVirtualMemoryBlock  $\hat{=}$  var block : MEMORY_BLOCK_TYPE •
                                   kernel_create_virtual_memory_block.kernelid ?start ?size  $\longrightarrow$ 
                                   CreateMemoryBlock[start/start?, size/size?, block/block!];
                                   kernel_created_virtual_memory_block.kernelid !block  $\longrightarrow$  Skip

```

$\text{CreateProcVirtualMemory} \hat{=} \text{var } \text{block}, \text{stack}, \text{data}, \text{code} : \text{MEMORY\_BLOCK\_TYPE},$   
 $\text{procvm} : \text{PROCESS\_VIRTUAL\_MEMORY\_TYPE} \bullet$   
 $\text{kernel\_create\_process\_virtual\_memory.kernelid} \text{ ?base ?stacksize ?datasize}$   
 $\text{ ?codesize} \longrightarrow \text{CreateMemoryBlock}[(\text{PROCESS\_VIRTUAL\_ADDRESS\_SPACE.}$   
 $\text{Start})/\text{start?}, (\text{stacksize} + \text{datasize} + \text{codesize})/\text{size?}, \text{block}/\text{block!}];$   
 $\text{CreateMemoryBlock}[(\text{PROCESS\_VIRTUAL\_ADDRESS\_SPACE.Start})/\text{start?},$   
 $\text{stacksize}/\text{size?}, \text{stack}/\text{block!}];$   
 $\left( \begin{array}{l} \text{if } (\text{datasize} = 0) \longrightarrow \text{data} := \text{NULL\_BLOCK}; \\ \text{CreateMemoryBlock}[\text{nextpage}(\text{max}(\text{blockspace}(\text{stack}))) / \text{start?}, \text{codesize} / \\ \text{size?}, \text{code} / \text{block!}]; \\ \text{CreateProcessVirtualMemory}[\text{block} / \text{block?}, \text{base} / \text{base?}, \text{stack} / \text{stack?}, \text{data} / \\ \text{data?}, \text{code} / \text{code?}, \text{procvm} / \text{procvm!}]; \\ \text{kernel\_created\_process\_virtual\_memory.kernelid} \text{ !procvm} \longrightarrow \text{Skip} \\ \square (\text{datasize} \neq 0) \longrightarrow \\ \text{CreateMemoryBlock}[\text{nextpage}(\text{max}(\text{blockspace}(\text{stack}))) / \text{start?}, \text{datasize} / \\ \text{size?}, \text{data} / \text{block!}]; \\ \text{CreateMemoryBlock}[\text{nextpage}(\text{max}(\text{blockspace}(\text{data}))) / \text{start?}, \text{codesize} / \\ \text{size?}, \text{code} / \text{block!}]; \\ \text{CreateProcessVirtualMemory}[\text{block} / \text{block?}, \text{base} / \text{base?}, \text{stack} / \text{stack?}, \text{data} / \\ \text{data?}, \text{code} / \text{code?}, \text{procvm} / \text{procvm!}]; \\ \text{kernel\_created\_process\_virtual\_memory.kernelid} \text{ !procvm} \longrightarrow \text{Skip} \\ \text{fi} \end{array} \right)$

$\text{FullLoadProcPage} \hat{=} \text{var } \text{pagetable} : \text{PAGE\_TABLE\_TYPE}, \text{procpages} : \text{seq}[\text{PIECE\_TYPE}] \bullet$   
 $\text{kernel\_full\_load\_process\_pages.kernelid} \text{ ?procvm ?entrypoint ?exefile} \longrightarrow$   
 $\text{FullLoadProcPageTable}[\text{procvm} / \text{procvm?}, \text{entrypoint} / \text{entrypoint?}, \text{pagetable} / \text{pagetable!}];$   
 $\text{kernel\_full\_loaded\_process\_pages.kernelid} \text{ !pagetable} \longrightarrow$   
 $\text{pagetable} := \text{pagetable} \triangleleft \text{totalpage}(\text{procvm.Stack});$   
 $\text{procpages} := \text{slide}(\text{paging}(\text{exefile.Data}) \wedge \text{paging}(\text{exefile.Code}), \text{pagecount}(\text{procvm.Stack.}$   
 $\text{Size})); \text{LoadPages}(\text{pagetable}, \text{procpages})$

$\text{LoadPages} \hat{=} \text{pagetable} : \text{PAGE\_TABLE\_TYPE}, \text{procpages} : \text{seq}[\text{PIECE\_TYPE}] \bullet$   
 $\text{var } p : \text{PAGE\_TYPE}, i : \mathbb{N}_1 \bullet$   
 $(\text{pagetable} \neq \emptyset) \ \& \ p := \text{randompage}(\text{dom } \text{pagetable});$   
 $i := 1 + \text{bintounsigned}(p - \text{PROCESS\_VIRTUAL\_ADDRESS\_SPACE.Start}) \text{ div } \text{PAGE\_SIZE};$   
 $\text{memory\_management\_load\_page\_into\_main\_memory} \text{ !pagetable}(p) \text{ !procpages}(i) \longrightarrow$   
 $\text{memory\_management\_loaded\_page\_into\_main\_memory} \longrightarrow \text{LoadPages}(\{p\} \triangleleft \text{pagetable}, \text{procpages})$   
 $\square (\text{pagetable} = \emptyset) \ \& \ \text{Skip}$

$\text{MemoryManagementService} \hat{=} \text{SetAreaMemoryManagementRef}$   
 $\square \text{GetAreaMemoryManagementRef}$   
 $\square \text{GetAreaFreePages}$   
 $\square \text{GetAreaFreeBlock}$   
 $\square \text{AllocAreaFreeSpace}$   
 $\square \text{DeallocAreaUsedSpace}$   
 $\square \text{CreateVirtualMemoryBlock}$   
 $\square \text{CreateProcVirtualMemory}$   
 $\square \text{FullLoadProcPage}$

$\text{ExecMemoryManagementService} \hat{=} \mu X \bullet \text{MemoryManagementService} ; X$

$\bullet \text{module\_init} \longrightarrow (\text{Initialize} ; \text{ExecMemoryManagementService}) \Delta \text{module\_end} \longrightarrow \text{Skip}$

end



### D.2.3 System Clock

**process** *SystemClock*  $\hat{=}$

**begin**

**state** *SYSTEM\_CLOCK\_STATE\_TYPE*

*Initialize*  $\hat{=}$  *kernel\_init\_system\_clock*  $\longrightarrow$   
*system\_clock\_request\_current\_time*  $\longrightarrow$  *system\_clock\_get\_current\_time* ?*bt*  $\longrightarrow$   
*InitSystemClock*[*bintsigned*(*bt*)/*bt*?, *bintsigned*(*ClockTickInterval*)/*ti*?];  
*kernel\_inited\_system\_clock*  $\longrightarrow$  **Skip**

*GetTime*  $\hat{=}$  *kernel\_request\_system\_time.kernelid*  $\longrightarrow$   
*kernel\_get\_system\_time.kernelid* !*Time*  $\longrightarrow$  **Skip**

*GetHPTTime*  $\hat{=}$  *kernel\_request\_high\_precision\_time.kernelid*  $\longrightarrow$   
*system\_clock\_request\_high\_precision\_time*  $\longrightarrow$   
*system\_clock\_get\_high\_precision\_time* ?*hpt*  $\longrightarrow$   
*kernel\_get\_high\_precision\_time.kernelid* !*bintsigned*(*hpt*)  $\longrightarrow$  **Skip**

*ResetHPTimer*  $\hat{=}$  *kernel\_reset\_high\_precision\_timer.kernelid*  $\longrightarrow$   
*system\_clock\_reset\_high\_precision\_timer*  $\longrightarrow$   
*system\_clock\_have\_reset\_high\_precision\_timer*  $\longrightarrow$   
*kernel\_have\_reset\_high\_precision\_timer.kernelid*  $\longrightarrow$  **Skip**

*SetHPAlarm*  $\hat{=}$  *kernel\_set\_high\_precision\_timer\_alarm.kernelid* ?*a*  $\longrightarrow$   
*system\_clock\_set\_high\_precision\_timer\_alarm* !*signedtobin*(*a*)  $\longrightarrow$   
*system\_clock\_have\_set\_high\_precision\_timer\_alarm*  $\longrightarrow$   
*kernel\_have\_set\_high\_precision\_timer\_alarm.kernelid*  $\longrightarrow$  **Skip**

*EndHPTimer*  $\hat{=}$  *kernel\_end\_high\_precision\_timer.kernelid*  $\longrightarrow$   
*system\_clock\_end\_high\_precision\_timer*  $\longrightarrow$   
*system\_clock\_ended\_high\_precision\_timer*  $\longrightarrow$   
*kernel\_ended\_high\_precision\_timer.kernelid*  $\longrightarrow$  **Skip**

*UpdateTime*  $\hat{=}$  *isr\_clocktick\_update\_system\_time*  $\longrightarrow$  *UpdateSystemClock*;  
*isr\_clocktick\_updated\_system\_time*  $\longrightarrow$  **Skip**

*UpdateInterruptTime*  $\hat{=}$  *isr\_clocktick\_request\_high\_precision\_time*  $\longrightarrow$   
*system\_clock\_request\_high\_precision\_time*  $\longrightarrow$   
*system\_clock\_get\_high\_precision\_time* ?*hpt*  $\longrightarrow$  *InterruptTime* := *bintsigned*(*hpt*);  
*isr\_clocktick\_get\_high\_precision\_time* !*hpt*  $\longrightarrow$  **Skip**

*GetInterruptTime*  $\hat{=}$  *kernel\_request\_interrupt\_time.kernelid*  $\longrightarrow$   
*kernel\_get\_interrupt\_time.kernelid* !*InterruptTime*  $\longrightarrow$  **Skip**

*SystemClockService*  $\hat{=}$  *GetTime*  
 $\square$  *GetHPTTime*  
 $\square$  *ResetHPTimer*  
 $\square$  *SetHPAlarm*  
 $\square$  *EndHPTimer*  
 $\square$  *UpdateTime*  
 $\square$  *UpdateInterruptTime*  
 $\square$  *GetInterruptTime*

*ExecSystemClockService*  $\hat{=}$   $\mu X \bullet \text{SystemClockService} ; X$

- $module\_init \longrightarrow (Initialize ; ExecSystemClockService) \Delta module\_end \longrightarrow \mathbf{Skip}$

**end**





## D.2.4 Interrupt Controlling

**process** *InterruptControlling*  $\hat{=}$  ●  
**begin**

*Mask\_IntHandler*  $\hat{=}$  *interrupt\_handler\_mask\_interrupt* ?*i*  $\longrightarrow$   
*interrupt\_controlling\_mask\_interrupt* !*i*  $\longrightarrow$   
*interrupt\_controlling\_masked\_interrupt*  $\longrightarrow$   
*interrupt\_handler\_masked\_interrupt*  $\longrightarrow$  **Skip**

*Unmask\_IntHandler*  $\hat{=}$  *interrupt\_handler\_unmask\_interrupt* ?*i*  $\longrightarrow$   
*interrupt\_controlling\_unmask\_interrupt* !*i*  $\longrightarrow$   
*interrupt\_controlling\_unmasked\_interrupt*  $\longrightarrow$   
*interrupt\_handler\_unmasked\_interrupt*  $\longrightarrow$  **Skip**

*InterruptMaskService\_IntHandler*  $\hat{=}$  *Mask\_IntHandler*  $\square$  *Unmask\_IntHandler*

*Mask\_Kernel*  $\hat{=}$  *kernel\_mask\_interrupt.kernelid* ?*i*  $\longrightarrow$  *interrupt\_controlling\_mask\_interrupt* !*i*  $\longrightarrow$   
*interrupt\_controlling\_masked\_interrupt*  $\longrightarrow$  *kernel\_masked\_interrupt.kernelid*  $\longrightarrow$  **Skip**

*Unmask\_Kernel*  $\hat{=}$  *kernel\_unmask\_interrupt.kernelid* ?*i*  $\longrightarrow$  *interrupt\_controlling\_unmask\_interrupt* !*i*  $\longrightarrow$   
*interrupt\_controlling\_unmasked\_interrupt*  $\longrightarrow$  *kernel\_unmasked\_interrupt.kernelid*  $\longrightarrow$  **Skip**

*InterruptMaskService\_Kernel*  $\hat{=}$  *Mask\_Kernel*  $\square$  *Unmask\_Kernel*

*InterruptMaskService*  $\hat{=}$  *InterruptMaskService\_IntHandler*  $\square$  *InterruptMaskService\_Kernel*

*ExecInterruptMaskService*  $\hat{=}$   $\mu X \bullet \text{InterruptMaskService} ; X$

*Enable\_IntHandler*  $\hat{=}$  *interrupt\_handler\_enable\_interrupt*  $\longrightarrow$   
*interrupt\_controlling\_enable\_interrupt*  $\longrightarrow$   
*interrupt\_controlling\_enabled\_interrupt*  $\longrightarrow$   
*interrupt\_handler\_enabled\_interrupt*  $\longrightarrow$  **Skip**

*Disable\_IntHandler*  $\hat{=}$  *interrupt\_handler\_disable\_interrupt*  $\longrightarrow$   
*interrupt\_controlling\_disable\_interrupt*  $\longrightarrow$   
*interrupt\_controlling\_disabled\_interrupt*  $\longrightarrow$   
*interrupt\_handler\_disabled\_interrupt*  $\longrightarrow$  **Skip**

*InterruptEnableService\_IntHandler*  $\hat{=}$  *Enable\_IntHandler*  $\square$  *Disable\_IntHandler*

*Enable\_Kernel*  $\hat{=}$  *kernel\_enable\_interrupt.kernelid*  $\longrightarrow$  *interrupt\_controlling\_enable\_interrupt*  $\longrightarrow$   
*interrupt\_controlling\_enabled\_interrupt*  $\longrightarrow$  *kernel\_enabled\_interrupt.kernelid*  $\longrightarrow$  **Skip**

*Disable\_Kernel*  $\hat{=}$  *kernel\_disable\_interrupt.kernelid*  $\longrightarrow$  *interrupt\_controlling\_disable\_interrupt*  $\longrightarrow$   
*interrupt\_controlling\_disabled\_interrupt*  $\longrightarrow$  *kernel\_disabled\_interrupt.kernelid*  $\longrightarrow$  **Skip**

*InterruptEnableService\_Kernel*  $\hat{=}$  *Enable\_Kernel*  $\square$  *Disable\_Kernel*

*InterruptEnableService*  $\hat{=}$  *InterruptEnableService\_IntHandler*  $\square$  *InterruptEnableService\_Kernel*

*ExecInterruptEnableService*  $\hat{=}$   $\mu X \bullet \text{InterruptEnableService} ; X$

*ExecInterruptControlling*  $\hat{=}$  *ExecInterruptMaskService*  $\parallel \parallel$  *ExecInterruptEnableService*

● *module\_init*  $\longrightarrow$  *ExecInterruptControlling*  $\Delta$  *module\_end*  $\longrightarrow$  **Skip**

**end**

### D.2.5 ChannelSets for communication within Interrupt Handler

```
channelset SelectISR    ==  { interrupt_handler_invoke_service_routine_clocktick }  
channelset ISRReturn  ==  { interrupt_service_routine_end }
```

## D.2.6 Interrupt Handler

**process** *InterruptHandler*  $\hat{=}$  *IntHandlerConfig* : *INTERRUPT\_HANDLER\_CONFIG\_TYPE* •  
**begin**  
**state** *INTERRUPT\_HANDLER\_STATE\_TYPE*

*Initialize*  $\hat{=}$  *kernel\_init\_interrupt\_handler* ?*pagetable*  $\longrightarrow$   
*interrupt\_handler\_request\_interrupt\_stack* !(*IntHandlerConfig*.*InterruptStackSize*)  $\longrightarrow$   
*interrupt\_handler\_get\_interrupt\_stack* ?*intstack*  $\longrightarrow$   
*InitInterruptHandler*[*intstack*/*intstack*?, *pagetable*/*pagetable*?];  
*kernel\_inited\_interrupt\_handler*  $\longrightarrow$  **Skip**

*InterruptHandle\_Pre*  $\hat{=}$  **var** *ssreg* : *SSREGISTER\_TYPE* •  
*interrupt\_handler\_start\_interrupt\_handling* ?*i*  $\longrightarrow$   
*interrupt\_handler\_disable\_interrupt*  $\longrightarrow$  *interrupt\_handler\_disabled\_interrupt*  $\longrightarrow$   
*interrupt\_handler\_save\_context*  $\longrightarrow$  *interrupt\_handler\_saved\_context* ?*cpureg* ?*pt*  $\longrightarrow$   
*TempContext* := (makecontext(*cpureg*, *pt*))  $\wedge$  *TempContext*;  
 $\left( \begin{array}{l} \text{if } ((\text{first } (\text{head } \text{TempContext})).\text{SSRegister}.\text{SS} \neq \text{InterruptStack}.\text{Start}) \longrightarrow \\ \quad \text{CreateStackSegment}[(\text{InterruptStack}.\text{Start})/\text{ss?}, \text{unsignedtobin}(\text{InterruptStack}.\text{Size})/\text{sl?}, 0_{PSU}/\text{bp?}, 0_{PSU}/\text{sp?}, \text{ssreg}/\text{ssreg!}]; \\ \quad \text{interrupt\_handler\_switch\_stack } !\text{ssreg } !\text{KernelPageTableRef} \longrightarrow \\ \quad \text{interrupt\_handler\_switched\_stack} \longrightarrow \\ \quad \text{interrupt\_handler\_enable\_interrupt} \longrightarrow \\ \quad \text{interrupt\_handler\_enabled\_interrupt} \longrightarrow \text{SelectInterruptServiceRoutine}(i) \\ \quad \square \\ \quad ((\text{first } (\text{head } \text{TempContext})).\text{SSRegister}.\text{SS} = \text{InterruptStack}.\text{Start}) \longrightarrow \\ \quad \quad \text{CreateStackSegment}[(\text{InterruptStack}.\text{Start})/\text{ss?}, \text{unsignedtobin}(\text{InterruptStack}.\text{Size})/\text{sl?}, (\text{cpureg}.\text{SSRegister}.\text{SP} + 1_{PSU})/\text{bp?}, (\text{cpureg}.\text{SSRegister}.\text{SP} + 1_{PSU})/\text{sp?}, \text{ssreg}/\text{ssreg!}]; \\ \quad \quad \text{interrupt\_handler\_switch\_stack } !\text{ssreg } !\text{KernelPageTableRef} \longrightarrow \\ \quad \quad \text{interrupt\_handler\_switched\_stack} \longrightarrow \\ \quad \quad \text{interrupt\_handler\_enable\_interrupt} \longrightarrow \\ \quad \quad \text{interrupt\_handler\_enabled\_interrupt} \longrightarrow \text{SelectInterruptServiceRoutine}(i) \\ \text{fi} \end{array} \right)$

*SelectInterruptServiceRoutine*  $\hat{=}$  *i* : *INTERRUPT\_TYPE* •  
(*i* = *CLOCK\_TICK*) & *interrupt\_handler\_invoke\_service\_routine\_clocktick*  $\longrightarrow$   
**Skip**

*ISR\_ClockTick*  $\hat{=}$  *interrupt\_handler\_invoke\_service\_routine\_clocktick*  $\longrightarrow$   
*isr\_clocktick\_request\_high\_precision\_time*  $\longrightarrow$   
*isr\_clocktick\_get\_high\_precision\_time* ?*hpt*  $\longrightarrow$   
 $\left( \begin{array}{l} \text{if } (\text{hpt mod ClockTickInterval} \neq 0_{PSU}) \longrightarrow \\ \quad \text{interrupt\_service\_routine\_end } !\text{CLOCK\_TICK} \longrightarrow \text{Skip} \\ \quad \square \\ \quad (\text{hpt mod ClockTickInterval} = 0_{PSU}) \longrightarrow \\ \quad \quad \text{isr\_clocktick\_update\_system\_time} \longrightarrow \\ \quad \quad \text{isr\_clocktick\_updated\_system\_time} \longrightarrow \\ \quad \quad \text{interrupt\_service\_routine\_end } !\text{CLOCK\_TICK} \longrightarrow \text{Skip} \\ \text{fi} \end{array} \right)$

$InterruptServiceRoutines \hat{=} ISR\_ClockTick$

$InterruptHandle\_Pro \hat{=} interrupt\_service\_routine\_end ?i \longrightarrow$   
 $interrupt\_handler\_disable\_interrupt \longrightarrow interrupt\_handler\_disabled\_interrupt \longrightarrow$   
 $interrupt\_handler\_finish\_interrupt\_handling !i \longrightarrow$   
 $\left( \begin{array}{l} \text{if } (\# TempContext > 1) \longrightarrow \\ \quad interrupt\_handler\_restore\_context \\ \quad !(first (head TempContext)) !(second (head TempContext)) \longrightarrow \\ \quad interrupt\_handler\_restored\_context \longrightarrow TempContext := tail TempContext; \\ \quad interrupt\_handler\_enable\_interrupt \longrightarrow \\ \quad interrupt\_handler\_enabled\_interrupt \longrightarrow \mathbf{Skip} \\ \quad \square (\# TempContext = 1) \longrightarrow \\ \quad \quad interrupt\_handler\_invoke\_kernel \longrightarrow \\ \quad \quad \left( \begin{array}{l} kernel\_continue\_interrupted\_process.kernelid \longrightarrow \\ \quad interrupt\_handler\_restore\_context !(first (head TempContext)) !(second \\ \quad (head TempContext)) \longrightarrow interrupt\_handler\_restored\_context \longrightarrow \\ \quad TempContext := tail TempContext; \\ \quad interrupt\_handler\_enable\_interrupt \longrightarrow \\ \quad interrupt\_handler\_enabled\_interrupt \longrightarrow \mathbf{Skip} \end{array} \right) \\ \quad \square \left( \begin{array}{l} kernel\_request\_interrupted\_process\_context.kernelid \longrightarrow \\ \quad kernel\_get\_interrupted\_process\_context.kernelid \\ \quad !(first (head TempContext)) !(second (head TempContext)) \longrightarrow \\ \quad TempContext := tail TempContext \end{array} \right) \\ \text{fi} \end{array} \right)$

$InterruptHandle \hat{=} (InterruptHandle\_Pre \llbracket SelectISR \rrbracket InterruptServiceRoutines \llbracket ISRReturn \rrbracket$   
 $InterruptHandle\_Pro)$   
 $\square (InterruptHandle\_Pre \llbracket SelectISR \rrbracket InterruptServiceRoutines \llbracket ISRReturn \rrbracket$   
 $InterruptHandle\_Pro) \Delta InterruptHandle$

$ExecInterruptHandle \hat{=} \mu X \bullet InterruptHandle ; X$

$\bullet module\_init \longrightarrow (Initialize ; ExecInterruptHandle) \Delta module\_end \longrightarrow \mathbf{Skip}$

end

## D.2.7 ChannelSets for communication between different parts of Hardware Interface Software Layer

$channelset IH\_CS == \{ interrupt\_handler\_save\_context, interrupt\_handler\_saved\_context,$   
 $interrupt\_handler\_restore\_context, interrupt\_handler\_restored\_context,$   
 $interrupt\_handler\_switch\_stack, interrupt\_handler\_switched\_stack \}$   
 $channelset IH\_CLOCK == \{ isr\_clocktick\_update\_system\_time, isr\_clocktick\_updated\_system\_time,$   
 $isr\_clocktick\_request\_high\_precision\_time, isr\_clocktick\_get\_high\_precision\_time \}$   
 $channelset IH\_IC == \{ interrupt\_handler\_mask\_interrupt, interrupt\_handler\_masked\_interrupt,$   
 $interrupt\_handler\_unmask\_interrupt, interrupt\_handler\_unmasked\_interrupt,$   
 $interrupt\_handler\_enable\_interrupt, interrupt\_handler\_enabled\_interrupt,$   
 $interrupt\_handler\_disable\_interrupt, interrupt\_handler\_disabled\_interrupt \}$   
 $channelset HISLayerChannels == IH\_CS \cup IH\_CLOCK \cup IH\_IC$

## D.2.8 Hardware Interface Software Layer Model

**process** *Hardware\_Interface\_Software\_Layer*  $\hat{=}$  *IntHandlerConfig* : *INTERRUPT\_HANDLER\_CONFIG\_TYPE* •

( *ContextSwitching*  $\llbracket$  *HISLayerChannels*  $\rrbracket$  *SystemClock*  $\llbracket$  *HISLayerChannels*  $\rrbracket$  *InterruptControlling*  
 $\llbracket$  *HISLayerChannels*  $\rrbracket$  *InterruptHandler(IntHandlerConfig)*  $\parallel$  *MemoryManagement*



## D.3 ARINC 653 O/S Layer

### D.3.1 Core Kernel

**process** *CoreKernel*  $\hat{=}$  *OSKernelConfig* : *OS\_KERNEL\_CONFIG\_TYPE* •

**begin**

**state** *CORE\_KERNEL\_STATE\_TYPE*

*Initialize\_CoreKernel*  $\hat{=}$  *InitCoreKernel*[*OSKernelConfig*/config?]

*Initialize\_PartitionKernels*  $\hat{=}$   $\parallel \parallel \parallel$  *partid* : *dom*(*PartitionManagement.PartitionTable*) •  
*core\_kernel\_init\_partition\_kernel.partid* !*KernelPageTable*  $\longrightarrow$   
*core\_kernel\_init\_partition\_kernel.partid*  $\longrightarrow$  **Skip**

*Initialize\_MemoryManagement*  $\hat{=}$  *kernel\_init\_memory\_management* !*MemoryManagement*  $\longrightarrow$   
*kernel\_init\_memory\_management*  $\longrightarrow$  **Skip**

*Initialize\_InterruptHandler*  $\hat{=}$  *kernel\_init\_interrupt\_handler* !*KernelPageTable*  $\longrightarrow$   
*interrupt\_handler\_request\_interrupt\_stack* ?*size*  $\longrightarrow$   
*kernel\_allocate\_area\_free\_block.CORE\_KERNEL* !*size*  $\longrightarrow$   
*kernel\_allocated\_area\_free\_block.CORE\_KERNEL* ?*block*  $\longrightarrow$   
*kernel\_create\_virtual\_memory\_block.CORE\_KERNEL*  
!(*KernelPageTable*  $\sim$  (*block.Start*)) !*size*  $\longrightarrow$   
*kernel\_created\_virtual\_memory\_block.CORE\_KERNEL* ?*intstack*  $\longrightarrow$   
*interrupt\_handler\_get\_interrupt\_stack* !*intstack*  $\longrightarrow$   
*kernel\_init\_interrupt\_handler*  $\longrightarrow$  **Skip**

*Initialize\_SystemClock*  $\hat{=}$  *kernel\_init\_system\_clock*  $\longrightarrow$  *kernel\_init\_system\_clock*  $\longrightarrow$  **Skip**

*Initialize*  $\hat{=}$  *Initialize\_CoreKernel* ; *Initialize\_PartitionKernels* ; *Initialize\_MemoryManagement* ;  
*Initialize\_InterruptHandler* ; *Initialize\_SystemClock*

*StartPartitionKernel*  $\hat{=}$   $\parallel \parallel \parallel$  *partid* : *dom*(*PartitionManagement.PartitionTable*) •  
*PartitionManagement.PartitionTable*(*partid*).*OperatingMode* = *COLD\_START* ;  
*PartitionManagement.PartitionTable*(*partid*).*LockLevel* = *MAX\_LOCK\_LEVEL*

*StartCoreKernel*  $\hat{=}$  *KernelProcManagement.CurrentProcess* := *IDLE\_PROCESS\_ID* ;  
*kernel\_restore\_context.CORE\_KERNEL* !*ALL* !(*first* (*head KernelProcManagement.ProcessTable*(*KernelProcManagement.CurrentProcess*).*KernelTempContext*))  
!(*second* (*head KernelProcManagement.ProcessTable*(*KernelProcManagement.CurrentProcess*).*KernelTempContext*))  $\longrightarrow$   
*kernel\_restored\_context.CORE\_KERNEL*  $\longrightarrow$   
*KernelProcManagement.ProcessTable*(*KernelProcManagement.CurrentProcess*).  
*KernelTempContext* :=  
*tail KernelProcManagement.ProcessTable*(*KernelProcManagement.CurrentProcess*).  
*KernelTempContext* ;  
*kernel\_enable\_interrupt.CORE\_KERNEL*  $\longrightarrow$   
*kernel\_enabled\_interrupt.CORE\_KERNEL*  $\longrightarrow$   
*KernelProcManagement.ProcessTable*(*KernelProcManagement.CurrentProcess*).  
*ProcessState* := *RUNNING*

*Start*  $\hat{=}$  *StartPartitionKernel* ; *StartCoreKernel*

$Lock \hat{=} kernel\_disable\_interrupt.CORE\_KERNEL \longrightarrow kernel\_disabled\_interrupt.CORE\_KERNEL \longrightarrow \mathbf{Skip}$   
 $Unlock \hat{=} kernel\_enable\_interrupt.CORE\_KERNEL \longrightarrow kernel\_enabled\_interrupt.CORE\_KERNEL \longrightarrow \mathbf{Skip}$   
 $Core\_GetOperatingMode \hat{=} \mathbf{var} \, om : OPERATING\_MODE\_TYPE \bullet$   
 $\quad core\_kernel\_service\_get\_operating\_mode.partid \longrightarrow$   
 $\quad om := PartitionManagement.PartitionTable(partid).OperatingMode;$   
 $\quad core\_kernel\_service\_get\_operating\_mode\_output.partid !om \longrightarrow$   
 $\quad core\_kernel\_service\_get\_operating\_mode\_return.partid \longrightarrow \mathbf{Skip}$   
 $Core\_GetPartitionStatus \hat{=} \mathbf{var} \, parts : PARTITION\_STATUS\_TYPE \bullet$   
 $\quad core\_kernel\_service\_get\_partition\_status.partid \longrightarrow$   
 $\quad GetPartitionStatus[parts / parts!];$   
 $\quad core\_kernel\_service\_get\_partition\_status\_output.partid !parts \longrightarrow$   
 $\quad core\_kernel\_service\_get\_partition\_status\_return.partid \longrightarrow \mathbf{Skip}$   
 $Core\_SetOperatingMode \hat{=} core\_kernel\_service\_set\_operating\_mode.partid \longrightarrow$   
 $\quad core\_kernel\_service\_set\_operating\_mode\_input.partid ?om \longrightarrow$   
 $\quad PartitionManagement.PartitionTable(partid).OperatingMode := om;$   
 $\quad \left( \begin{array}{l} \mathbf{if} \, (om = IDLE \vee om = NORMAL) \longrightarrow \\ \quad PartitionManagement.PartitionTable(partid).LockLevel := MIN\_ \\ \quad LOCK\_LEVEL; \\ \quad core\_kernel\_service\_set\_operating\_mode\_return.partid \longrightarrow \mathbf{Skip} \\ \quad \parallel \\ \quad (om = COLD\_START \vee om = WARM\_START) \longrightarrow \\ \quad PartitionManagement.PartitionTable(partid).LockLevel := MAX\_ \\ \quad LOCK\_LEVEL; \\ \quad core\_kernel\_service\_set\_operating\_mode\_return.partid \longrightarrow \mathbf{Skip} \\ \mathbf{fi} \end{array} \right)$



$Core\_GetNextPeriodicStart \hat{=} \text{var } ct, nps : SYSTEM\_TIME\_TYPE \bullet$   
 $\text{core\_kernel\_service\_get\_next\_periodic\_start.partid} \longrightarrow$   
 $Lock;$   
 $\text{kernel\_request\_system\_time.CORE\_KERNEL} \longrightarrow$   
 $\text{kernel\_get\_system\_time.CORE\_KERNEL } ?t \longrightarrow$   
 $\text{kernel\_request\_high\_precision\_time.CORE\_KERNEL} \longrightarrow$   
 $\text{kernel\_get\_high\_precision\_time.CORE\_KERNEL } ?hpt \longrightarrow$   
 $ct := t + hpt \bmod \text{bintolsigned}(ClockTickInterval);$   
 $Unlock;$   
 $GetNextPeriodicStart[ct/ct?, nps/nps!];$   
 $\text{core\_kernel\_service\_get\_next\_periodic\_start\_output.partid } !nps \longrightarrow$   
 $\text{core\_kernel\_service\_get\_next\_periodic\_start\_return.partid} \longrightarrow \text{Skip}$

$Core\_GetDelayedPeriodicStart \hat{=} \text{var } ct, dps : SYSTEM\_TIME\_TYPE \bullet$   
 $\text{core\_kernel\_service\_get\_delayed\_periodic\_start.partid} \longrightarrow$   
 $\text{core\_kernel\_service\_get\_delayed\_periodic\_start\_input.partid } ?dt \longrightarrow$   
 $Lock;$   
 $\text{kernel\_request\_system\_time.CORE\_KERNEL} \longrightarrow$   
 $\text{kernel\_get\_system\_time.CORE\_KERNEL } ?t \longrightarrow$   
 $\text{kernel\_request\_high\_precision\_time.CORE\_KERNEL} \longrightarrow$   
 $\text{kernel\_get\_high\_precision\_time.CORE\_KERNEL } ?hpt \longrightarrow$   
 $ct := t + hpt \bmod \text{bintolsigned}(ClockTickInterval);$   
 $Unlock;$   
 $GetDelayedPeriodicStart[ct/ct?, dt/dt?, nps/nps!];$   
 $\text{core\_kernel\_service\_get\_delayed\_periodic\_start\_output.partid } !dps \longrightarrow$   
 $\text{core\_kernel\_service\_get\_delayed\_periodic\_start\_return.partid} \longrightarrow \text{Skip}$

$Core\_GetLockLevel \hat{=} \text{var } ll : LOCK\_LEVEL\_TYPE \bullet$   
 $\text{core\_kernel\_service\_get\_lock\_level.partid} \longrightarrow$   
 $ll := \text{PartitionManagement.PartitionTable(partid).LockLevel};$   
 $\text{core\_kernel\_service\_get\_lock\_level\_output.partid } !ll \longrightarrow$   
 $\text{core\_kernel\_service\_get\_lock\_level\_return.partid} \longrightarrow \text{Skip}$

$Core\_ResetLockLevel \hat{=} \text{core\_kernel\_service\_reset\_lock\_level.partid} \longrightarrow$   
 $\text{PartitionManagement.PartitionTable(partid).LockLevel} := \text{MIN\_LOCK\_LEVEL};$   
 $\text{core\_kernel\_service\_reset\_lock\_level\_return.partid} \longrightarrow \text{Skip}$

$Core\_IncreaseLockLevel \hat{=} \text{core\_kernel\_service\_increase\_lock\_level.partid} \longrightarrow$   
 $\text{PartitionManagement.PartitionTable(partid).LockLevel} :=$   
 $\text{PartitionManagement.PartitionTable(partid).LockLevel} + 1;$   
 $\text{core\_kernel\_service\_increase\_lock\_level\_return.partid} \longrightarrow \text{Skip}$

$Core\_DecreaseLockLevel \hat{=} \text{core\_kernel\_service\_decrease\_lock\_level.partid} \longrightarrow$   
 $\text{PartitionManagement.PartitionTable(partid).LockLevel} :=$   
 $\text{PartitionManagement.PartitionTable(partid).LockLevel} - 1;$   
 $\text{core\_kernel\_service\_decrease\_lock\_level\_return.partid} \longrightarrow \text{Skip}$

$CoreKernelService \hat{=} Core\_GetOperatingMode$   
 $\square Core\_GetPartitionStatus$   
 $\square Core\_SetOperatingMode$   
 $\square Core\_GetNextPeriodicStart$   
 $\square Core\_GetDelayedPeriodicStart$   
 $\square Core\_GetLockLevel$   
 $\square Core\_ResetLockLevel$   
 $\square Core\_IncreaseLockLevel$   
 $\square Core\_DecreaseLockLevel$

$ExecCoreKernelService \hat{=} \parallel \parallel \text{partid} : \text{dom}(\text{PartitionManagement.PartitionTable}) \bullet (\mu X \bullet CoreKernelService ; X)$

$PartitionScheduler \hat{=} \text{var } partid : PARTITION\_ID\_TYPE \bullet$   
 $interrupt\_handler\_invoke\_kernel \longrightarrow kernel\_request\_system\_time.CORE\_KERNEL \longrightarrow$   
 $kernel\_get\_system\_time.CORE\_KERNEL ? t \longrightarrow GetNextPartition[t/t?, partid/partid!];$   
 $\left( \begin{array}{l} \text{if } (partid = PartitionManagement.CurrentPartition) \longrightarrow \\ \quad \left( \begin{array}{l} \text{if } (PartitionManagement.CurrentPartition = NULL\_PARTITION\_ID) \\ \longrightarrow \\ kernel\_continue\_interrupted\_process.CORE\_KERNEL \longrightarrow \text{Skip} \\ \square (PartitionManagement.CurrentPartition \neq NULL\_PARTITION\_ID) \\ \longrightarrow \\ partition\_kernel\_continue\_execution.(PartitionManagement. \\ CurrentPartition) \longrightarrow \text{Skip} \end{array} \right) \\ \text{fi} \\ \square (partid \neq PartitionManagement.CurrentPartition) \longrightarrow \\ \quad \left( \begin{array}{l} \text{if } (PartitionManagement.CurrentPartition = NULL\_PARTITION\_ID) \\ \longrightarrow \\ SuspendCoreKernelProcess; \\ PartitionManagement.CurrentPartition := partid; \\ ExecuteCurrentPartition(t) \\ \square (partid = NULL\_PARTITION\_ID) \longrightarrow \\ SuspendCurrentPartition; \\ PartitionManagement.CurrentPartition := partid; \\ ResumeCoreKernelProcess \\ \square (PartitionManagement.CurrentPartition \neq NULL\_PARTITION\_ID \\ \wedge partid \neq NULL\_PARTITION\_ID) \longrightarrow \\ SuspendCurrentPartition; \\ PartitionManagement.CurrentPartition := partid; \\ ExecuteCurrentPartition(t) \\ \text{fi} \end{array} \right) \end{array} \right)$   
 $\text{fi}$

$SuspendCoreKernelProcess \hat{=} kernel\_request\_interrupted\_process\_context.CORE\_KERNEL \longrightarrow$   
 $kernel\_get\_interrupted\_process\_context.CORE\_KERNEL ? cpureg ? pt \longrightarrow$   
 $KernelProcManagement.ProcessTable(KernelProcManagement.CurrentProcess).$   
 $KernelTempContext := \langle makecontext(cpureg, pt) \rangle \wedge KernelProcManagement.$   
 $ProcessTable(KernelProcManagement.CurrentProcess).KernelTempContext;$   
 $kernel\_request\_area\_memory\_management\_reference.CORE\_KERNEL \longrightarrow$   
 $kernel\_get\_area\_memory\_management\_reference.CORE\_KERNEL ? areamm \longrightarrow$   
 $MemoryManagement := areamm$

$ResumeCoreKernelProcess \hat{=} kernel\_set\_area\_memory\_management\_reference.CORE\_KERNEL$   
 $!MemoryManagement \longrightarrow$   
 $kernel\_have\_set\_area\_memory\_management\_reference.CORE\_KERNEL \longrightarrow$   
 $kernel\_restore\_context.CORE\_KERNEL !ALL !(first (head KernelProcManagement.$   
 $ProcessTable(KernelProcManagement.CurrentProcess).KernelTempContext))$   
 $!(second (head KernelProcManagement.ProcessTable(KernelProcManagement.$   
 $CurrentProcess).KernelTempContext)) \longrightarrow$   
 $kernel\_restored\_context.CORE\_KERNEL \longrightarrow$   
 $KernelProcManagement.ProcessTable(KernelProcManagement.CurrentProcess).$   
 $KernelTempContext :=$   
 $tail KernelProcManagement.ProcessTable(KernelProcManagement.CurrentProcess).$   
 $KernelTempContext;$   
 $kernel\_enable\_interrupt.CORE\_KERNEL \longrightarrow$   
 $kernel\_enabled\_interrupt.CORE\_KERNEL \longrightarrow \text{Skip}$

*SuspendCurrentPartition*  $\hat{=}$  *partition\_kernel\_suspend\_execution*.(*PartitionManagement.CurrentPartition*)  $\longrightarrow$   
*partition\_kernel\_suspended\_execution*.(*PartitionManagement.CurrentPartition*)  $\longrightarrow$   
**Skip**

*ExecuteCurrentPartition*  $\hat{=}$   $t : \text{SYSTEM\_TIME\_TYPE} \bullet$   
(*PartitionManagement.PartitionTable*(*PartitionManagement.CurrentPartition*).  
*OperatingMode* = *IDLE*) &  
*partition\_kernel\_idle\_execution*.(*PartitionManagement.CurrentPartition*)  $\longrightarrow$   
**Skip**  
(*PartitionManagement.PartitionTable*(*PartitionManagement.CurrentPartition*).  
*OperatingMode*  $\in \{ \text{WARM\_START}, \text{COLD\_START} \}$ ) &  
*partition\_kernel\_prepare\_execution*.(*PartitionManagement.CurrentPartition*)  $\longrightarrow$   
**Skip**  
(*PartitionManagement.PartitionTable*(*PartitionManagement.CurrentPartition*).  
*OperatingMode* = *NORMAL*) &  
*partition\_kernel\_update\_system\_time*.(*PartitionManagement.CurrentPartition*)  
! $t \longrightarrow$   
*partition\_kernel\_start\_execution*.(*PartitionManagement.CurrentPartition*)  $\longrightarrow$   
**Skip**

*ExecPartitionScheduler*  $\hat{=}$   $\mu X \bullet \text{PartitionScheduler} ; X$

$\bullet \text{ module\_init} \longrightarrow (\text{Initialize} ; \text{Start} ; (\text{ExecCoreKernelService} \parallel \text{ExecPartitionScheduler})) \Delta \text{ module\_end} \longrightarrow \text{Skip}$

**end**

### D.3.2 ChannelSets for communication within Partition Kernel

```
channelset SelectSysCall == { system_call_handler_invoke_service_routine_get_operating_mode,
                             system_call_handler_invoke_service_routine_get_partition_status,
                             system_call_handler_invoke_service_routine_set_operating_mode,
                             system_call_handler_invoke_service_routine_get_process_names,
                             system_call_handler_invoke_service_routine_get_process_ids,
                             system_call_handler_invoke_service_routine_get_free_process_ids,
                             system_call_handler_invoke_service_routine_get_free_space,
                             system_call_handler_invoke_service_routine_get_partition_period,
                             system_call_handler_invoke_service_routine_get_process_state,
                             system_call_handler_invoke_service_routine_get_next_periodic_start,
                             system_call_handler_invoke_service_routine_get_delayed_periodic_start,
                             system_call_handler_invoke_service_routine_get_process_kind,
                             system_call_handler_invoke_service_routine_get_process_period,
                             system_call_handler_invoke_service_routine_get_process_time_capacity,
                             system_call_handler_invoke_service_routine_get_partition_lock_level,
                             system_call_handler_invoke_service_routine_get_process_id,
                             system_call_handler_invoke_service_routine_get_process_status,
                             system_call_handler_invoke_service_routine_create_process,
                             system_call_handler_invoke_service_routine_set_priority,
                             system_call_handler_invoke_service_routine_suspend_self,
                             system_call_handler_invoke_service_routine_suspend,
                             system_call_handler_invoke_service_routine_resume,
                             system_call_handler_invoke_service_routine_stop_self,
                             system_call_handler_invoke_service_routine_stop,
                             system_call_handler_invoke_service_routine_start,
                             system_call_handler_invoke_service_routine_delayed_start,
                             system_call_handler_invoke_service_routine_lock_preemption,
                             system_call_handler_invoke_service_routine_unlock_preemption,
                             system_call_handler_invoke_service_routine_get_my_id,
                             system_call_handler_invoke_service_routine_get_current_time,
                             system_call_handler_invoke_service_routine_get_partition_time,
                             system_call_handler_invoke_service_routine_get_next_release_point,
                             system_call_handler_invoke_service_routine_timed_wait,
                             system_call_handler_invoke_service_routine_periodic_wait,
                             system_call_handler_invoke_service_routine_get_time,
                             system_call_handler_invoke_service_routine_replenish }

channelset SysCallReturn == { system_call_service_routine_end }
```

### D.3.3 Partition Kernel

```

process PartitionKernel  $\hat{=}$  PartitionId : PARTITION_ID_TYPE;
                               PartitionConfig : PARTITION_KERNEL_CONFIG_TYPE •
begin
state PARTITION_KERNEL_STATE_TYPE

Initialize  $\hat{=}$  core_kernel_init_partition_kernel.PartitionId ?pagetable  $\longrightarrow$ 
               InitPartitionKernel[PartitionConfig/config?, pagetable/pagetable?];
               core_kernel_init_partition_kernel.PartitionId  $\longrightarrow$  Skip

Lock  $\hat{=}$  kernel_disable_interrupt.PartitionId  $\longrightarrow$  kernel_disabled_interrupt.PartitionId  $\longrightarrow$  Skip

Unlock  $\hat{=}$  kernel_enable_interrupt.PartitionId  $\longrightarrow$  kernel_enabled_interrupt.PartitionId  $\longrightarrow$  Skip

AddTimeCounter  $\hat{=}$  procid : PROCESS_ID_TYPE, alarm : SYSTEM_TIME_TYPE,
                  om : OPERATING_MODE_TYPE •
                  var tc : TIME_COUNTER_TYPE •
                  CreateTimeCounter[procid/procid?, alarm/alarm?, tc/tc!];
                  EnqTimeCounterQueue[tc/tc?];
                   $\left( \begin{array}{l} \text{if } (om \neq \text{NORMAL} \vee tc \neq \text{head TimeCounterQueue}) \longrightarrow \text{Skip} \\ \quad \square \quad (om = \text{NORMAL} \wedge tc = \text{head TimeCounterQueue}) \longrightarrow \\ \quad \quad \text{Lock;} \\ \quad \quad \text{kernel\_set\_high\_precision\_timer\_alarm.PartitionId} \\ \quad \quad \text{!(tc.Alarm)} \longrightarrow \\ \quad \quad \text{kernel\_have\_set\_high\_precision\_timer\_alarm.PartitionId} \longrightarrow \\ \quad \quad \text{Unlock} \\ \text{fi} \end{array} \right)$ 

RemoveTimeCounter  $\hat{=}$  procid : PROCESS_ID_TYPE, om : OPERATING_MODE_TYPE •
                  var alarm : SYSTEM_TIME_TYPE •
                  GetTimingProcessAlarm[procid/procid?, alarm, alarm!];
                  DeqTimeCounterQueue[procid/procid?];
                   $\left( \begin{array}{l} \text{if } (om \neq \text{NORMAL} \vee \text{alarm} \geq (\text{head TimeCounterQueue}). \\ \quad \text{Alarm}) \longrightarrow \text{Skip} \\ \quad \square \quad (om = \text{NORMAL} \wedge \text{alarm} < (\text{head TimeCounterQueue}). \\ \quad \quad \text{Alarm}) \longrightarrow \\ \quad \quad \text{Lock;} \\ \quad \quad \text{kernel\_set\_high\_precision\_timer\_alarm.PartitionId ! | (head} \\ \quad \quad \text{TimeCounterQueue).Alarm |} \longrightarrow \\ \quad \quad \text{kernel\_have\_set\_high\_precision\_timer\_alarm.PartitionId} \longrightarrow \\ \quad \quad \text{Unlock} \\ \text{fi} \end{array} \right)$ 

CheckSchedulingCondition  $\hat{=}$  core_kernel_service_get_lock_level.PartitionId  $\longrightarrow$ 
                           core_kernel_service_get_lock_level_return.PartitionId  $\longrightarrow$ 
                           core_kernel_service_get_lock_level_output.PartitionId ?ll  $\longrightarrow$ 
                            $\left( \begin{array}{l} \text{if } (ll > \text{MIN\_LOCK\_LEVEL}) \longrightarrow \text{Skip} \\ \quad \square \quad (ll = \text{MIN\_LOCK\_LEVEL}) \longrightarrow \\ \quad \quad \text{general\_process\_scheduling.PartitionId} \longrightarrow \text{Skip} \\ \text{fi} \end{array} \right)$ 

```

$SystemCallHandle\_Pre \hat{=} \text{var } ssreg : SSREGISTER\_TYPE \bullet$   
 $system\_call.PartitionId.callerid ?i \longrightarrow$   
 $kernel\_disable\_interrupt.PartitionId \longrightarrow kernel\_disabled\_interrupt.PartitionId \longrightarrow$   
 $kernel\_save\_context.PartitionId !PART \longrightarrow$   
 $kernel\_saved\_context.PartitionId ?cpureg ?pt \longrightarrow$   
 $ProcessTable(callerid).KernelTempContext := \langle makecontext(cpureg, pt) \rangle^{\wedge}$   
 $ProcessTable(callerid).KernelTempContext;$   
 $CreateStackSegment[(ProcessTable(callerid).KernelStack.Start)/ss?, unsignedtobin$   
 $(ProcessTable(callerid).KernelStack.Size)/sl?, 0_{PSU}/bp?, 0_{PSU}/sp?, ssreg/ssreg!];$   
 $kernel\_switch\_stack.PartitionId !ssreg !KernelPageTableRef \longrightarrow$   
 $kernel\_switched\_stack.PartitionId \longrightarrow$   
 $kernel\_enable\_interrupt.PartitionId \longrightarrow kernel\_enabled\_interrupt.PartitionId \longrightarrow ;$   
 $SelectSystemCallServiceRoutine(callerid, i)$

$SelectSysCallServiceRoutine \hat{=} callerid : PROCESS\_ID\_TYPE, i : SYSTEM\_CALL\_TYPE \bullet$   
 $(i \in SystemCall\_Partition) \& SelectSysCallServiceRoutine\_Partition(callerid, i)$   
 $(i \in SystemCall\_Process) \& SelectSysCallServiceRoutine\_Process(callerid, i)$   
 $(i \in SystemCall\_Time) \& SelectSysCallServiceRoutine\_Time(callerid, i)$

$SelectSysCallServiceRoutine\_Partition \hat{=} callerid : PROCESS\_ID\_TYPE, i : SYSTEM\_CALL\_TYPE \bullet$   
 $(i = GET\_OPERATING\_MODE) \& system\_call\_handler\_invoke\_$   
 $service\_routine\_get\_operating\_mode.PartitionId.callerid \longrightarrow \text{Skip}$   
 $(i = GET\_PARTITION\_STATUS) \& system\_call\_handler\_invoke\_$   
 $service\_routine\_get\_partition\_status.PartitionId.callerid \longrightarrow \text{Skip}$   
 $(i = SET\_OPERATING\_MODE) \& system\_call\_handler\_invoke\_$   
 $service\_routine\_set\_operating\_mode.PartitionId.callerid \longrightarrow \text{Skip}$

$SelectSysCallServiceRoutine\_Process \hat{=} callerid : PROCESS\_ID\_TYPE, i : SYSTEM\_CALL\_TYPE \bullet$   
 $(i = GET\_PROCESS\_NAMES) \& system\_call\_handler\_invoke\_service\_routine\_get\_process\_names.PartitionId.callerid \longrightarrow \mathbf{Skip}$   
 $(i = GET\_PROCESS\_IDS) \& system\_call\_handler\_invoke\_service\_routine\_get\_process\_ids.PartitionId.callerid \longrightarrow \mathbf{Skip}$   
 $(i = GET\_FREE\_PROCESS\_IDS) \& system\_call\_handler\_invoke\_service\_routine\_get\_free\_process\_ids.PartitionId.callerid \longrightarrow \mathbf{Skip}$   
 $(i = GET\_FREE\_SPACE) \& system\_call\_handler\_invoke\_service\_routine\_get\_free\_space.PartitionId.callerid \longrightarrow \mathbf{Skip}$   
 $(i = GET\_PARTITION\_PERIOD) \& system\_call\_handler\_invoke\_service\_routine\_get\_partition\_period.PartitionId.callerid \longrightarrow \mathbf{Skip}$   
 $(i = GET\_PROCESS\_STATE) \& system\_call\_handler\_invoke\_service\_routine\_get\_process\_state.PartitionId.callerid \longrightarrow \mathbf{Skip}$   
 $(i = GET\_NEXT\_PERIODIC\_START) \& system\_call\_handler\_invoke\_service\_routine\_get\_next\_periodic\_start.PartitionId.callerid \longrightarrow \mathbf{Skip}$   
 $(i = GET\_DELAYED\_PERIODIC\_START) \& system\_call\_handler\_invoke\_service\_routine\_get\_delayed\_periodic\_start.PartitionId.callerid \longrightarrow \mathbf{Skip}$   
 $(i = GET\_PROCESS\_KIND) \& system\_call\_handler\_invoke\_service\_routine\_get\_process\_kind.PartitionId.callerid \longrightarrow \mathbf{Skip}$   
 $(i = GET\_PROCESS\_PERIOD) \& system\_call\_handler\_invoke\_service\_routine\_get\_process\_period.PartitionId.callerid \longrightarrow \mathbf{Skip}$   
 $(i = GET\_PROCESS\_TIME\_CAPACITY) \& system\_call\_handler\_invoke\_service\_routine\_get\_process\_time\_capacity.PartitionId.callerid \longrightarrow \mathbf{Skip}$   
 $(i = GET\_PARTITION\_LOCK\_LEVEL) \& system\_call\_handler\_invoke\_service\_routine\_get\_partition\_lock\_level.PartitionId.callerid \longrightarrow \mathbf{Skip}$   
 $(i = GET\_PROCESS\_ID) \& system\_call\_handler\_invoke\_service\_routine\_get\_process\_id.PartitionId.callerid \longrightarrow \mathbf{Skip}$   
 $(i = GET\_PROCESS\_STATUS) \& system\_call\_handler\_invoke\_service\_routine\_get\_process\_status.PartitionId.callerid \longrightarrow \mathbf{Skip}$   
 $(i = CREATE\_PROCESS) \& system\_call\_handler\_invoke\_service\_routine\_create\_process.PartitionId.callerid \longrightarrow \mathbf{Skip}$   
 $(i = SET\_PRIORITY) \& system\_call\_handler\_invoke\_service\_routine\_set\_priority.PartitionId.callerid \longrightarrow \mathbf{Skip}$   
 $(i = SUSPEND\_SELF) \& system\_call\_handler\_invoke\_service\_routine\_suspend\_self.PartitionId.callerid \longrightarrow \mathbf{Skip}$   
 $(i = SUSPEND) \& system\_call\_handler\_invoke\_service\_routine\_suspend.PartitionId.callerid \longrightarrow \mathbf{Skip}$   
 $(i = RESUME) \& system\_call\_handler\_invoke\_service\_routine\_resume.PartitionId.callerid \longrightarrow \mathbf{Skip}$   
 $(i = STOP\_SELF) \& system\_call\_handler\_invoke\_service\_routine\_stop\_self.PartitionId.callerid \longrightarrow \mathbf{Skip}$   
 $(i = STOP) \& system\_call\_handler\_invoke\_service\_routine\_stop.PartitionId.callerid \longrightarrow \mathbf{Skip}$   
 $(i = START) \& system\_call\_handler\_invoke\_service\_routine\_start.PartitionId.callerid \longrightarrow \mathbf{Skip}$   
 $(i = DELAYED\_START) \& system\_call\_handler\_invoke\_service\_routine\_delayed\_start.PartitionId.callerid \longrightarrow \mathbf{Skip}$   
 $(i = LOCK\_PREEMPTION) \& system\_call\_handler\_invoke\_service\_routine\_lock\_preemption.PartitionId.callerid \longrightarrow \mathbf{Skip}$   
 $(i = UNLOCK\_PREEMPTION) \& system\_call\_handler\_invoke\_service\_routine\_unlock\_preemption.PartitionId.callerid \longrightarrow \mathbf{Skip}$   
 $(i = GET\_MY\_ID) \& system\_call\_handler\_invoke\_service\_routine\_get\_my\_id.PartitionId.callerid \longrightarrow \mathbf{Skip}$

$$\begin{aligned}
\text{SelectSysCallServiceRoutine\_Time} &\hat{=} \text{callerid} : \text{PROCESS\_ID\_TYPE}, i : \text{SYSTEM\_CALL\_TYPE} \bullet \\
&\quad (i = \text{GET\_CURRENT\_TIME}) \& \text{system\_call\_handler\_invoke\_} \\
&\quad \text{service\_routine\_get\_current\_time.PartitionId.callerid} \longrightarrow \text{Skip} \\
&\quad (i = \text{GET\_PARTITION\_TIME}) \& \text{system\_call\_handler\_invoke\_} \\
&\quad \text{service\_routine\_get\_partition\_time.PartitionId.callerid} \longrightarrow \text{Skip} \\
&\quad (i = \text{GET\_NEXT\_RELEASE\_POINT}) \& \text{system\_call\_handler\_invoke\_} \\
&\quad \text{service\_routine\_get\_next\_release\_point.PartitionId.callerid} \longrightarrow \text{Skip} \\
&\quad (i = \text{TIMED\_WAIT}) \& \text{system\_call\_handler\_invoke\_} \\
&\quad \text{service\_routine\_timed\_wait.PartitionId.callerid} \longrightarrow \text{Skip} \\
&\quad (i = \text{PERIODIC\_WAIT}) \& \text{system\_call\_handler\_invoke\_} \\
&\quad \text{service\_routine\_periodic\_wait.PartitionId.callerid} \longrightarrow \text{Skip} \\
&\quad (i = \text{GET\_TIME}) \& \text{system\_call\_handler\_invoke\_} \\
&\quad \text{service\_routine\_get\_time.PartitionId.callerid} \longrightarrow \text{Skip} \\
&\quad (i = \text{REPLENISH}) \& \text{system\_call\_handler\_invoke\_} \\
&\quad \text{service\_routine\_replenish.PartitionId.callerid} \longrightarrow \text{Skip} \\
\\
\text{SysCall\_GetOperatingMode} &\hat{=} \text{system\_call\_handler\_invoke\_service\_routine\_get\_operating\_mode.PartitionId.} \\
&\quad \text{callerid} \longrightarrow \\
&\quad \text{core\_kernel\_service\_get\_operating\_mode.PartitionId} \longrightarrow \\
&\quad \text{core\_kernel\_service\_get\_operating\_mode\_return.PartitionId} \longrightarrow \\
&\quad \text{core\_kernel\_service\_get\_operating\_mode\_output.PartitionId} \text{ ?om} \longrightarrow \\
&\quad \text{system\_call\_service\_routine\_get\_operating\_mode\_output.PartitionId.callerid} \\
&\quad \text{!om} \longrightarrow \\
&\quad \text{system\_call\_service\_routine\_end.PartitionId.callerid} \longrightarrow \text{Skip} \\
\\
\text{SysCall\_GetPartitionStatus} &\hat{=} \text{system\_call\_handler\_invoke\_service\_routine\_get\_partition\_status.PartitionId.} \\
&\quad \text{callerid} \longrightarrow \\
&\quad \text{core\_kernel\_service\_get\_partition\_status.PartitionId} \longrightarrow \\
&\quad \text{core\_kernel\_service\_get\_partition\_status\_return.PartitionId} \longrightarrow \\
&\quad \text{core\_kernel\_service\_get\_partition\_status\_output.PartitionId} \text{ ?parts} \longrightarrow \\
&\quad \text{system\_call\_service\_routine\_get\_partition\_status\_output.PartitionId.callerid} \\
&\quad \text{!parts} \longrightarrow \\
&\quad \text{system\_call\_service\_routine\_end.PartitionId.callerid} \longrightarrow \text{Skip} \\
\\
\text{SysCall\_SetOperatingMode} &\hat{=} \text{system\_call\_handler\_invoke\_service\_routine\_set\_operating\_mode.PartitionId.} \\
&\quad \text{callerid} \longrightarrow \\
&\quad \text{system\_call\_service\_routine\_set\_operating\_mode\_input.PartitionId.callerid} \\
&\quad \text{?om} \longrightarrow \\
&\quad \text{Lock;} \\
&\quad \text{core\_kernel\_service\_set\_operating\_mode\_input.PartitionId !om} \longrightarrow \\
&\quad \text{core\_kernel\_service\_set\_operating\_mode.PartitionId} \longrightarrow \\
&\quad \text{core\_kernel\_service\_set\_operating\_mode\_return.PartitionId} \longrightarrow \\
&\quad \left( \begin{array}{l} \text{if } (om = \text{IDLE}) \longrightarrow \text{TerminatePartition} \\ \parallel \\ (om = \text{COLD\_START}) \longrightarrow \text{ColdStartPartition} \\ \parallel \\ (om = \text{WARM\_START}) \longrightarrow \text{WarmStartPartition} \\ \parallel \\ (om = \text{NORMAL}) \longrightarrow \text{LaunchPartition} \\ \text{fi} \end{array} \right)
\end{aligned}$$



$TerminatePartition \hat{=} kernel\_end\_high\_precision\_timer.PartitionId \longrightarrow$   
 $kernel\_ended\_high\_precision\_timer.PartitionId \longrightarrow$   
 $partition\_kernel\_end\_service.PartitionId \longrightarrow$   
 $partition\_kernel\_end\_process\_scheduler.PartitionId \longrightarrow$   
 $Unlock;$   
 $ScheduleProcess(IDLE\_PROCESS\_ID)$

$ColdStartPartition \hat{=} kernel\_end\_high\_precision\_timer.PartitionId \longrightarrow$   
 $kernel\_ended\_high\_precision\_timer.PartitionId \longrightarrow$   
 $partition\_kernel\_end\_service.PartitionId \longrightarrow$   
 $partition\_kernel\_end\_process\_scheduler.PartitionId \longrightarrow$   
 $InitPartitionKernel[PartitionConfig/config?, KernelPageTableRef/pagetable?];$   
 $kernel\_set\_area\_memory\_management\_reference.PartitionId !MemoryManagement \longrightarrow$   
 $kernel\_have\_set\_area\_memory\_management\_reference.PartitionId \longrightarrow$   
 $partition\_kernel\_start\_service.PartitionId!PART \longrightarrow$   
 $Unlock;$   
 $ScheduleProcess(IDLE\_PROCESS\_ID)$

$WarmStartPartition \hat{=} kernel\_end\_high\_precision\_timer.PartitionId \longrightarrow$   
 $kernel\_ended\_high\_precision\_timer.PartitionId \longrightarrow$   
 $partition\_kernel\_end\_service.PartitionId \longrightarrow$   
 $partition\_kernel\_end\_process\_scheduler.PartitionId \longrightarrow$   
 $TimeCounterQueue := \langle \rangle; ReadyQueue := \langle \rangle; WaitingQueue := \langle \rangle;$   
 $||| procid : dom ProcessTable \bullet ProcessTable(procid).ProcessState := DORMANT;$   
 $partition\_kernel\_start\_service.PartitionId!PART \longrightarrow$   
 $Unlock;$   
 $ScheduleProcess(IDLE\_PROCESS\_ID)$

$LaunchPartition \hat{=} \text{var } ct : SYSTEM\_TIME\_TYPE, tprocs : \mathbb{P} PROCESS\_ID\_TYPE \bullet$   
 $partition\_kernel\_end\_service.PartitionId \longrightarrow$   
 $kernel\_request\_system\_time.PartitionId \longrightarrow$   
 $kernel\_get\_system\_time.PartitionId ?t \longrightarrow$   
 $kernel\_request\_high\_precision\_time.PartitionId \longrightarrow$   
 $kernel\_get\_high\_precision\_time.PartitionId ?hpt \longrightarrow$   
 $ct := t + hpt \text{ mod } bintosigned(ClockTickInterval);$   
 $||| procid : ran ReadyQueue \bullet UpdateStartedProcess(procid, ct);$   
 $GetTimingProcess[tprocs/tprocs!];$   
 $||| procid : tprocs \bullet UpdateDelayedStartedProcess(procid, ct);$   
 $\left( \begin{array}{l} \text{if } (TotalProcess \in dom ProcessTable) \longrightarrow \\ \quad partition\_kernel\_enable\_error\_handler.PartitionId \longrightarrow \\ \quad partition\_kernel\_enabled\_error\_handler.PartitionId \longrightarrow \\ \quad partition\_kernel\_start\_service.PartitionId!ALL \longrightarrow \\ \quad partition\_kernel\_start\_process\_scheduler.PartitionId \longrightarrow \\ \quad Unlock; \\ \quad MustScheduling \\ \quad \square (TotalProcess \notin dom ProcessTable) \longrightarrow \\ \quad \quad partition\_kernel\_start\_service.PartitionId!ALL \longrightarrow \\ \quad \quad partition\_kernel\_start\_process\_scheduler.PartitionId \longrightarrow \\ \quad \quad Unlock; \\ \quad \quad MustScheduling \\ \text{fi} \end{array} \right)$

$$\begin{aligned}
\text{UpdateStartedProcess} \quad \hat{=} \quad & \text{procid} : \text{PROCESS\_ID\_TYPE}, ct : \text{SYSTEM\_TIME\_TYPE} \bullet \\
& \left( \text{if } (\text{ProcessTable}(\text{procid}).\text{ProcessKind} = \text{APERIODIC}) \longrightarrow \right. \\
& \quad \left( \text{if } ((ct + \text{ProcessTable}(\text{procid}).\text{TimeCapacity}) \in \text{SYSTEM\_TIME\_TYPE}) \longrightarrow \right. \\
& \quad \quad \text{ProcessTable}(\text{procid}).\text{ProcessState} := \text{READY}; \\
& \quad \quad \text{ProcessTable}(\text{procid}).\text{ReleasePoint} := ct; \\
& \quad \quad \text{ProcessTable}(\text{procid}).\text{DeadlineTime} := ct + \text{ProcessTable}(\text{procid}). \\
& \quad \quad \quad \text{TimeCapacity} \\
& \quad \quad \square ((ct + \text{ProcessTable}(\text{procid}).\text{TimeCapacity}) \notin \text{SYSTEM\_TIME\_TYPE}) \longrightarrow \\
& \quad \quad \quad \text{DeqReadyQueue}[\text{procid}/\text{procid?}]; \\
& \quad \quad \quad \text{partition\_kernel\_invoke\_health\_monitor}.\text{PartitionId} \text{ !procid} \longrightarrow \\
& \quad \quad \quad \text{Skip} \\
& \quad \text{fi} \\
& \quad \square (\text{ProcessTable}(\text{procid}).\text{ProcessKind} = \text{PERIODIC}) \longrightarrow \\
& \quad \quad \text{DeqReadyQueue}[\text{procid}/\text{procid?}]; \\
& \quad \quad \text{core\_kernel\_service\_get\_next\_periodic\_start}.\text{PartitionId} \longrightarrow \\
& \quad \quad \text{core\_kernel\_service\_get\_next\_periodic\_start\_return}.\text{PartitionId} \longrightarrow \\
& \quad \quad \text{core\_kernel\_service\_get\_next\_periodic\_start\_output}.\text{PartitionId} \text{ ?nps} \longrightarrow \\
& \quad \quad \left( \text{if } ((nps + \text{ProcessTable}(\text{procid}).\text{TimeCapacity}) \in \text{SYSTEM\_TIME\_TYPE}) \longrightarrow \right. \\
& \quad \quad \quad \text{ProcessTable}(\text{procid}).\text{ReleasePoint} := nps; \\
& \quad \quad \quad \text{ProcessTable}(\text{procid}).\text{DeadlineTime} := nps + \text{ProcessTable}(\text{procid}). \\
& \quad \quad \quad \text{TimeCapacity} \\
& \quad \quad \quad \square ((nps + \text{ProcessTable}(\text{procid}).\text{TimeCapacity}) \notin \text{SYSTEM\_TIME\_TYPE}) \longrightarrow \\
& \quad \quad \quad \text{partition\_kernel\_invoke\_health\_monitor}.\text{PartitionId} \text{ !procid} \longrightarrow \\
& \quad \quad \quad \text{Skip} \\
& \quad \quad \text{fi} \\
& \text{fi}
\end{aligned}$$

$$\begin{aligned}
\text{UpdateDelayedStartedProcess} \quad \hat{=} \quad & \text{procid} : \text{PROCESS\_ID\_TYPE}, ct : \text{SYSTEM\_TIME\_TYPE} \bullet \\
& \left( \text{if } (\text{ProcessTable}(\text{procid}).\text{ProcessKind} = \text{APERIODIC}) \longrightarrow \right. \\
& \quad \text{UpdateDelayedStartedAperiodicProcess}(\text{procid}, ct) \\
& \quad \square (\text{ProcessTable}(\text{procid}).\text{ProcessKind} = \text{PERIODIC}) \longrightarrow \\
& \quad \quad \text{UpdateDelayedStartedPeriodicProcess}(\text{procid}) \\
& \text{fi}
\end{aligned}$$

$$\begin{aligned}
\text{UpdateDelayedStartedAperiodicProcess} \quad \hat{=} \quad & \text{procid} : \text{PROCESS\_ID\_TYPE}, ct : \text{SYSTEM\_TIME\_TYPE} \bullet \\
& \text{var alarm} : \text{SYSTEM\_TIME\_TYPE}, tc : \text{TIME\_COUNTER\_TYPE} \bullet \\
& \text{GetTimingProcessAlarm}[\text{procid}/\text{procid?}, \text{alarm}/\text{alarm!}]; \\
& \text{DeqTimeCounterQueue}[\text{procid}/\text{procid?}]; \\
& \left( \begin{array}{l} \text{if } (\text{alarm} < 0) \longrightarrow \\ \quad \left( \begin{array}{l} \text{if } ((ct + (-\text{alarm}) + \text{ProcessTable}(\text{procid}). \\ \text{TimeCapacity}) \in \text{SYSTEM\_TIME\_TYPE}) \longrightarrow \\ \quad \text{CreateTimeCounter}[\text{procid}/\text{procid?}, (-ct + \text{alarm})/ \\ \text{alarm?}, tc/tc!]; \\ \quad \text{EnqTimeCounterQueue}[tc/tc?]; \\ \quad \text{ProcessTable}(\text{procid}).\text{ReleasePoint} := ct + \\ (-\text{alarm}); \\ \quad \text{ProcessTable}(\text{procid}).\text{DeadlineTime} := ct + \\ (-\text{alarm}) + \text{ProcessTable}(\text{procid}).\text{TimeCapacity} \\ \quad \parallel ((ct + (-\text{alarm}) + \text{ProcessTable}(\text{procid}). \\ \text{TimeCapacity}) \notin \text{SYSTEM\_TIME\_TYPE}) \longrightarrow \\ \quad \text{partition\_kernel\_invoke\_health\_monitor}.\text{PartitionId} \\ \text{!procid} \longrightarrow \text{Skip} \\ \quad \text{fi} \end{array} \right) \\ \parallel (\text{alarm} > 0) \longrightarrow \\ \quad \left( \begin{array}{l} \text{if } ((ct + \text{alarm} + \text{ProcessTable}(\text{procid}).\text{TimeCapacity}) \\ \in \text{SYSTEM\_TIME\_TYPE}) \longrightarrow \\ \quad \text{CreateTimeCounter}[\text{procid}/\text{procid?}, (ct + \text{alarm})/ \\ \text{alarm?}, tc/tc!]; \\ \quad \text{EnqTimeCounterQueue}[tc/tc?]; \\ \quad \text{ProcessTable}(\text{procid}).\text{ReleasePoint} := ct + \text{alarm}; \\ \quad \text{ProcessTable}(\text{procid}).\text{DeadlineTime} := ct + \text{alarm} + \\ \text{ProcessTable}(\text{procid}).\text{TimeCapacity} \\ \quad \parallel ((ct + \text{alarm} + \text{ProcessTable}(\text{procid}).\text{TimeCapacity}) \\ \notin \text{SYSTEM\_TIME\_TYPE}) \longrightarrow \\ \quad \text{partition\_kernel\_invoke\_health\_monitor}.\text{PartitionId} \\ \text{!procid} \longrightarrow \text{Skip} \\ \quad \text{fi} \end{array} \right) \\ \text{fi} \end{array} \right)
\end{aligned}$$

$$\begin{aligned}
\text{UpdateDelayedStartedPeriodicProcess} \quad \hat{=} \quad & \text{procid} : \text{PROCESS\_ID\_TYPE} \bullet \\
& \text{var alarm} : \text{SYSTEM\_TIME\_TYPE} \bullet \\
& \text{GetTimingProcessAlarm}[\text{procid}/\text{procid?}, \text{alarm}/\text{alarm!}]; \\
& \text{DeqTimeCounterQueue}[\text{procid}/\text{procid?}]; \\
& \text{core\_kernel\_service\_get\_delayed\_periodic\_start\_input}.\text{PartitionId} \\
& \text{!alarm} \longrightarrow \\
& \text{core\_kernel\_service\_get\_delayed\_periodic\_start}.\text{PartitionId} \longrightarrow \\
& \text{core\_kernel\_service\_get\_delayed\_periodic\_start\_return}.\text{PartitionId} \\
& \longrightarrow \\
& \text{core\_kernel\_service\_get\_delayed\_periodic\_start\_output}.\text{PartitionId} \\
& \text{?dps} \longrightarrow \\
& \left( \begin{array}{l} \text{if } ((\text{dps} + \text{ProcessTable}(\text{procid}).\text{TimeCapacity}) \in \text{SYSTEM\_} \\ \text{TIME\_TYPE}) \longrightarrow \\ \quad \text{ProcessTable}(\text{procid}).\text{ReleasePoint} := \text{dps}; \\ \quad \text{ProcessTable}(\text{procid}).\text{DeadlineTime} := \text{dps} + \text{ProcessTable} \\ (\text{procid}).\text{TimeCapacity} \\ \quad \parallel ((\text{dps} + \text{ProcessTable}(\text{procid}).\text{TimeCapacity}) \notin \text{SYSTEM\_} \\ \text{TIME\_TYPE}) \longrightarrow \\ \quad \text{partition\_kernel\_invoke\_health\_monitor}.\text{PartitionId} \\ \text{!procid} \longrightarrow \text{Skip} \\ \quad \text{fi} \end{array} \right)
\end{aligned}$$

$$\begin{aligned} \text{SysCallServiceRoutines\_Partition} \quad \hat{=} \quad & \text{SysCall\_GetOperatingMode} \\ & \square \text{SysCall\_GetPartitionStatus} \\ & \square \text{SysCall\_SetOperatingMode} \end{aligned}$$

$$\begin{aligned} \text{SysCall\_GetProcNames} \quad \hat{=} \quad & \mathbf{var} \text{ procns} : \mathbb{P} \text{PROCESS\_NAME\_TYPE} \bullet \\ & \text{system\_call\_handler\_invoke\_service\_routine\_get\_process\_names.PartitionId.} \\ & \text{callerid} \longrightarrow \\ & \text{GetProcessNames}[\text{procns}/\text{procns!}]; \\ & \text{system\_call\_service\_routine\_get\_process\_names\_output.PartitionId.callerid} \\ & !\text{procns} \longrightarrow \\ & \text{system\_call\_service\_routine\_end.PartitionId.callerid} \longrightarrow \mathbf{Skip} \end{aligned}$$

$$\begin{aligned} \text{SysCall\_GetProcIds} \quad \hat{=} \quad & \mathbf{var} \text{ procids} : \mathbb{P} \text{PROCESS\_ID\_TYPE} \bullet \\ & \text{system\_call\_handler\_invoke\_service\_routine\_get\_process\_ids.PartitionId.callerid} \longrightarrow \\ & \text{procids} := 1 \dots (\text{TotalProcess} - 1) \cap \text{dom ProcessTable}; \\ & \text{system\_call\_service\_routine\_get\_process\_ids\_output.PartitionId.callerid} !\text{procids} \longrightarrow \\ & \text{system\_call\_service\_routine\_end.PartitionId.callerid} \longrightarrow \mathbf{Skip} \end{aligned}$$

$$\begin{aligned} \text{SysCall\_GetFreeProcIds} \quad \hat{=} \quad & \mathbf{var} \text{ freeids} : \mathbb{P} \text{PROCESS\_ID\_TYPE} \bullet \\ & \text{system\_call\_handler\_invoke\_service\_routine\_get\_free\_process\_ids.PartitionId.} \\ & \text{callerid} \longrightarrow \\ & \text{freeids} := 1 \dots (\text{TotalProcess} - 1) \setminus \text{dom ProcessTable}; \\ & \text{system\_call\_service\_routine\_get\_free\_process\_ids\_output.PartitionId.callerid} \\ & !\text{freeids} \longrightarrow \\ & \text{system\_call\_service\_routine\_end.PartitionId.callerid} \longrightarrow \mathbf{Skip} \end{aligned}$$

$\text{SysCall\_GetFreeSpace} \hat{=} \text{var } \text{discontinuous}, \text{continuous} : \text{UNSIGNED\_INTEGER\_TYPE} \bullet$   
 $\text{system\_call\_handler\_invoke\_service\_routine\_get\_free\_space.PartitionId.callerid} \longrightarrow$   
 $\text{Lock};$   
 $\text{kernel\_request\_area\_free\_pages.PartitionId} \longrightarrow$   
 $\text{kernel\_get\_area\_free\_pages.PartitionId ?pages} \longrightarrow \text{discontinuous} := \text{pages} * \text{PAGE\_}$   
 $\text{SIZE};$   
 $\text{Unlock};$   
 $\text{Lock};$   
 $\text{kernel\_request\_area\_free\_block.PartitionId} \longrightarrow$   
 $\text{kernel\_get\_area\_free\_block.PartitionId ?maxblocksize} \longrightarrow \text{continuous} := \text{maxblocksize};$   
 $\text{Unlock};$   
 $\text{system\_call\_service\_routine\_get\_free\_space\_output.PartitionId.callerid !discontinuous}$   
 $\text{!continuous} \longrightarrow$   
 $\text{system\_call\_service\_routine\_end.PartitionId.callerid} \longrightarrow \text{Skip}$

$\text{SysCall\_GetPartPeriod} \hat{=} \text{var partp} : \text{SYSTEM\_TIME\_TYPE} \bullet$   
 $\text{system\_call\_handler\_invoke\_service\_routine\_get\_partition\_period.PartitionId.}$   
 $\text{callerid} \longrightarrow$   
 $\text{partp} := \text{Periodicity.Period};$   
 $\text{system\_call\_service\_routine\_get\_partition\_period\_output.PartitionId.callerid}$   
 $! \text{partp} \longrightarrow$   
 $\text{system\_call\_service\_routine\_end.PartitionId.callerid} \longrightarrow \text{Skip}$

$\text{SysCall\_GetProcState} \hat{=} \text{var procs} : \text{PROCESS\_STATE\_TYPE} \bullet$   
 $\text{system\_call\_handler\_invoke\_service\_routine\_get\_process\_state.PartitionId.}$   
 $\text{callerid} \longrightarrow$   
 $\text{system\_call\_service\_routine\_get\_process\_state\_input.PartitionId.callerid}$   
 $? \text{procid} \longrightarrow$   
 $\text{procs} := \text{ProcessTable(procid).ProcessState};$   
 $\text{system\_call\_service\_routine\_get\_process\_state\_output.PartitionId.callerid}$   
 $! \text{procs} \longrightarrow$   
 $\text{system\_call\_service\_routine\_end.PartitionId.callerid} \longrightarrow \text{Skip}$

$\text{SysCall\_GetNextPeriodicStart} \hat{=} \text{system\_call\_handler\_invoke\_service\_routine\_get\_next\_periodic\_start.}$   
 $\text{PartitionId.callerid} \longrightarrow$   
 $\text{core\_kernel\_service\_get\_next\_periodic\_start.PartitionId} \longrightarrow$   
 $\text{core\_kernel\_service\_get\_next\_periodic\_start\_return.PartitionId} \longrightarrow$   
 $\text{core\_kernel\_service\_get\_next\_periodic\_start\_output.PartitionId} ? \text{nps} \longrightarrow$   
 $\text{system\_call\_service\_routine\_get\_next\_periodic\_start\_output.PartitionId.}$   
 $\text{callerid} ! \text{nps} \longrightarrow$   
 $\text{system\_call\_service\_routine\_end.PartitionId.callerid} \longrightarrow \text{Skip}$

$\text{SysCall\_GetDelayedPeriodicStart} \hat{=} \text{system\_call\_handler\_invoke\_service\_routine\_get\_delayed\_periodic\_start.}$   
 $\text{PartitionId.callerid} \longrightarrow$   
 $\text{system\_call\_service\_routine\_get\_delayed\_periodic\_start\_input.PartitionId.}$   
 $\text{callerid} ? \text{dt} \longrightarrow$   
 $\text{core\_kernel\_service\_get\_delayed\_periodic\_start\_input.PartitionId} ! \text{dt} \longrightarrow$   
 $\text{core\_kernel\_service\_get\_delayed\_periodic\_start.PartitionId} \longrightarrow$   
 $\text{core\_kernel\_service\_get\_delayed\_periodic\_start\_return.PartitionId} \longrightarrow$   
 $\text{core\_kernel\_service\_get\_delayed\_periodic\_start\_output.PartitionId} ? \text{dps} \longrightarrow$   
 $\text{system\_call\_service\_routine\_get\_delayed\_periodic\_start\_output.PartitionId.}$   
 $\text{callerid} ! \text{dps} \longrightarrow$   
 $\text{system\_call\_service\_routine\_end.PartitionId.callerid} \longrightarrow \text{Skip}$

$\text{SysCall\_GetProcKind} \hat{=} \text{var prock} : \text{PROCESS\_KIND\_TYPE} \bullet$   
 $\text{system\_call\_handler\_invoke\_service\_routine\_get\_process\_kind.PartitionId.callerid} \longrightarrow$   
 $\text{system\_call\_service\_routine\_get\_process\_kind\_input.PartitionId.callerid} ? \text{procid} \longrightarrow$   
 $\text{prock} := \text{ProcessTable(procid).ProcessKind};$   
 $\text{system\_call\_service\_routine\_get\_process\_kind\_output.PartitionId.callerid} ! \text{prock} \longrightarrow$   
 $\text{system\_call\_service\_routine\_end.PartitionId.callerid} \longrightarrow \text{Skip}$

$\text{SysCall\_GetProcPeriod} \hat{=} \text{var procp} : \text{SYSTEM\_TIME\_TYPE} \bullet$   
 $\text{system\_call\_handler\_invoke\_service\_routine\_get\_process\_period.PartitionId.callerid} \longrightarrow$   
 $\text{system\_call\_service\_routine\_get\_process\_period\_input.PartitionId.callerid} ? \text{procid} \longrightarrow$   
 $\text{procp} := \text{ProcessTable(procid).Period};$   
 $\text{system\_call\_service\_routine\_get\_process\_period\_output.PartitionId.callerid} ! \text{procp} \longrightarrow$   
 $\text{system\_call\_service\_routine\_end.PartitionId.callerid} \longrightarrow \text{Skip}$

$\text{SysCall\_GetProcTimeCapacity} \hat{=} \text{var proctc} : \text{SYSTEM\_TIME\_TYPE} \bullet$   
 $\text{system\_call\_handler\_invoke\_service\_routine\_get\_process\_time\_capacity.}$   
 $\text{PartitionId.callerid} \longrightarrow$   
 $\text{system\_call\_service\_routine\_get\_process\_time\_capacity\_input.PartitionId.}$   
 $\text{callerid} ? \text{procid} \longrightarrow$   
 $\text{proctc} := \text{ProcessTable(procid).TimeCapacity};$   
 $\text{system\_call\_service\_routine\_get\_process\_time\_capacity\_output.PartitionId.}$

$\text{SysCall\_GetPartLockLevel} \hat{=} \text{system\_call\_handler\_invoke\_service\_routine\_get\_partition\_lock\_level.PartitionId.callerid} \longrightarrow$   
 $\text{core\_kernel\_service\_get\_lock\_level.PartitionId} \longrightarrow$   
 $\text{core\_kernel\_service\_get\_lock\_level\_return.PartitionId} \longrightarrow$   
 $\text{core\_kernel\_service\_get\_lock\_level\_output.PartitionId} \text{ ?ll} \longrightarrow$   
 $\text{system\_call\_service\_routine\_get\_partition\_lock\_level\_output.PartitionId.callerid}$   
 $\text{!ll} \longrightarrow$   
 $\text{system\_call\_service\_routine\_end.PartitionId.callerid} \longrightarrow \mathbf{Skip}$

$\text{SysCall\_GetProcessId} \hat{=} \mathbf{var} \text{ procid} : \text{PROCESS\_ID\_TYPE} \bullet$   
 $\text{system\_call\_handler\_invoke\_service\_routine\_get\_process\_id.PartitionId.callerid} \longrightarrow$   
 $\text{system\_call\_service\_routine\_get\_process\_id\_input.PartitionId.callerid} \text{ ?procn} \longrightarrow$   
 $\text{GetProcessId[procn/procn?, procid/procid!];}$   
 $\text{system\_call\_service\_routine\_get\_process\_id\_output.PartitionId.callerid} \text{ !procid} \longrightarrow$   
 $\text{system\_call\_service\_routine\_end.PartitionId.callerid} \longrightarrow \mathbf{Skip}$

$\text{SysCall\_GetProcessStatus} \hat{=} \mathbf{var} \text{ procs} : \text{PROCESS\_STATUS\_TYPE} \bullet$   
 $\text{system\_call\_handler\_invoke\_service\_routine\_get\_process\_status.PartitionId.callerid} \longrightarrow$   
 $\text{system\_call\_service\_routine\_get\_process\_status\_input.PartitionId.callerid}$   
 $\text{?procid} \longrightarrow$   
 $\text{GetProcessStatus[procid/procid?, procs/procs!];}$   
 $\text{system\_call\_service\_routine\_get\_process\_status\_output.PartitionId.callerid}$   
 $\text{!procs} \longrightarrow$   
 $\text{system\_call\_service\_routine\_end.PartitionId.callerid} \longrightarrow \mathbf{Skip}$

$\text{SysCall\_CreateProcess} \hat{=} \mathbf{var} \text{ procid} : \text{PROCESS\_ID\_TYPE} \bullet$   
 $\text{system\_call\_handler\_invoke\_service\_routine\_create\_process.PartitionId.callerid} \longrightarrow$   
 $\text{system\_call\_service\_routine\_create\_process\_input.PartitionId.callerid} \text{ ?proca ?exefile}$   
 $\text{?exefilepath ?swapfilepath} \longrightarrow$   
 $\left( \begin{array}{l} \mathbf{if} \text{ (proca.ProcessKind} \neq \text{ERROR\_HANDLER)} \longrightarrow \\ \text{procid} := \min(1 \dots (\text{TotalProcess} - 1) \setminus \text{dom ProcessTable}); \\ \text{CreateProcEntity(procid, proca, exefile, exefilepath, swapfilepath);} \\ \text{system\_call\_service\_routine\_create\_process\_output.PartitionId.callerid} \\ \text{!procid} \longrightarrow \\ \text{system\_call\_service\_routine\_end.PartitionId.callerid} \longrightarrow \mathbf{Skip} \\ \square \\ \text{(proca.ProcessKind} = \text{ERROR\_HANDLER)} \longrightarrow \text{procid} := \text{TotalProcess;} \\ \text{CreateProcEntity(procid, proca, exefile, exefilepath, swapfilepath);} \\ \text{system\_call\_service\_routine\_create\_process\_output.PartitionId.callerid} \\ \text{!procid} \longrightarrow \\ \text{system\_call\_service\_routine\_end.PartitionId.callerid} \longrightarrow \mathbf{Skip} \\ \mathbf{fi} \end{array} \right)$

$CreateProcessEntity \hat{=}$  *procid* : *PROCESS\_ID\_TYPE*, *proca* : *PROCESS\_ATTRIBUTE\_TYPE*,  
*exefile* : *EXECUTABLE\_FILE\_TYPE*, *exefilepath*, *swapfilepath* : *PATH\_TYPE* •  
**var** *proccb* : *PROCESS\_CONTROL\_BLOCK\_TYPE* •  
*Lock*;  
*kernel\_allocate\_area\_free\_block.PartitionId* !*KERNEL\_STACK\_SIZE*  $\longrightarrow$   
*kernel\_allocated\_area\_free\_block.PartitionId* ?*block*  $\longrightarrow$   
*Unlock*;  
*Lock*;  
*kernel\_create\_virtual\_memory\_block.PartitionId*  
!(*KernelPageTableRef*  $\sim$  (*block.Start*)) !*KERNEL\_STACK\_SIZE*  $\longrightarrow$   
*kernel\_created\_virtual\_memory\_block.PartitionId* ?*kstack*  $\longrightarrow$   
*Unlock*;  
*Lock*;  
*kernel\_allocate\_area\_free\_pages.PartitionId* !(*pagecount*(*proca.StackSize*) + *pagecount*(#  
(*exefile.Data*)) + *pagecount*(#(*exefile.Code*)))  $\longrightarrow$   
*kernel\_allocated\_area\_free\_pages.PartitionId* ?*base*  $\longrightarrow$   
*Unlock*;  
*Lock*;  
*kernel\_create\_process\_virtual\_memory.PartitionId* !*base* !(*proca.StackSize*) !*sizecount*(#  
(*exefile.Data*)) !*sizecount*(#(*exefile.Code*)))  $\longrightarrow$   
*kernel\_created\_process\_virtual\_memory.PartitionId* ?*procvm*  $\longrightarrow$   
*Unlock*;  
*Lock*;  
*kernel\_full\_load\_process\_pages.PartitionId* !*procvm* !(*proca.EntryPoint*) !*exefile*  $\longrightarrow$   
*kernel\_full\_loaded\_process\_pages.PartitionId* ?*pagetable*  $\longrightarrow$   
*procvm.VMBlock.PageTable* := *pagetable*;  
*Unlock*;  
*CreateProcessControlBlock*[*proca/proca?*, *exefilepath/exefilepath?*, *swapfilepath/swapfilepath?*,  
*kstack/kstack?*, *procvm/procvm?*, *proccb/proccb!*];  
*ProcessTable* := *ProcessTable*  $\cup$  {*procid*  $\mapsto$  *proccb*}

$SysCall_SetPriority \hat{=}$  *system\_call\_handler\_invoke\_service\_routine\_set\_priority.PartitionId.callerid*  $\longrightarrow$   
*system\_call\_service\_routine\_set\_priority\_input.PartitionId.callerid* ?*procid* ?*p*  $\longrightarrow$   
 $\left( \begin{array}{l} \text{if } (procid = callerid) \longrightarrow \\ \left( \begin{array}{l} \text{if } (p = ProcessTable(procid).CurrentPriority) \longrightarrow \\ \quad system\_call\_service\_routine\_end.PartitionId.callerid \longrightarrow \text{Skip} \\ \quad \parallel (p > ProcessTable(procid).CurrentPriority) \longrightarrow \\ \quad \quad ProcessTable(procid).CurrentPriority := p; \\ \quad \quad system\_call\_service\_routine\_end.PartitionId.callerid \longrightarrow \text{Skip} \\ \quad \parallel (p < ProcessTable(procid).CurrentPriority) \longrightarrow \\ \quad \quad ProcessTable(procid).CurrentPriority := -p; \\ \quad \quad CheckSchedulingCondition; \\ \quad \quad system\_call\_service\_routine\_end.PartitionId.callerid \longrightarrow \text{Skip} \\ \quad \text{fi} \end{array} \right) \\ \parallel (procid \neq callerid) \longrightarrow \\ \left( \begin{array}{l} \text{if } (p = ProcessTable(procid).CurrentPriority) \longrightarrow \\ \quad system\_call\_service\_routine\_end.PartitionId.callerid \longrightarrow \text{Skip} \\ \quad \parallel (p > ProcessTable(procid).CurrentPriority) \longrightarrow \\ \quad \quad ProcessTable(procid).CurrentPriority := p; \\ \quad \quad CheckSchedulingCondition; \\ \quad \quad system\_call\_service\_routine\_end.PartitionId.callerid \longrightarrow \text{Skip} \\ \quad \parallel (p < ProcessTable(procid).CurrentPriority) \longrightarrow \\ \quad \quad ProcessTable(procid).CurrentPriority := p; \\ \quad \quad system\_call\_service\_routine\_end.PartitionId.callerid \longrightarrow \text{Skip} \\ \quad \text{fi} \end{array} \right) \\ \text{fi} \end{array} \right)$



$$\begin{aligned}
\text{SysCall\_SuspendSelf} \quad \hat{=} \quad & \text{system\_call\_handler\_invoke\_service\_routine\_suspend\_self.PartitionId.callerid} \longrightarrow \\
& \text{system\_call\_service\_routine\_suspend\_self\_input.PartitionId.callerid ?hpt ?delta} \longrightarrow \\
& \left( \begin{array}{l}
\text{if } (\text{delta} = 0) \longrightarrow \\
\quad \text{ProcessTable}(\text{callerid}).\text{ProcessState} := \text{READY}; \\
\quad \text{EnqReadyQueue}_2[\text{callerid}/\text{procid?}]; \\
\quad \text{general\_process\_scheduling.PartitionId} \longrightarrow \\
\quad \text{system\_call\_service\_routine\_suspend\_self\_output.PartitionId.callerid} \\
\quad \text{!TRUE} \longrightarrow \\
\quad \text{system\_call\_service\_routine\_end.PartitionId.callerid} \longrightarrow \text{Skip} \\
\quad \square (\text{delta} < 0) \longrightarrow \\
\quad \quad \text{ProcessTable}(\text{callerid}).\text{ProcessState} := \text{WAITING}; \\
\quad \quad \text{general\_process\_scheduling.PartitionId} \longrightarrow \\
\quad \quad \text{suspended\_process\_get\_resumed.PartitionId.callerid} \longrightarrow \\
\quad \quad \text{system\_call\_service\_routine\_suspend\_self\_output.PartitionId.callerid} \\
\quad \quad \text{!TRUE} \longrightarrow \\
\quad \quad \text{system\_call\_service\_routine\_end.PartitionId.callerid} \longrightarrow \text{Skip} \\
\quad \square (\text{delta} > 0) \longrightarrow \\
\quad \quad \text{ProcessTable}(\text{callerid}).\text{ProcessState} := \text{WAITING}; \\
\quad \quad \text{AddTimeCounter}(\text{callerid}, (\text{hpt} + \text{delta}), \text{NORMAL}); \\
\quad \quad \text{general\_process\_scheduling.PartitionId} \longrightarrow \\
\quad \quad \left( \begin{array}{l}
\text{suspended\_process\_get\_resumed.PartitionId.callerid} \longrightarrow \\
\text{system\_call\_service\_routine\_suspend\_self\_output.PartitionId.} \\
\text{callerid !TRUE} \longrightarrow \\
\text{system\_call\_service\_routine\_end.PartitionId.callerid} \longrightarrow \text{Skip}
\end{array} \right) \\
\quad \square \left( \begin{array}{l}
\text{time\_out\_expired.PartitionId.callerid} \longrightarrow \\
\text{system\_call\_service\_routine\_suspend\_self\_output.PartitionId.} \\
\text{callerid !FALSE} \longrightarrow \\
\text{system\_call\_service\_routine\_end.PartitionId.callerid} \longrightarrow \text{Skip}
\end{array} \right) \\
\text{fi}
\end{array} \right)
\end{aligned}$$

$$\begin{aligned}
SysCall\_Suspend \quad \hat{=} \quad & system\_call\_handler\_invoke\_service\_routine\_suspend.PartitionId.callerid \longrightarrow \\
& system\_call\_service\_routine\_suspend\_input.PartitionId.callerid \ ?procid \longrightarrow \\
& \left( \begin{array}{l} \textbf{if} \quad (procid \in \text{ran } ReadyQueue) \longrightarrow \\ \quad DeqReadyQueue[procid/procid?]; \\ \quad ProcessTable(procid).ProcessState := WAITING; \\ \quad system\_call\_service\_routine\_suspend\_output.PartitionId.callerid \\ \quad !TRUE \longrightarrow \\ \quad system\_call\_service\_routine\_end.PartitionId.callerid \longrightarrow \textbf{Skip} \\ \quad \parallel \\ \quad (procid \notin \text{ran } ReadyQueue) \longrightarrow \\ \quad \quad SuspendWaitingProcess(callerid, procid); \\ \quad \quad system\_call\_service\_routine\_end.PartitionId.callerid \longrightarrow \textbf{Skip} \\ \textbf{fi} \end{array} \right)
\end{aligned}$$

$$\begin{aligned}
\text{SuspendWaitingProcess} \quad \hat{=} \quad & \text{callerid, procid} : \text{PROCESS\_ID\_TYPE} \bullet \\
& \text{var tprocsids} : \mathbb{P} \text{PROCESS\_ID\_TYPE} \bullet \\
& \text{GetTimingProcess}[tprocsids/tprocsids!]; \\
& \left( \begin{array}{l} \text{if } (\text{ProcessTable}(\text{procid}).\text{CurrentPriority} < 0 \vee \text{procid} \notin \text{tprocsids}) \longrightarrow \\ \quad \text{system\_call\_service\_routine\_suspend\_output}.\text{PartitionId}.\text{callerid} \\ \quad \text{!FALSE} \longrightarrow \text{Skip} \\ \quad \parallel (\text{ProcessTable}(\text{procid}).\text{CurrentPriority} > 0 \wedge \text{procid} \in \text{tprocsids} \\ \quad \wedge \# \text{ProcessTable}(\text{procid?}).\text{KernelTempContext} = 1) \longrightarrow \\ \quad \quad \text{TurnOverTimeCounter}[\text{procid}/\text{procid?}]; \\ \quad \quad \text{system\_call\_service\_routine\_suspend\_output}.\text{PartitionId}.\text{callerid} \\ \quad \quad \text{!TRUE} \longrightarrow \text{Skip} \\ \quad \parallel (\text{ProcessTable}(\text{procid}).\text{CurrentPriority} > 0 \wedge \text{procid} \in \text{tprocsids} \\ \quad \wedge \# \text{ProcessTable}(\text{procid?}).\text{KernelTempContext} > 1) \longrightarrow \\ \quad \quad \text{system\_call\_service\_routine\_suspend\_output}.\text{PartitionId}.\text{callerid} \\ \quad \quad \text{!FALSE} \longrightarrow \text{Skip} \\ \text{fi} \end{array} \right)
\end{aligned}$$

$$\begin{aligned}
\text{SysCall\_Resume} \quad \hat{=} \quad & \text{var tprocsids} : \mathbb{P} \text{PROCESS\_ID\_TYPE} \bullet \\
& \text{system\_call\_handler\_invoke\_service\_routine\_resume}.\text{PartitionId}.\text{callerid} \longrightarrow \\
& \text{system\_call\_service\_routine\_resume\_input}.\text{PartitionId}.\text{callerid} \text{ ?procid} \longrightarrow \\
& \left( \begin{array}{l} \text{if } (\text{procid} \in \text{ran WaitingQueue}) \longrightarrow \\ \quad \text{system\_call\_service\_routine\_end}.\text{PartitionId}.\text{callerid} \longrightarrow \text{Skip} \\ \quad \parallel (\text{procid} \notin \text{ran WaitingQueue}) \longrightarrow \\ \quad \text{GetTimingProcess}[tprocsids/tprocsids!]; \\ \quad \left( \begin{array}{l} \text{if } (\text{procid} \notin \text{tprocsids}) \longrightarrow \\ \quad \text{ProcessTable}(\text{procid}).\text{ProcessState} := \text{READY}; \\ \quad \text{EnqReadyQueue}_2[\text{procid}/\text{procid?}]; \\ \quad \text{CheckSchedulingCondition}; \\ \quad \text{system\_call\_service\_routine\_end}.\text{PartitionId}.\text{callerid} \longrightarrow \text{Skip} \\ \quad \parallel (\text{procid} \in \text{tprocsids}) \longrightarrow \\ \quad \quad \text{ResumeTimingProcess}(\text{callerid}, \text{procid}); \\ \quad \quad \text{system\_call\_service\_routine\_end}.\text{PartitionId}.\text{callerid} \longrightarrow \text{Skip} \\ \text{fi} \end{array} \right) \\ \text{fi} \end{array} \right)
\end{aligned}$$

$$\begin{aligned}
\text{ResumeTimingProcess} \quad \hat{=} \quad & \text{callerid, procid} : \text{PROCESS\_ID\_TYPE} \bullet \\
& \text{var alarm} : \text{SYSTEM\_TIME\_TYPE} \bullet \\
& \left( \begin{array}{l} \text{if } (\text{ProcessTable}(\text{procid}).\text{CurrentPriority} < 0) \longrightarrow \text{Skip} \\ \quad \parallel (\text{ProcessTable}(\text{procid}).\text{CurrentPriority} > 0 \\ \quad \wedge \# \text{ProcessTable}(\text{procid?}).\text{KernelTempContext} > 1) \longrightarrow \\ \quad \quad \text{RemoveTimeCounter}(\text{procid}, \text{NORMAL}); \\ \quad \quad \text{ProcessTable}(\text{procid}).\text{ProcessState} := \text{READY}; \\ \quad \quad \text{EnqReadyQueue}_2[\text{procid}/\text{procid?}]; \\ \quad \quad \text{suspended\_process\_get\_resumed}.\text{PartitionId} \text{ !procid} \longrightarrow \\ \quad \quad \text{CheckSchedulingCondition} \\ \quad \parallel (\text{ProcessTable}(\text{procid}).\text{CurrentPriority} > 0 \\ \quad \wedge \# \text{ProcessTable}(\text{procid?}).\text{KernelTempContext} = 1) \longrightarrow \\ \quad \quad \text{GetTimingProcessAlarm}[\text{procid}/\text{procid?}, \text{alarm}/\text{alarm!}]; \\ \quad \quad \left( \begin{array}{l} \text{if } (\text{alarm} > 0) \longrightarrow \text{Skip} \\ \quad \parallel (\text{alarm} < 0) \longrightarrow \text{TurnOverTimeCounter}[\text{procid}/\text{procid?}] \\ \text{fi} \end{array} \right) \\ \text{fi} \end{array} \right)
\end{aligned}$$

$$\begin{aligned}
\text{SysCall\_StopSelf} \quad \hat{=} \quad & \text{system\_call\_handler\_invoke\_service\_routine\_stop\_self.PartitionId.callerid} \longrightarrow \\
& \text{ProcessTable(callerid).ProcessState} := \text{DORMANT}; \\
& \left( \begin{array}{l} \text{if } (\text{ProcessTable(callerid).ProcessKind} \neq \text{ERROR\_HANDLER}) \longrightarrow \\ \quad \text{core\_kernel\_service\_reset\_lock\_level.PartitionId} \longrightarrow \\ \quad \text{core\_kernel\_service\_reset\_lock\_level\_return.PartitionId} \longrightarrow \\ \quad \text{general\_process\_scheduling.PartitionId} \longrightarrow \text{Skip} \\ \quad \parallel (\text{ProcessTable(callerid).ProcessKind} = \text{ERROR\_HANDLER}) \longrightarrow \\ \quad \text{error\_process\_id ?eprocid} \longrightarrow \\ \quad \text{core\_kernel\_service\_get\_lock\_level.PartitionId} \longrightarrow \\ \quad \text{core\_kernel\_service\_get\_lock\_level\_return.PartitionId} \longrightarrow \\ \quad \text{core\_kernel\_service\_get\_lock\_level\_output.PartitionId ?ll} \longrightarrow \\ \quad \left( \begin{array}{l} \text{if } (ll = \text{MIN\_LOCK\_LEVEL}) \longrightarrow \\ \quad \text{general\_process\_scheduling.PartitionId} \longrightarrow \text{Skip} \\ \quad \parallel (ll > \text{MIN\_LOCK\_LEVEL} \wedge \text{ProcessTable(eprocid).} \\ \quad \text{ProcessState} \neq \text{DORMANT}) \longrightarrow \\ \quad \text{specific\_process\_scheduling.PartitionId !eprocid} \longrightarrow \text{Skip} \end{array} \right) \\ \text{fi} \end{array} \right) \\
& \text{fi}
\end{aligned}$$

$$\begin{aligned}
\text{SysCall\_Stop} \quad \hat{=} \quad & \text{system\_call\_handler\_invoke\_service\_routine\_stop.PartitionId.callerid} \longrightarrow \\
& \text{system\_call\_service\_routine\_stop\_input.PartitionId.callerid ?procid} \longrightarrow \\
& \left( \begin{array}{l} \text{if } (\text{ProcessTable(callerid).ProcessKind} = \text{ERROR\_HANDLER}) \longrightarrow \\ \quad \text{error\_process\_id ?eprocid} \longrightarrow \\ \quad \left( \begin{array}{l} \text{if } (\text{procid} = \text{eprocid}) \longrightarrow \text{StopErroredProcess(procid);} \\ \quad \text{system\_call\_service\_routine\_end.PartitionId.callerid} \longrightarrow \text{Skip} \\ \quad \parallel (\text{procid} \neq \text{eprocid} \wedge \text{ProcessTable(procid).ProcessState} = \\ \quad \text{READY}) \longrightarrow \text{StopReadyProcess(procid);} \\ \quad \text{system\_call\_service\_routine\_end.PartitionId.callerid} \longrightarrow \text{Skip} \\ \quad \parallel (\text{procid} \neq \text{eprocid} \wedge \text{ProcessTable(procid).ProcessState} = \\ \quad \text{WAITING}) \longrightarrow \text{StopWaitingProcess(procid);} \\ \quad \text{system\_call\_service\_routine\_end.PartitionId.callerid} \longrightarrow \text{Skip} \end{array} \right) \\ \quad \text{fi} \\ \parallel (\text{ProcessTable(callerid).ProcessKind} \neq \text{ERROR\_HANDLER}) \longrightarrow \\ \quad \left( \begin{array}{l} \text{if } (\text{ProcessTable(procid).ProcessState} = \text{READY}) \longrightarrow \\ \quad \text{StopReadyProcess(procid);} \\ \quad \text{system\_call\_service\_routine\_end.PartitionId.callerid} \longrightarrow \text{Skip} \\ \quad \parallel (\text{ProcessTable(procid).ProcessState} = \text{WAITING}) \longrightarrow \\ \quad \text{StopWaitingProcess(procid);} \\ \quad \text{system\_call\_service\_routine\_end.PartitionId.callerid} \longrightarrow \text{Skip} \end{array} \right) \\ \quad \text{fi} \end{array} \right) \\
& \text{fi}
\end{aligned}$$

$StopErroredProcess \hat{=} procid : PROCESS\_ID\_TYPE \bullet$   
 $core\_kernel\_service\_reset\_lock\_level.PartitionId \longrightarrow$   
 $core\_kernel\_service\_reset\_lock\_level\_return.PartitionId \longrightarrow$   
 $ProcessTable(procid).ProcessState := DORMANT$

$StopReadyProcess \hat{=} procid : PROCESS\_ID\_TYPE \bullet$   
 $DeqReadyQueue[procid/procid?]; ProcessTable(procid).ProcessState := DORMANT$

$StopWaitingProcess \hat{=} procid : PROCESS\_ID\_TYPE \bullet$   
 $\mathbf{var} \ tprocs : \mathbb{P} \ PROCESS\_ID\_TYPE \bullet$   
 $GetTimingProcess[tprocs/tprocs!];$   
 $\left( \begin{array}{l} \mathbf{if} \ (procid \notin \text{ran } WaitingQueue \wedge procid \notin tprocs) \longrightarrow \\ \quad \left( \begin{array}{l} \mathbf{if} \ (procid \in \text{ran } ReadyQueue) \longrightarrow \\ \quad DeqReadyQueue[procid/procid?]; \\ \quad ProcessTable(procid).ProcessState := DORMANT \\ \quad \parallel (procid \notin \text{ran } ReadyQueue) \longrightarrow \\ \quad \quad ProcessTable(procid).ProcessState := DORMANT \end{array} \right) \\ \quad \mathbf{fi} \\ \parallel (procid \notin \text{ran } WaitingQueue \wedge procid \in tprocs) \longrightarrow \\ \quad ProcessTable(procid).ProcessState := DORMANT; \\ \quad core\_kernel\_service\_get\_operating\_mode.PartitionId \longrightarrow \\ \quad core\_kernel\_service\_get\_operating\_mode\_return.PartitionId \longrightarrow \\ \quad core\_kernel\_service\_get\_operating\_mode\_output.PartitionId \\ \quad ?om \longrightarrow RemoveTimeCounter(procid, om) \\ \parallel (procid \in \text{ran } WaitingQueue \wedge procid \notin tprocs) \longrightarrow \\ \quad DeqWaitingQueue[procid/procid?]; \\ \quad ProcessTable(procid).ProcessState := DORMANT \\ \parallel (procid \in \text{ran } WaitingQueue \wedge procid \in tprocs) \longrightarrow \\ \quad DeqWaitingQueue[procid/procid?]; \\ \quad ProcessTable(procid).ProcessState := DORMANT; \\ \quad core\_kernel\_service\_get\_operating\_mode.PartitionId \longrightarrow \\ \quad core\_kernel\_service\_get\_operating\_mode\_return.PartitionId \longrightarrow \\ \quad core\_kernel\_service\_get\_operating\_mode\_output.PartitionId \\ \quad ?om \longrightarrow RemoveTimeCounter(procid, om) \end{array} \right)$   
 $\mathbf{fi}$

$$\begin{aligned}
\text{SysCall\_Start} &\hat{=} \text{system\_call\_handler\_invoke\_service\_routine\_start.PartitionId.callerid} \longrightarrow \\
&\text{system\_call\_service\_routine\_start\_input.PartitionId.callerid ?procid ?rp} \\
&\text{?dt ?om} \longrightarrow \\
&\left( \begin{array}{l} \text{if } (\text{ProcessTable}(\text{procid}).\text{ProcessKind} = \text{APERIODIC}) \longrightarrow \\ \quad \text{StartAperiodicProcess}(\text{procid}, \text{rp}, 0, \text{dt}, \text{om}); \\ \quad \text{system\_call\_service\_routine\_end.PartitionId.callerid} \longrightarrow \text{Skip} \\ \parallel \\ \quad (\text{ProcessTable}(\text{procid}).\text{ProcessKind} = \text{PERIODIC}) \longrightarrow \\ \quad \text{StartPeriodicProcess}(\text{procid}, \text{rp}, 0, \text{dt}, \text{om}); \\ \quad \text{system\_call\_service\_routine\_end.PartitionId.callerid} \longrightarrow \text{Skip} \\ \text{fi} \end{array} \right) \\
\\
\text{SysCall\_DelayedStart} &\hat{=} \text{system\_call\_handler\_invoke\_service\_routine\_delayed\_start.PartitionId.callerid} \longrightarrow \\
&\text{system\_call\_service\_routine\_delayed\_start\_input.PartitionId.callerid ?procid ?rp} \\
&\text{?delta ?dt ?om} \longrightarrow \\
&\left( \begin{array}{l} \text{if } (\text{ProcessTable}(\text{procid}).\text{ProcessKind} = \text{APERIODIC}) \longrightarrow \\ \quad \text{StartAperiodicProcess}(\text{procid}, \text{rp}, \text{delta}, \text{dt}, \text{om}); \\ \quad \text{system\_call\_service\_routine\_end.PartitionId.callerid} \longrightarrow \text{Skip} \\ \parallel \\ \quad (\text{ProcessTable}(\text{procid}).\text{ProcessKind} = \text{PERIODIC}) \longrightarrow \\ \quad \text{StartPeriodicProcess}(\text{procid}, \text{rp}, \text{delta}, \text{dt}, \text{om}); \\ \quad \text{system\_call\_service\_routine\_end.PartitionId.callerid} \longrightarrow \text{Skip} \\ \text{fi} \end{array} \right) \\
\\
\text{StartAperiodicProcess} &\hat{=} \text{procid : PROCESS\_ID\_TYPE, release, delta, deadline : SYSTEM\_TIME\_TYPE,} \\
&\text{om : OPERATING\_MODE\_TYPE} \bullet \\
&\text{var regstate : CPU\_REGISTER\_TYPE, pt : PAGE\_TABLE\_TYPE} \bullet \\
&\text{ProcessTable}(\text{procid}).\text{CurrentPriority} := \text{ProcessTable}(\text{procid}).\text{BasePriority}; \\
&\text{InitProcRegisterState}[(\text{ProcessTable}(\text{procid}).\text{EntryPoint})/\text{entrypoint?}, \\
&\text{ProcessTable}(\text{procid}).\text{VirtualMemory}/\text{procv?}, \text{regstate}/\text{regstate!}; \\
&\text{pt} := \text{ProcessTable}(\text{procid}).\text{VirtualMemory.VMBlock.PageTable}; \\
&\text{ProcessTable}(\text{procid}).\text{UserTempContext} := \langle \rangle; \\
&\text{ProcessTable}(\text{procid}).\text{KernelTempContext} := \langle \text{makecontext}(\text{regstate}, \text{pt}) \rangle; \\
&\left( \begin{array}{l} \text{if } (\text{om} = \text{NORMAL}) \longrightarrow \\ \quad \left( \begin{array}{l} \text{if } (\text{delta} = 0) \longrightarrow \\ \quad \text{ProcessTable}(\text{procid}).\text{ProcessState} := \text{READY}; \\ \quad \text{EnqReadyQueue}_2[\text{procid}/\text{procid?}]; \\ \quad \text{ProcessTable}(\text{procid}).\text{ReleasePoint} := \text{release}; \\ \quad \text{ProcessTable}(\text{procid}).\text{DeadlineTime} := \text{deadline}; \\ \quad \text{CheckSchedulingCondition} \\ \parallel \\ \quad (\text{delta} > 0) \longrightarrow \\ \quad \text{ProcessTable}(\text{procid}).\text{ProcessState} := \text{WAITING}; \\ \quad \text{ProcessTable}(\text{procid}).\text{ReleasePoint} := \text{release} + \text{delta}; \\ \quad \text{ProcessTable}(\text{procid}).\text{DeadlineTime} := \text{deadline}; \\ \quad \text{kernel\_request\_high\_precision\_time.PartitionId} \longrightarrow \\ \quad \text{kernel\_get\_high\_precision\_time.PartitionId ?hpt} \longrightarrow \\ \quad \text{AddTimeCounter}(\text{procid}, (\text{hpt} + \text{delta}), \text{om}) \\ \text{fi} \end{array} \right) \\ \parallel \\ \quad (\text{om} = \text{COLD\_START} \vee \text{om} = \text{WARM\_START}) \longrightarrow \\ \quad \left( \begin{array}{l} \text{if } (\text{delta} = 0) \longrightarrow \\ \quad \text{ProcessTable}(\text{procid}).\text{ProcessState} := \text{WAITING}; \\ \quad \text{EnqReadyQueue}_2[\text{procid}/\text{procid?}] \\ \parallel \\ \quad (\text{delta} > 0) \longrightarrow \\ \quad \text{ProcessTable}(\text{procid}).\text{ProcessState} := \text{WAITING}; \\ \quad \text{AddTimeCounter}(\text{procid}, \text{delta}, \text{om}) \\ \text{fi} \end{array} \right) \\ \text{fi} \end{array} \right)
\end{aligned}$$

$StartPeriodicProcess \hat{=}$   $procid : PROCESS\_ID\_TYPE, release, delta, deadline : SYSTEM\_TIME\_TYPE,$   
 $om : OPERATING\_MODE\_TYPE \bullet$   
 $\mathbf{var}$   $regstate : CPU\_REGISTER\_TYPE, pt : PAGE\_TABLE\_TYPE \bullet$   
 $ProcessTable(procid).CurrentPriority := ProcessTable(procid).BasePriority;$   
 $InitProcRegisterState[(ProcessTable(procid).EntryPoint)/entrypoint?,$   
 $ProcessTable(procid).VirtualMemory/procvm?, regstate/regstate!];$   
 $pt := ProcessTable(procid).VirtualMemory.VMBlock.PageTable;$   
 $ProcessTable(procid).UserTempContext := \langle \rangle;$   
 $ProcessTable(procid).KernelTempContext := \langle makecontext(regstate, pt) \rangle;$   
 $\left( \begin{array}{l} \mathbf{if} \ (om = NORMAL) \longrightarrow \\ \quad ProcessTable(procid).ProcessState := WAITING; \\ \quad ProcessTable(procid).ReleasePoint := release; \\ \quad ProcessTable(procid).DeadlineTime := deadline \\ \quad \parallel \ (om = COLD\_START \vee om = WARM\_START) \longrightarrow \\ \quad \quad \left( \begin{array}{l} \mathbf{if} \ (delta = 0) \longrightarrow \\ \quad \quad ProcessTable(procid).ProcessState := WAITING; \\ \quad \quad EnqReadyQueue_2[procid/procid?] \\ \quad \quad \parallel \ (delta > 0) \longrightarrow \\ \quad \quad \quad ProcessTable(procid).ProcessState := WAITING; \\ \quad \quad \quad AddTimeCounter(procid, delta, om) \\ \quad \quad \mathbf{fi} \end{array} \right) \\ \mathbf{fi} \end{array} \right)$

$SysCall\_LockPreemption \hat{=}$   $system\_call\_handler\_invoke\_service\_routine\_lock\_preemption.PartitionId.$   
 $callerid \longrightarrow$   
 $core\_kernel\_service\_increase\_lock\_level.PartitionId \longrightarrow$   
 $core\_kernel\_service\_increase\_lock\_level\_return.PartitionId \longrightarrow$   
 $core\_kernel\_service\_get\_lock\_level.PartitionId \longrightarrow$   
 $core\_kernel\_service\_get\_lock\_level\_return.PartitionId \longrightarrow$   
 $core\_kernel\_service\_get\_lock\_level\_output.PartitionId ?ll \longrightarrow$   
 $system\_call\_service\_routine\_lock\_preemption\_output.PartitionId.callerid$   
 $!ll \longrightarrow$   
 $system\_call\_service\_routine\_end.PartitionId.callerid \longrightarrow \mathbf{Skip}$

$SysCall\_UnlockPreemption \hat{=}$   $system\_call\_handler\_invoke\_service\_routine\_unlock\_preemption.PartitionId.$   
 $callerid \longrightarrow$   
 $core\_kernel\_service\_decrease\_lock\_level.PartitionId \longrightarrow$   
 $core\_kernel\_service\_decrease\_lock\_level\_return.PartitionId \longrightarrow$   
 $core\_kernel\_service\_get\_lock\_level.PartitionId \longrightarrow$   
 $core\_kernel\_service\_get\_lock\_level\_return.PartitionId \longrightarrow$   
 $core\_kernel\_service\_get\_lock\_level\_output.PartitionId ?ll \longrightarrow$   
 $system\_call\_service\_routine\_unlock\_preemption\_output.PartitionId.callerid$   
 $!ll \longrightarrow$   
 $\left( \begin{array}{l} \mathbf{if} \ (ll > MIN\_LOCK\_LEVEL) \longrightarrow \\ \quad system\_call\_service\_routine\_end.PartitionId.callerid \longrightarrow \mathbf{Skip} \\ \quad \parallel \ (ll = MIN\_LOCK\_LEVEL) \longrightarrow \\ \quad \quad general\_process\_scheduling.PartitionId \longrightarrow \\ \quad \quad system\_call\_service\_routine\_end.PartitionId.callerid \longrightarrow \mathbf{Skip} \\ \mathbf{fi} \end{array} \right)$

$SysCall\_GetMyId \hat{=}$   $system\_call\_handler\_invoke\_service\_routine\_get\_my\_id.PartitionId.callerid \longrightarrow$   
 $system\_call\_service\_routine\_get\_my\_id\_output.PartitionId.callerid !CurrentProcess \longrightarrow$   
 $system\_call\_service\_routine\_end.PartitionId.callerid \longrightarrow \mathbf{Skip}$

$SysCallServiceRoutines\_Process \hat{=}$   $SysCall\_GetProcNames$   
 $\square SysCall\_GetProcIds$   
 $\square SysCall\_GetFreeProcIds$   
 $\square SysCall\_GetFreeSpace$   
 $\square SysCall\_GetPartPeriod$   
 $\square SysCall\_GetPartDuration$   
 $\square SysCall\_GetPartSize$

$\text{SysCall\_GetCurrentTime} \hat{=} \text{var } ct : \text{SYSTEM\_TIME\_TYPE} \bullet$   
 $\text{system\_call\_handler\_invoke\_service\_routine\_get\_current\_time.PartitionId.}$   
 $\text{callerid} \longrightarrow$   
 $\text{Lock};$   
 $\text{kernel\_request\_system\_time.PartitionId} \longrightarrow$   
 $\text{kernel\_get\_system\_time.PartitionId } ?t \longrightarrow$   
 $\text{kernel\_request\_high\_precision\_time.PartitionId} \longrightarrow$   
 $\text{kernel\_get\_high\_precision\_time.PartitionId } ?hpt \longrightarrow$   
 $ct := t + hpt \bmod \text{bintsigned}(\text{ClockTickInterval});$   
 $\text{Unlock};$   
 $\text{system\_call\_service\_routine\_get\_current\_time\_output.PartitionId.callerid}$   
 $!ct \longrightarrow$   
 $\text{system\_call\_service\_routine\_end.PartitionId.callerid} \longrightarrow \text{Skip}$

$\text{SysCall\_GetPartitionTime} \hat{=} \text{system\_call\_handler\_invoke\_service\_routine\_get\_partition\_time.PartitionId.}$   
 $\text{callerid} \longrightarrow$   
 $\text{Lock};$   
 $\text{kernel\_request\_high\_precision\_time.PartitionId} \longrightarrow$   
 $\text{kernel\_get\_high\_precision\_time.PartitionId } ?hpt \longrightarrow$   
 $\text{Unlock};$   
 $\text{system\_call\_service\_routine\_get\_partition\_time\_output.PartitionId.callerid}$   
 $!hpt \longrightarrow$   
 $\text{system\_call\_service\_routine\_end.PartitionId.callerid} \longrightarrow \text{Skip}$

$\text{SysCall\_GetNextReleasePoint} \hat{=} \text{var } nrp : \text{SYSTEM\_TIME\_TYPE} \bullet$   
 $\text{system\_call\_handler\_invoke\_service\_routine\_get\_next\_release\_point.}$   
 $\text{PartitionId.callerid} \longrightarrow$   
 $\text{system\_call\_service\_routine\_get\_next\_release\_point\_input.PartitionId.}$   
 $\text{callerid } ?procid \longrightarrow$   
 $nrp := \text{ProcessTable}(procid).\text{ReleasePoint} + \text{ProcessTable}(procid).\text{Period};$   
 $\text{system\_call\_service\_routine\_get\_next\_release\_point\_output.PartitionId.}$   
 $\text{callerid } !nrp \longrightarrow$   
 $\text{system\_call\_service\_routine\_end.PartitionId.callerid} \longrightarrow \text{Skip}$



$$\begin{aligned}
\text{SysCall\_TimedWait} \quad \hat{=} \quad & \text{system\_call\_handler\_invoke\_service\_routine\_timed\_wait.PartitionId.callerid} \longrightarrow \\
& \text{system\_call\_service\_routine\_timed\_wait\_input.PartitionId.callerid ?hpt ?delta} \longrightarrow \\
& \text{ProcessTable(callerid).CurrentPriority} := - \text{ProcessTable(callerid).CurrentPriority}; \\
& \left( \begin{array}{l} \text{if } (\text{delta} = 0) \longrightarrow \\ \quad \text{ProcessTable(callerid).ProcessState} := \text{READY}; \\ \quad \text{EnqReadyQueue}_2[\text{callerid/procid?}]; \\ \quad \text{general\_process\_scheduling.PartitionId} \longrightarrow \\ \quad \text{system\_call\_service\_routine\_end.PartitionId.callerid} \longrightarrow \text{Skip} \\ \quad \parallel \\ \quad (\text{delta} > 0) \longrightarrow \\ \quad \text{ProcessTable(callerid).ProcessState} := \text{WAITING}; \\ \quad \text{AddTimeCounter(callerid, (hpt + delta), NORMAL)}; \\ \quad \text{general\_process\_scheduling.PartitionId} \longrightarrow \\ \quad \text{system\_call\_service\_routine\_end.PartitionId.callerid} \longrightarrow \text{Skip} \\ \text{fi} \end{array} \right)
\end{aligned}$$

$$\begin{aligned}
\text{SysCall\_PeriodicWait} \quad \hat{=} \quad & \text{system\_call\_handler\_invoke\_service\_routine\_periodic\_wait.PartitionId.callerid} \longrightarrow \\
& \text{system\_call\_service\_routine\_periodic\_wait\_input.PartitionId.callerid ?rp ?dt} \longrightarrow \\
& \text{ProcessTable(callerid).ProcessState} := \text{WAITING}; \\
& \text{ProcessTable(callerid).ReleasePoint} := \text{rp}; \\
& \text{ProcessTable(callerid).DeadlineTime} := \text{dt}; \\
& \text{general\_process\_scheduling.PartitionId} \longrightarrow \\
& \text{system\_call\_service\_routine\_end.PartitionId.callerid} \longrightarrow \text{Skip}
\end{aligned}$$

$$\begin{aligned}
\text{SysCall\_GetTime} \quad \hat{=} \quad & \text{system\_call\_handler\_invoke\_service\_routine\_get\_time.PartitionId.callerid} \longrightarrow \\
& \text{Lock}; \\
& \text{kernel\_request\_system\_time.PartitionId} \longrightarrow \\
& \text{kernel\_get\_system\_time.PartitionId ?t} \longrightarrow \\
& \text{Unlock}; \\
& \text{system\_call\_service\_routine\_get\_time\_output.PartitionId.callerid !t} \longrightarrow \\
& \text{system\_call\_service\_routine\_end.PartitionId.callerid} \longrightarrow \text{Skip}
\end{aligned}$$

$$\begin{aligned}
SysCall\_Replenish \quad \hat{=} \quad & system\_call\_handler\_invoke\_service\_routine\_replenish.PartitionId.callerid \longrightarrow \\
& system\_call\_service\_routine\_replenish\_input.PartitionId.callerid \ ?ct \ ?delta \longrightarrow \\
& \left( \begin{array}{l} \textbf{if} \quad (\delta < 0) \longrightarrow \\ \quad ProcessTable(callerid).DeadlineTime := \delta; \\ \quad system\_call\_service\_routine\_end.PartitionId.callerid \longrightarrow \textbf{Skip} \\ \quad \parallel \\ \quad (\delta > 0) \longrightarrow \\ \quad ProcessTable(callerid).DeadlineTime := ct + \delta; \\ \quad system\_call\_service\_routine\_end.PartitionId.callerid \longrightarrow \textbf{Skip} \\ \textbf{fi} \end{array} \right)
\end{aligned}$$

$$\begin{aligned}
SysCallServiceRoutines\_Time \quad \hat{=} \quad & SysCall\_GetCurrentTime \\
& \square SysCall\_GetPartitionTime \\
& \square SysCall\_GetNextReleasePoint \\
& \square SysCall\_TimedWait \\
& \square SysCall\_PeriodicWait \\
& \square SysCall\_GetSystemTime \\
& \square SysCall\_Replenish
\end{aligned}$$

$$SysCallServiceRoutines\_Part \quad \hat{=} \quad SysCallServiceRoutines\_Partition \square SysCallServiceRoutines\_Process$$

$$\begin{aligned}
SysCallServiceRoutines\_All \quad \hat{=} \quad & SysCallServiceRoutines\_Partition \\
& \square SysCallServiceRoutines\_Process \\
& \square SysCallServiceRoutines\_Time
\end{aligned}$$

$$\begin{aligned}
SystemCallHandle\_Pro &\hat{=}\ system\_call\_service\_routine\_end.PartitionId.callerid \longrightarrow \\
&\quad kernel\_disable\_interrupt.PartitionId \longrightarrow kernel\_disabled\_interrupt.PartitionId \longrightarrow \\
&\quad kernel\_restore\_context.PartitionId \text{ !PART !}(first(head\ ProcessTable(callerid). \\
&\quad KernelTempContext)) \text{ !(second(head}\ ProcessTable(callerid).KernelTempContext)) \longrightarrow \\
&\quad kernel\_restored\_context.PartitionId \longrightarrow \\
&\quad ProcessTable(callerid).KernelTempContext := tail\ ProcessTable(callerid). \\
&\quad KernelTempContext; \\
&\quad kernel\_enable\_interrupt.PartitionId \longrightarrow kernel\_enabled\_interrupt.PartitionId \longrightarrow \\
&\quad system\_call\_return.PartitionId.callerid \longrightarrow \mathbf{Skip}
\end{aligned}$$

$$SystemCallHandle\_Part \hat{=}\ SystemCallHandle\_Pre \llbracket SelectSysCall \rrbracket SysCallServiceRoutines\_Part \llbracket SysCallReturn \rrbracket \\
SystemCallHandle\_Pro$$

$$SystemCallHandle\_All \hat{=}\ SystemCallHandle\_Pre \llbracket SelectSysCall \rrbracket SysCallServiceRoutines\_All \llbracket SysCallReturn \rrbracket \\
SystemCallHandle\_Pro$$

$$ExecSystemCallHandle\_Part \hat{=}\ \mu X \bullet SystemCallHandle\_Part ; X$$

$$ExecSystemCallHandle\_All \hat{=}\ \mu X \bullet SystemCallHandle\_All ; X$$

$$ExecPartitionKernelService \hat{=}\ \mu X \bullet \left( \begin{array}{l} partition\_kernel\_start\_service.PartitionId?option \longrightarrow \\ (option = PART) \ \& \ ExecSystemCallHandle\_Part \\ \Delta \left( \begin{array}{l} partition\_kernel\_end\_service.PartitionId \longrightarrow \mathbf{Skip} \\ \square module\_end \longrightarrow \mathbf{Skip} \end{array} \right) \\ (option = ALL) \ \& \ ||| callerid : 0 \dots TotalProcess \bullet \\ ExecSystemCallHandle\_All \\ \Delta \left( \begin{array}{l} partition\_kernel\_end\_service.PartitionId \longrightarrow \mathbf{Skip} \\ \square module\_end \longrightarrow \mathbf{Skip} \end{array} \right) \end{array} \right) ; X$$

$$\begin{aligned}
GeneralScheduling &\hat{=}\ general\_process\_scheduling.PartitionId \longrightarrow \\
&\quad kernel\_disable\_interrupt.PartitionId \longrightarrow kernel\_disabled\_interrupt.PartitionId \longrightarrow \\
&\quad kernel\_save\_context.PartitionId \text{ !ALL} \longrightarrow \\
&\quad kernel\_saved\_context.PartitionId \text{ ?cpureg ?pt} \longrightarrow \\
&\quad ProcessTable(CurrentProcess).KernelTempContext := \langle makecontext(cpureg, pt) \rangle^{\wedge} \\
&\quad ProcessTable(CurrentProcess).KernelTempContext; \\
&\quad \left( \begin{array}{l} \mathbf{if} \ (ProcessTable(CurrentProcess).ProcessState = DORMANT) \longrightarrow \\ \quad \left( \begin{array}{l} \mathbf{if} \ (ReadyQueue = \langle \rangle) \longrightarrow ScheduleProcess(IDLE\_PROCESS\_ID) \\ \parallel \\ (ReadyQueue \neq \langle \rangle) \longrightarrow MustScheduling \\ \mathbf{fi} \end{array} \right) \\ \parallel \\ (ProcessTable(CurrentProcess).ProcessState \in \{WAITING, READY\}) \longrightarrow \\ \quad \left( \begin{array}{l} \mathbf{if} \ (ReadyQueue = \langle \rangle) \longrightarrow ScheduleProcess(IDLE\_PROCESS\_ID) \\ \parallel \\ (ReadyQueue \neq \langle \rangle) \longrightarrow MustScheduling \\ \mathbf{fi} \end{array} \right) \\ \parallel \\ (ProcessTable(CurrentProcess).ProcessState = RUNNING) \longrightarrow \\ \quad \left( \begin{array}{l} \mathbf{if} \ (ReadyQueue = \langle \rangle) \longrightarrow \\ \quad ProcessTable(CurrentProcess).CurrentPriority := | ProcessTable \\ \quad (CurrentProcess).CurrentPriority | ; \\ \quad ScheduleProcess(CurrentProcess) \\ \parallel \\ (ReadyQueue \neq \langle \rangle) \longrightarrow NeedScheduling \\ \mathbf{fi} \end{array} \right) \\ \mathbf{fi} \end{array} \right)
\end{aligned}$$

$$\begin{aligned}
MustScheduling &\hat{=}\ \mathbf{var} \ hp : PRIORITY\_TYPE \bullet \\
&\quad GetHighestPriority[hp/hp!] ; ScheduleReadyProcess(hp)
\end{aligned}$$

$NeedScheduling \hat{=} \text{var } hp : \text{PRIORITY\_TYPE} \bullet$   
 $GetHighestPriority[hp/hp!];$   
 $\left( \begin{array}{l} \text{if } (| \text{ProcessTable}(\text{CurrentProcess}).\text{CurrentPriority} | > hp) \longrightarrow \\ \quad \text{ProcessTable}(\text{CurrentProcess}).\text{CurrentPriority} := \\ \quad | \text{ProcessTable}(\text{CurrentProcess}).\text{CurrentPriority} | ; \\ \quad \text{ScheduleProcess}(\text{CurrentProcess}) \\ \square (| \text{ProcessTable}(\text{CurrentProcess}).\text{CurrentPriority} | = hp) \longrightarrow \\ \quad \left( \begin{array}{l} \text{if } (\text{ProcessTable}(\text{CurrentProcess}).\text{CurrentPriority} > 0) \longrightarrow \\ \quad \text{ScheduleProcess}(\text{CurrentProcess}) \\ \square (\text{ProcessTable}(\text{CurrentProcess}).\text{CurrentPriority} < 0) \longrightarrow \\ \quad \text{ProcessTable}(\text{CurrentProcess}).\text{CurrentPriority} := \\ \quad | \text{ProcessTable}(\text{CurrentProcess}).\text{CurrentPriority} | ; \\ \quad \text{ProcessTable}(\text{CurrentProcess}).\text{ProcessState} := \text{READY}; \\ \quad \text{EnqReadyQueue}_2[\text{CurrentProcess}/\text{procid?}]; \\ \quad \text{ScheduleReadyProcess}(hp) \end{array} \right) \\ \text{fi} \\ \square (| \text{ProcessTable}(\text{CurrentProcess}).\text{CurrentPriority} | < hp) \longrightarrow \\ \quad \left( \begin{array}{l} \text{if } (\text{ProcessTable}(\text{CurrentProcess}).\text{CurrentPriority} > 0) \longrightarrow \\ \quad \text{ProcessTable}(\text{CurrentProcess}).\text{ProcessState} := \text{READY}; \\ \quad \text{EnqReadyQueue}_1[\text{CurrentProcess}/\text{procid?}]; \\ \quad \text{ScheduleReadyProcess}(hp) \\ \square (\text{ProcessTable}(\text{CurrentProcess}).\text{CurrentPriority} < 0) \longrightarrow \\ \quad \text{ProcessTable}(\text{CurrentProcess}).\text{CurrentPriority} := \\ \quad | \text{ProcessTable}(\text{CurrentProcess}).\text{CurrentPriority} | ; \\ \quad \text{ProcessTable}(\text{CurrentProcess}).\text{ProcessState} := \text{READY}; \\ \quad \text{EnqReadyQueue}_2[\text{CurrentProcess}/\text{procid?}]; \\ \quad \text{ScheduleReadyProcess}(hp) \end{array} \right) \\ \text{fi} \end{array} \right)$   
 $\text{fi}$

$ScheduleReadyProcess \hat{=} hp : \text{PRIORITY\_TYPE} \bullet$   
 $\text{var } queue : \text{iseq}[\text{PROCESS\_ID\_TYPE}], \text{procid} : \text{PROCESS\_ID\_TYPE} \bullet$   
 $queue := (\text{ReadyQueue} \upharpoonright \{\text{procid} : \text{PROCESS\_ID\_TYPE} \mid \text{ProcessTable}(\text{procid}).$   
 $\text{CurrentPriority} = hp\}) \wedge (\text{ReadyQueue} \upharpoonright \{\text{procid} : \text{PROCESS\_ID\_TYPE} \mid$   
 $\text{ProcessTable}(\text{procid}).\text{CurrentPriority} = -hp\});$   
 $\text{procid} := \text{head } queue ; \text{DeqReadyQueue}[\text{procid}/\text{procid?}];$   
 $\text{ProcessTable}(\text{procid}).\text{CurrentPriority} := | \text{ProcessTable}(\text{procid}).\text{CurrentPriority} | ;$   
 $\text{ScheduleProcess}(\text{procid})$

$SpecialScheduling \hat{=} \text{specific\_process\_scheduling}.\text{PartitionId} ? \text{procid} \longrightarrow$   
 $\text{kernel\_disable\_interrupt}.\text{PartitionId} \longrightarrow \text{kernel\_disabled\_interrupt}.\text{PartitionId} \longrightarrow$   
 $\text{kernel\_save\_context}.\text{PartitionId} ! \text{ALL} \longrightarrow$   
 $\text{kernel\_saved\_context}.\text{PartitionId} ? \text{cpureg} ? \text{pt} \longrightarrow$   
 $\text{ProcessTable}(\text{CurrentProcess}).\text{KernelTempContext} := \langle \text{makecontext}(\text{cpureg}, \text{pt}) \rangle \wedge$   
 $\text{ProcessTable}(\text{CurrentProcess}).\text{KernelTempContext};$   
 $\text{ScheduleProcess}(\text{procid})$



$$\begin{aligned}
\text{PrepareExecution} \quad \hat{=} \quad & \text{partition\_kernel\_prepare\_execution.PartitionId} \longrightarrow \\
& \left( \begin{array}{l}
\text{if } (\text{CurrentProcess} = \text{NULL\_PROCESS\_ID}) \longrightarrow \\
\quad \text{kernel\_set\_area\_memory\_management\_reference.} \\
\quad \text{PartitionId !MemoryManagement} \longrightarrow \\
\quad \text{kernel\_have\_set\_area\_memory\_management\_reference.} \\
\quad \text{PartitionId} \longrightarrow \\
\quad \text{kernel\_reset\_high\_precision\_timer.PartitionId} \longrightarrow \\
\quad \text{kernel\_have\_reset\_high\_precision\_timer.PartitionId} \longrightarrow \\
\quad \text{partition\_kernel\_start\_service.PartitionId!PART} \longrightarrow \\
\quad \text{ScheduleProcess(IDLE\_PROCESS\_ID)} \\
\quad \square (\text{CurrentProcess} \neq \text{NULL\_PROCESS\_ID}) \longrightarrow \\
\quad \text{kernel\_set\_area\_memory\_management\_reference.} \\
\quad \text{PartitionId !MemoryManagement} \longrightarrow \\
\quad \text{kernel\_have\_set\_area\_memory\_management\_reference.} \\
\quad \text{PartitionId} \longrightarrow \\
\quad \text{kernel\_reset\_high\_precision\_timer.PartitionId} \longrightarrow \\
\quad \text{kernel\_have\_reset\_high\_precision\_timer.PartitionId} \longrightarrow \\
\quad \text{partition\_kernel\_start\_service.PartitionId!PART} \longrightarrow \\
\quad \text{ScheduleProcess(CurrentProcess)} \\
\text{fi}
\end{array} \right)
\end{aligned}$$

$$\begin{aligned}
\text{StartExecution} \quad \hat{=} \quad & \text{var procids : iseq[PROCESS\_ID\_TYPE] } \bullet \\
& \text{partition\_kernel\_start\_execution.PartitionId} \longrightarrow \\
& \text{kernel\_set\_area\_memory\_management\_reference.PartitionId !MemoryManagement} \longrightarrow \\
& \text{kernel\_have\_set\_area\_memory\_management\_reference.PartitionId} \longrightarrow \\
& \text{partition\_kernel\_update\_system\_time.PartitionId ?t} \longrightarrow \\
& \text{CheckReleasePionts[t/t?, procids/procids!]; UpdateReadyProcesses(procids);} \\
& \text{AlignTimeCounters;} \\
& \text{kernel\_reset\_high\_precision\_timer.PartitionId} \longrightarrow \\
& \text{kernel\_have\_reset\_high\_precision\_timer.PartitionId} \longrightarrow \text{UpdateTimeCounters(0);} \\
& \text{partition\_kernel\_start\_service.PartitionId!ALL} \longrightarrow \\
& \text{partition\_kernel\_start\_process\_scheduler.PartitionId} \longrightarrow \\
& \text{core\_kernel\_service\_get\_lock\_level.PartitionId} \longrightarrow \\
& \text{core\_kernel\_service\_get\_lock\_level\_return.PartitionId} \longrightarrow \\
& \text{core\_kernel\_service\_get\_lock\_level\_output.PartitionId ?ll} \longrightarrow \\
& \left( \begin{array}{l}
\text{if } (ll > \text{MIN\_LOCK\_LEVEL}) \longrightarrow \\
\quad \text{ScheduleProcess(CurrentProcess)} \\
\quad \square (ll = \text{MIN\_LOCK\_LEVEL}) \longrightarrow \text{GetHighestPriority[hp/hp!];} \\
\quad \left( \begin{array}{l}
\text{if } (hp = | \text{ProcessTable(CurrentProcess).CurrentPriority} |) \longrightarrow \\
\quad \text{ScheduleProcess(CurrentProcess)} \\
\quad \square (hp > | \text{ProcessTable(CurrentProcess).CurrentPriority} | \\
\quad \text{ProcessTable(CurrentProcess).CurrentPriority} \leq 0) \longrightarrow \\
\quad \text{ScheduleProcess(CurrentProcess)} \\
\quad \square (hp > | \text{ProcessTable(CurrentProcess).CurrentPriority} | \\
\quad \text{ProcessTable(CurrentProcess).CurrentPriority} > 0) \longrightarrow \\
\quad \text{ProcessTable(CurrentProcess).ProcessState := READY;} \\
\quad \text{EnqReadyQueue}_1[\text{CurrentProcess/procid?}]; \\
\quad \text{ScheduleReadyProcess(hp)} \\
\text{fi}
\end{array} \right) \\
\text{fi}
\end{array} \right)
\end{aligned}$$

$ContinueExecution \hat{=} \text{var } hp : \text{PRIORITY\_TYPE} \bullet$   
 $\text{partition\_kernel\_continue\_execution.PartitionId} \longrightarrow$   
 $\text{kernel\_request\_interrupt\_time.PartitionId} \longrightarrow$   
 $\text{kernel\_get\_interrupt\_time.PartitionId} \text{ ?hpt } \longrightarrow \text{UpdateTimeCounters(hpt);}$   
 $\text{core\_kernel\_service\_get\_lock\_level.PartitionId} \longrightarrow$   
 $\text{core\_kernel\_service\_get\_lock\_level\_return.PartitionId} \longrightarrow$   
 $\text{core\_kernel\_service\_get\_lock\_level\_output.PartitionId} \text{ ?ll} \longrightarrow$   
 $\left( \begin{array}{l} \text{if } (ll > \text{MIN\_LOCK\_LEVEL}) \longrightarrow \\ \quad \text{kernel\_continue\_interrupted\_process.PartitionId} \longrightarrow \text{Skip} \\ \quad \square \quad (ll = \text{MIN\_LOCK\_LEVEL}) \longrightarrow \text{GetHighestPriority}[hp/hp!]; \\ \quad \left( \begin{array}{l} \text{if } (hp = | \text{ProcessTable}(\text{CurrentProcess}).\text{CurrentPriority} |) \longrightarrow \\ \quad \text{kernel\_continue\_interrupted\_process.PartitionId} \longrightarrow \text{Skip} \\ \quad \square \quad (hp > | \text{ProcessTable}(\text{CurrentProcess}).\text{CurrentPriority} | \\ \quad \wedge \text{ProcessTable}(\text{CurrentProcess}).\text{CurrentPriority} \leq 0) \longrightarrow \\ \quad \text{kernel\_continue\_interrupted\_process.PartitionId} \longrightarrow \text{Skip} \\ \quad \square \quad (hp > | \text{ProcessTable}(\text{CurrentProcess}).\text{CurrentPriority} | \\ \quad \wedge \text{ProcessTable}(\text{CurrentProcess}).\text{CurrentPriority} > 0) \longrightarrow \\ \quad \text{kernel\_request\_interrupted\_process\_context.PartitionId} \longrightarrow \\ \quad \text{kernel\_get\_interrupted\_process\_context.PartitionId} \text{ ?cpureg} \\ \quad \text{?pt} \longrightarrow \\ \quad \text{ProcessTable}(\text{CurrentProcess}).\text{KernelTempContext} := \\ \quad \langle \text{makecontext}(\text{cpureg}, \text{pt}) \rangle \wedge \text{ProcessTable}(\text{CurrentProcess}). \\ \quad \text{KernelTempContext}; \\ \quad \text{ProcessTable}(\text{CurrentProcess}).\text{ProcessState} := \text{READY}; \\ \quad \text{EnqReadyQueue}_1[\text{CurrentProcess}/\text{procid?}]; \\ \quad \text{ScheduleReadyProcess}(hp) \end{array} \right) \\ \text{fi} \end{array} \right)$   
 $\text{fi}$

$SuspendExecution \hat{=} \text{partition\_kernel\_suspend\_execution.PartitionId} \longrightarrow$   
 $\text{kernel\_end\_high\_precision\_timer.PartitionId} \longrightarrow$   
 $\text{kernel\_ended\_high\_precision\_timer.PartitionId} \longrightarrow$   
 $\text{partition\_kernel\_end\_service.PartitionId} \longrightarrow$   
 $\text{partition\_kernel\_end\_process\_scheduler.PartitionId} \longrightarrow$   
 $\text{kernel\_request\_interrupted\_process\_context.PartitionId} \longrightarrow$   
 $\text{kernel\_get\_interrupted\_process\_context.PartitionId} \text{ ?cpureg ?pt} \longrightarrow$   
 $\text{ProcessTable}(\text{CurrentProcess}).\text{KernelTempContext} := \langle \text{makecontext}(\text{cpureg}, \text{pt}) \rangle \wedge$   
 $\text{ProcessTable}(\text{CurrentProcess}).\text{KernelTempContext};$   
 $\text{kernel\_request\_area\_memory\_management\_reference.PartitionId} \longrightarrow$   
 $\text{kernel\_get\_area\_memory\_management\_reference.PartitionId} \text{ ?areamm} \longrightarrow$   
 $\text{MemoryManagement} := \text{areamm}$   
 $\text{partition\_kernel\_suspended\_execution.PartitionId} \longrightarrow \text{Skip}$

$IdleExecution \hat{=} \text{partition\_kernel\_idle\_execution.PartitionId} \longrightarrow \text{ScheduleProcess}(\text{IDLE\_PROCESS\_ID})$

$PartitionControl \hat{=} \text{PrepareExecution}$   
 $\square \text{StartExecution}$   
 $\square \text{ContinueExecution}$   
 $\square \text{SuspendExecution}$   
 $\square \text{IdleExecution}$

$ExecPartitionControl \hat{=} \mu X \bullet \text{PartitionControl}; X$

$\bullet \text{module\_init} \longrightarrow (\text{Initialize}; \text{ExecPartitionControl}) \Delta \text{module\_end} \longrightarrow \text{Skip}$

end

### D.3.4 ChannelSets for communication between different parts of ARINC 653 O/S Layer

```

channelset CORE_KERNEL_SERVICE == { core_kernel_init_partition_kernel,
                                     core_kernel_init_partition_kernel,
                                     core_kernel_service_get_operating_mode,
                                     core_kernel_service_get_operating_mode_output,
                                     core_kernel_service_get_operating_mode_return,
                                     core_kernel_service_get_partition_status,
                                     core_kernel_service_get_partition_status_output,
                                     core_kernel_service_get_partition_status_return,
                                     core_kernel_service_set_operating_mode,
                                     core_kernel_service_set_operating_mode_input,
                                     core_kernel_service_set_operating_mode_return,
                                     core_kernel_service_get_next_periodic_start,
                                     core_kernel_service_get_next_periodic_start_output,
                                     core_kernel_service_get_next_periodic_start_return,
                                     core_kernel_service_get_delayed_periodic_start,
                                     core_kernel_service_get_delayed_periodic_start_input,
                                     core_kernel_service_get_delayed_periodic_start_output,
                                     core_kernel_service_get_delayed_periodic_start_return,
                                     core_kernel_service_get_lock_level,
                                     core_kernel_service_get_lock_level_output,
                                     core_kernel_service_get_lock_level_return,
                                     core_kernel_service_reset_lock_level,
                                     core_kernel_service_reset_lock_level_return,
                                     core_kernel_service_increase_lock_level,
                                     core_kernel_service_increase_lock_level_return,
                                     core_kernel_service_decrease_lock_level,
                                     core_kernel_service_decrease_lock_level_return }

channelset CORE_KERNEL_CONTROL == { partition_kernel_continue_execution,
                                     partition_kernel_suspend_execution,
                                     partition_kernel_suspended_execution,
                                     partition_kernel_idle_execution,
                                     partition_kernel_prepare_execution,
                                     partition_kernel_update_system_time,
                                     partition_kernel_start_execution }

channelset OSLayerChannels == CORE_KERNEL_SERVICE ∪ CORE_KERNEL_CONTROL

```

### D.3.5 ARINC 653 O/S Layer Model

**process** *ARINC653\_OS\_Layer*  $\hat{=}$  *OSKernelConfig* : *OS\_KERNEL\_CONFIG\_TYPE* •

*CoreKernel*(*OSKernelConfig*)  $\llbracket$  *OSLayerChannels*  $\rrbracket$  ( $\llbracket$  *partid* : *dom*(*OSKernelConfig.Partitions*) •  
*PartitionKernel*(*partid*, *OSKernelConfig.Partitions*(*partid*)))



## D.4 Application/Executive(APEX) Layer

### D.4.1 Application/Executive(APEX) Interface

**process** *APEX\_Interface*  $\hat{=}$  *partid* : *PARTITION\_ID\_TYPE*; *callerid* : *PROCESS\_ID\_TYPE* •  
**begin**

*GetPartitionStatus*  $\hat{=}$  *apex\_function\_get\_partition\_status.partid.callerid*  $\longrightarrow$   
*system\_call.partid.callerid !GET\_PARTITION\_STATUS*  $\longrightarrow$   
*system\_call\_return.partid.callerid*  $\longrightarrow$   
*system\_call\_service\_routine\_get\_partition\_status\_output.partid.callerid ?parts*  $\longrightarrow$   
*apex\_function\_get\_partition\_status\_output.partid.callerid !parts*  $\longrightarrow$   
*apex\_function\_return\_code.partid.callerid !NO\_ERROR*  $\longrightarrow$   
*apex\_function\_get\_partition\_status\_return.partid.callerid*  $\longrightarrow$  **Skip**

$$\begin{aligned}
\text{SetOperatingMode} \quad \hat{=} \quad & \text{apex\_function\_set\_operating\_mode.partid.callerid} \longrightarrow \\
& \text{apex\_function\_set\_operating\_mode\_input.partid.callerid} \text{ ?nom} \longrightarrow \\
& \left( \begin{array}{l}
\text{if } (\text{nom} \notin \text{OPERATING\_MODE\_TYPE}) \longrightarrow \\
\quad \text{apex\_function\_return\_code.partid.callerid} \text{ !INVALID\_PARAM} \longrightarrow \\
\quad \text{apex\_function\_set\_operating\_mode\_return.partid.callerid} \longrightarrow \text{Skip} \\
\quad \square (\text{nom} \in \text{OPERATING\_MODE\_TYPE}) \longrightarrow \\
\quad \quad \text{system\_call.partid.callerid} \text{ !GET\_OPERATING\_MODE} \longrightarrow \\
\quad \quad \text{system\_call\_return.partid.callerid} \longrightarrow \\
\quad \quad \text{system\_call\_service\_routine\_get\_operating\_mode\_output.partid.callerid} \\
\quad \quad \text{?om} \longrightarrow \\
\quad \left( \begin{array}{l}
\text{if } (\text{om} = \text{NORMAL}) \longrightarrow \\
\quad \left( \begin{array}{l}
\text{if } (\text{nom} = \text{NORMAL}) \longrightarrow \\
\quad \text{apex\_function\_return\_code.partid.callerid} \text{ !NO\_} \\
\quad \text{ACTION} \longrightarrow \\
\quad \text{apex\_function\_set\_operating\_mode\_return.partid.} \\
\quad \text{callerid} \longrightarrow \text{Skip} \\
\quad \square (\text{nom} \neq \text{NORMAL}) \longrightarrow \\
\quad \quad \text{apex\_function\_return\_code.partid.callerid} \text{ !NO\_} \\
\quad \quad \text{ERROR} \longrightarrow \\
\quad \quad \text{system\_call\_service\_routine\_set\_operating\_mode\_} \\
\quad \quad \text{input.partid.callerid} \text{ !nom} \longrightarrow \\
\quad \quad \text{system\_call.partid.callerid} \text{ !SET\_OPERATING\_} \\
\quad \quad \text{MODE} \longrightarrow \text{Skip}
\end{array} \right) \\
\quad \text{fi}
\end{array} \right) \\
\quad \square (\text{om} = \text{COLD\_START}) \longrightarrow \\
\quad \left( \begin{array}{l}
\text{if } (\text{nom} = \text{WARM\_START}) \longrightarrow \\
\quad \text{apex\_function\_return\_code.partid.callerid} \\
\quad \text{!INVALID\_MODE} \longrightarrow \\
\quad \text{apex\_function\_set\_operating\_mode\_return.partid.} \\
\quad \text{callerid} \longrightarrow \text{Skip} \\
\quad \square (\text{nom} \neq \text{WARM\_START}) \longrightarrow \\
\quad \quad \text{apex\_function\_return\_code.partid.callerid} \text{ !NO\_} \\
\quad \quad \text{ERROR} \longrightarrow \\
\quad \quad \text{system\_call\_service\_routine\_set\_operating\_mode\_} \\
\quad \quad \text{input.partid.callerid} \text{ !nom} \longrightarrow \\
\quad \quad \text{system\_call.partid.callerid} \text{ !SET\_OPERATING\_} \\
\quad \quad \text{MODE} \longrightarrow \text{Skip}
\end{array} \right) \\
\quad \text{fi} \\
\quad \square (\text{om} = \text{WARM\_START}) \longrightarrow \\
\quad \quad \text{apex\_function\_return\_code.partid.callerid} \text{ !NO\_ERROR} \longrightarrow \\
\quad \quad \text{system\_call\_service\_routine\_set\_operating\_mode\_input.} \\
\quad \quad \text{partid.callerid} \text{ !nom} \longrightarrow \\
\quad \quad \text{system\_call.partid.callerid} \text{ !SET\_OPERATING\_MODE} \longrightarrow \\
\quad \quad \text{Skip}
\end{array} \right) \\
& \text{fi}
\end{aligned}$$

$$\begin{aligned}
\text{GetProcessId} \quad \hat{=} \quad & \text{apex\_function\_get\_process\_id.partid.callerid} \longrightarrow \\
& \text{apex\_function\_get\_process\_id\_input.partid.callerid} \text{ ?procn} \longrightarrow \\
& \text{system\_call.partid.callerid} \text{ !GET\_PROCESS\_NAMES} \longrightarrow \\
& \text{system\_call\_return.partid.callerid} \longrightarrow \\
& \text{system\_call\_service\_routine\_get\_process\_names\_output.partid.callerid} \text{ ?procns} \longrightarrow \\
& \left( \begin{array}{l} \text{if } (\text{procn} \notin \text{procns}) \longrightarrow \\ \quad \text{apex\_function\_get\_process\_id\_output.partid.callerid} \text{ !NULL\_PROCESS\_ID} \longrightarrow \\ \quad \text{apex\_function\_return\_code.partid.callerid} \text{ !INVALID\_CONFIG} \longrightarrow \\ \quad \text{apex\_function\_get\_process\_id\_return.partid.callerid} \longrightarrow \text{Skip} \\ \quad \square (\text{procn} \in \text{procns}) \longrightarrow \\ \quad \quad \text{system\_call\_service\_routine\_get\_process\_id\_input.partid.callerid} \text{ !procn} \longrightarrow \\ \quad \quad \text{system\_call.partid.callerid} \text{ !GET\_PROCESS\_ID} \longrightarrow \\ \quad \quad \text{system\_call\_return.partid.callerid} \longrightarrow \\ \quad \quad \text{system\_call\_service\_routine\_get\_process\_id\_output.partid.callerid} \text{ ?procid} \longrightarrow \\ \quad \quad \text{apex\_function\_get\_process\_id\_output.partid.callerid} \text{ !procid} \longrightarrow \\ \quad \quad \text{apex\_function\_return\_code.partid.callerid} \text{ !NO\_ERROR} \longrightarrow \\ \quad \quad \text{apex\_function\_get\_process\_id\_return.partid.callerid} \longrightarrow \text{Skip} \\ \text{fi} \end{array} \right)
\end{aligned}$$

$$\begin{aligned}
\text{GetProcessStatus} \quad \hat{=} \quad & \text{apex\_function\_get\_process\_status.partid.callerid} \longrightarrow \\
& \text{apex\_function\_get\_process\_status\_input.partid.callerid} \text{ ?procid} \longrightarrow \\
& \text{system\_call.partid.callerid} \text{ !GET\_PROCESS\_IDS} \longrightarrow \\
& \text{system\_call\_return.partid.callerid} \longrightarrow \\
& \text{system\_call\_service\_routine\_get\_process\_ids\_output.partid.callerid} \text{ ?procids} \longrightarrow \\
& \left( \begin{array}{l} \text{if } (\text{procid} \notin \text{procids}) \longrightarrow \\ \quad \text{apex\_function\_get\_process\_status\_output.partid.callerid} \text{ !NULL\_} \\ \quad \text{PROCESS\_STATUS} \longrightarrow \\ \quad \text{apex\_function\_return\_code.partid.callerid} \text{ !INVALID\_PARAM} \longrightarrow \\ \quad \text{apex\_function\_get\_process\_status\_return.partid.callerid} \longrightarrow \text{Skip} \\ \quad \square (\text{procid} \in \text{procids}) \longrightarrow \\ \quad \quad \text{system\_call\_service\_routine\_get\_process\_status\_input.partid.} \\ \quad \quad \text{callerid} \text{ !procid} \longrightarrow \\ \quad \quad \text{system\_call.partid.callerid} \text{ !GET\_PROCESS\_STATUS} \longrightarrow \\ \quad \quad \text{system\_call\_return.partid.callerid} \longrightarrow \\ \quad \quad \text{system\_call\_service\_routine\_get\_process\_status\_output.partid.} \\ \quad \quad \text{callerid} \text{ ?procs} \longrightarrow \\ \quad \quad \text{apex\_function\_get\_process\_status\_output.partid.callerid} \text{ !procs} \longrightarrow \\ \quad \quad \text{apex\_function\_return\_code.partid.callerid} \text{ !NO\_ERROR} \longrightarrow \\ \quad \quad \text{apex\_function\_get\_process\_status\_return.partid.callerid} \longrightarrow \text{Skip} \\ \text{fi} \end{array} \right)
\end{aligned}$$

$\text{CreateProcess} \hat{=} \text{var } \text{procsz} : \text{UNSIGNED\_INTEGER\_TYPE} \bullet$   
 $\text{apex\_function\_create\_process.partid.callerid} \longrightarrow$   
 $\text{apex\_function\_create\_process\_input.partid.callerid} \text{ ?proca ?exfilepath ?swapfilepath} \longrightarrow$   
 $\text{apex\_function\_request\_executable\_file.partid.callerid !exfilepath} \longrightarrow$   
 $\text{apex\_function\_get\_executable\_file.partid.callerid ?exfile} \longrightarrow$   
 $\text{procsz} := (\text{proca.StackSize}) + \#(\text{exfile.Data}) + \#(\text{exfile.Code});$   
 $\text{system\_call.partid.callerid !GET\_FREE\_SPACE} \longrightarrow$   
 $\text{system\_call\_return.partid.callerid} \longrightarrow$   
 $\text{system\_call\_service\_routine\_get\_free\_space\_output.partid.callerid} \text{ ?discontinuous}$   
 $\text{?continuous} \longrightarrow$   
 $\left( \begin{array}{l} \text{if } (\text{continuous} < \text{KERNEL\_STACK\_SIZE} \vee \text{discontinuous} < \text{procsz}) \longrightarrow \\ \quad \text{apex\_function\_create\_process\_output.partid.callerid !NULL\_PROCESS\_ID} \longrightarrow \\ \quad \text{apex\_function\_return\_code.partid.callerid !INVALID\_CONFIG} \longrightarrow \\ \quad \text{apex\_function\_create\_process\_return.partid.callerid} \longrightarrow \text{Skip} \\ \quad \parallel (\text{continuous} \geq \text{KERNEL\_STACK\_SIZE} \wedge \text{discontinuous} \geq \text{procsz}) \longrightarrow \\ \quad \quad \text{system\_call.partid.callerid !GET\_OPERATING\_MODE} \longrightarrow \\ \quad \quad \text{system\_call\_return.partid.callerid} \longrightarrow \\ \quad \quad \text{system\_call\_service\_routine\_get\_operating\_mode\_output.partid.callerid} \text{ ?om} \longrightarrow \\ \quad \quad \left( \begin{array}{l} \text{if } (\text{om} = \text{NORMAL}) \longrightarrow \\ \quad \text{apex\_function\_create\_process\_output.partid.callerid !NULL\_} \\ \quad \text{PROCESS\_ID} \longrightarrow \\ \quad \text{apex\_function\_return\_code.partid.callerid !INVALID\_MODE} \longrightarrow \\ \quad \text{apex\_function\_create\_process\_return.partid.callerid} \longrightarrow \text{Skip} \\ \quad \parallel (\text{om} = \text{COLD\_START} \vee \text{om} = \text{WARM\_START}) \longrightarrow \\ \quad \quad \text{CheckProcessAttributes}(\text{proca}, \text{exfile}, \text{exfilepath}, \text{swapfilepath}) \end{array} \right) \\ \text{fi} \end{array} \right)$   
 $\text{fi}$

$\text{CheckProcessAttribute} \hat{=} \text{proca} : \text{PROCESS\_ATTRIBUTE\_TYPE}, \text{exfile} : \text{EXECUTABLE\_FILE\_TYPE},$   
 $\text{exfilepath}, \text{swapfilepath} : \text{PATH\_TYPE} \bullet$   
 $\text{system\_call.partid.callerid !GET\_PROCESS\_NAMES} \longrightarrow$   
 $\text{system\_call\_return.partid.callerid} \longrightarrow$   
 $\text{system\_call\_service\_routine\_get\_process\_names\_output.partid.callerid} \text{ ?procns} \longrightarrow$   
 $\left( \begin{array}{l} \text{if } ((\text{proca.Name}) \in \text{procns}) \longrightarrow \\ \quad \text{apex\_function\_create\_process\_output.partid.callerid !NULL\_PROCESS\_} \\ \quad \text{ID} \longrightarrow \\ \quad \text{apex\_function\_return\_code.partid.callerid !NO\_ACTION} \longrightarrow \\ \quad \text{apex\_function\_create\_process\_return.partid.callerid} \longrightarrow \text{Skip} \\ \quad \parallel ((\text{proca.Name}) \notin \text{procns}) \longrightarrow \\ \quad \quad \left( \begin{array}{l} \text{if } ((\text{proca.StackSize}) \notin \text{STACK\_SIZE\_RANGE} \vee (\text{proca.} \\ \text{BasePriority}) \notin \text{PRIORITY\_RANGE}) \longrightarrow \\ \quad \text{apex\_function\_create\_process\_output.partid.callerid !NULL\_} \\ \quad \text{PROCESS\_ID} \longrightarrow \\ \quad \text{apex\_function\_return\_code.partid.callerid !INVALID\_PARAM} \\ \quad \longrightarrow \\ \quad \text{apex\_function\_create\_process\_return.partid.callerid} \longrightarrow \text{Skip} \\ \quad \parallel ((\text{proca.StackSize}) \in \text{STACK\_SIZE\_RANGE} \wedge (\text{proca.} \\ \text{BasePriority}) \in \text{PRIORITY\_RANGE}) \longrightarrow \\ \quad \quad \text{CheckProcessTimeAttributes}(\text{proca}, \text{exfile}, \text{exfilepath}, \\ \text{swapfilepath}) \end{array} \right) \\ \text{fi} \end{array} \right)$   
 $\text{fi}$

$$\begin{aligned}
\text{CheckProcessTimeAttribute} &\hat{=} \text{proca} : \text{PROCESS\_ATTRIBUTE\_TYPE}, \text{exefile} : \text{EXECUTABLE\_FILE\_TYPE}, \\
&\quad \text{exefilepath}, \text{swapfilepath} : \text{PATH\_TYPE} \bullet \\
&\quad \left( \begin{array}{l} \text{if } (\text{proca.ProcessKind} = \text{APERIODIC}) \longrightarrow \\ \quad \text{CheckAperiodicProcTimeAttribute}(\text{proca}, \text{exefile}, \text{exefilepath}, \text{swapfilepath}) \\ \quad \square (\text{proca.ProcessKind} = \text{PERIODIC}) \longrightarrow \\ \quad \text{CheckPeriodicProcTimeAttribute}(\text{proca}, \text{exefile}, \text{exefilepath}, \text{swapfilepath}) \\ \text{fi} \end{array} \right) \\
\\
\text{CheckAperiodicProcTimeAttribute} &\hat{=} \text{proca} : \text{PROCESS\_ATTRIBUTE\_TYPE}, \text{exefile} : \text{EXECUTABLE\_FILE\_TYPE}, \\
&\quad \text{exefilepath}, \text{swapfilepath} : \text{PATH\_TYPE} \bullet \\
&\quad \left( \begin{array}{l} \text{if } (\text{proca.TimeCapacity} = 0 \vee \text{proca.TimeCapacity} \notin \text{SYSTEM\_TIME\_TYPE}) \longrightarrow \\ \quad \text{apex\_function\_create\_process\_output.partid.callerid} \text{ !NULL\_PROCESS\_ID} \longrightarrow \\ \quad \text{apex\_function\_return\_code.partid.callerid} \text{ !INVALID\_PARAM} \longrightarrow \\ \quad \text{apex\_function\_create\_process\_return.partid.callerid} \longrightarrow \text{Skip} \\ \quad \square (\text{proca.TimeCapacity} \neq 0 \wedge \text{proca.TimeCapacity} \in \text{SYSTEM\_TIME\_TYPE}) \longrightarrow \\ \quad \text{system\_call\_service\_routine\_create\_process\_input.partid.callerid} \text{ !proca !exefile !exefilepath !swapfilepath} \longrightarrow \\ \quad \text{system\_call.partid.callerid} \text{ !CREATE\_PROCESS} \longrightarrow \\ \quad \text{system\_call\_return.partid.callerid} \longrightarrow \\ \quad \text{system\_call\_service\_routine\_create\_process\_output.partid.callerid} \text{ ?procid} \longrightarrow \\ \quad \text{apex\_function\_create\_process\_output.partid.callerid} \text{ !procid} \longrightarrow \\ \quad \text{apex\_function\_return\_code.partid.callerid} \text{ !NO\_ERROR} \longrightarrow \\ \quad \text{apex\_function\_create\_process\_return.partid.callerid} \longrightarrow \text{Skip} \\ \text{fi} \end{array} \right)
\end{aligned}$$

$$\begin{aligned}
\text{CheckPeriodicProcTimeAttribute} \quad \hat{=} \quad & \text{proca} : \text{PROCESS\_ATTRIBUTE\_TYPE}, \text{exefile} : \text{EXECUTABLE\_FILE\_} \\
& \text{TYPE}, \text{exefilepath}, \text{swapfilepath} : \text{PATH\_TYPE} \bullet \\
& \left( \begin{array}{l}
\text{if } (\text{proca}.\text{TimeCapacity} \leq 0 \vee \text{proca}.\text{TimeCapacity} > \text{proca}.\text{Period}) \longrightarrow \\
\quad \text{apex\_function\_create\_process\_output.partid.callerid !NULL\_} \\
\quad \text{PROCESS\_ID} \longrightarrow \\
\quad \text{apex\_function\_return\_code.partid.callerid !INVALID\_PARAM} \longrightarrow \\
\quad \text{apex\_function\_create\_process\_return.partid.callerid} \longrightarrow \text{Skip} \\
\quad \square (\text{proca}.\text{TimeCapacity} > 0 \wedge \text{proca}.\text{TimeCapacity} \leq \text{proca}.\text{Period}) \longrightarrow \\
\quad \text{system\_call.partid.callerid !GET\_PARTITION\_PERIOD} \longrightarrow \\
\quad \text{system\_call\_return.partid.callerid} \longrightarrow \\
\quad \text{system\_call\_service\_routine\_get\_partition\_period\_output.partid.} \\
\quad \text{callerid ?partp} \longrightarrow \\
\quad \left( \begin{array}{l}
\text{if } (\text{proca}.\text{Period} \bmod \text{partp} \neq 0) \longrightarrow \\
\quad \text{apex\_function\_create\_process\_output.partid.callerid} \\
\quad \text{!NULL\_PROCESS\_ID} \longrightarrow \\
\quad \text{apex\_function\_return\_code.partid.callerid !INVALID\_} \\
\quad \text{PARAM} \longrightarrow \\
\quad \text{apex\_function\_create\_process\_return.partid.callerid} \longrightarrow \\
\quad \text{Skip} \\
\quad \square (\text{proca}.\text{Period} \bmod \text{partp} = 0) \longrightarrow \\
\quad \text{system\_call\_service\_routine\_create\_process\_input.partid.} \\
\quad \text{callerid !proca !exefile !exefilepath !swapfilepath} \longrightarrow \\
\quad \text{system\_call.partid.callerid !CREATE\_PROCESS} \longrightarrow \\
\quad \text{system\_call\_return.partid.callerid} \longrightarrow \\
\quad \text{system\_call\_service\_routine\_create\_process\_output.partid.} \\
\quad \text{callerid ?procid} \longrightarrow \\
\quad \text{apex\_function\_create\_process\_output.partid.callerid} \\
\quad \text{!procid} \longrightarrow \\
\quad \text{apex\_function\_return\_code.partid.callerid !NO\_ERROR} \\
\quad \longrightarrow \\
\quad \text{apex\_function\_create\_process\_return.partid.callerid} \longrightarrow \\
\quad \text{Skip}
\end{array} \right) \\
\text{fi}
\end{array} \right)
\end{aligned}$$

$$\begin{aligned}
\text{SetPriority} \quad \hat{=} \quad & \text{apex\_function\_set\_priority.partid.callerid} \longrightarrow \\
& \text{apex\_function\_set\_priority\_input.partid.callerid ?procid ?p} \longrightarrow \\
& \text{system\_call.partid.callerid !GET\_PROCESS\_IDS} \longrightarrow \\
& \text{system\_call\_return.partid.callerid} \longrightarrow \\
& \text{system\_call\_service\_routine\_get\_process\_ids\_output.partid.callerid ?procids} \longrightarrow \\
& \left( \begin{array}{l} \text{if } (\text{procid} \notin \text{procids} \vee p \notin \text{PRIORITY\_RANGE}) \longrightarrow \\ \quad \text{apex\_function\_return\_code.partid.callerid !INVALID\_PARAM} \longrightarrow \\ \quad \text{apex\_function\_set\_priority\_return.partid.callerid} \longrightarrow \mathbf{Skip} \\ \quad \parallel (\text{procid} \in \text{procids} \wedge p \in \text{PRIORITY\_RANGE}) \longrightarrow \\ \quad \text{system\_call\_service\_routine\_get\_process\_state\_input.partid.callerid !procid} \longrightarrow \\ \quad \text{system\_call.partid.callerid !GET\_PROCESS\_STATE} \longrightarrow \\ \quad \text{system\_call\_return.partid.callerid} \longrightarrow \\ \quad \text{system\_call\_service\_routine\_get\_process\_state\_output.partid.callerid ?procs} \longrightarrow \\ \quad \left( \begin{array}{l} \text{if } (\text{procs} = \text{DORMANT}) \longrightarrow \\ \quad \text{apex\_function\_return\_code.partid.callerid !INVALID\_MODE} \longrightarrow \\ \quad \text{apex\_function\_set\_priority\_return.partid.callerid} \longrightarrow \mathbf{Skip} \\ \quad \parallel (\text{procs} \neq \text{DORMANT}) \longrightarrow \\ \quad \text{system\_call\_service\_routine\_set\_priority\_input.partid.callerid !procid} \\ \quad \text{!p} \longrightarrow \\ \quad \text{system\_call.partid.callerid !SET\_PRIORITY} \longrightarrow \\ \quad \text{system\_call\_return.partid.callerid} \longrightarrow \\ \quad \text{apex\_function\_return\_code.partid.callerid !NO\_ERROR} \longrightarrow \\ \quad \text{apex\_function\_set\_priority\_return.partid.callerid} \longrightarrow \mathbf{Skip} \end{array} \right) \\ \text{fi} \end{array} \right) \\
& \text{fi}
\end{aligned}$$

$$\begin{aligned}
\text{SuspendSelf} \quad \hat{=} \quad & \text{apex\_function\_suspend\_self.partid.callerid} \longrightarrow \\
& \text{apex\_function\_suspend\_self\_input.partid.callerid ?to} \longrightarrow \\
& \text{system\_call.partid.callerid !GET\_PARTITION\_LOCK\_LEVEL} \longrightarrow \\
& \text{system\_call\_return.partid.callerid} \longrightarrow \\
& \text{system\_call\_service\_routine\_get\_partition\_lock\_level\_output.partid.callerid ?ll} \longrightarrow \\
& \text{system\_call.partid.callerid !GET\_MY\_ID} \longrightarrow \\
& \text{system\_call\_return.partid.callerid} \longrightarrow \\
& \text{system\_call\_service\_routine\_get\_my\_id\_output.partid.callerid ?myid} \longrightarrow \\
& \text{system\_call\_service\_routine\_get\_process\_kind\_input.partid.callerid !myid} \longrightarrow \\
& \text{system\_call.partid.callerid !GET\_PROCESS\_KIND} \longrightarrow \\
& \text{system\_call\_return.partid.callerid} \longrightarrow \\
& \text{system\_call\_service\_routine\_get\_process\_kind\_output.partid.callerid ?mykind} \longrightarrow \\
& \left( \text{if } (ll > \text{MIN\_LOCK\_LEVEL} \vee \text{mykind} \in \{\text{PERIODIC}, \text{ERROR\_HANDLER}\}) \longrightarrow \right. \\
& \quad \text{apex\_function\_return\_code.partid.callerid !INVALID\_MODE} \longrightarrow \\
& \quad \text{apex\_function\_suspend\_self\_return.partid.callerid} \longrightarrow \text{Skip} \\
& \quad \square (ll = \text{MIN\_LOCK\_LEVEL} \wedge \text{mykind} = \text{APERIODIC}) \longrightarrow \\
& \quad \text{system\_call.partid.callerid !GET\_PARTITION\_TIME} \longrightarrow \\
& \quad \text{system\_call\_return.partid.callerid} \longrightarrow \\
& \quad \text{system\_call\_service\_routine\_get\_partition\_time\_output.partid.callerid ?pt} \longrightarrow \\
& \quad \left( \text{if } (to < 0) \longrightarrow \right. \\
& \quad \quad \text{system\_call\_service\_routine\_suspend\_self\_input.partid.callerid !pt !to} \\
& \quad \quad \text{system\_call.partid.callerid !SUSPEND\_SELF} \longrightarrow \\
& \quad \quad \text{system\_call\_return.partid.callerid} \longrightarrow \\
& \quad \quad \text{system\_call\_service\_routine\_suspend\_self\_output.partid.callerid ?result} \\
& \quad \quad \longrightarrow \\
& \quad \quad \left( \text{if } (result = \text{TRUE}) \longrightarrow \right. \\
& \quad \quad \quad \text{apex\_function\_return\_code.partid.callerid !NO\_ERROR} \longrightarrow \\
& \quad \quad \quad \text{apex\_function\_suspend\_self\_return.partid.callerid} \longrightarrow \text{Skip} \\
& \quad \quad \quad \square (result = \text{FALSE}) \longrightarrow \\
& \quad \quad \quad \text{apex\_function\_return\_code.partid.callerid !TIMED\_OUT} \\
& \quad \quad \quad \longrightarrow \\
& \quad \quad \quad \text{apex\_function\_suspend\_self\_return.partid.callerid} \longrightarrow \text{Skip} \\
& \quad \quad \text{fi} \\
& \quad \quad \square (to > 0 \wedge (pt + to) \notin \text{SYSTEM\_TIME\_TYPE}) \longrightarrow \\
& \quad \quad \quad \text{apex\_function\_return\_code.partid.callerid !INVALID\_PARAM} \longrightarrow \\
& \quad \quad \quad \text{apex\_function\_suspend\_self\_return.partid.callerid} \longrightarrow \text{Skip} \\
& \quad \quad \square (to > 0 \wedge (pt + to) \in \text{SYSTEM\_TIME\_TYPE}) \longrightarrow \\
& \quad \quad \quad \text{system\_call\_service\_routine\_suspend\_self\_input.partid.callerid !pt !to} \\
& \quad \quad \quad \longrightarrow \\
& \quad \quad \quad \text{system\_call.partid.callerid !SUSPEND\_SELF} \longrightarrow \\
& \quad \quad \quad \text{system\_call\_return.partid.callerid} \longrightarrow \\
& \quad \quad \quad \text{system\_call\_service\_routine\_suspend\_self\_output.partid.callerid ?result} \\
& \quad \quad \quad \longrightarrow \\
& \quad \quad \quad \left( \text{if } (result = \text{TRUE}) \longrightarrow \right. \\
& \quad \quad \quad \quad \text{apex\_function\_return\_code.partid.callerid !NO\_ERROR} \longrightarrow \\
& \quad \quad \quad \quad \text{apex\_function\_suspend\_self\_return.partid.callerid} \longrightarrow \text{Skip} \\
& \quad \quad \quad \quad \square (result = \text{FALSE}) \longrightarrow \\
& \quad \quad \quad \quad \text{apex\_function\_return\_code.partid.callerid !TIMED\_OUT} \\
& \quad \quad \quad \quad \longrightarrow \\
& \quad \quad \quad \quad \text{apex\_function\_suspend\_self\_return.partid.callerid} \longrightarrow \text{Skip} \\
& \quad \quad \quad \text{fi} \\
& \quad \quad \text{fi} \\
& \quad \text{fi} \\
& \text{fi} \\
& \left. \right)
\end{aligned}$$



$$\begin{aligned}
\text{Suspend} \hat{=} & \text{apex\_function\_suspend.partid.callerid} \longrightarrow \\
& \text{apex\_function\_suspend\_input.partid.callerid} \text{ ?procid} \longrightarrow \\
& \text{system\_call.partid.callerid} \text{ !GET\_PROCESS\_IDS} \longrightarrow \\
& \text{system\_call\_return.partid.callerid} \longrightarrow \\
& \text{system\_call\_service\_routine\_get\_process\_ids\_output.partid.callerid} \text{ ?procids} \longrightarrow \\
& \text{system\_call.partid.callerid} \text{ !GET\_MY\_ID} \longrightarrow \\
& \text{system\_call\_return.partid.callerid} \longrightarrow \\
& \text{system\_call\_service\_routine\_get\_my\_id\_output.partid.callerid} \text{ ?myid} \longrightarrow \\
& \left( \begin{array}{l} \text{if } (\text{procid} \notin \text{procids} \vee \text{procid} = \text{myid}) \longrightarrow \\ \quad \text{apex\_function\_return\_code.partid.callerid} \text{ !INVALID\_PARAM} \longrightarrow \\ \quad \text{apex\_function\_suspend\_return.partid.callerid} \longrightarrow \mathbf{Skip} \\ \quad \square (\text{procid} \in \text{procids} \wedge \text{procid} \neq \text{myid}) \longrightarrow \\ \quad \quad \text{system\_call\_service\_routine\_get\_process\_kind\_input.partid.callerid} \text{ !procid} \longrightarrow \\ \quad \quad \text{system\_call.partid.callerid} \text{ !GET\_PROCESS\_KIND} \longrightarrow \\ \quad \quad \text{system\_call\_return.partid.callerid} \longrightarrow \\ \quad \quad \text{system\_call\_service\_routine\_get\_process\_kind\_output.partid.callerid} \text{ ?prock} \longrightarrow \\ \quad \quad \text{system\_call\_service\_routine\_get\_process\_state\_input.partid.callerid} \text{ !procid} \longrightarrow \\ \quad \quad \text{system\_call.partid.callerid} \text{ !GET\_PROCESS\_STATE} \longrightarrow \\ \quad \quad \text{system\_call\_return.partid.callerid} \longrightarrow \\ \quad \quad \text{system\_call\_service\_routine\_get\_process\_state\_output.partid.callerid} \text{ ?procs} \longrightarrow \\ \quad \quad \left( \begin{array}{l} \text{if } (\text{prock} = \text{PERIODIC} \vee \text{procs} = \text{DORMANT}) \longrightarrow \\ \quad \text{apex\_function\_return\_code.partid.callerid} \text{ !INVALID\_MODE} \longrightarrow \\ \quad \text{apex\_function\_suspend\_return.partid.callerid} \longrightarrow \mathbf{Skip} \\ \quad \square (\text{prock} = \text{APERIODIC} \wedge \text{procs} \in \{\text{READY}, \text{WAITING}, \text{RUNNING}\}) \longrightarrow \\ \quad \quad \text{system\_call\_service\_routine\_get\_process\_kind\_input.partid.callerid} \text{ !myid} \\ \quad \quad \longrightarrow \\ \quad \quad \text{system\_call.partid.callerid} \text{ !GET\_PROCESS\_KIND} \longrightarrow \\ \quad \quad \text{system\_call\_return.partid.callerid} \longrightarrow \\ \quad \quad \text{system\_call\_service\_routine\_get\_process\_kind\_output.partid.callerid} \\ \quad \quad \text{?mykind} \longrightarrow \\ \quad \quad \left( \begin{array}{l} \text{if } (\text{mykind} \neq \text{ERROR\_HANDLER}) \longrightarrow \text{SuspendProcess}(\text{procid}) \\ \quad \square (\text{mykind} = \text{ERROR\_HANDLER}) \longrightarrow \text{SuspendErroredProcess} \\ \quad \quad (\text{procid}) \end{array} \right) \\ \quad \quad \mathbf{fi} \end{array} \right) \\ \quad \mathbf{fi} \end{array} \right)
\end{aligned}$$

$$\begin{aligned}
\text{SuspendErroredProcess} \hat{=} & \text{procid} : \text{procid} : \text{PROCESS\_ID\_TYPE} \bullet \\
& \text{system\_call.partid.callerid} \text{ !GET\_PARTITION\_LOCK\_LEVEL} \longrightarrow \\
& \text{system\_call\_return.partid.callerid} \longrightarrow \\
& \text{system\_call\_service\_routine\_get\_partition\_lock\_level\_output.partid.callerid} \\
& \text{?ll} \longrightarrow \\
& \text{error\_process\_id} \text{ ?eprocid} \longrightarrow \\
& \left( \begin{array}{l} \text{if } (\text{ll} > \text{MIN\_LOCK\_LEVEL} \wedge \text{eprocid} = \text{procid}) \longrightarrow \\ \quad \text{apex\_function\_return\_code.partid.callerid} \text{ !INVALID\_MODE} \longrightarrow \\ \quad \text{apex\_function\_suspend\_return.partid.callerid} \longrightarrow \mathbf{Skip} \\ \quad \square (\text{ll} = \text{MIN\_LOCK\_LEVEL} \vee \text{eprocid} \neq \text{procid}) \longrightarrow \\ \quad \quad \text{SuspendProcess}(\text{procid}) \\ \quad \mathbf{fi} \end{array} \right)
\end{aligned}$$

$$\begin{aligned}
\text{SuspendProcess} \quad \hat{=} \quad & \text{procid} : \text{procid} : \text{PROCESS\_ID\_TYPE} \bullet \\
& \text{system\_call\_service\_routine\_suspend\_input.partid.callerid} \rightarrow \text{!procid} \longrightarrow \\
& \text{system\_call.partid.callerid} \rightarrow \text{!SUSPEND} \longrightarrow \\
& \text{system\_call\_return.partid.callerid} \longrightarrow \\
& \text{system\_call\_service\_routine\_suspend\_output.partid.callerid} \rightarrow \text{?result} \longrightarrow \\
& \left( \begin{array}{l} \text{if } (\text{result} = \text{TRUE}) \longrightarrow \\ \quad \text{apex\_function\_return\_code.partid.callerid} \rightarrow \text{!NO\_ERROR} \longrightarrow \\ \quad \text{apex\_function\_suspend\_return.partid.callerid} \longrightarrow \text{Skip} \\ \quad \parallel (\text{result} = \text{FALSE}) \longrightarrow \\ \quad \text{apex\_function\_return\_code.partid.callerid} \rightarrow \text{!NO\_ACTION} \longrightarrow \\ \quad \text{apex\_function\_suspend\_return.partid.callerid} \longrightarrow \text{Skip} \\ \text{fi} \end{array} \right)
\end{aligned}$$

$$\begin{aligned}
\text{Resume} \quad \hat{=} \quad & \text{apex\_function\_resume.partid.callerid} \longrightarrow \\
& \text{apex\_function\_resume\_input.partid.callerid} \rightarrow \text{?procid} \longrightarrow \\
& \text{system\_call.partid.callerid} \rightarrow \text{!GET\_PROCESS\_IDS} \longrightarrow \\
& \text{system\_call\_return.partid.callerid} \longrightarrow \\
& \text{system\_call\_service\_routine\_get\_process\_ids\_output.partid.callerid} \rightarrow \text{?procids} \longrightarrow \\
& \left( \begin{array}{l} \text{if } (\text{procid} \notin \text{procids}) \longrightarrow \\ \quad \text{apex\_function\_return\_code.partid.callerid} \rightarrow \text{!INVALID\_PARAM} \longrightarrow \\ \quad \text{apex\_function\_resume\_return.partid.callerid} \longrightarrow \text{Skip} \\ \quad \parallel (\text{procid} \in \text{procids}) \longrightarrow \\ \quad \text{system\_call\_service\_routine\_get\_process\_kind\_input.partid.callerid} \rightarrow \text{!procid} \longrightarrow \\ \quad \text{system\_call.partid.callerid} \rightarrow \text{!GET\_PROCESS\_KIND} \longrightarrow \\ \quad \text{system\_call\_return.partid.callerid} \longrightarrow \\ \quad \text{system\_call\_service\_routine\_get\_process\_kind\_output.partid.callerid} \rightarrow \text{?prock} \longrightarrow \\ \quad \text{system\_call\_service\_routine\_get\_process\_state\_input.partid.callerid} \rightarrow \text{!procid} \longrightarrow \\ \quad \text{system\_call.partid.callerid} \rightarrow \text{!GET\_PROCESS\_STATE} \longrightarrow \\ \quad \text{system\_call\_return.partid.callerid} \longrightarrow \\ \quad \text{system\_call\_service\_routine\_get\_process\_state\_output.partid.callerid} \rightarrow \text{?procs} \longrightarrow \\ \quad \left( \begin{array}{l} \text{if } (\text{prock} = \text{PERIODIC} \vee \text{procs} = \text{DORMANT}) \longrightarrow \\ \quad \text{apex\_function\_return\_code.partid.callerid} \rightarrow \text{!INVALID\_MODE} \longrightarrow \\ \quad \text{apex\_function\_resume\_return.partid.callerid} \longrightarrow \text{Skip} \\ \quad \parallel (\text{prock} = \text{APERIODIC} \wedge \text{procs} = \text{READY}) \longrightarrow \\ \quad \text{apex\_function\_return\_code.partid.callerid} \rightarrow \text{!NO\_ACTION} \longrightarrow \\ \quad \text{apex\_function\_resume\_return.partid.callerid} \longrightarrow \text{Skip} \\ \quad \parallel (\text{prock} = \text{APERIODIC} \wedge \text{procs} = \text{WAITING}) \longrightarrow \\ \quad \text{system\_call\_service\_routine\_resume\_input.partid.callerid} \rightarrow \text{!procid} \longrightarrow \\ \quad \text{system\_call.partid.callerid} \rightarrow \text{!RESUME} \longrightarrow \\ \quad \text{system\_call\_return.partid.callerid} \longrightarrow \\ \quad \text{apex\_function\_return\_code.partid.callerid} \rightarrow \text{!NO\_ERROR} \longrightarrow \\ \quad \text{apex\_function\_resume\_return.partid.callerid} \longrightarrow \text{Skip} \\ \text{fi} \end{array} \right) \\ \text{fi} \end{array} \right)
\end{aligned}$$

$$\begin{aligned}
\text{StopSelf} \quad \hat{=} \quad & \text{apex\_function\_stop\_self.partid.callerid} \longrightarrow \\
& \text{system\_call.partid.callerid} \rightarrow \text{!STOP\_SELF} \longrightarrow \text{Skip}
\end{aligned}$$

$$\begin{aligned}
\text{Stop} \quad \hat{=} \quad & \text{apex\_function\_stop.partid.callerid} \longrightarrow \\
& \text{apex\_function\_stop\_input.partid.callerid} \text{ ?procid} \longrightarrow \\
& \text{system\_call.partid.callerid} \text{ !GET\_PROCESS\_IDS} \longrightarrow \\
& \text{system\_call\_return.partid.callerid} \longrightarrow \\
& \text{system\_call\_service\_routine\_get\_process\_ids\_output.partid.callerid} \text{ ?procids} \longrightarrow \\
& \text{system\_call.partid.callerid} \text{ !GET\_MY\_ID} \longrightarrow \\
& \text{system\_call\_return.partid.callerid} \longrightarrow \\
& \text{system\_call\_service\_routine\_get\_my\_id\_output.partid.callerid} \text{ ?myid} \longrightarrow \\
& \left( \begin{array}{l} \text{if } (\text{procid} \notin \text{procids} \vee \text{procid} = \text{myid}) \longrightarrow \\ \quad \text{apex\_function\_return\_code.partid.callerid} \text{ !INVALID\_PARAM} \longrightarrow \\ \quad \text{apex\_function\_stop\_return.partid.callerid} \longrightarrow \mathbf{Skip} \\ \quad \square (\text{procid} \in \text{procids} \wedge \text{procid} \neq \text{myid}) \longrightarrow \\ \quad \quad \text{system\_call\_service\_routine\_get\_process\_state\_input.partid.callerid} \\ \quad \quad \text{!procid} \longrightarrow \\ \quad \quad \text{system\_call.partid.callerid} \text{ !GET\_PROCESS\_STATE} \longrightarrow \\ \quad \quad \text{system\_call\_return.partid.callerid} \longrightarrow \\ \quad \quad \text{system\_call\_service\_routine\_get\_process\_state\_output.partid.callerid} \\ \quad \quad \text{?procs} \longrightarrow \\ \quad \quad \left( \begin{array}{l} \text{if } (\text{procs} = \text{DORMANT}) \longrightarrow \\ \quad \text{apex\_function\_return\_code.partid.callerid} \text{ !NO\_ACTION} \longrightarrow \\ \quad \text{apex\_function\_stop\_return.partid.callerid} \longrightarrow \mathbf{Skip} \\ \quad \square (\text{procs} \in \{\text{READY}, \text{WAITING}, \text{RUNNING}\}) \longrightarrow \\ \quad \quad \text{system\_call\_service\_routine\_stop\_input.partid.callerid} \text{ !procid} \\ \quad \quad \longrightarrow \\ \quad \quad \text{system\_call.partid.callerid} \text{ !STOP} \longrightarrow \\ \quad \quad \text{system\_call\_return.partid.callerid} \longrightarrow \\ \quad \quad \text{apex\_function\_return\_code.partid.callerid} \text{ !NO\_ERROR} \longrightarrow \\ \quad \quad \text{apex\_function\_stop\_return.partid.callerid} \longrightarrow \mathbf{Skip} \end{array} \right) \\ \text{fi} \end{array} \right) \\
& \text{fi}
\end{aligned}$$

$$\begin{aligned}
\text{Start} \quad \hat{=} \quad & \text{apex\_function\_start.partid.callerid} \longrightarrow \\
& \text{apex\_function\_start\_input.partid.callerid} \text{ ?procid} \longrightarrow \\
& \text{system\_call.partid.callerid} \text{ !GET\_PROCESS\_IDS} \longrightarrow \\
& \text{system\_call\_return.partid.callerid} \longrightarrow \\
& \text{system\_call\_service\_routine\_get\_process\_ids\_output.partid.callerid} \text{ ?procids} \longrightarrow \\
& \left( \begin{array}{l} \text{if } (\text{procid} \notin \text{procids}) \longrightarrow \\ \quad \text{apex\_function\_return\_code.partid.callerid} \text{ !INVALID\_PARAM} \longrightarrow \\ \quad \text{apex\_function\_start\_return.partid.callerid} \longrightarrow \mathbf{Skip} \\ \quad \parallel (\text{procid} \in \text{procids}) \longrightarrow \\ \quad \text{system\_call\_service\_routine\_get\_process\_state\_input.partid.callerid} \text{ !procid} \longrightarrow \\ \quad \text{system\_call.partid.callerid} \text{ !GET\_PROCESS\_STATE} \longrightarrow \\ \quad \text{system\_call\_return.partid.callerid} \longrightarrow \\ \quad \text{system\_call\_service\_routine\_get\_process\_state\_output.partid.callerid} \text{ ?procs} \longrightarrow \\ \quad \left( \begin{array}{l} \text{if } (\text{procs} \in \{\text{READY}, \text{WAITING}, \text{RUNNING}\}) \longrightarrow \\ \quad \text{apex\_function\_return\_code.partid.callerid} \text{ !NO\_ACTION} \longrightarrow \\ \quad \text{apex\_function\_start\_return.partid.callerid} \longrightarrow \mathbf{Skip} \\ \quad \parallel (\text{procs} = \text{DORMANT}) \longrightarrow \\ \quad \text{system\_call\_service\_routine\_get\_process\_kind\_input.partid.callerid} \\ \quad \text{!procid} \longrightarrow \\ \quad \text{system\_call.partid.callerid} \text{ !GET\_PROCESS\_KIND} \longrightarrow \\ \quad \text{system\_call\_return.partid.callerid} \longrightarrow \\ \quad \text{system\_call\_service\_routine\_get\_process\_kind\_output.partid.callerid} \\ \quad \text{?prock} \longrightarrow \\ \quad \left( \begin{array}{l} \text{if } (\text{prock} = \text{APERIODIC}) \longrightarrow \text{StartAperiodicProcess}(\text{procid}) \\ \quad \parallel (\text{prock} = \text{PERIODIC}) \longrightarrow \text{StartPeriodicProcess}(\text{procid}) \\ \text{fi} \end{array} \right) \end{array} \right) \\ \text{fi} \end{array} \right)
\end{aligned}$$

$$\begin{aligned}
\text{StartAperiodicProcess} \quad \hat{=} \quad & \text{procid} : \text{procid} : \text{PROCESS\_ID\_TYPE} \bullet \\
& \text{system\_call.partid.callerid} \text{ !GET\_OPERATING\_MODE} \longrightarrow \\
& \text{system\_call\_return.partid.callerid} \longrightarrow \\
& \text{system\_call\_service\_routine\_get\_operating\_mode\_output.partid.callerid} \\
& \text{?om} \longrightarrow \\
& \left( \begin{array}{l}
\text{if } (\text{om} \in \{\text{COLD\_START}, \text{WARM\_START}\}) \longrightarrow \\
\quad \text{system\_call\_service\_routine\_start\_input.partid.callerid} \text{ !procid} \\
\quad \text{!DEFAULT\_TIME !DEFAULT\_TIME !om} \longrightarrow \\
\quad \text{system\_call.partid.callerid} \text{ !START} \longrightarrow \\
\quad \text{system\_call\_return.partid.callerid} \longrightarrow \\
\quad \text{apex\_function\_return\_code.partid.callerid} \text{ !NO\_ERROR} \longrightarrow \\
\quad \text{apex\_function\_start\_return.partid.callerid} \longrightarrow \text{Skip} \\
\quad \square (\text{om} = \text{NORMAL}) \longrightarrow \\
\quad \text{system\_call.partid.callerid} \text{ !GET\_CURRENT\_TIME} \longrightarrow \\
\quad \text{system\_call\_return.partid.callerid} \longrightarrow \\
\quad \text{system\_call\_service\_routine\_get\_current\_time\_output.partid.} \\
\quad \text{callerid ?ct} \longrightarrow \\
\quad \text{system\_call\_service\_routine\_get\_process\_time\_capacity\_input.} \\
\quad \text{partid.callerid !procid} \longrightarrow \\
\quad \text{system\_call.partid.callerid} \text{ !GET\_PROCESS\_TIME\_CAPACITY} \\
\quad \longrightarrow \\
\quad \text{system\_call\_return.partid.callerid} \longrightarrow \\
\quad \text{system\_call\_service\_routine\_get\_process\_time\_capacity\_output.} \\
\quad \text{partid.callerid ?tc} \longrightarrow \\
\quad \left( \begin{array}{l}
\text{if } ((\text{ct} + \text{tc}) \notin \text{SYSTEM\_TIME\_TYPE}) \longrightarrow \\
\quad \text{apex\_function\_return\_code.partid.callerid} \text{ !INVALID\_} \\
\quad \text{CONFIG} \longrightarrow \\
\quad \text{apex\_function\_start\_return.partid.callerid} \longrightarrow \text{Skip} \\
\quad \square ((\text{ct} + \text{tc}) \in \text{SYSTEM\_TIME\_TYPE}) \longrightarrow \\
\quad \text{system\_call\_service\_routine\_start\_input.partid.callerid} \\
\quad \text{!procid !ct !(ct + tc) !om} \longrightarrow \\
\quad \text{system\_call.partid.callerid} \text{ !START} \longrightarrow \\
\quad \text{system\_call\_return.partid.callerid} \longrightarrow \\
\quad \text{apex\_function\_return\_code.partid.callerid} \text{ !NO\_ERROR} \\
\quad \longrightarrow \\
\quad \text{apex\_function\_start\_return.partid.callerid} \longrightarrow \text{Skip}
\end{array} \right) \\
\text{fi}
\end{array} \right)
\end{aligned}$$

$StartPeriodicProcess \hat{=} procid : procid : PROCESS\_ID\_TYPE \bullet$   
 $system\_call.partid.callerid !GET\_OPERATING\_MODE \longrightarrow$   
 $system\_call\_return.partid.callerid \longrightarrow$   
 $system\_call\_service\_routine\_get\_operating\_mode\_output.partid.callerid ?om \longrightarrow$   
 $\left( \begin{array}{l} \text{if } (om \in \{COLD\_START, WARM\_START\}) \longrightarrow \\ \quad system\_call\_service\_routine\_start\_input.partid.callerid !procid \\ \quad !DEFAULT\_TIME !DEFAULT\_TIME !om \longrightarrow \\ \quad system\_call.partid.callerid !START \longrightarrow \\ \quad system\_call\_return.partid.callerid \longrightarrow \\ \quad apex\_function\_return\_code.partid.callerid !NO\_ERROR \longrightarrow \\ \quad apex\_function\_start\_return.partid.callerid \longrightarrow \text{Skip} \\ \quad \square (om = NORMAL) \longrightarrow \\ \quad \quad system\_call.partid.callerid !GET\_NEXT\_PERIODIC\_START \longrightarrow \\ \quad \quad system\_call\_return.partid.callerid \longrightarrow \\ \quad \quad system\_call\_service\_routine\_get\_next\_periodic\_start\_output.partid. \\ \quad \quad callerid ?nps \longrightarrow \\ \quad \quad system\_call\_service\_routine\_get\_process\_time\_capacity\_input.partid. \\ \quad \quad callerid !procid \longrightarrow \\ \quad \quad system\_call.partid.callerid !GET\_PROCESS\_TIME\_CAPACITY \\ \quad \quad \longrightarrow \\ \quad \quad system\_call\_return.partid.callerid \longrightarrow \\ \quad \quad system\_call\_service\_routine\_get\_process\_time\_capacity\_output. \\ \quad \quad partid.callerid ?tc \longrightarrow \\ \quad \quad \left( \begin{array}{l} \text{if } ((nps + tc) \notin SYSTEM\_TIME\_TYPE) \longrightarrow \\ \quad apex\_function\_return\_code.partid.callerid !INVALID\_ \\ \quad CONFIG \longrightarrow \\ \quad apex\_function\_start\_return.partid.callerid \longrightarrow \text{Skip} \\ \quad \square ((nps + tc) \in SYSTEM\_TIME\_TYPE) \longrightarrow \\ \quad \quad system\_call\_service\_routine\_start\_input.partid.callerid \\ \quad \quad !procid !nps !(nps + tc) !om \longrightarrow \\ \quad \quad system\_call.partid.callerid !START \longrightarrow \\ \quad \quad system\_call\_return.partid.callerid \longrightarrow \\ \quad \quad apex\_function\_return\_code.partid.callerid !NO\_ERROR \\ \quad \quad \longrightarrow \\ \quad \quad apex\_function\_start\_return.partid.callerid \longrightarrow \text{Skip} \end{array} \right) \\ \text{fi} \end{array} \right)$   
 $\text{fi}$

$$\begin{aligned}
\text{DelayedStart} \quad \hat{=} \quad & \text{apex\_function\_delayed\_start.partid.callerid} \longrightarrow \\
& \text{apex\_function\_delayed\_start\_input.partid.callerid} \text{ ?procid ?delay} \longrightarrow \\
& \text{system\_call.partid.callerid} \text{ !GET\_PROCESS\_IDS} \longrightarrow \\
& \text{system\_call\_return.partid.callerid} \longrightarrow \\
& \text{system\_call\_service\_routine\_get\_process\_ids\_output.partid.callerid} \text{ ?procids} \longrightarrow \\
& \left( \begin{array}{l} \text{if } (\text{procid} \notin \text{procids} \vee \text{delay} < 0 \vee \text{delay} \notin \text{SYSTEM\_TIME\_TYPE}) \longrightarrow \\ \quad \text{apex\_function\_return\_code.partid.callerid} \text{ !INVALID\_PARAM} \longrightarrow \\ \quad \text{apex\_function\_delayed\_start\_return.partid.callerid} \longrightarrow \mathbf{Skip} \\ \quad \parallel (\text{procid} \in \text{procids} \wedge \text{delay} \geq 0 \wedge \text{delay} \in \text{SYSTEM\_TIME\_TYPE}) \longrightarrow \\ \quad \text{system\_call\_service\_routine\_get\_process\_state\_input.partid.callerid} \\ \quad \text{!procid} \longrightarrow \\ \quad \text{system\_call.partid.callerid} \text{ !GET\_PROCESS\_STATE} \longrightarrow \\ \quad \text{system\_call\_return.partid.callerid} \longrightarrow \\ \quad \text{system\_call\_service\_routine\_get\_process\_state\_output.partid.callerid} \\ \quad \text{?procs} \longrightarrow \\ \quad \left( \begin{array}{l} \text{if } (\text{procs} \in \{\text{READY}, \text{WAITING}, \text{RUNNING}\}) \longrightarrow \\ \quad \text{apex\_function\_return\_code.partid.callerid} \text{ !NO\_ACTION} \longrightarrow \\ \quad \text{apex\_function\_delayed\_start\_return.partid.callerid} \longrightarrow \mathbf{Skip} \\ \quad \parallel (\text{procs} = \text{DORMANT}) \longrightarrow \\ \quad \text{system\_call\_service\_routine\_get\_process\_kind\_input.partid.} \\ \quad \text{callerid !procid} \longrightarrow \\ \quad \text{system\_call.partid.callerid} \text{ !GET\_PROCESS\_KIND} \longrightarrow \\ \quad \text{system\_call\_return.partid.callerid} \longrightarrow \\ \quad \text{system\_call\_service\_routine\_get\_process\_kind\_output.partid.} \\ \quad \text{callerid ?prock} \longrightarrow \\ \quad \left( \begin{array}{l} \text{if } (\text{prock} = \text{APERIODIC}) \longrightarrow \\ \quad \text{DelayedStartAperiodicProcess}(\text{procid}, \text{delay}) \\ \quad \parallel (\text{prock} = \text{PERIODIC}) \longrightarrow \\ \quad \text{DelayedStartPeriodicProcess}(\text{procid}, \text{delay}) \end{array} \right) \\ \quad \mathbf{fi} \end{array} \right) \\ \mathbf{fi} \end{array} \right)
\end{aligned}$$

$$\begin{aligned}
\text{DelayedStartAperiodicProcess} \quad \hat{=} \quad & \text{procid} : \text{procid} : \text{PROCESS\_ID\_TYPE}, \text{delay} : \text{SYSTEM\_TIME\_TYPE} \bullet \\
& \text{system\_call.partid.callerid !GET\_OPERATING\_MODE} \longrightarrow \\
& \text{system\_call\_return.partid.callerid} \longrightarrow \\
& \text{system\_call\_service\_routine\_get\_operating\_mode\_output.partid.callerid} \\
& ?om \longrightarrow \\
& \left( \begin{array}{l}
\text{if } (om \in \{COLD\_START, WARM\_START\}) \longrightarrow \\
\quad \text{system\_call\_service\_routine\_delayed\_start\_input.partid.callerid} \\
\quad !\text{procid !DEFAULT\_TIME !delay !DEFAULT\_TIME !om} \longrightarrow \\
\quad \text{system\_call.partid.callerid !DELAYED\_START} \longrightarrow \\
\quad \text{system\_call\_return.partid.callerid} \longrightarrow \\
\quad \text{apex\_function\_return\_code.partid.callerid !NO\_ERROR} \longrightarrow \\
\quad \text{apex\_function\_delayed\_start\_return.partid.callerid} \longrightarrow \text{Skip} \\
\quad \square \\
\quad (om = \text{NORMAL}) \longrightarrow \\
\quad \text{system\_call.partid.callerid !GET\_CURRENT\_TIME} \longrightarrow \\
\quad \text{system\_call\_return.partid.callerid} \longrightarrow \\
\quad \text{system\_call\_service\_routine\_get\_current\_time\_output.partid.} \\
\quad \text{callerid ?ct} \longrightarrow \\
\quad \text{system\_call\_service\_routine\_get\_process\_time\_capacity\_input.} \\
\quad \text{partid.callerid !procid} \longrightarrow \\
\quad \text{system\_call.partid.callerid !GET\_PROCESS\_TIME\_} \\
\quad \text{CAPACITY} \longrightarrow \\
\quad \text{system\_call\_return.partid.callerid} \longrightarrow \\
\quad \text{system\_call\_service\_routine\_get\_process\_time\_capacity\_output.} \\
\quad \text{partid.callerid ?tc} \longrightarrow \\
\quad \left( \begin{array}{l}
\text{if } ((ct + \text{delay} + tc) \notin \text{SYSTEM\_TIME\_TYPE}) \longrightarrow \\
\quad \text{apex\_function\_return\_code.partid.callerid !INVALID\_} \\
\quad \text{CONFIG} \longrightarrow \\
\quad \text{apex\_function\_delayed\_start\_return.partid.callerid} \longrightarrow \\
\quad \text{Skip} \\
\quad \square \\
\quad ((ct + \text{delay} + tc) \in \text{SYSTEM\_TIME\_TYPE}) \longrightarrow \\
\quad \text{system\_call\_service\_routine\_start\_input.partid.callerid} \\
\quad !\text{procid !ct !delay !(ct + \text{delay} + tc) !om} \longrightarrow \\
\quad \text{system\_call.partid.callerid !DELAYED\_START} \longrightarrow \\
\quad \text{system\_call\_return.partid.callerid} \longrightarrow \\
\quad \text{apex\_function\_return\_code.partid.callerid !NO\_} \\
\quad \text{ERROR} \longrightarrow \\
\quad \text{apex\_function\_delayed\_start\_return.partid.callerid} \longrightarrow \\
\quad \text{Skip}
\end{array} \right) \\
\quad \text{fi}
\end{array} \right) \\
& \text{fi}
\end{aligned}$$



$$\begin{aligned}
\text{DelayedStartPeriodicProcess} \quad \hat{=} \quad & \text{procid} : \text{procid} : \text{PROCESS\_ID\_TYPE}, \text{delay} : \text{SYSTEM\_TIME\_TYPE} \bullet \\
& \text{system\_call\_service\_routine\_get\_process\_period\_input.partid.callerid} \text{ !procid} \\
& \longrightarrow \\
& \text{system\_call.partid.callerid} \text{ !GET\_PROCESS\_PERIOD} \longrightarrow \\
& \text{system\_call\_return.partid.callerid} \longrightarrow \\
& \text{system\_call\_service\_routine\_get\_process\_period\_output.partid.callerid} \text{ ?procp} \\
& \longrightarrow \\
& \left( \begin{array}{l} \text{if } (\text{delay} \geq \text{procp}) \longrightarrow \\ \quad \text{apex\_function\_return\_code.partid.callerid} \text{ !INVALID\_PARAM} \longrightarrow \\ \quad \text{apex\_function\_delayed\_start\_return.partid.callerid} \longrightarrow \text{Skip} \\ \quad \square (\text{delay} < \text{procp}) \longrightarrow \\ \quad \text{system\_call.partid.callerid} \text{ !GET\_OPERATING\_MODE} \longrightarrow \\ \quad \text{system\_call\_return.partid.callerid} \longrightarrow \\ \quad \text{system\_call\_service\_routine\_get\_operating\_mode\_output.partid.} \\ \quad \text{callerid} \text{ ?om} \longrightarrow \\ \quad \left( \begin{array}{l} \text{if } (\text{om} \in \{\text{COLD\_START}, \text{WARM\_START}\}) \longrightarrow \\ \quad \text{system\_call\_service\_routine\_delayed\_start\_input.partid.} \\ \quad \text{callerid} \text{ !procid !DEFAULT\_TIME !delay !DEFAULT\_} \\ \quad \text{TIME !om} \longrightarrow \\ \quad \text{system\_call.partid.callerid} \text{ !DELAYED\_START} \longrightarrow \\ \quad \text{system\_call\_return.partid.callerid} \longrightarrow \\ \quad \text{apex\_function\_return\_code.partid.callerid} \text{ !NO\_ERROR} \\ \quad \longrightarrow \\ \quad \text{apex\_function\_delayed\_start\_return.partid.callerid} \longrightarrow \\ \quad \text{Skip} \\ \quad \square (\text{om} = \text{NORMAL}) \longrightarrow \\ \quad \text{DelayedStartPeriodicProcess\_Normal}(\text{procid}, \text{delay}, \text{om}) \end{array} \right) \\ \text{fi} \end{array} \right) \\
& \text{fi}
\end{aligned}$$

$$\begin{aligned}
\text{DelayedStartPeriodicProcess\_Normal} \quad \hat{=} \quad & \text{procid} : \text{procid} : \text{PROCESS\_ID\_TYPE}, \text{delay} : \text{SYSTEM\_TIME\_TYPE}, \\
& \text{om} : \text{OPERATING\_MODE\_TYPE} \bullet \\
& \text{system\_call.partid.callerid} \text{ !GET\_DELAYED\_PERIODIC\_START} \longrightarrow \\
& \text{system\_call\_return.partid.callerid} \longrightarrow \\
& \text{system\_call\_service\_routine\_get\_delayed\_periodic\_start\_output.partid.} \\
& \text{callerid} \text{ ?dps} \longrightarrow \\
& \text{system\_call\_service\_routine\_get\_process\_time\_capacity\_input.partid.} \\
& \text{callerid} \text{ !procid} \longrightarrow \\
& \text{system\_call.partid.callerid} \text{ !GET\_PROCESS\_TIME\_CAPACITY} \longrightarrow \\
& \text{system\_call\_return.partid.callerid} \longrightarrow \\
& \text{system\_call\_service\_routine\_get\_process\_time\_capacity\_output.partid.} \\
& \text{callerid} \text{ ?tc} \longrightarrow \\
& \left( \begin{array}{l} \text{if } ((\text{dps} + \text{tc}) \notin \text{SYSTEM\_TIME\_TYPE}) \longrightarrow \\ \quad \text{apex\_function\_return\_code.partid.callerid} \text{ !INVALID\_} \\ \quad \text{CONFIG} \longrightarrow \\ \quad \text{apex\_function\_delayed\_start\_return.partid.callerid} \longrightarrow \text{Skip} \\ \quad \square ((\text{dps} + \text{tc}) \in \text{SYSTEM\_TIME\_TYPE}) \longrightarrow \\ \quad \text{system\_call\_service\_routine\_start\_input.partid.callerid} \\ \quad \text{!procid !dps !delay !(dps + tc) !om} \longrightarrow \\ \quad \text{system\_call.partid.callerid} \text{ !DELAYED\_START} \longrightarrow \\ \quad \text{system\_call\_return.partid.callerid} \longrightarrow \\ \quad \text{apex\_function\_return\_code.partid.callerid} \text{ !NO\_ERROR} \longrightarrow \\ \quad \text{apex\_function\_delayed\_start\_return.partid.callerid} \longrightarrow \text{Skip} \\ \text{fi} \end{array} \right)
\end{aligned}$$

$$\begin{aligned}
\text{LockPreemption} \quad \hat{=} \quad & \text{apex\_function\_lock\_preemption.partid.callerid} \longrightarrow \\
& \text{system\_call.partid.callerid !GET\_OPERATING\_MODE} \longrightarrow \\
& \text{system\_call\_return.partid.callerid} \longrightarrow \\
& \text{system\_call\_service\_routine\_get\_operating\_mode\_output.partid.callerid ?om} \longrightarrow \\
& \text{system\_call.partid.callerid !GET\_MY\_ID} \longrightarrow \\
& \text{system\_call\_return.partid.callerid} \longrightarrow \\
& \text{system\_call\_service\_routine\_get\_my\_id\_output.partid.callerid ?myid} \longrightarrow \\
& \text{system\_call\_service\_routine\_get\_process\_kind\_input.partid.callerid !myid} \longrightarrow \\
& \text{system\_call.partid.callerid !GET\_PROCESS\_KIND} \longrightarrow \\
& \text{system\_call\_return.partid.callerid} \longrightarrow \\
& \text{system\_call\_service\_routine\_get\_process\_kind\_output.partid.callerid ?mykind} \longrightarrow \\
& \left( \begin{array}{l}
\text{if } (om \in \{COLD\_START, WARM\_START\} \vee mykind = ERROR\_HANDLER) \longrightarrow \\
\quad \text{system\_call.partid.callerid !GET\_PARTITION\_LOCK\_LEVEL} \longrightarrow \\
\quad \text{system\_call\_return.partid.callerid} \longrightarrow \\
\quad \text{system\_call\_service\_routine\_get\_partition\_lock\_level\_output.partid.callerid ?ll} \longrightarrow \\
\quad \text{apex\_function\_lock\_preemption\_output.partid.callerid !ll} \longrightarrow \\
\quad \text{apex\_function\_return\_code.partid.callerid !NO\_ACTION} \longrightarrow \\
\quad \text{apex\_function\_lock\_preemption\_return.partid.callerid} \longrightarrow \text{Skip} \\
\quad \square (om = NORMAL \wedge mykind \in \{APERIODIC, PERIODIC\}) \longrightarrow \\
\quad \text{system\_call.partid.callerid !GET\_PARTITION\_LOCK\_LEVEL} \longrightarrow \\
\quad \text{system\_call\_return.partid.callerid} \longrightarrow \\
\quad \text{system\_call\_service\_routine\_get\_partition\_lock\_level\_output.partid.callerid ?ll} \longrightarrow \\
\quad \left( \begin{array}{l}
\text{if } (ll \geq MAX\_LOCK\_LEVEL) \longrightarrow \\
\quad \text{apex\_function\_lock\_preemption\_output.partid.callerid !ll} \longrightarrow \\
\quad \text{apex\_function\_return\_code.partid.callerid !INVALID\_CONFIG} \longrightarrow \\
\quad \text{apex\_function\_lock\_preemption\_return.partid.callerid} \longrightarrow \text{Skip} \\
\quad \square (ll < MAX\_LOCK\_LEVEL) \longrightarrow \\
\quad \text{system\_call.partid.callerid !LOCK\_PREEMPTION} \longrightarrow \\
\quad \text{system\_call\_return.partid.callerid} \longrightarrow \\
\quad \text{system\_call\_service\_routine\_lock\_preemption\_output.partid.callerid ?ll} \longrightarrow \\
\quad \text{apex\_function\_lock\_preemption\_output.partid.callerid !ll} \longrightarrow \\
\quad \text{apex\_function\_return\_code.partid.callerid !NO\_ERROR} \longrightarrow \\
\quad \text{apex\_function\_lock\_preemption\_return.partid.callerid} \longrightarrow \text{Skip}
\end{array} \right) \\
\text{fi}
\end{array} \right)
\end{aligned}$$

$$\begin{aligned}
\text{UnlockPreemption} \quad \hat{=} \quad & \text{apex\_function\_unlock\_preemption.partid.callerid} \longrightarrow \\
& \text{system\_call.partid.callerid !GET\_OPERATING\_MODE} \longrightarrow \\
& \text{system\_call\_return.partid.callerid} \longrightarrow \\
& \text{system\_call\_service\_routine\_get\_operating\_mode\_output.partid.callerid ?om} \longrightarrow \\
& \text{system\_call.partid.callerid !GET\_MY\_ID} \longrightarrow \\
& \text{system\_call\_return.partid.callerid} \longrightarrow \\
& \text{system\_call\_service\_routine\_get\_my\_id\_output.partid.callerid ?myid} \longrightarrow \\
& \text{system\_call\_service\_routine\_get\_process\_kind\_input.partid.callerid !myid} \longrightarrow \\
& \text{system\_call.partid.callerid !GET\_PROCESS\_KIND} \longrightarrow \\
& \text{system\_call\_return.partid.callerid} \longrightarrow \\
& \text{system\_call\_service\_routine\_get\_process\_kind\_output.partid.callerid ?mykind} \longrightarrow \\
& \text{system\_call.partid.callerid !GET\_PARTITION\_LOCK\_LEVEL} \longrightarrow \\
& \text{system\_call\_return.partid.callerid} \longrightarrow \\
& \text{system\_call\_service\_routine\_get\_partition\_lock\_level\_output.partid.callerid ?ll} \longrightarrow \\
& \left( \begin{array}{l} \text{if } (om \in \{COLD\_START, WARM\_START\} \vee mykind = ERROR\_HANDLER \vee ll = MIN\_LOCK\_LEVEL) \longrightarrow \\ \quad \text{apex\_function\_unlock\_preemption\_output.partid.callerid !ll} \longrightarrow \\ \quad \text{apex\_function\_return\_code.partid.callerid !NO\_ACTION} \longrightarrow \\ \quad \text{apex\_function\_unlock\_preemption\_return.partid.callerid} \longrightarrow \text{Skip} \\ \quad \square (om = NORMAL \wedge mykind \in \{APERIODIC, PERIODIC\} \wedge ll > MIN\_LOCK\_LEVEL) \longrightarrow \\ \quad \text{system\_call.partid.callerid !UNLOCK\_PREEMPTION} \longrightarrow \\ \quad \text{system\_call\_return.partid.callerid} \longrightarrow \\ \quad \text{system\_call\_service\_routine\_unlock\_preemption\_output.partid.callerid ?ll} \longrightarrow \\ \quad \text{apex\_function\_unlock\_preemption\_output.partid.callerid !ll} \longrightarrow \\ \quad \text{apex\_function\_return\_code.partid.callerid !NO\_ERROR} \longrightarrow \\ \quad \text{apex\_function\_unlock\_preemption\_return.partid.callerid} \longrightarrow \text{Skip} \\ \text{fi} \end{array} \right)
\end{aligned}$$

$$\begin{aligned}
\text{GetMyId} \quad \hat{=} \quad & \text{apex\_function\_get\_my\_id.partid.callerid} \longrightarrow \\
& \text{system\_call.partid.callerid !GET\_MY\_ID} \longrightarrow \\
& \text{system\_call\_return.partid.callerid} \longrightarrow \\
& \text{system\_call\_service\_routine\_get\_my\_id\_output.partid.callerid ?myid} \longrightarrow \\
& \text{system\_call\_service\_routine\_get\_process\_kind\_input.partid.callerid !myid} \longrightarrow \\
& \text{system\_call.partid.callerid !GET\_PROCESS\_KIND} \longrightarrow \\
& \text{system\_call\_return.partid.callerid} \longrightarrow \\
& \text{system\_call\_service\_routine\_get\_process\_kind\_output.partid.callerid ?mykind} \longrightarrow \\
& \left( \begin{array}{l} \text{if } (mykind = ERROR\_HANDLER) \longrightarrow \\ \quad \text{apex\_function\_return\_code.partid.callerid !INVALID\_MODE} \longrightarrow \\ \quad \text{apex\_function\_get\_my\_id\_return.partid.callerid} \longrightarrow \text{Skip} \\ \quad \square (mykind = APERIODIC \vee mykind = PERIODIC) \longrightarrow \\ \quad \text{apex\_function\_get\_my\_id\_output.partid.callerid !myid} \longrightarrow \\ \quad \text{apex\_function\_return\_code.partid.callerid !NO\_ERROR} \longrightarrow \\ \quad \text{apex\_function\_get\_my\_id\_return.partid.callerid} \longrightarrow \text{Skip} \\ \text{fi} \end{array} \right)
\end{aligned}$$

$$\begin{aligned}
\text{TimedWait} \quad \hat{=} \quad & \text{apex\_function\_timed\_wait.partid.callerid} \longrightarrow \\
& \text{apex\_function\_timed\_wait\_input.partid.callerid} \text{ ?delay} \longrightarrow \\
& \text{system\_call.partid.callerid} \text{ !GET\_PARTITION\_LOCK\_LEVEL} \longrightarrow \\
& \text{system\_call\_return.partid.callerid} \longrightarrow \\
& \text{system\_call\_service\_routine\_get\_partition\_lock\_level\_output.partid.callerid} \text{ ?ll} \longrightarrow \\
& \text{apex\_function\_timed\_wait\_input.partid.callerid} \text{ ?delay} \longrightarrow \\
& \text{system\_call.partid.callerid} \text{ !GET\_MY\_ID} \longrightarrow \\
& \text{system\_call\_return.partid.callerid} \longrightarrow \\
& \text{system\_call\_service\_routine\_get\_my\_id\_output.partid.callerid} \text{ ?myid} \longrightarrow \\
& \text{system\_call\_service\_routine\_get\_process\_kind\_input.partid.callerid} \text{ !myid} \longrightarrow \\
& \text{system\_call.partid.callerid} \text{ !GET\_PROCESS\_KIND} \longrightarrow \\
& \text{system\_call\_return.partid.callerid} \longrightarrow \\
& \text{system\_call\_service\_routine\_get\_process\_kind\_output.partid.callerid} \text{ ?mykind} \longrightarrow \\
& \left( \begin{array}{l} \text{if } (ll > \text{MIN\_LOCK\_LEVEL} \vee \text{mykind} = \text{ERROR\_HANDLER}) \longrightarrow \\ \quad \text{apex\_function\_return\_code.partid.callerid} \text{ !INVALID\_MODE} \longrightarrow \\ \quad \text{apex\_function\_timed\_wait\_return.partid.callerid} \longrightarrow \text{Skip} \\ \quad \square \quad (ll = \text{MIN\_LOCK\_LEVEL} \wedge \text{mykind} \in \{\text{APERIODIC}, \text{PERIODIC}\}) \longrightarrow \\ \quad \text{system\_call.partid.callerid} \text{ !GET\_PARTITION\_TIME} \longrightarrow \\ \quad \text{system\_call\_return.partid.callerid} \longrightarrow \\ \quad \text{system\_call\_service\_routine\_get\_partition\_time\_output.partid.callerid} \text{ ?pt} \\ \quad \longrightarrow \\ \quad \left( \begin{array}{l} \text{if } (\text{delay} < 0 \vee (\text{pt} + \text{delay}) \notin \text{SYSTEM\_TIME\_TYPE}) \longrightarrow \\ \quad \text{apex\_function\_return\_code.partid.callerid} \text{ !INVALID\_PARAM} \\ \quad \longrightarrow \\ \quad \text{apex\_function\_timed\_wait\_return.partid.callerid} \longrightarrow \text{Skip} \\ \quad \square \quad (\text{delay} \geq 0 \wedge (\text{pt} + \text{delay}) \in \text{SYSTEM\_TIME\_TYPE}) \longrightarrow \\ \quad \text{system\_call\_service\_routine\_timed\_wait\_input.partid.callerid} \\ \quad \text{!delay} \longrightarrow \\ \quad \text{system\_call.partid.callerid} \text{ !TIMED\_WAIT} \longrightarrow \\ \quad \text{system\_call\_return.partid.callerid} \longrightarrow \\ \quad \text{apex\_function\_return\_code.partid.callerid} \text{ !NO\_ERROR} \longrightarrow \\ \quad \text{apex\_function\_timed\_wait\_return.partid.callerid} \longrightarrow \text{Skip} \end{array} \right) \\ \text{fi} \end{array} \right) \\
& \text{fi}
\end{aligned}$$

$PeriodicWait \hat{=}$ 
 $apex\_function\_periodic\_wait.partid.callerid \longrightarrow$   
 $system\_call.partid.callerid !GET\_PARTITION\_LOCK\_LEVEL \longrightarrow$   
 $system\_call\_return.partid.callerid \longrightarrow$   
 $system\_call\_service\_routine\_get\_partition\_lock\_level\_output.partid.callerid ?ll \longrightarrow$   
 $apex\_function\_timed\_wait\_input.partid.callerid ?delay \longrightarrow$   
 $system\_call.partid.callerid !GET\_MY\_ID \longrightarrow$   
 $system\_call\_return.partid.callerid \longrightarrow$   
 $system\_call\_service\_routine\_get\_my\_id\_output.partid.callerid ?myid \longrightarrow$   
 $system\_call\_service\_routine\_get\_process\_kind\_input.partid.callerid !myid \longrightarrow$   
 $system\_call.partid.callerid !GET\_PROCESS\_KIND \longrightarrow$   
 $system\_call\_return.partid.callerid \longrightarrow$   
 $system\_call\_service\_routine\_get\_process\_kind\_output.partid.callerid ?mykind \longrightarrow$   
 $\left( \begin{array}{l} \text{if } (ll > MIN\_LOCK\_LEVEL \vee mykind \in \{APERIODIC, ERROR\_HANDLER\}) \longrightarrow \\ \quad apex\_function\_return\_code.partid.callerid !INVALID\_MODE \longrightarrow \\ \quad apex\_function\_periodic\_wait\_return.partid.callerid \longrightarrow \text{Skip} \\ \quad \square (ll = MIN\_LOCK\_LEVEL \wedge mykind = PERIODIC) \longrightarrow \\ \quad \quad system\_call\_service\_routine\_get\_next\_release\_point\_input.partid.callerid \\ \quad \quad !myid \longrightarrow \\ \quad \quad system\_call.partid.callerid !GET\_NEXT\_RELEASE\_POINT \longrightarrow \\ \quad \quad system\_call\_return.partid.callerid \longrightarrow \\ \quad \quad system\_call\_service\_routine\_get\_next\_release\_point\_output.partid.callerid \\ \quad \quad ?nrp \longrightarrow \\ \quad \quad system\_call\_service\_routine\_get\_process\_time\_capacity\_input.partid. \\ \quad \quad callerid !myid \longrightarrow \\ \quad \quad system\_call.partid.callerid !GET\_PROCESS\_TIME\_CAPACITY \longrightarrow \\ \quad \quad system\_call\_return.partid.callerid \longrightarrow \\ \quad \quad system\_call\_service\_routine\_get\_process\_time\_capacity\_output.partid. \\ \quad \quad callerid ?tc \longrightarrow \\ \quad \quad \left( \begin{array}{l} \text{if } ((nrp + tc) \notin SYSTEM\_TIME\_TYPE) \longrightarrow \\ \quad apex\_function\_return\_code.partid.callerid !INVALID\_CONFIG \\ \quad \longrightarrow \\ \quad apex\_function\_periodic\_wait\_return.partid.callerid \longrightarrow \text{Skip} \\ \quad \square ((nrp + tc) \in SYSTEM\_TIME\_TYPE) \longrightarrow \\ \quad \quad system\_call\_service\_routine\_periodic\_wait\_input.partid.callerid \\ \quad \quad !nrp !(nrp + tc) \longrightarrow \\ \quad \quad system\_call.partid.callerid !PERIODIC\_WAIT \longrightarrow \\ \quad \quad system\_call\_return.partid.callerid \longrightarrow \\ \quad \quad apex\_function\_return\_code.partid.callerid !NO\_ERROR \longrightarrow \\ \quad \quad apex\_function\_periodic\_wait\_return.partid.callerid \longrightarrow \text{Skip} \end{array} \right) \\ \text{fi} \end{array} \right)$

$GetTime \hat{=}$ 
 $apex\_function\_get\_time.partid.callerid \longrightarrow$   
 $system\_call.partid.callerid !GET\_TIME \longrightarrow$   
 $system\_call\_return.partid.callerid \longrightarrow$   
 $system\_call\_service\_routine\_get\_time\_output.partid.callerid ?t \longrightarrow$   
 $apex\_function\_get\_time\_output.partid.callerid !t \longrightarrow$   
 $apex\_function\_return\_code.partid.callerid !NO\_ERROR \longrightarrow$   
 $apex\_function\_get\_time\_return.partid.callerid \longrightarrow \text{Skip}$

$$\begin{aligned}
\text{Replenish} \quad \hat{=} \quad & \text{apex\_function\_replenish.partid.callerid} \longrightarrow \\
& \text{apex\_function\_replenish\_input.partid.callerid} \text{ ?budget} \longrightarrow \\
& \text{system\_call.partid.callerid} \text{ !GET\_OPERATING\_MODE} \longrightarrow \\
& \text{system\_call\_return.partid.callerid} \longrightarrow \\
& \text{system\_call\_service\_routine\_get\_operating\_mode\_output.partid.callerid} \text{ ?om} \longrightarrow \\
& \text{system\_call.partid.callerid} \text{ !GET\_MY\_ID} \longrightarrow \\
& \text{system\_call\_return.partid.callerid} \longrightarrow \\
& \text{system\_call\_service\_routine\_get\_my\_id\_output.partid.callerid} \text{ ?myid} \longrightarrow \\
& \text{system\_call\_service\_routine\_get\_process\_kind\_input.partid.callerid} \text{ !myid} \longrightarrow \\
& \text{system\_call.partid.callerid} \text{ !GET\_PROCESS\_KIND} \longrightarrow \\
& \text{system\_call\_return.partid.callerid} \longrightarrow \\
& \text{system\_call\_service\_routine\_get\_process\_kind\_output.partid.callerid} \text{ ?mykind} \longrightarrow \\
& \left( \begin{array}{l} \text{if } (om \in \{COLD\_START, WARM\_START\} \vee mykind = ERROR\_HANDLER) \longrightarrow \\ \quad \text{apex\_function\_return\_code.partid.callerid} \text{ !NO\_ACTION} \longrightarrow \\ \quad \text{apex\_function\_replenish\_return.partid.callerid} \longrightarrow \text{Skip} \\ \quad \square (om = NORMAL \wedge mykind = APERIODIC) \longrightarrow \text{ReplenishAperiodicProcess}(budget) \\ \quad \square (om = NORMAL \wedge mykind = PERIODIC) \longrightarrow \\ \quad \quad \text{system\_call\_service\_routine\_get\_next\_release\_point\_input.partid.callerid} \text{ !myid} \longrightarrow \\ \quad \quad \text{system\_call.partid.callerid} \text{ !GET\_NEXT\_RELEASE\_POINT} \longrightarrow \\ \quad \quad \text{system\_call\_return.partid.callerid} \longrightarrow \\ \quad \quad \text{system\_call\_service\_routine\_get\_next\_release\_point\_output.partid.callerid} \text{ ?nrp} \longrightarrow \\ \quad \quad \text{ReplenishPeriodicProcess}(nrp, budget) \\ \text{fi} \end{array} \right)
\end{aligned}$$

$$\begin{aligned}
\text{ReplenishAperiodicProcess} \quad \hat{=} \quad & budget : \text{SYSTEM\_TIME\_TYPE} \bullet \\
& \text{system\_call.partid.callerid} \text{ !GET\_CURRENT\_TIME} \longrightarrow \\
& \text{system\_call\_return.partid.callerid} \longrightarrow \\
& \text{system\_call\_service\_routine\_get\_current\_time\_output.partid.callerid} \text{ ?ct} \longrightarrow \\
& \left( \begin{array}{l} \text{if } (budget = 0) \longrightarrow \\ \quad \text{apex\_function\_return\_code.partid.callerid} \text{ !NO\_ERROR} \longrightarrow \\ \quad \text{apex\_function\_replenish\_return.partid.callerid} \longrightarrow \text{Skip} \\ \quad \square (budget < 0) \longrightarrow \\ \quad \quad \text{system\_call\_service\_routine\_replenish\_input.partid.callerid} \text{ !ct} \\ \quad \quad \text{!budget} \longrightarrow \\ \quad \quad \text{system\_call.partid.callerid} \text{ !REPLENISH} \longrightarrow \\ \quad \quad \text{system\_call\_return.partid.callerid} \longrightarrow \\ \quad \quad \text{apex\_function\_return\_code.partid.callerid} \text{ !NO\_ERROR} \longrightarrow \\ \quad \quad \text{apex\_function\_replenish\_return.partid.callerid} \longrightarrow \text{Skip} \\ \quad \square (budget > 0 \wedge (ct + budget) \notin \text{SYSTEM\_TIME\_TYPE}) \longrightarrow \\ \quad \quad \text{apex\_function\_return\_code.partid.callerid} \text{ !INVALID\_PARAM} \longrightarrow \\ \quad \quad \text{apex\_function\_replenish\_return.partid.callerid} \longrightarrow \text{Skip} \\ \quad \square (budget > 0 \wedge (ct + budget) \in \text{SYSTEM\_TIME\_TYPE}) \longrightarrow \\ \quad \quad \text{system\_call\_service\_routine\_replenish\_input.partid.callerid} \text{ !ct} \\ \quad \quad \text{!budget} \longrightarrow \\ \quad \quad \text{system\_call.partid.callerid} \text{ !REPLENISH} \longrightarrow \\ \quad \quad \text{system\_call\_return.partid.callerid} \longrightarrow \\ \quad \quad \text{apex\_function\_return\_code.partid.callerid} \text{ !NO\_ERROR} \longrightarrow \\ \quad \quad \text{apex\_function\_replenish\_return.partid.callerid} \longrightarrow \text{Skip} \\ \text{fi} \end{array} \right)
\end{aligned}$$

$$\begin{aligned}
\text{ReplenishPeriodicProcess} \quad \hat{=} \quad & \text{nrp, budget : SYSTEM\_TIME\_TYPE} \bullet \\
& \text{system\_call.partition.callerid !GET\_CURRENT\_TIME} \longrightarrow \\
& \text{system\_call\_return.partition.callerid} \longrightarrow \\
& \text{system\_call\_service\_routine\_get\_current\_time\_output.partition.callerid ?ct} \longrightarrow \\
& \left( \begin{array}{l}
\text{if } (\text{budget} = 0) \longrightarrow \\
\quad \text{apex\_function\_return\_code.partition.callerid !NO\_ERROR} \longrightarrow \\
\quad \text{apex\_function\_replenish\_return.partition.callerid} \longrightarrow \text{Skip} \\
\quad \square (\text{budget} < 0) \longrightarrow \\
\quad \text{apex\_function\_return\_code.partition.callerid !INVALID\_PARAM} \longrightarrow \\
\quad \text{apex\_function\_replenish\_return.partition.callerid} \longrightarrow \text{Skip} \\
\quad \square (\text{budget} > 0 \wedge (\text{ct} + \text{budget}) \notin \text{SYSTEM\_TIME\_TYPE}) \longrightarrow \\
\quad \text{apex\_function\_return\_code.partition.callerid !INVALID\_PARAM} \longrightarrow \\
\quad \text{apex\_function\_replenish\_return.partition.callerid} \longrightarrow \text{Skip} \\
\quad \square (\text{budget} > 0 \wedge (\text{ct} + \text{budget}) \in \text{SYSTEM\_TIME\_TYPE}) \longrightarrow \\
\quad \left( \begin{array}{l}
\text{if } (\text{ct} + \text{budget} > \text{nrp}) \longrightarrow \\
\quad \text{apex\_function\_return\_code.partition.callerid !INVALID\_} \\
\quad \text{MODE} \longrightarrow \\
\quad \text{apex\_function\_replenish\_return.partition.callerid} \longrightarrow \text{Skip} \\
\quad \square (\text{ct} + \text{budget} \leq \text{nrp}) \longrightarrow \\
\quad \text{system\_call\_service\_routine\_replenish\_input.partition.} \\
\quad \text{callerid !ct !budget} \longrightarrow \\
\quad \text{system\_call.partition.callerid !REPLENISH} \longrightarrow \\
\quad \text{system\_call\_return.partition.callerid} \longrightarrow \\
\quad \text{apex\_function\_return\_code.partition.callerid !NO\_ERROR} \\
\quad \longrightarrow \\
\quad \text{apex\_function\_replenish\_return.partition.callerid} \longrightarrow \text{Skip}
\end{array} \right) \\
\text{fi}
\end{array} \right) \\
& \text{fi}
\end{aligned}$$

$$\begin{aligned}
\text{APEXService} \quad \hat{=} \quad & \text{GetPartitionStatus} \\
& \square \text{SetOperatingMode} \\
& \square \text{GetProcessId} \\
& \square \text{GetProcessStatus} \\
& \square \text{CreateProcess} \\
& \square \text{SetPriority} \\
& \square \text{SuspendSelf} \\
& \square \text{Suspend} \\
& \square \text{Resume} \\
& \square \text{StopSelf} \\
& \square \text{Stop} \\
& \square \text{Start} \\
& \square \text{DelayedStart} \\
& \square \text{LockPreemption} \\
& \square \text{UnlockPreemption} \\
& \square \text{GetMyId} \\
& \square \text{TimedWait} \\
& \square \text{PeriodicWait} \\
& \square \text{GetTime} \\
& \square \text{Replenish}
\end{aligned}$$

$$\text{ExecAPEXService} \quad \hat{=} \quad \mu X \bullet \text{APEXService} ; X$$

$$\bullet \text{ module\_init} \longrightarrow \text{ExecAPEXService} \Delta \text{ module\_end} \longrightarrow \text{Skip}$$

end

## D.4.2 Application/Executive(APEX) Layer Model

**process**  $APEX\_Layer \hat{=} OSKernelConfig : OS\_KERNEL\_CONFIG\_TYPE \bullet$   
 $\begin{array}{l} \text{||| } partid : \text{dom}(OSKernelConfig.Partitions) \bullet \\ \text{||| } \text{procid} : 0 \dots (OSKernelConfig.Partitions(partid).TotalProcess) \bullet APEX(partid, procid) \end{array}$

## D.5 Core Module

### D.5.1 ChannelSets for communication between different layers of Core Module

**channelset**  $CH\_HIS == \{ \text{context\_switching\_save\_part\_cpu\_registers,}$   
 $\text{context\_switching\_saved\_part\_cpu\_registers,}$   
 $\text{context\_switching\_save\_all\_cpu\_registers, context\_switching\_saved\_all\_cpu\_registers,}$   
 $\text{context\_switching\_restore\_part\_cpu\_registers,}$   
 $\text{context\_switching\_restored\_part\_cpu\_registers,}$   
 $\text{context\_switching\_restore\_all\_cpu\_registers,}$   
 $\text{context\_switching\_restored\_all\_cpu\_registers,}$   
 $\text{context\_switching\_set\_stack\_segment\_registers,}$   
 $\text{context\_switching\_have\_set\_stack\_segment\_registers,}$   
 $\text{interrupt\_controlling\_enable\_interrupt, interrupt\_controlling\_enabled\_interrupt,}$   
 $\text{interrupt\_controlling\_disable\_interrupt, interrupt\_controlling\_disabled\_interrupt,}$   
 $\text{interrupt\_handler\_start\_interrupt\_handling,}$   
 $\text{interrupt\_handler\_finish\_interrupt\_handling,}$   
 $\text{exception\_handler\_start\_exception\_handling,}$   
 $\text{exception\_handler\_finish\_exception\_handling,}$   
 $\text{context\_switching\_set\_page\_table, context\_switching\_have\_set\_page\_table,}$   
 $\text{context\_switching\_request\_page\_table, context\_switching\_get\_page\_table,}$   
 $\text{memory\_management\_load\_page\_into\_main\_memory,}$   
 $\text{memory\_management\_loaded\_page\_into\_main\_memory,}$   
 $\text{memory\_management\_extract\_page\_from\_main\_memory,}$   
 $\text{memory\_management\_extracted\_page\_from\_main\_memory,}$   
 $\text{system\_clock\_request\_current\_time, system\_clock\_get\_current\_time,}$   
 $\text{system\_clock\_request\_high\_precision\_time, system\_clock\_get\_high\_precision\_time,}$   
 $\text{system\_clock\_set\_high\_precision\_timer\_alarm,}$   
 $\text{system\_clock\_have\_set\_high\_precision\_timer\_alarm,}$   
 $\text{system\_clock\_reset\_high\_precision\_timer,}$   
 $\text{system\_clock\_have\_reset\_high\_precision\_timer,}$   
 $\text{system\_clock\_end\_high\_precision\_timer, system\_clock\_ended\_high\_precision\_timer,}$   
 $\text{interrupt\_controlling\_mask\_interrupt, interrupt\_controlling\_masked\_interrupt,}$   
 $\text{interrupt\_controlling\_unmask\_interrupt, interrupt\_controlling\_unmasked\_interrupt} \}$



```

channelset HIS_OS == {
    kernel_save_context, kernel_saved_context,
    kernel_restore_context, kernel_restored_context,
    kernel_switch_stack, kernel_switched_stack,
    kernel_init_memory_management, kernel_init_memory_management,
    kernel_set_area_memory_management_reference,
    kernel_have_set_area_memory_management_reference,
    kernel_request_area_memory_management_reference,
    kernel_get_area_memory_management_reference,
    kernel_request_area_free_pages, kernel_get_area_free_pages,
    kernel_request_area_free_block, kernel_get_area_free_block,
    kernel_allocate_area_free_pages, kernel_allocated_area_free_pages,
    kernel_allocate_area_free_block, kernel_allocated_area_free_block,
    kernel_deallocate_area_used_pages, kernel_deallocated_area_used_pages,
    kernel_deallocate_area_used_block, kernel_deallocated_area_used_block,
    kernel_create_virtual_memory_block, kernel_created_virtual_memory_block,
    kernel_create_process_virtual_memory, kernel_created_process_virtual_memory,
    kernel_full_load_process_pages, kernel_full_loaded_process_pages,
    kernel_init_system_clock, kernel_init_system_clock,
    kernel_request_system_time, kernel_get_system_time,
    kernel_request_high_precision_time, kernel_get_high_precision_time,
    kernel_reset_high_precision_timer, kernel_have_reset_high_precision_timer,
    kernel_set_high_precision_timer_alarm, kernel_have_set_high_precision_timer_alarm,
    kernel_end_high_precision_timer, kernel_ended_high_precision_timer,
    kernel_request_interrupt_time, kernel_get_interrupt_time,
    kernel_mask_interrupt, kernel_masked_interrupt,
    kernel_unmask_interrupt, kernel_unmasked_interrupt,
    kernel_enable_interrupt, kernel_enabled_interrupt,
    kernel_disable_interrupt, kernel_disabled_interrupt,
    kernel_init_interrupt_handler, interrupt_handler_request_interrupt_stack,
    interrupt_handler_get_interrupt_stack, kernel_init_interrupt_handler,
    interrupt_handler_invoke_kernel, kernel_continue_interrupted_process,
    kernel_request_interrupted_process_context, kernel_get_interrupted_process_context }

```

```

channelset OS_APEX == { system_call,
    system_call_service_routine_get_operating_mode_output,
    system_call_service_routine_get_partition_status_output,
    system_call_service_routine_set_operating_mode_input,
    system_call_service_routine_get_process_names_output,
    system_call_service_routine_get_process_ids_output,
    system_call_service_routine_get_free_process_ids_output,
    system_call_service_routine_get_free_space_output,
    system_call_service_routine_get_partition_period_output,
    system_call_service_routine_get_process_state_input,
    system_call_service_routine_get_process_state_output,
    system_call_service_routine_get_next_periodic_start_output,
    system_call_service_routine_get_delayed_periodic_start_input,
    system_call_service_routine_get_delayed_periodic_start_output,
    system_call_service_routine_get_process_kind_input,
    system_call_service_routine_get_process_kind_output,
    system_call_service_routine_get_process_period_input,
    system_call_service_routine_get_process_period_output,
    system_call_service_routine_get_process_time_capacity_input,
    system_call_service_routine_get_process_time_capacity_output,
    system_call_service_routine_get_partition_lock_level_output,
    system_call_service_routine_get_process_id_input,
    system_call_service_routine_get_process_id_output,
    system_call_service_routine_get_process_status_input,
    system_call_service_routine_get_process_status_output,
    system_call_service_routine_create_process_input,
    system_call_service_routine_create_process_output,
    system_call_service_routine_set_priority_input,
    system_call_service_routine_suspend_self_input,
    system_call_service_routine_suspend_self_output,
    system_call_service_routine_suspend_input,
    system_call_service_routine_suspend_output,
    system_call_service_routine_resume_input,
    system_call_service_routine_stop_input,
    system_call_service_routine_start_input,
    system_call_service_routine_delayed_start_input,
    system_call_service_routine_lock_preemption_output,
    system_call_service_routine_unlock_preemption_output,
    system_call_service_routine_get_my_id_output,
    system_call_service_routine_get_current_time_output,
    system_call_service_routine_get_partition_time_output,
    system_call_service_routine_get_next_release_point_input,
    system_call_service_routine_get_next_release_point_output,
    system_call_service_routine_timed_wait_input,
    system_call_service_routine_periodic_wait_input,
    system_call_service_routine_get_time_output,
    system_call_service_routine_replenish_input,
    system_call_return }

```

### D.5.2 Core Module Model

**process** *CoreModule*  $\hat{=}$  *ModuleConfig* : *MODULE\_CONFIG\_TYPE* •

*Core\_Hardware\_Layer*  $\llbracket$  *CH\_HIS*  $\rrbracket$  *Hardware\_Interface\_Software\_Layer*(*ModuleConfig.InterruptHandlerConfig*)  
 $\llbracket$  *HIS\_OS*  $\rrbracket$  *ARINC653\_OS\_Layer*(*ModuleConfig.OSKernelConfig*)  $\llbracket$  *OS\_APEX*  $\rrbracket$  *APEX\_Layer*(*ModuleConfig.OSKernelConfig*)
